# Supplementary material for: Isoscalar $\pi\pi, K\overline{K}, \eta\eta$ scattering and the $\sigma, f_0, f_2$ mesons from QCD
Source: arXiv:1708.06667 source file (2017-08-20)
Supplement: Supplementary file 1 [file SupplementalMaterial.pdf]

## Operator Lists

|                                 |                                 |                                 |                                 |                                 |                                 |                                 |                                 |                                  |                                 |                                 |                                 | [200] $A_1$                     |                                 |                                 |
|---------------------------------|---------------------------------|---------------------------------|---------------------------------|---------------------------------|---------------------------------|---------------------------------|---------------------------------|----------------------------------|---------------------------------|---------------------------------|---------------------------------|---------------------------------|---------------------------------|---------------------------------|
| [000] $A_1^+$                   |                                 |                                 | [100] $A_1$                     |                                 |                                 | [110] $A_1$                     |                                 |                                  | [111] $A_1$                     |                                 |                                 | 24 <sup>3</sup>                 | 20 <sup>3</sup>                 | 16 <sup>3</sup>                 |
| 24 <sup>3</sup>                 | 20 <sup>3</sup>                 | 16 <sup>3</sup>                 | 24 <sup>3</sup>                 | 20 <sup>3</sup>                 | 16 <sup>3</sup>                 | 24 <sup>3</sup>                 | 20 <sup>3</sup>                 | 16 <sup>3</sup>                  | 24 <sup>3</sup>                 | 20 <sup>3</sup>                 | 16 <sup>3</sup>                 | $\pi_0\pi_4$                    | $\pi_0\pi_4$                    | $\pi_0\pi_4$                    |
| $\pi_0\pi_0$                    | $\pi_0\pi_0$                    | $\pi_0\pi_0$                    | $\pi_0\pi_1$                    | $\pi_0\pi_1$                    | $\pi_0\pi_1$                    | $\pi_0\pi_2$                    | $\pi_0\pi_2$                    | $\pi_0\pi_2$                     | $\pi_0\pi_3$                    | $\pi_0\pi_3$                    | $\pi_0\pi_3$                    | $\pi_1\pi_1$                    | $\pi_1\pi_1$                    | $\pi_1\pi_1$                    |
| $\pi_1\pi_1$                    | $\pi_1\pi_1$                    | $\pi_1\pi_1$                    | $\pi_1\pi_2$                    | $\pi_1\pi_2$                    | $\pi_1\pi_2$                    | $\pi_1\pi_3$                    | $\pi_1\pi_3$                    | $\pi_1\pi_3$                     | $\pi_1\pi_2$                    | $\pi_1\pi_2$                    | $\pi_1\pi_2$                    | $\pi_2\pi_2$                    | $\pi_2\pi_2$                    | $\pi_2\pi_2$                    |
| $\pi_2\pi_2$                    | $\pi_2\pi_2$                    | $\pi_2\pi_2$                    | $\pi_1\pi_4$                    |                                 |                                 | $\pi_2\pi_2$                    | $\pi_2\pi_2$                    |                                  | $\pi_3\pi_4$                    |                                 | $\pi_3\pi_4$                    | $\pi_3\pi_3$                    | $\pi_3\pi_3$                    |                                 |
| $K_0\bar{K}_0$                  | $K_0\bar{K}_0$                  | $K_0\bar{K}_0$                  | $K_0\bar{K}_1$                  | $K_0\bar{K}_1$                  | $K_0\bar{K}_1$                  | $K_0\bar{K}_2$                  | $K_0\bar{K}_2$                  | $K_0\bar{K}_2$                   | $K_0\bar{K}_3$                  | $K_0\bar{K}_3$                  | $K_0\bar{K}_3$                  | $K_0\bar{K}_4$                  | $K_0\bar{K}_4$                  | $K_0\bar{K}_4$                  |
| $K_1\bar{K}_1$                  | $K_1\bar{K}_1$                  | $K_1\bar{K}_1$                  | $K_1\bar{K}_2$                  | $K_1\bar{K}_2$                  |                                 | $K_1\bar{K}_1$                  | $K_1\bar{K}_1$                  | $K_1\bar{K}_1$                   | $K_1\bar{K}_2$                  | $K_1\bar{K}_2$                  | $K_1\bar{K}_2$                  | $K_1\bar{K}_1$                  | $K_1\bar{K}_1$                  | $K_1\bar{K}_1$                  |
|                                 |                                 |                                 |                                 |                                 |                                 |                                 |                                 |                                  |                                 |                                 |                                 | $K_2\bar{K}_2$                  | $K_2\bar{K}_2$                  |                                 |
| $\eta_0\eta_0$                  | $\eta_0\eta_0$                  | $\eta_0\eta_0$                  | $\eta_0\eta_1$                  | $\eta_0\eta_1$                  | $\eta_0\eta_1$                  | $\eta_0\eta_2$                  | $\eta_0\eta_2$                  | $\eta_0\eta_2$                   | $\eta_0\eta_3$                  | $\eta_0\eta_3$                  | $\eta_0\eta_3$                  | $\eta_0\eta_4$                  | $\eta_0\eta_4$                  | $\eta_0\eta_4$                  |
| $\bar{\ell}\Gamma\ell \times 4$ | $\bar{\ell}\Gamma\ell \times 4$ | $\bar{\ell}\Gamma\ell \times 6$ | $\eta_1\eta_2$                  |                                 |                                 | $\eta_1\eta_1$                  | $\eta_1\eta_1$                  | $\eta_1\eta_1$                   | $\eta_1\eta_2$                  | $\eta_1\eta_2$                  | $\eta_1\eta_2$                  | $\eta_1\eta_1$                  | $\eta_1\eta_1$                  | $\eta_1\eta_1$                  |
| $\bar{s}\Gamma s \times 4$      | $\bar{s}\Gamma s \times 4$      | $\bar{s}\Gamma s \times 6$      | $\bar{\ell}\Gamma\ell \times 4$ | $\bar{\ell}\Gamma\ell \times 4$ | $\bar{\ell}\Gamma\ell \times 8$ | $\bar{\ell}\Gamma\ell \times 3$ | $\bar{\ell}\Gamma\ell \times 7$ | $\bar{\ell}\Gamma\ell \times 12$ | $\bar{\ell}\Gamma\ell \times 5$ | $\bar{\ell}\Gamma\ell \times 3$ | $\bar{\ell}\Gamma\ell \times 9$ | $\eta_2\eta_2$                  | $\eta_2\eta_2$                  |                                 |
|                                 |                                 |                                 | $\bar{s}\Gamma s \times 4$      | $\bar{s}\Gamma s \times 4$      | $\bar{s}\Gamma s \times 8$      | $\bar{s}\Gamma s \times 3$      | $\bar{s}\Gamma s \times 7$      | $\bar{s}\Gamma s \times 12$      | $\bar{s}\Gamma s \times 5$      | $\bar{s}\Gamma s \times 3$      | $\bar{s}\Gamma s \times 9$      | $\bar{\ell}\Gamma\ell \times 5$ | $\bar{\ell}\Gamma\ell \times 6$ | $\bar{\ell}\Gamma\ell \times 8$ |
|                                 |                                 |                                 |                                 |                                 |                                 |                                 |                                 |                                  |                                 |                                 |                                 | $\bar{s}\Gamma s \times 5$      | $\bar{s}\Gamma s \times 6$      | $\bar{s}\Gamma s \times 8$      |

[illegible]

## $J^P = 0^+$ Amplitudes

### Inverse of $\mathbf{K}$ as a polynomial

Amplitudes with names of the form `k_inv_poly_ABCDEF` are of the form

$$\mathbf{K}^{-1}(s) = \begin{pmatrix} A(s) & B(s) & C(s) \\ B(s) & D(s) & E(s) \\ C(s) & E(s) & F(s) \end{pmatrix} \quad (1)$$

with row/column ordering  $\pi\pi, K\bar{K}, \eta\eta$ . The encoding of  $A \dots F$  indicates the order of the polynomial used in the relevant element, e.g.

$$\begin{aligned} \mathbf{A}=\mathbf{x} &\implies A(s) = 0 \\ \mathbf{A}=\mathbf{c} &\implies A(s) = \text{const} \\ \mathbf{A}=\mathbf{l} &\implies A(s) = a + b s \\ \mathbf{A}=\mathbf{q} &\implies A(s) = a + b s + c s^2 \\ \mathbf{A}=\mathbf{s} &\implies A(s) = b s \end{aligned}$$

If the amplitude name features `_noCM`, the naive phase-space is used,  $I_{ij}(s) = -\rho_i(s)\delta_{ij}$ , otherwise the Chew-Mandelstam phase-space subtracted at threshold is used.

The parameter names should be self-explanatory: e.g.

`JP0+_c_kaon:kaon/1^S_0|pi:pi/1^S_0_order0`, `JP0+_c_kaon:kaon/1^S_0|pi:pi/1^S_0_order1`

appear in a  $B(s) = a + b s$  element as  $a, b$  respectively.

## K as a polynomial

Amplitudes with names of the form `k_ABCDEF` are of the form

$$\mathbf{K}(s) = \begin{pmatrix} A(s) & B(s) & C(s) \\ B(s) & D(s) & E(s) \\ C(s) & E(s) & F(s) \end{pmatrix} \quad (2)$$

with row/column ordering  $\pi\pi, K\bar{K}, \eta\eta$ . The encoding of  $A \dots F$  indicates the order of the polynomial used in the relevant element, e.g.

$$\begin{aligned} \mathbf{A}=\mathbf{x} &\implies A(s) = 0 \\ \mathbf{A}=\mathbf{c} &\implies A(s) = \text{const} \\ \mathbf{A}=\mathbf{l} &\implies A(s) = a + b s \\ \mathbf{A}=\mathbf{q} &\implies A(s) = a + b s + c s^2 \\ \mathbf{A}=\mathbf{s} &\implies A(s) = b s \end{aligned}$$

If the amplitude name features `_noCM`, the naive phase-space is used,  $I_{ij}(s) = -\rho_i(s)\delta_{ij}$ , otherwise the Chew-Mandelstam phase-space subtracted at threshold is used.

The parameter names should be self-explanatory: e.g.

`JP0+_gamma_pi:pi/1^S_0|pi:pi/1^S_0_order0`, `JP0+_gamma_pi:pi/1^S_0|pi:pi/1^S_0_order1`

appear in an  $A(s) = a + b s$  element as  $a, b$  respectively.

### K as a pole plus a polynomial

Amplitudes with names of the form `k_sigma_pole_ABCDEF` are of the form

$$\mathbf{K}(s) = \frac{1}{m^2 - s} \begin{pmatrix} g_{\pi\pi}^2 & g_{\pi\pi}g_{K\bar{K}} & g_{\pi\pi}g_{\eta\eta} \\ g_{\pi\pi}g_{K\bar{K}} & g_{K\bar{K}}^2 & g_{K\bar{K}}g_{\eta\eta} \\ g_{\pi\pi}g_{\eta\eta} & g_{K\bar{K}}g_{\eta\eta} & g_{\eta\eta}^2 \end{pmatrix} + \begin{pmatrix} A(s) & B(s) & C(s) \\ B(s) & D(s) & E(s) \\ C(s) & E(s) & F(s) \end{pmatrix} \quad (3)$$

with row/column ordering  $\pi\pi, K\bar{K}, \eta\eta$ . The encoding of  $A \dots F$  indicates the order of the polynomial used in the relevant element, e.g.

$$\begin{aligned} \mathbf{A}=\mathbf{x} &\implies A(s) = 0 \\ \mathbf{A}=\mathbf{c} &\implies A(s) = \text{const} \\ \mathbf{A}=\mathbf{l} &\implies A(s) = a + b\,s \\ \mathbf{A}=\mathbf{q} &\implies A(s) = a + b\,s + c\,s^2 \\ \mathbf{A}=\mathbf{s} &\implies A(s) = b\,s \end{aligned}$$

If the amplitude name features `_noCM`, the naive phase-space is used,  $I_{ij}(s) = -\rho_i(s)\delta_{ij}$ , otherwise the Chew-Mandelstam phase-space subtracted **at the  $K$ -matrix pole position**,  $s = m^2$ .

The parameter names should be self-explanatory.

$$a_t E_{\text{cm}} < 0.24$$

# k\_inv\_poly\_llcccc

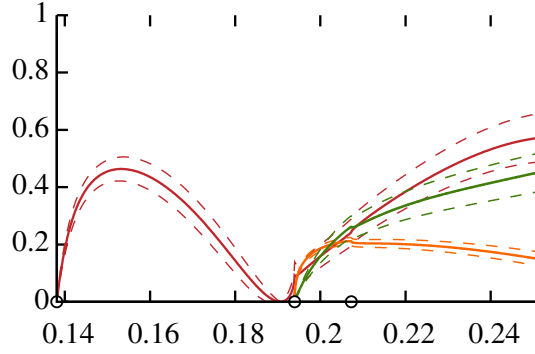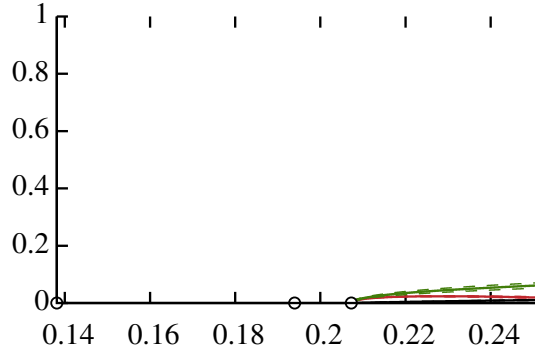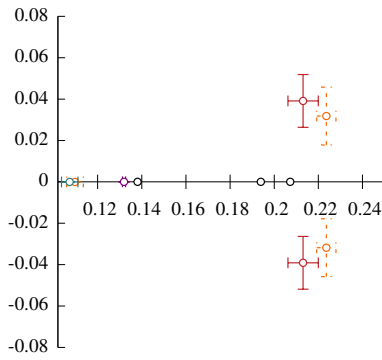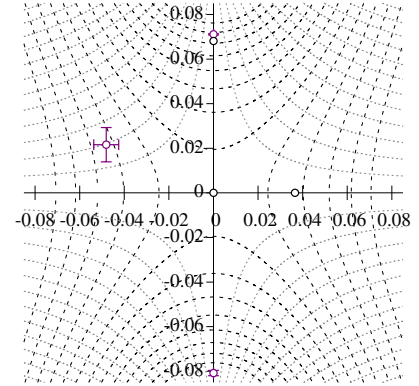

## parameter values

minimised with  $\text{chisq}/\text{nDoF} = 44.10 / (57 - 8) = 0.90$

|                                               |  |                       |  |      |      |      |      |       |       |       |       |
|-----------------------------------------------|--|-----------------------|--|------|------|------|------|-------|-------|-------|-------|
| JP0+_c_eta:eta/1^S_0 eta:eta/1^S_0_order0     |  | 21.665 +/- 0.38655    |  | 1.00 | 0.71 | 0.06 | 0.06 | -0.05 | 0.09  | -0.03 | -0.00 |
| JP0+_c_eta:eta/1^S_0 kaon:kaon/1^S_0_order0   |  | 8.4603 +/- 0.10569    |  |      | 1.00 | 0.13 | 0.62 | -0.17 | 0.04  | -0.08 | 0.04  |
| JP0+_c_eta:eta/1^S_0 pi:pi/1^S_0_order0       |  | 1.0390 +/- 0.10605    |  |      |      | 1.00 | 0.01 | 0.46  | 0.30  | -0.25 | 0.23  |
| JP0+_c_kaon:kaon/1^S_0 kaon:kaon/1^S_0_order0 |  | 3.0897 +/- 0.048207   |  |      |      |      | 1.00 | 0.01  | 0.11  | -0.05 | 0.02  |
| JP0+_c_kaon:kaon/1^S_0 pi:pi/1^S_0_order0     |  | 1.0965 +/- 0.044007   |  |      |      |      |      | 1.00  | -0.32 | 0.45  | -0.26 |
| JP0+_c_kaon:kaon/1^S_0 pi:pi/1^S_0_order1     |  | -0.15923 +/- 0.049964 |  |      |      |      |      |       | 1.00  | -0.35 | 0.21  |
| JP0+_c_pi:pi/1^S_0 pi:pi/1^S_0_order0         |  | 1.4470 +/- 0.10499    |  |      |      |      |      |       |       | 1.00  | -0.86 |
| JP0+_c_pi:pi/1^S_0 pi:pi/1^S_0_order1         |  | -1.3163 +/- 0.10139   |  |      |      |      |      |       |       |       | 1.00  |

## pole singularities

\*\*\*\*\*  
JP=0+ || eta:eta/1^S\_0[+] kaon:kaon/1^S\_0[+] pi:pi/1^S\_0[+]

$\text{sqrt}(s)_{\text{pole}} = (0.13197 \pm 0.00071527) + (i/2) * (5.0066e-13 \pm 1.4595e-10) [0.05]$

| eta:eta/1^S_0                | kaon:kaon/1^S_0              | pi:pi/1^S_0                   |
|------------------------------|------------------------------|-------------------------------|
| k_re= 0.0000 +/- 0.0000      | k_re= 0.0000 +/- 0.0000      | k_re= 0.0000 +/- 0.0000       |
| k_im= 0.0799 +/- 0.0003      | k_im= 0.0711 +/- 0.0003      | k_im= 0.0204 +/- 0.0012       |
| corr= [-0.05]                | corr= [-0.05]                | corr= [-0.05]                 |
| g = 0.0551 +/- 0.0038        | g = 0.1561 +/- 0.0092        | g = 0.0942 +/- 0.0029         |
| arg(g)/pi= 0.0000 +/- 0.0000 | arg(g)/pi= 1.0000 +/- 0.0000 | arg(g)/pi= -0.0000 +/- 0.0000 |
| g_re= 0.0551 +/- 0.0038      | g_re= -0.1561 +/- 0.0092     | g_re= 0.0942 +/- 0.0029       |
| g_im= 0.0000 +/- 0.0000      | g_im= 0.0000 +/- 0.0000      | g_im= -0.0000 +/- 0.0000      |
| corr= [-1.00]                | corr= [0.94]                 | corr= [0.01]                  |

\*\*\*\*\*  
JP=0+ || eta:eta/1^S\_0[+] kaon:kaon/1^S\_0[+] pi:pi/1^S\_0[-]

$\text{sqrt}(s)_{\text{pole}} = (0.21308 \pm 0.0068791) + (i/2) * (-0.039116 \pm 0.012777) [0.59]$

| eta:eta/1^S_0 | kaon:kaon/1^S_0 | pi:pi/1^S_0 |
|---------------|-----------------|-------------|
|---------------|-----------------|-------------|

```

=====|=====|=====|
k_re= -0.0365 +/- 0.0054 | k_re= -0.0481 +/- 0.0056 | k_re= 0.0815 +/- 0.0043 |
k_im= 0.0286 +/- 0.0094 | k_im= 0.0216 +/- 0.0077 | k_im= -0.0128 +/- 0.0043 |
corr= [ 0.36] | corr= [ 0.53] | corr= [ 0.59] |
=====|=====|=====|
|g|= 0.0770 +/- 0.0108 | |g|= 0.2059 +/- 0.0307 | |g|= 0.1666 +/- 0.0223 |
arg(g)/pi= 0.3277 +/- 0.0420 | arg(g)/pi= -0.6381 +/- 0.0452 | arg(g)/pi= 0.7483 +/- 0.0764 |
=====|=====|=====|
g_re= 0.0397 +/- 0.0126 | g_re= -0.0865 +/- 0.0352 | g_re= -0.1172 +/- 0.0263 |
g_im= 0.0660 +/- 0.0079 | g_im= -0.1868 +/- 0.0237 | g_im= 0.1184 +/- 0.0375 |
corr= [ 0.34] | corr= [ 0.41] | corr= [ 0.56] |
=====|=====|=====|
*****

```

```

*****
JP=0+ || eta:eta/1^S_0[+] kaon:kaon/1^S_0[-] pi:pi/1^S_0[-]

```

```

sqrt(s)_pole = (0.10735 +/- 0.0037341)
+ (i/2)*(-1.7471e-13 +/- 5.2208e-11) [ 0.02]

```

```

=====|=====|=====|
eta:eta/1^S_0 | kaon:kaon/1^S_0 | pi:pi/1^S_0 |
=====|=====|=====|
k_re= -0.0000 +/- 0.0000 | k_re= 0.0000 +/- 0.0000 | k_re= 0.0000 +/- 0.0000 |
k_im= 0.0887 +/- 0.0011 | k_im= -0.0808 +/- 0.0012 | k_im= -0.0435 +/- 0.0023 |
corr= [-0.02] | corr= [-0.02] | corr= [-0.02] |
=====|=====|=====|
|g|= 0.0126 +/- 0.0008 | |g|= 0.0223 +/- 0.0013 | |g|= 0.0880 +/- 0.0034 |
arg(g)/pi= 0.5000 +/- 0.0000 | arg(g)/pi= -0.5000 +/- 0.0000 | arg(g)/pi= -0.5000 +/- 0.0000 |
=====|=====|=====|
g_re= 0.0000 +/- 0.0000 | g_re= 0.0000 +/- 0.0000 | g_re= 0.0000 +/- 0.0000 |
g_im= 0.0126 +/- 0.0008 | g_im= -0.0223 +/- 0.0013 | g_im= -0.0880 +/- 0.0034 |
corr= [-1.00] | corr= [ 0.42] | corr= [ 0.58] |
=====|=====|=====|
*****

```

```

*****
JP=0+ || eta:eta/1^S_0[+] kaon:kaon/1^S_0[-] pi:pi/1^S_0[-]

```

```

sqrt(s)_pole = (0.25907 +/- 0.00703)
+ (i/2)*(-0.14346 +/- 0.013452) [-0.39]

```

```

=====|=====|=====|
eta:eta/1^S_0 | kaon:kaon/1^S_0 | pi:pi/1^S_0 |
=====|=====|=====|
k_re= -0.0871 +/- 0.0051 | k_re= 0.0927 +/- 0.0048 | k_re= 0.1116 +/- 0.0041 |
k_im= 0.0533 +/- 0.0039 | k_im= -0.0501 +/- 0.0039 | k_im= -0.0416 +/- 0.0037 |
corr= [-0.32] | corr= [-0.34] | corr= [-0.38] |
=====|=====|=====|
|g|= 0.0357 +/- 0.0017 | |g|= 0.0854 +/- 0.0075 | |g|= 0.1794 +/- 0.0077 |
arg(g)/pi= -0.3228 +/- 0.0482 | arg(g)/pi= 0.6108 +/- 0.0482 | arg(g)/pi= -0.9753 +/- 0.0029 |
=====|=====|=====|
g_re= 0.0189 +/- 0.0038 | g_re= -0.0291 +/- 0.0097 | g_re= -0.1788 +/- 0.0076 |
g_im= -0.0303 +/- 0.0042 | g_im= 0.0803 +/- 0.0114 | g_im= -0.0139 +/- 0.0020 |
corr= [ 0.97] | corr= [ 0.98] | corr= [ 0.70] |
=====|=====|=====|
*****

```

```

*****
JP=0+ || eta:eta/1^S_0[-] kaon:kaon/1^S_0[+] pi:pi/1^S_0[+]

```

```

sqrt(s)_pole = (0.14479 +/- 0.0058672)
+ (i/2)*(-0.13244 +/- 0.0075059) [-0.91]

```

```

=====|=====|=====|
eta:eta/1^S_0 | kaon:kaon/1^S_0 | pi:pi/1^S_0 |
=====|=====|=====|
k_re= 0.0279 +/- 0.0029 | k_re= -0.0305 +/- 0.0032 | k_re= -0.0459 +/- 0.0039 |
k_im= -0.0859 +/- 0.0010 | k_im= 0.0787 +/- 0.0009 | k_im= 0.0522 +/- 0.0009 |
corr= [ 0.80] | corr= [ 0.73] | corr= [-0.55] |
=====|=====|=====|
|g|= 0.0982 +/- 0.0055 | |g|= 0.2486 +/- 0.0133 | |g|= 0.0874 +/- 0.0037 |
arg(g)/pi= 0.2596 +/- 0.0055 | arg(g)/pi= -0.7693 +/- 0.0061 | arg(g)/pi= 0.0652 +/- 0.0139 |
=====|=====|=====|
g_re= 0.0673 +/- 0.0031 | g_re= -0.1861 +/- 0.0081 | g_re= 0.0856 +/- 0.0031 |
g_im= 0.0715 +/- 0.0048 | g_im= -0.1648 +/- 0.0116 | g_im= 0.0178 +/- 0.0044 |
corr= [ 0.88] | corr= [ 0.87] | corr= [ 0.78] |
=====|=====|=====|
*****

```

```

*****
JP=0+ || eta:eta/1^S_0[-] kaon:kaon/1^S_0[+] pi:pi/1^S_0[-]

```

```

sqrt(s)_pole = (0.22362 +/- 0.0043712)
+ (i/2)*(-0.031787 +/- 0.013969) [ 0.44]

```

```

=====|=====|=====|
eta:eta/1^S_0 | kaon:kaon/1^S_0 | pi:pi/1^S_0 |
=====|=====|=====|
k_re= 0.0456 +/- 0.0042 | k_re= -0.0572 +/- 0.0037 | k_re= 0.0882 +/- 0.0027 |
k_im= -0.0195 +/- 0.0083 | k_im= 0.0155 +/- 0.0069 | k_im= -0.0101 +/- 0.0045 |
corr= [ 0.05] | corr= [ 0.24] | corr= [ 0.40] |
=====|=====|=====|
|g|= 0.0744 +/- 0.0053 | |g|= 0.1932 +/- 0.0139 | |g|= 0.1468 +/- 0.0100 |
arg(g)/pi= 0.3881 +/- 0.0165 | arg(g)/pi= -0.5898 +/- 0.0172 | arg(g)/pi= 0.8435 +/- 0.0358 |
=====|=====|=====|
g_re= 0.0256 +/- 0.0045 | g_re= -0.0538 +/- 0.0116 | g_re= -0.1294 +/- 0.0089 |
g_im= 0.0699 +/- 0.0048 | g_im= -0.1856 +/- 0.0130 | g_im= 0.0693 +/- 0.0172 |
corr= [ 0.39] | corr= [ 0.34] | corr= [ 0.20] |
=====|=====|=====|
*****

```

```

*****
JP=0+ || eta:eta/1^S_0[-] kaon:kaon/1^S_0[+] pi:pi/1^S_0[-]

```

```

sqrt(s)_pole = (0.083902 +/- 0.0039024)

```

```

+ (i/2)*(+2.2922e-15 +/- 5.2426e-13) [-0.08]

eta:eta/1^S_0 | kaon:kaon/1^S_0 | pi:pi/1^S_0 |
=====|=====|=====|
k_re= -0.0000 +/- 0.0000 | k_re= 0.0000 +/- 0.0000 | k_re= -0.0000 +/- 0.0000 |
k_im= -0.0948 +/- 0.0009 | k_im= 0.0874 +/- 0.0009 | k_im= -0.0549 +/- 0.0015 |
corr= [ 0.08] | corr= [ 0.08] | corr= [ 0.08] |
=====|=====|=====|
|g|= 0.0383 +/- 0.0025 | |g|= 0.0747 +/- 0.0055 | |g|= 0.0458 +/- 0.0043 |
arg(g)/pi= 0.5000 +/- 0.0000 | arg(g)/pi= -0.5000 +/- 0.0000 | arg(g)/pi= -0.5000 +/- 0.0000 |
=====|=====|=====|
g_re= 0.0000 +/- 0.0000 | g_re= 0.0000 +/- 0.0000 | g_re= 0.0000 +/- 0.0000 |
g_im= 0.0383 +/- 0.0025 | g_im= -0.0747 +/- 0.0055 | g_im= -0.0458 +/- 0.0043 |
corr= [-1.00] | corr= [ 0.87] | corr= [-0.20] |
=====|=====|=====|
*****

```

```

*****
JP=0+ || eta:eta/1^S_0[-] kaon:kaon/1^S_0[-] pi:pi/1^S_0[-]

```

```

sqrt(s)_pole = (0.25615 +/- 0.007047)
+ (i/2)*(-0.14136 +/- 0.012267) [-0.44]

```

```

eta:eta/1^S_0 | kaon:kaon/1^S_0 | pi:pi/1^S_0 |
=====|=====|=====|
k_re= 0.0851 +/- 0.0051 | k_re= 0.0908 +/- 0.0049 | k_re= 0.1099 +/- 0.0041 |
k_im= -0.0532 +/- 0.0035 | k_im= -0.0499 +/- 0.0035 | k_im= -0.0412 +/- 0.0033 |
corr= [-0.31] | corr= [-0.34] | corr= [-0.41] |
=====|=====|=====|
|g|= 0.0307 +/- 0.0016 | |g|= 0.0697 +/- 0.0072 | |g|= 0.1817 +/- 0.0077 |
arg(g)/pi= -0.2827 +/- 0.0460 | arg(g)/pi= 0.6152 +/- 0.0459 | arg(g)/pi= -0.9766 +/- 0.0025 |
=====|=====|=====|
g_re= 0.0193 +/- 0.0025 | g_re= -0.0247 +/- 0.0070 | g_re= -0.1812 +/- 0.0076 |
g_im= -0.0238 +/- 0.0040 | g_im= 0.0651 +/- 0.0101 | g_im= -0.0133 +/- 0.0019 |
corr= [ 0.96] | corr= [ 0.95] | corr= [ 0.81] |
=====|=====|=====|
*****

```

```

*****
JP=0+ || eta:eta/1^S_0[-] kaon:kaon/1^S_0[-] pi:pi/1^S_0[-]

```

```

sqrt(s)_pole = (0.10975 +/- 0.0037625)
+ (i/2)*(-2.4682e-12 +/- 7.384e-10) [ 0.02]

```

```

eta:eta/1^S_0 | kaon:kaon/1^S_0 | pi:pi/1^S_0 |
=====|=====|=====|
k_re= 0.0000 +/- 0.0000 | k_re= 0.0000 +/- 0.0000 | k_re= 0.0000 +/- 0.0000 |
k_im= -0.0879 +/- 0.0012 | k_im= -0.0800 +/- 0.0013 | k_im= -0.0419 +/- 0.0025 |
corr= [-0.02] | corr= [-0.02] | corr= [-0.02] |
=====|=====|=====|
|g|= 0.0127 +/- 0.0007 | |g|= 0.0175 +/- 0.0011 | |g|= 0.0908 +/- 0.0032 |
arg(g)/pi= 0.5000 +/- 0.0000 | arg(g)/pi= -0.5000 +/- 0.0000 | arg(g)/pi= -0.5000 +/- 0.0000 |
=====|=====|=====|
g_re= 0.0000 +/- 0.0000 | g_re= 0.0000 +/- 0.0000 | g_re= 0.0000 +/- 0.0000 |
g_im= 0.0127 +/- 0.0007 | g_im= -0.0175 +/- 0.0011 | g_im= -0.0908 +/- 0.0032 |
corr= [-1.00] | corr= [ 0.06] | corr= [ 0.47] |
=====|=====|=====|
*****

```



# k\_inv\_poly\_lcccc

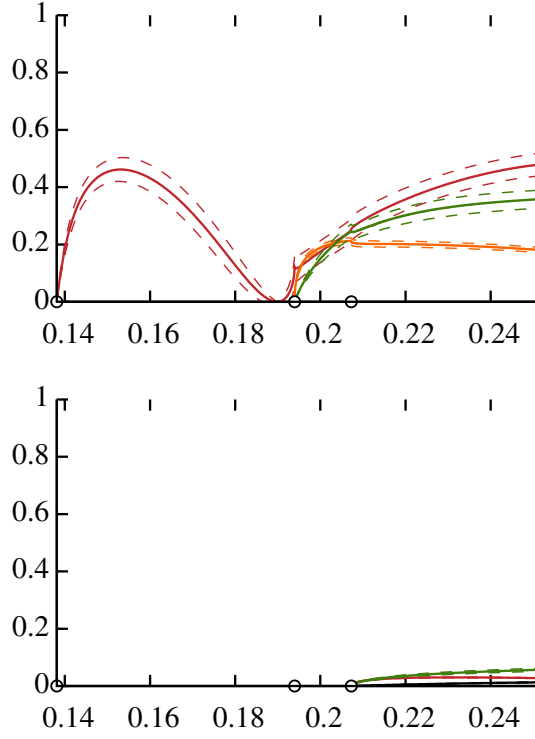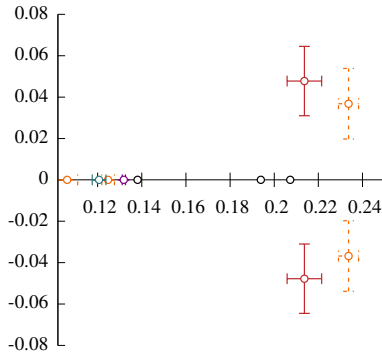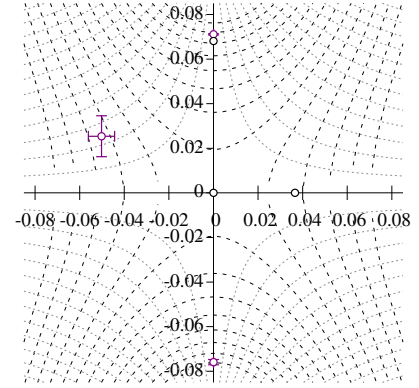

## parameter values

minimised with  $\text{chisq}/\text{nDoF} = 45.81 / (57 - 7) = 0.92$

|                                               |  |                      |  |      |      |      |       |       |       |       |
|-----------------------------------------------|--|----------------------|--|------|------|------|-------|-------|-------|-------|
| JPO+_c_eta:eta/1^S_0 eta:eta/1^S_0_order0     |  | 20.323 +/- 0.53781   |  | 1.00 | 0.79 | 0.09 | 0.11  | -0.10 | -0.01 | -0.03 |
| JPO+_c_eta:eta/1^S_0 kaon:kaon/1^S_0_order0   |  | 8.5604 +/- 0.1469    |  |      | 1.00 | 0.11 | 0.62  | -0.12 | -0.10 | 0.03  |
| JPO+_c_eta:eta/1^S_0 pi:pi/1^S_0_order0       |  | 2.1489 +/- 0.12233   |  |      |      | 1.00 | -0.04 | 0.74  | -0.04 | 0.21  |
| JPO+_c_kaon:kaon/1^S_0 kaon:kaon/1^S_0_order0 |  | 3.3675 +/- 0.06568   |  |      |      |      | 1.00  | 0.08  | -0.04 | -0.00 |
| JPO+_c_kaon:kaon/1^S_0 pi:pi/1^S_0_order0     |  | 1.4169 +/- 0.051195  |  |      |      |      |       | 1.00  | 0.43  | -0.14 |
| JPO+_c_pi:pi/1^S_0 pi:pi/1^S_0_order0         |  | 1.2101 +/- 0.099134  |  |      |      |      |       |       | 1.00  | -0.85 |
| JPO+_c_pi:pi/1^S_0 pi:pi/1^S_0_order1         |  | -0.99764 +/- 0.10409 |  |      |      |      |       |       |       | 1.00  |

## pole singularities

\*\*\*\*\*  
JP=0+ || eta:eta/1^S\_0[+] kaon:kaon/1^S\_0[+] pi:pi/1^S\_0[+]

$\text{sqrt}(s)_{\text{pole}} = (0.13187 \pm 0.00075136) + (i/2) * (1.224e-12 \pm 3.6166e-10) [0.02]$

| eta:eta/1^S_0                | kaon:kaon/1^S_0              | pi:pi/1^S_0                   |
|------------------------------|------------------------------|-------------------------------|
| k_re= 0.0000 +/- 0.0000      | k_re= 0.0000 +/- 0.0000      | k_re= 0.0000 +/- 0.0000       |
| k_im= 0.0800 +/- 0.0003      | k_im= 0.0711 +/- 0.0003      | k_im= 0.0205 +/- 0.0012       |
| corr= [-0.02]                | corr= [-0.02]                | corr= [-0.02]                 |
| g = 0.0469 +/- 0.0030        | g = 0.1382 +/- 0.0066        | g = 0.0948 +/- 0.0027         |
| arg(g)/pi= 0.0000 +/- 0.0000 | arg(g)/pi= 1.0000 +/- 0.0000 | arg(g)/pi= -0.0000 +/- 0.0000 |
| g_re= 0.0469 +/- 0.0030      | g_re= -0.1382 +/- 0.0066     | g_re= 0.0948 +/- 0.0027       |
| g_im= 0.0000 +/- 0.0000      | g_im= 0.0000 +/- 0.0000      | g_im= -0.0000 +/- 0.0000      |
| corr= [-1.00]                | corr= [0.88]                 | corr= [-0.27]                 |

\*\*\*\*\*  
JP=0+ || eta:eta/1^S\_0[+] kaon:kaon/1^S\_0[+] pi:pi/1^S\_0[-]

$\text{sqrt}(s)_{\text{pole}} = (0.21369 \pm 0.0078353) + (i/2) * (-0.047765 \pm 0.016768) [0.56]$

| eta:eta/1^S_0 | kaon:kaon/1^S_0 | pi:pi/1^S_0 |
|---------------|-----------------|-------------|
|---------------|-----------------|-------------|

|                          |                          |                          |
|--------------------------|--------------------------|--------------------------|
| k_re= -0.0396 +/- 0.0058 | k_re= -0.0502 +/- 0.0059 | k_re= 0.0821 +/- 0.0048  |
| k_im= 0.0322 +/- 0.0106  | k_im= 0.0254 +/- 0.0092  | k_im= -0.0155 +/- 0.0056 |
| corr= [ 0.20]            | corr= [ 0.42]            | corr= [ 0.55]            |

---

|                              |                               |                              |
|------------------------------|-------------------------------|------------------------------|
| g = 0.0997 +/- 0.0188        | g = 0.2522 +/- 0.0535         | g = 0.2031 +/- 0.0405        |
| arg(g)/pi= 0.2679 +/- 0.0688 | arg(g)/pi= -0.6638 +/- 0.0744 | arg(g)/pi= 0.7292 +/- 0.1056 |

---

|                         |                          |                          |
|-------------------------|--------------------------|--------------------------|
| g_re= 0.0664 +/- 0.0256 | g_re= -0.1241 +/- 0.0702 | g_re= -0.1339 +/- 0.0442 |
| g_im= 0.0743 +/- 0.0128 | g_im= -0.2195 +/- 0.0375 | g_im= 0.1527 +/- 0.0650  |
| corr= [-0.08]           | corr= [ 0.27]            | corr= [ 0.56]            |

JP=0+ || eta:eta/1^S\_0[+] kaon:kaon/1^S\_0[-] pi:pi/1^S\_0[-]

sqrt(s)\_pole = (0.12063 +/- 0.0030913)  
+ (i/2)\*(+1.0527e-16 +/- 3.6161e-14) [-0.04]

|                         |                          |                          |
|-------------------------|--------------------------|--------------------------|
| eta:eta/1^S_0           | kaon:kaon/1^S_0          | pi:pi/1^S_0              |
| k_re= 0.0000 +/- 0.0000 | k_re= -0.0000 +/- 0.0000 | k_re= -0.0000 +/- 0.0000 |
| k_im= 0.0843 +/- 0.0011 | k_im= -0.0759 +/- 0.0012 | k_im= -0.0336 +/- 0.0028 |
| corr= [ 0.04]           | corr= [ 0.04]            | corr= [ 0.04]            |

---

|                              |                               |                               |
|------------------------------|-------------------------------|-------------------------------|
| g = 0.0196 +/- 0.0007        | g = 0.0240 +/- 0.0011         | g = 0.0951 +/- 0.0013         |
| arg(g)/pi= 0.5000 +/- 0.0000 | arg(g)/pi= -0.5000 +/- 0.0000 | arg(g)/pi= -0.5000 +/- 0.0000 |

---

|                         |                          |                          |
|-------------------------|--------------------------|--------------------------|
| g_re= 0.0000 +/- 0.0000 | g_re= 0.0000 +/- 0.0000  | g_re= 0.0000 +/- 0.0000  |
| g_im= 0.0196 +/- 0.0007 | g_im= -0.0240 +/- 0.0011 | g_im= -0.0951 +/- 0.0013 |
| corr= [-1.00]           | corr= [-0.32]            | corr= [ 0.05]            |

JP=0+ || eta:eta/1^S\_0[-] kaon:kaon/1^S\_0[+] pi:pi/1^S\_0[+]

sqrt(s)\_pole = ( 0.143 +/- 0.0039936)  
+ (i/2)\*(-0.11698 +/- 0.006639) [-0.82]

|                          |                          |                          |
|--------------------------|--------------------------|--------------------------|
| eta:eta/1^S_0            | kaon:kaon/1^S_0          | pi:pi/1^S_0              |
| k_re= 0.0248 +/- 0.0021  | k_re= -0.0272 +/- 0.0023 | k_re= -0.0430 +/- 0.0029 |
| k_im= -0.0843 +/- 0.0008 | k_im= 0.0768 +/- 0.0008  | k_im= 0.0486 +/- 0.0011  |
| corr= [ 0.54]            | corr= [ 0.44]            | corr= [-0.53]            |

---

|                              |                               |                              |
|------------------------------|-------------------------------|------------------------------|
| g = 0.0964 +/- 0.0041        | g = 0.2306 +/- 0.0076         | g = 0.0819 +/- 0.0031        |
| arg(g)/pi= 0.2776 +/- 0.0050 | arg(g)/pi= -0.7645 +/- 0.0042 | arg(g)/pi= 0.0015 +/- 0.0159 |

---

|                         |                          |                         |
|-------------------------|--------------------------|-------------------------|
| g_re= 0.0620 +/- 0.0028 | g_re= -0.1703 +/- 0.0063 | g_re= 0.0819 +/- 0.0031 |
| g_im= 0.0739 +/- 0.0034 | g_im= -0.1555 +/- 0.0052 | g_im= 0.0004 +/- 0.0041 |
| corr= [ 0.76]           | corr= [ 0.72]            | corr= [ 0.75]           |

JP=0+ || eta:eta/1^S\_0[-] kaon:kaon/1^S\_0[+] pi:pi/1^S\_0[-]

sqrt(s)\_pole = (0.10617 +/- 0.0047771)  
+ (i/2)\*(+2.1596e-13 +/- 6.4371e-11) [ 0.05]

|                          |                         |                          |
|--------------------------|-------------------------|--------------------------|
| eta:eta/1^S_0            | kaon:kaon/1^S_0         | pi:pi/1^S_0              |
| k_re= -0.0000 +/- 0.0000 | k_re= 0.0000 +/- 0.0000 | k_re= -0.0000 +/- 0.0000 |
| k_im= -0.0890 +/- 0.0014 | k_im= 0.0812 +/- 0.0016 | k_im= -0.0442 +/- 0.0029 |
| corr= [-0.05]            | corr= [-0.05]           | corr= [-0.05]            |

---

|                              |                               |                               |
|------------------------------|-------------------------------|-------------------------------|
| g = 0.0532 +/- 0.0026        | g = 0.0934 +/- 0.0060         | g = 0.0623 +/- 0.0062         |
| arg(g)/pi= 0.5000 +/- 0.0000 | arg(g)/pi= -0.5000 +/- 0.0000 | arg(g)/pi= -0.5000 +/- 0.0000 |

---

|                         |                          |                          |
|-------------------------|--------------------------|--------------------------|
| g_re= 0.0000 +/- 0.0000 | g_re= 0.0000 +/- 0.0000  | g_re= 0.0000 +/- 0.0000  |
| g_im= 0.0532 +/- 0.0026 | g_im= -0.0934 +/- 0.0060 | g_im= -0.0623 +/- 0.0062 |
| corr= [-1.00]           | corr= [ 0.45]            | corr= [-0.63]            |

JP=0+ || eta:eta/1^S\_0[-] kaon:kaon/1^S\_0[+] pi:pi/1^S\_0[-]

sqrt(s)\_pole = (0.23366 +/- 0.0045629)  
+ (i/2)\*(-0.036805 +/- 0.017039) [-0.41]

|                          |                          |                          |
|--------------------------|--------------------------|--------------------------|
| eta:eta/1^S_0            | kaon:kaon/1^S_0          | pi:pi/1^S_0              |
| k_re= 0.0564 +/- 0.0055  | k_re= -0.0665 +/- 0.0045 | k_re= 0.0945 +/- 0.0029  |
| k_im= -0.0190 +/- 0.0077 | k_im= 0.0162 +/- 0.0070  | k_im= -0.0114 +/- 0.0052 |
| corr= [-0.60]            | corr= [-0.55]            | corr= [-0.45]            |

---

|                              |                               |                              |
|------------------------------|-------------------------------|------------------------------|
| g = 0.0964 +/- 0.0094        | g = 0.2331 +/- 0.0251         | g = 0.1791 +/- 0.0198        |
| arg(g)/pi= 0.3893 +/- 0.0140 | arg(g)/pi= -0.5581 +/- 0.0142 | arg(g)/pi= 0.8834 +/- 0.0246 |

---

|                         |                          |                          |
|-------------------------|--------------------------|--------------------------|
| g_re= 0.0329 +/- 0.0045 | g_re= -0.0423 +/- 0.0101 | g_re= -0.1672 +/- 0.0149 |
| g_im= 0.0906 +/- 0.0093 | g_im= -0.2293 +/- 0.0252 | g_im= 0.0641 +/- 0.0190  |
| corr= [ 0.38]           | corr= [ 0.13]            | corr= [-0.80]            |

JP=0+ || eta:eta/1^S\_0[-] kaon:kaon/1^S\_0[-] pi:pi/1^S\_0[-]

sqrt(s)\_pole = (0.12473 +/- 0.0028506)  
+ (i/2)\*(+2.8237e-16 +/- 7.9998e-14) [ 0.03]

| eta:eta/1^S_0                | kaon:kaon/1^S_0               | pi:pi/1^S_0                   |
|------------------------------|-------------------------------|-------------------------------|
| =====                        | =====                         | =====                         |
| k_re= -0.0000 +/- 0.0000     | k_re= -0.0000 +/- 0.0000      | k_re= -0.0000 +/- 0.0000      |
| k_im= -0.0828 +/- 0.0011     | k_im= -0.0743 +/- 0.0012      | k_im= -0.0297 +/- 0.0030      |
| corr= [-0.03]                | corr= [-0.03]                 | corr= [-0.03]                 |
| =====                        | =====                         | =====                         |
| g = 0.0187 +/- 0.0007        | g = 0.0156 +/- 0.0012         | g = 0.0961 +/- 0.0011         |
| arg(g)/pi= 0.5000 +/- 0.0000 | arg(g)/pi= -0.5000 +/- 0.0000 | arg(g)/pi= -0.5000 +/- 0.0000 |
| =====                        | =====                         | =====                         |
| g_re= 0.0000 +/- 0.0000      | g_re= 0.0000 +/- 0.0000       | g_re= 0.0000 +/- 0.0000       |
| g_im= 0.0187 +/- 0.0007      | g_im= -0.0156 +/- 0.0012      | g_im= -0.0961 +/- 0.0011      |
| corr= [-1.00]                | corr= [-0.64]                 | corr= [ 0.02]                 |
| =====                        | =====                         | =====                         |

\*\*\*\*\*

# k\_inv\_poly\_lcclcc

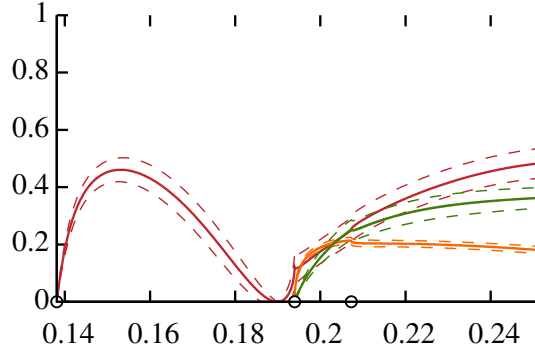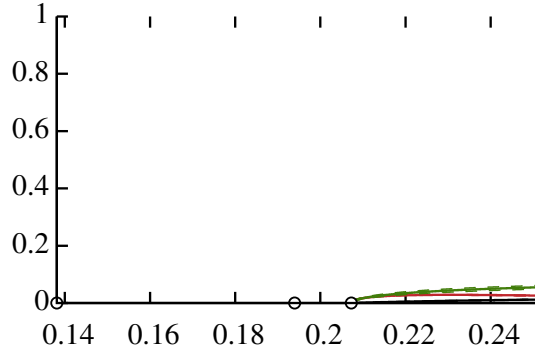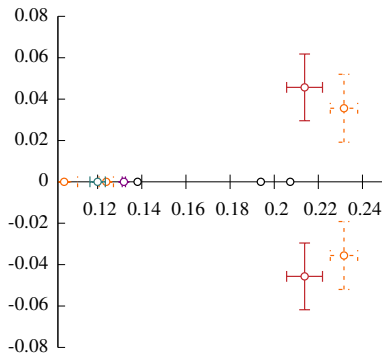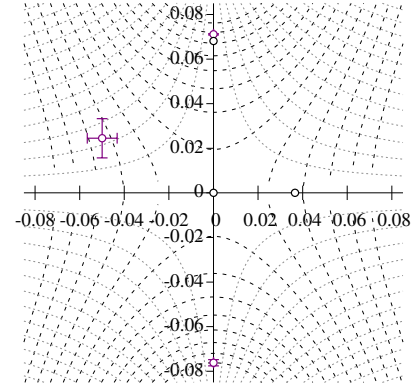

## parameter values

minimised with  $\text{chisq}/\text{nDoF} = 45.78 / (57 - 8) = 0.93$

|                                               |  |                       |  |      |      |      |       |       |       |       |       |
|-----------------------------------------------|--|-----------------------|--|------|------|------|-------|-------|-------|-------|-------|
| JPO+_c_eta:eta/1^S_0 eta:eta/1^S_0_order0     |  | 21.054 +/- 0.48523    |  | 1.00 | 0.60 | 0.09 | 0.06  | -0.15 | -0.05 | -0.06 | 0.00  |
| JPO+_c_eta:eta/1^S_0 kaon:kaon/1^S_0_order0   |  | 8.6619 +/- 0.1414     |  | 1.00 | 0.09 | 0.46 | 0.47  | -0.20 | 0.11  | -0.10 |       |
| JPO+_c_eta:eta/1^S_0 pi:pi/1^S_0_order0       |  | 2.1660 +/- 0.11335    |  |      |      | 1.00 | -0.05 | -0.02 | 0.70  | -0.08 | 0.22  |
| JPO+_c_kaon:kaon/1^S_0 kaon:kaon/1^S_0_order0 |  | 3.3032 +/- 0.057687   |  |      |      |      | 1.00  | -0.12 | 0.11  | -0.08 | 0.03  |
| JPO+_c_kaon:kaon/1^S_0 kaon:kaon/1^S_0_order1 |  | 0.026445 +/- 0.076432 |  |      |      |      |       | 1.00  | -0.21 | 0.39  | -0.25 |
| JPO+_c_kaon:kaon/1^S_0 pi:pi/1^S_0_order0     |  | 1.3995 +/- 0.047062   |  |      |      |      |       |       | 1.00  | 0.29  | -0.08 |
| JPO+_c_pi:pi/1^S_0 pi:pi/1^S_0_order0         |  | 1.2344 +/- 0.10374    |  |      |      |      |       |       |       | 1.00  | -0.86 |
| JPO+_c_pi:pi/1^S_0 pi:pi/1^S_0_order1         |  | -1.0201 +/- 0.1044    |  |      |      |      |       |       |       |       | 1.00  |

## pole singularities

\*\*\*\*\*  
JP=0+ || eta:eta/1^S\_0[+] kaon:kaon/1^S\_0[+] pi:pi/1^S\_0[+]

$\text{sqrt}(s)_{\text{pole}} = (0.13189 \pm 0.00073397) + (i/2) * (3.5631e-12 \pm 1.0595e-09) [0.06]$

| eta:eta/1^S_0                | kaon:kaon/1^S_0              | pi:pi/1^S_0                   |
|------------------------------|------------------------------|-------------------------------|
| k_re= 0.0000 +/- 0.0000      | k_re= 0.0000 +/- 0.0000      | k_re= 0.0000 +/- 0.0000       |
| k_im= 0.0800 +/- 0.0003      | k_im= 0.0711 +/- 0.0003      | k_im= 0.0205 +/- 0.0012       |
| corr= [-0.06]                | corr= [-0.06]                | corr= [-0.06]                 |
| g = 0.0476 +/- 0.0056        | g = 0.1422 +/- 0.0124        | g = 0.0946 +/- 0.0028         |
| arg(g)/pi= 0.0000 +/- 0.0000 | arg(g)/pi= 1.0000 +/- 0.0000 | arg(g)/pi= -0.0000 +/- 0.0000 |
| g_re= 0.0476 +/- 0.0056      | g_re= -0.1422 +/- 0.0124     | g_re= 0.0946 +/- 0.0028       |
| g_im= 0.0000 +/- 0.0000      | g_im= 0.0000 +/- 0.0000      | g_im= -0.0000 +/- 0.0000      |
| corr= [-1.00]                | corr= [0.96]                 | corr= [-0.12]                 |

\*\*\*\*\*  
JP=0+ || eta:eta/1^S\_0[+] kaon:kaon/1^S\_0[+] pi:pi/1^S\_0[-]

$\text{sqrt}(s)_{\text{pole}} = (0.21376 \pm 0.0081252) + (i/2) * (-0.045664 \pm 0.016128) [0.41]$

|               |                 |             |
|---------------|-----------------|-------------|
| eta:eta/1^S_0 | kaon:kaon/1^S_0 | pi:pi/1^S_0 |
|---------------|-----------------|-------------|

```

=====|=====|=====|
k_re= -0.0391 +/- 0.0069 | k_re= -0.0499 +/- 0.0067 | k_re= 0.0821 +/- 0.0051 |
k_im= 0.0312 +/- 0.0102 | k_im= 0.0245 +/- 0.0088 | k_im= -0.0149 +/- 0.0053 |
corr= [ 0.19] | corr= [ 0.33] | corr= [ 0.41] |
=====|=====|=====|
|g|= 0.0951 +/- 0.0173 | |g|= 0.2462 +/- 0.0499 | |g|= 0.1963 +/- 0.0407 |
arg(g)/pi= 0.2778 +/- 0.0632 | arg(g)/pi= -0.6551 +/- 0.0686 | arg(g)/pi= 0.7371 +/- 0.0977 |
=====|=====|=====|
g_re= 0.0611 +/- 0.0227 | g_re= -0.1152 +/- 0.0629 | g_re= -0.1331 +/- 0.0440 |
g_im= 0.0728 +/- 0.0117 | g_im= -0.2175 +/- 0.0367 | g_im= 0.1443 +/- 0.0580 |
corr= [ 0.01] | corr= [ 0.30] | corr= [ 0.41] |
=====|=====|=====|

```

```

*****
JP=0+ || eta:eta/1^S_0[+] kaon:kaon/1^S_0[-] pi:pi/1^S_0[-]

```

```

sqrt(s)_pole = (0.12001 +/- 0.0034817)
+ (i/2)*(+3.7087e-17 +/- 6.8459e-14) [-0.12]

```

```

=====|=====|=====|
eta:eta/1^S_0 | kaon:kaon/1^S_0 | pi:pi/1^S_0 |
=====|=====|=====|
k_re= 0.0000 +/- 0.0000 | k_re= -0.0000 +/- 0.0000 | k_re= -0.0000 +/- 0.0000 |
k_im= 0.0845 +/- 0.0012 | k_im= -0.0762 +/- 0.0014 | k_im= -0.0342 +/- 0.0031 |
corr= [ 0.11] | corr= [ 0.11] | corr= [ 0.11] |
=====|=====|=====|
|g|= 0.0189 +/- 0.0008 | |g|= 0.0234 +/- 0.0019 | |g|= 0.0952 +/- 0.0015 |
arg(g)/pi= 0.5000 +/- 0.0000 | arg(g)/pi= -0.5000 +/- 0.0000 | arg(g)/pi= -0.5000 +/- 0.0000 |
=====|=====|=====|
g_re= 0.0000 +/- 0.0000 | g_re= 0.0000 +/- 0.0000 | g_re= 0.0000 +/- 0.0000 |
g_im= 0.0189 +/- 0.0008 | g_im= -0.0234 +/- 0.0019 | g_im= -0.0952 +/- 0.0015 |
corr= [-1.00] | corr= [-0.40] | corr= [-0.10] |
=====|=====|=====|

```

```

*****
JP=0+ || eta:eta/1^S_0[-] kaon:kaon/1^S_0[+] pi:pi/1^S_0[+]

```

```

sqrt(s)_pole = (0.14355 +/- 0.011819)
+ (i/2)*(-0.11669 +/- 0.0079812) [-0.78]

```

```

=====|=====|=====|
eta:eta/1^S_0 | kaon:kaon/1^S_0 | pi:pi/1^S_0 |
=====|=====|=====|
k_re= 0.0249 +/- 0.0044 | k_re= -0.0274 +/- 0.0049 | k_re= -0.0433 +/- 0.0072 |
k_im= -0.0840 +/- 0.0033 | k_im= 0.0765 +/- 0.0033 | k_im= 0.0484 +/- 0.0020 |
corr= [ 0.92] | corr= [ 0.91] | corr= [ 0.67] |
=====|=====|=====|
|g|= 0.0959 +/- 0.0081 | |g|= 0.2352 +/- 0.0164 | |g|= 0.0821 +/- 0.0031 |
arg(g)/pi= 0.2806 +/- 0.0247 | arg(g)/pi= -0.7600 +/- 0.0256 | arg(g)/pi= 0.0078 +/- 0.0154 |
=====|=====|=====|
g_re= 0.0610 +/- 0.0029 | g_re= -0.1714 +/- 0.0065 | g_re= 0.0821 +/- 0.0031 |
g_im= 0.0741 +/- 0.0106 | g_im= -0.1610 +/- 0.0242 | g_im= 0.0020 +/- 0.0040 |
corr= [-0.17] | corr= [-0.17] | corr= [ 0.67] |
=====|=====|=====|

```

```

*****
JP=0+ || eta:eta/1^S_0[-] kaon:kaon/1^S_0[+] pi:pi/1^S_0[-]

```

```

sqrt(s)_pole = (0.23159 +/- 0.006201)
+ (i/2)*(-0.035569 +/- 0.016413) [-0.24]

```

```

=====|=====|=====|
eta:eta/1^S_0 | kaon:kaon/1^S_0 | pi:pi/1^S_0 |
=====|=====|=====|
k_re= 0.0543 +/- 0.0069 | k_re= -0.0646 +/- 0.0057 | k_re= 0.0932 +/- 0.0039 |
k_im= -0.0190 +/- 0.0078 | k_im= 0.0159 +/- 0.0069 | k_im= -0.0111 +/- 0.0050 |
corr= [-0.33] | corr= [-0.31] | corr= [-0.26] |
=====|=====|=====|
|g|= 0.0922 +/- 0.0093 | |g|= 0.2288 +/- 0.0252 | |g|= 0.1741 +/- 0.0222 |
arg(g)/pi= 0.3894 +/- 0.0151 | arg(g)/pi= -0.5583 +/- 0.0147 | arg(g)/pi= 0.8780 +/- 0.0298 |
=====|=====|=====|
g_re= 0.0314 +/- 0.0054 | g_re= -0.0417 +/- 0.0113 | g_re= -0.1615 +/- 0.0202 |
g_im= 0.0866 +/- 0.0088 | g_im= -0.2250 +/- 0.0248 | g_im= 0.0651 +/- 0.0187 |
corr= [ 0.51] | corr= [ 0.33] | corr= [-0.35] |
=====|=====|=====|

```

```

*****
JP=0+ || eta:eta/1^S_0[-] kaon:kaon/1^S_0[+] pi:pi/1^S_0[-]

```

```

sqrt(s)_pole = (0.10484 +/- 0.0060787)
+ (i/2)*(+1.1051e-13 +/- 3.2253e-11) [ 0.01]

```

```

=====|=====|=====|
eta:eta/1^S_0 | kaon:kaon/1^S_0 | pi:pi/1^S_0 |
=====|=====|=====|
k_re= -0.0000 +/- 0.0000 | k_re= 0.0000 +/- 0.0000 | k_re= -0.0000 +/- 0.0000 |
k_im= -0.0894 +/- 0.0018 | k_im= 0.0816 +/- 0.0020 | k_im= -0.0450 +/- 0.0035 |
corr= [-0.01] | corr= [-0.01] | corr= [-0.01] |
=====|=====|=====|
|g|= 0.0520 +/- 0.0038 | |g|= 0.0941 +/- 0.0098 | |g|= 0.0614 +/- 0.0096 |
arg(g)/pi= 0.5000 +/- 0.0000 | arg(g)/pi= -0.5000 +/- 0.0000 | arg(g)/pi= -0.5000 +/- 0.0000 |
=====|=====|=====|
g_re= 0.0000 +/- 0.0000 | g_re= 0.0000 +/- 0.0000 | g_re= 0.0000 +/- 0.0000 |
g_im= 0.0520 +/- 0.0038 | g_im= -0.0941 +/- 0.0098 | g_im= -0.0614 +/- 0.0096 |
corr= [-1.00] | corr= [ 0.61] | corr= [-0.84] |
=====|=====|=====|

```

```

*****
JP=0+ || eta:eta/1^S_0[-] kaon:kaon/1^S_0[-] pi:pi/1^S_0[-]

```

```

sqrt(s)_pole = (0.12391 +/- 0.0032883)

```

$$+ (i/2)*(+3.3232e-14 \pm 9.8989e-12) [-0.04]$$

| eta:eta/1^S_0                | kaon:kaon/1^S_0               | pi:pi/1^S_0                   |
|------------------------------|-------------------------------|-------------------------------|
| =====                        | =====                         | =====                         |
| k_re= -0.0000 +/- 0.0000     | k_re= -0.0000 +/- 0.0000      | k_re= -0.0000 +/- 0.0000      |
| k_im= -0.0831 +/- 0.0012     | k_im= -0.0746 +/- 0.0014      | k_im= -0.0305 +/- 0.0033      |
| corr= [ 0.04]                | corr= [ 0.04]                 | corr= [ 0.04]                 |
| =====                        | =====                         | =====                         |
| g = 0.0182 +/- 0.0007        | g = 0.0155 +/- 0.0018         | g = 0.0964 +/- 0.0011         |
| arg(g)/pi= 0.5000 +/- 0.0000 | arg(g)/pi= -0.5000 +/- 0.0000 | arg(g)/pi= -0.5000 +/- 0.0000 |
| =====                        | =====                         | =====                         |
| g_re= 0.0000 +/- 0.0000      | g_re= 0.0000 +/- 0.0000       | g_re= 0.0000 +/- 0.0000       |
| g_im= 0.0182 +/- 0.0007      | g_im= -0.0155 +/- 0.0018      | g_im= -0.0964 +/- 0.0011      |
| corr= [-1.00]                | corr= [-0.74]                 | corr= [-0.40]                 |
| =====                        | =====                         | =====                         |

\*\*\*\*\*

# k\_inv\_poly\_qccccc

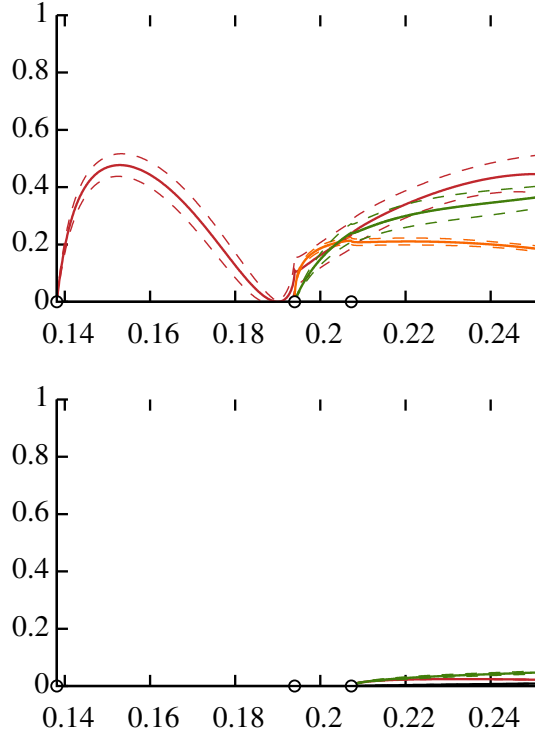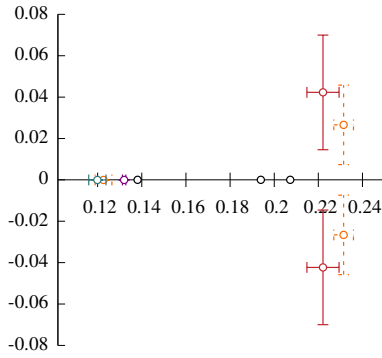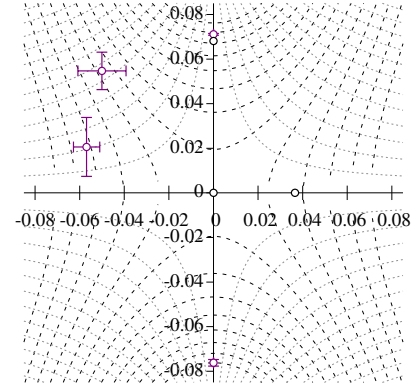

## parameter values

minimised with  $\text{chisq}/\text{nDoF} = 45.55 / (57 - 8) = 0.93$

|                                               |                      |      |      |      |       |       |       |       |       |
|-----------------------------------------------|----------------------|------|------|------|-------|-------|-------|-------|-------|
| JP0+_c_eta:eta/1^S_0 eta:eta/1^S_0_order0     | 22.708 +/- 0.586     | 1.00 | 0.76 | 0.08 | 0.06  | -0.08 | 0.00  | -0.05 | 0.04  |
| JP0+_c_eta:eta/1^S_0 kaon:kaon/1^S_0_order0   | 8.4871 +/- 0.14467   | 1.00 | 0.12 | 0.61 | -0.15 | -0.09 | -0.08 | 0.11  |       |
| JP0+_c_eta:eta/1^S_0 pi:pi/1^S_0_order0       | 1.7877 +/- 0.13003   |      |      | 1.00 | -0.03 | 0.64  | -0.06 | -0.07 | 0.17  |
| JP0+_c_kaon:kaon/1^S_0 kaon:kaon/1^S_0_order0 | 2.9483 +/- 0.060431  |      |      |      | 1.00  | 0.06  | -0.02 | -0.06 | 0.06  |
| JP0+_c_kaon:kaon/1^S_0 pi:pi/1^S_0_order0     | 1.1930 +/- 0.050375  |      |      |      |       | 1.00  | 0.40  | 0.14  | -0.25 |
| JP0+_c_pi:pi/1^S_0 pi:pi/1^S_0_order0         | 1.0453 +/- 0.098014  |      |      |      |       |       | 1.00  | -0.43 | 0.05  |
| JP0+_c_pi:pi/1^S_0 pi:pi/1^S_0_order1         | -0.65331 +/- 0.22688 |      |      |      |       |       |       | 1.00  | -0.89 |
| JP0+_c_pi:pi/1^S_0 pi:pi/1^S_0_order2         | -0.22525 +/- 0.17121 |      |      |      |       |       |       |       | 1.00  |

## pole singularities

\*\*\*\*\*  
JP=0+ || eta:eta/1^S\_0[+] kaon:kaon/1^S\_0[+] pi:pi/1^S\_0[+]

$\text{sqrt}(s)_{\text{pole}} = (0.132 \pm 0.00075775) + (i/2)*(-1.3205e-15 \pm 8.0364e-13) [0.05]$

| eta:eta/1^S_0                | kaon:kaon/1^S_0              | pi:pi/1^S_0                   |
|------------------------------|------------------------------|-------------------------------|
| k_re= -0.0000 +/- 0.0000     | k_re= -0.0000 +/- 0.0000     | k_re= -0.0000 +/- 0.0000      |
| k_im= 0.0799 +/- 0.0003      | k_im= 0.0711 +/- 0.0004      | k_im= 0.0203 +/- 0.0012       |
| corr= [-0.05]                | corr= [-0.05]                | corr= [-0.05]                 |
| g = 0.0448 +/- 0.0032        | g = 0.1428 +/- 0.0080        | g = 0.0957 +/- 0.0030         |
| arg(g)/pi= 0.0000 +/- 0.0000 | arg(g)/pi= 1.0000 +/- 0.0000 | arg(g)/pi= -0.0000 +/- 0.0000 |
| g_re= 0.0448 +/- 0.0032      | g_re= -0.1428 +/- 0.0080     | g_re= 0.0957 +/- 0.0030       |
| g_im= 0.0000 +/- 0.0000      | g_im= 0.0000 +/- 0.0000      | g_im= -0.0000 +/- 0.0000      |
| corr= [-1.00]                | corr= [0.89]                 | corr= [-0.28]                 |

\*\*\*\*\*  
JP=0+ || eta:eta/1^S\_0[+] kaon:kaon/1^S\_0[+] pi:pi/1^S\_0[-]

$\text{sqrt}(s)_{\text{pole}} = (0.19685 \pm 0.01718) + (i/2)*(-0.11126 \pm 0.019965) [-0.04]$

| eta:eta/1^S_0 | kaon:kaon/1^S_0 | pi:pi/1^S_0 |
|---------------|-----------------|-------------|
|---------------|-----------------|-------------|

```

=====|=====|=====|
k_re= -0.0444 +/- 0.0101 | k_re= -0.0500 +/- 0.0108 | k_re= 0.0742 +/- 0.0105 |
k_im= 0.0616 +/- 0.0088 | k_im= 0.0547 +/- 0.0084 | k_im= -0.0369 +/- 0.0063 |
corr= [ 0.48] | corr= [ 0.44] | corr= [ 0.17] |
=====|=====|=====|
|g|= 0.0880 +/- 0.0274 | |g|= 0.2728 +/- 0.0798 | |g|= 0.2264 +/- 0.0910 |
arg(g)/pi= -0.0394 +/- 0.0850 | arg(g)/pi= -0.9926 +/- 0.0716 | arg(g)/pi= 0.2494 +/- 0.0628 |
=====|=====|=====|
g_re= 0.0874 +/- 0.0257 | g_re= -0.2727 +/- 0.0806 | g_re= 0.1604 +/- 0.0760 |
g_im= -0.0109 +/- 0.0254 | g_im= -0.0064 +/- 0.0604 | g_im= 0.1598 +/- 0.0671 |
corr= [-0.57] | corr= [-0.55] | corr= [ 0.62] |
=====|=====|=====|
*****

```

```

*****
JP=0+ || eta:eta/1^S_0[+] kaon:kaon/1^S_0[+] pi:pi/1^S_0[-]

```

```

sqrt(s)_pole = (0.22208 +/- 0.0072935)
+ (i/2)*(-0.042279 +/- 0.027701) [ 0.43]

```

```

=====|=====|=====|
eta:eta/1^S_0 | kaon:kaon/1^S_0 | pi:pi/1^S_0 |
=====|=====|=====|
k_re= -0.0461 +/- 0.0070 | k_re= -0.0569 +/- 0.0059 | k_re= 0.0873 +/- 0.0044 |
k_im= 0.0255 +/- 0.0150 | k_im= 0.0206 +/- 0.0132 | k_im= -0.0134 +/- 0.0088 |
corr= [-0.23] | corr= [ 0.05] | corr= [ 0.36] |
=====|=====|=====|
|g|= 0.0821 +/- 0.0327 | |g|= 0.2307 +/- 0.1001 | |g|= 0.2056 +/- 0.0865 |
arg(g)/pi= 0.3807 +/- 0.0633 | arg(g)/pi= -0.5551 +/- 0.0684 | arg(g)/pi= 0.8546 +/- 0.0937 |
=====|=====|=====|
g_re= 0.0301 +/- 0.0214 | g_re= -0.0397 +/- 0.0554 | g_re= -0.1845 +/- 0.0641 |
g_im= 0.0764 +/- 0.0296 | g_im= -0.2273 +/- 0.0970 | g_im= 0.0907 +/- 0.0839 |
corr= [ 0.58] | corr= [ 0.44] | corr= [-0.66] |
=====|=====|=====|
*****

```

```

*****
JP=0+ || eta:eta/1^S_0[+] kaon:kaon/1^S_0[-] pi:pi/1^S_0[-]

```

```

sqrt(s)_pole = (0.11989 +/- 0.0039274)
+ (i/2)*(-8.5404e-16 +/- 9.4374e-14) [ 0.06]

```

```

=====|=====|=====|
eta:eta/1^S_0 | kaon:kaon/1^S_0 | pi:pi/1^S_0 |
=====|=====|=====|
k_re= -0.0000 +/- 0.0000 | k_re= 0.0000 +/- 0.0000 | k_re= 0.0000 +/- 0.0000 |
k_im= 0.0845 +/- 0.0014 | k_im= -0.0762 +/- 0.0015 | k_im= -0.0343 +/- 0.0034 |
corr= [-0.06] | corr= [-0.06] | corr= [-0.06] |
=====|=====|=====|
|g|= 0.0157 +/- 0.0007 | |g|= 0.0233 +/- 0.0012 | |g|= 0.0929 +/- 0.0025 |
arg(g)/pi= 0.5000 +/- 0.0000 | arg(g)/pi= -0.5000 +/- 0.0000 | arg(g)/pi= -0.5000 +/- 0.0000 |
=====|=====|=====|
g_re= 0.0000 +/- 0.0000 | g_re= 0.0000 +/- 0.0000 | g_re= 0.0000 +/- 0.0000 |
g_im= 0.0157 +/- 0.0007 | g_im= -0.0233 +/- 0.0012 | g_im= -0.0929 +/- 0.0025 |
corr= [-1.00] | corr= [-0.09] | corr= [ 0.27] |
=====|=====|=====|
*****

```

```

*****
JP=0+ || eta:eta/1^S_0[-] kaon:kaon/1^S_0[+] pi:pi/1^S_0[+]

```

```

sqrt(s)_pole = (0.13291 +/- 0.0038793)
+ (i/2)*(-0.11126 +/- 0.0080107) [-0.89]

```

```

=====|=====|=====|
eta:eta/1^S_0 | kaon:kaon/1^S_0 | pi:pi/1^S_0 |
=====|=====|=====|
k_re= 0.0213 +/- 0.0022 | k_re= -0.0233 +/- 0.0024 | k_re= -0.0370 +/- 0.0030 |
k_im= -0.0869 +/- 0.0006 | k_im= 0.0794 +/- 0.0006 | k_im= 0.0500 +/- 0.0011 |
corr= [ 0.45] | corr= [ 0.31] | corr= [-0.70] |
=====|=====|=====|
|g|= 0.0872 +/- 0.0038 | |g|= 0.2343 +/- 0.0080 | |g|= 0.0854 +/- 0.0035 |
arg(g)/pi= 0.2580 +/- 0.0045 | arg(g)/pi= -0.7761 +/- 0.0039 | arg(g)/pi= 0.0512 +/- 0.0191 |
=====|=====|=====|
g_re= 0.0601 +/- 0.0029 | g_re= -0.1787 +/- 0.0069 | g_re= 0.0843 +/- 0.0030 |
g_im= 0.0632 +/- 0.0028 | g_im= -0.1516 +/- 0.0051 | g_im= 0.0137 +/- 0.0054 |
corr= [ 0.81] | corr= [ 0.77] | corr= [ 0.55] |
=====|=====|=====|
*****

```

```

*****
JP=0+ || eta:eta/1^S_0[-] kaon:kaon/1^S_0[+] pi:pi/1^S_0[-]

```

```

sqrt(s)_pole = (0.094486 +/- 0.0056375)
+ (i/2)*(+1.9942e-15 +/- 1.0347e-12) [ 0.03]

```

```

=====|=====|=====|
eta:eta/1^S_0 | kaon:kaon/1^S_0 | pi:pi/1^S_0 |
=====|=====|=====|
k_re= -0.0000 +/- 0.0000 | k_re= 0.0000 +/- 0.0000 | k_re= -0.0000 +/- 0.0000 |
k_im= -0.0922 +/- 0.0014 | k_im= 0.0847 +/- 0.0016 | k_im= -0.0504 +/- 0.0026 |
corr= [-0.03] | corr= [-0.03] | corr= [-0.03] |
=====|=====|=====|
|g|= 0.0497 +/- 0.0037 | |g|= 0.1036 +/- 0.0084 | |g|= 0.0468 +/- 0.0063 |
arg(g)/pi= 0.5000 +/- 0.0000 | arg(g)/pi= -0.5000 +/- 0.0000 | arg(g)/pi= -0.5000 +/- 0.0000 |
=====|=====|=====|
g_re= 0.0000 +/- 0.0000 | g_re= 0.0000 +/- 0.0000 | g_re= 0.0000 +/- 0.0000 |
g_im= 0.0497 +/- 0.0037 | g_im= -0.1036 +/- 0.0084 | g_im= -0.0468 +/- 0.0063 |
corr= [-1.00] | corr= [ 0.82] | corr= [-0.33] |
=====|=====|=====|
*****

```

```

*****
JP=0+ || eta:eta/1^S_0[-] kaon:kaon/1^S_0[+] pi:pi/1^S_0[-]

```

```

sqrt(s)_pole = (0.23144 +/- 0.0044408)

```



```

+ (i/2)*(-0.026606 +/- 0.019184) [-0.48]

eta:eta/1^S_0 | kaon:kaon/1^S_0 | pi:pi/1^S_0 |
=====|=====|=====|
k_re= 0.0531 +/- 0.0059 | k_re= -0.0639 +/- 0.0046 | k_re= 0.0930 +/- 0.0028 |
k_im= -0.0145 +/- 0.0094 | k_im= 0.0120 +/- 0.0082 | k_im= -0.0083 +/- 0.0059 |
corr= [-0.67] | corr= [-0.61] | corr= [-0.52] |
=====|=====|=====|
|g|= 0.0748 +/- 0.0118 | |g|= 0.2025 +/- 0.0344 | |g|= 0.1628 +/- 0.0288 |
arg(g)/pi= 0.4123 +/- 0.0181 | arg(g)/pi= -0.5410 +/- 0.0189 | arg(g)/pi= 0.9146 +/- 0.0321 |
=====|=====|=====|
g_re= 0.0204 +/- 0.0050 | g_re= -0.0260 +/- 0.0122 | g_re= -0.1570 +/- 0.0245 |
g_im= 0.0720 +/- 0.0115 | g_im= -0.2008 +/- 0.0343 | g_im= 0.0431 +/- 0.0223 |
corr= [ 0.49] | corr= [ 0.21] | corr= [-0.85] |
=====|=====|=====|
*****

```

```

*****
JP=0+ || eta:eta/1^S_0[-] kaon:kaon/1^S_0[-] pi:pi/1^S_0[-]

```

```

sqrt(s)_pole = (0.12264 +/- 0.0037997)
+ (i/2)*(-9.3408e-14 +/- 2.7958e-11) [-0.00]

```

```

eta:eta/1^S_0 | kaon:kaon/1^S_0 | pi:pi/1^S_0 |
=====|=====|=====|
k_re= 0.0000 +/- 0.0000 | k_re= 0.0000 +/- 0.0000 | k_re= 0.0000 +/- 0.0000 |
k_im= -0.0836 +/- 0.0014 | k_im= -0.0751 +/- 0.0016 | k_im= -0.0318 +/- 0.0037 |
corr= [ 0.00] | corr= [ 0.00] | corr= [ 0.00] |
=====|=====|=====|
|g|= 0.0153 +/- 0.0006 | |g|= 0.0173 +/- 0.0012 | |g|= 0.0941 +/- 0.0018 |
arg(g)/pi= 0.5000 +/- 0.0000 | arg(g)/pi= -0.5000 +/- 0.0000 | arg(g)/pi= -0.5000 +/- 0.0000 |
=====|=====|=====|
g_re= 0.0000 +/- 0.0000 | g_re= 0.0000 +/- 0.0000 | g_re= 0.0000 +/- 0.0000 |
g_im= 0.0153 +/- 0.0006 | g_im= -0.0173 +/- 0.0012 | g_im= -0.0941 +/- 0.0018 |
corr= [-1.00] | corr= [-0.48] | corr= [ 0.04] |
=====|=====|=====|
*****

```

# k\_inv\_poly\_lcccc1

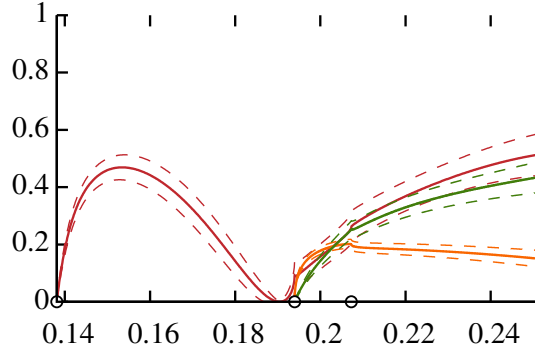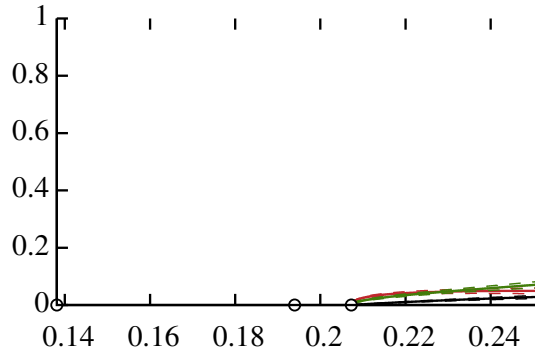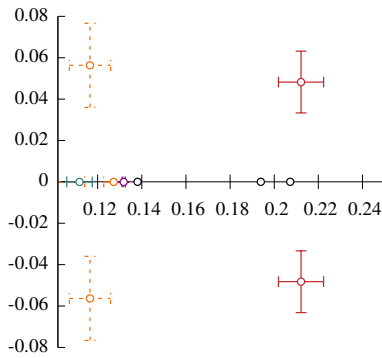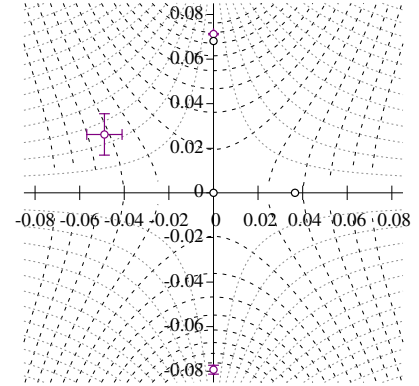

## parameter values

minimised with  $\text{chisq}/\text{nDoF} = 45.23 / (57 - 8) = 0.92$

|                                               |                      |      |       |      |      |       |       |       |       |
|-----------------------------------------------|----------------------|------|-------|------|------|-------|-------|-------|-------|
| JPO+_c_eta:eta/1^S_0 eta:eta/1^S_0_order0     | 26.962 +/- 1.1848    | 1.00 | -0.25 | 0.73 | 0.38 | 0.10  | -0.20 | -0.13 | -0.15 |
| JPO+_c_eta:eta/1^S_0 eta:eta/1^S_0_order1     | -1.2133 +/- 0.7769   | 1.00 | 0.37  | 0.32 | 0.02 | -0.28 | -0.12 | -0.13 |       |
| JPO+_c_eta:eta/1^S_0 kaon:kaon/1^S_0_order0   | 10.534 +/- 0.27373   |      |       | 1.00 | 0.52 | 0.42  | -0.28 | -0.25 | -0.17 |
| JPO+_c_eta:eta/1^S_0 pi:pi/1^S_0_order0       | 7.6914 +/- 0.21321   |      |       |      | 1.00 | -0.06 | 0.37  | 0.19  | 0.22  |
| JPO+_c_kaon:kaon/1^S_0 kaon:kaon/1^S_0_order0 | 4.0796 +/- 0.072748  |      |       |      |      | 1.00  | 0.21  | -0.13 | -0.06 |
| JPO+_c_kaon:kaon/1^S_0 pi:pi/1^S_0_order0     | 3.6692 +/- 0.068302  |      |       |      |      |       | 1.00  | 0.67  | 0.18  |
| JPO+_c_pi:pi/1^S_0 pi:pi/1^S_0_order0         | 3.3208 +/- 0.11506   |      |       |      |      |       |       | 1.00  | -0.48 |
| JPO+_c_pi:pi/1^S_0 pi:pi/1^S_0_order1         | -0.98255 +/- 0.11719 |      |       |      |      |       |       |       | 1.00  |

## pole singularities

\*\*\*\*\*  
JP=0+ || eta:eta/1^S\_0[+] kaon:kaon/1^S\_0[+] pi:pi/1^S\_0[+]

$\text{sqrt}(s)_{\text{pole}} = (0.1318 \pm 0.00073782) + (i/2)(-3.8924e-16 \pm 7.3951e-14) [0.04]$

| eta:eta/1^S_0                | kaon:kaon/1^S_0              | pi:pi/1^S_0                   |
|------------------------------|------------------------------|-------------------------------|
| k_re= -0.0000 +/- 0.0000     | k_re= -0.0000 +/- 0.0000     | k_re= -0.0000 +/- 0.0000      |
| k_im= 0.0800 +/- 0.0003      | k_im= 0.0712 +/- 0.0003      | k_im= 0.0207 +/- 0.0012       |
| corr= [-0.04]                | corr= [-0.04]                | corr= [-0.04]                 |
| g = 0.0249 +/- 0.0034        | g = 0.1334 +/- 0.0074        | g = 0.0955 +/- 0.0030         |
| arg(g)/pi= 0.0000 +/- 0.0000 | arg(g)/pi= 1.0000 +/- 0.0000 | arg(g)/pi= -0.0000 +/- 0.0000 |
| g_re= 0.0249 +/- 0.0034      | g_re= -0.1334 +/- 0.0074     | g_re= 0.0955 +/- 0.0030       |
| g_im= 0.0000 +/- 0.0000      | g_im= 0.0000 +/- 0.0000      | g_im= -0.0000 +/- 0.0000      |
| corr= [-1.00]                | corr= [0.88]                 | corr= [-0.36]                 |

\*\*\*\*\*  
JP=0+ || eta:eta/1^S\_0[+] kaon:kaon/1^S\_0[+] pi:pi/1^S\_0[-]

$\text{sqrt}(s)_{\text{pole}} = (0.21216 \pm 0.010229) + (i/2)(-0.048246 \pm 0.014918) [0.59]$

| eta:eta/1^S_0 | kaon:kaon/1^S_0 | pi:pi/1^S_0 |
|---------------|-----------------|-------------|
|---------------|-----------------|-------------|

```

=====|=====|=====|
k_re= -0.0384 +/- 0.0072 | k_re= -0.0489 +/- 0.0079 | k_re= 0.0812 +/- 0.0064 |
k_im= 0.0333 +/- 0.0112 | k_im= 0.0262 +/- 0.0093 | k_im= -0.0158 +/- 0.0051 |
corr= [ 0.53] | corr= [ 0.63] | corr= [ 0.62] |
=====|=====|=====|
|g|= 0.0910 +/- 0.0101 | |g|= 0.2296 +/- 0.0395 | |g|= 0.1937 +/- 0.0327 |
arg(g)/pi= 0.1118 +/- 0.0835 | arg(g)/pi= -0.6791 +/- 0.0909 | arg(g)/pi= 0.7066 +/- 0.1246 |
=====|=====|=====|
g_re= 0.0855 +/- 0.0128 | g_re= -0.1225 +/- 0.0666 | g_re= -0.1171 +/- 0.0621 |
g_im= 0.0313 +/- 0.0226 | g_im= -0.1942 +/- 0.0378 | g_im= 0.1543 +/- 0.0544 |
corr= [-0.54] | corr= [-0.32] | corr= [ 0.68] |
=====|=====|=====|
*****

```

```

*****
JP=0+ || eta:eta/1^S_0[+] kaon:kaon/1^S_0[-] pi:pi/1^S_0[-]

```

```

sqrt(s)_pole = (0.11176 +/- 0.0057627)
+ (i/2)*(-1.1298e-14 +/- 3.187e-12) [ 0.06]

```

```

=====|=====|=====|
eta:eta/1^S_0 | kaon:kaon/1^S_0 | pi:pi/1^S_0 |
=====|=====|=====|
k_re= -0.0000 +/- 0.0000 | k_re= 0.0000 +/- 0.0000 | k_re= 0.0000 +/- 0.0000 |
k_im= 0.0873 +/- 0.0018 | k_im= -0.0793 +/- 0.0020 | k_im= -0.0406 +/- 0.0040 |
corr= [-0.06] | corr= [-0.06] | corr= [-0.06] |
=====|=====|=====|
|g|= 0.0356 +/- 0.0021 | |g|= 0.0266 +/- 0.0018 | |g|= 0.0893 +/- 0.0049 |
arg(g)/pi= 0.5000 +/- 0.0000 | arg(g)/pi= -0.5000 +/- 0.0000 | arg(g)/pi= -0.5000 +/- 0.0000 |
=====|=====|=====|
g_re= 0.0000 +/- 0.0000 | g_re= 0.0000 +/- 0.0000 | g_re= 0.0000 +/- 0.0000 |
g_im= 0.0356 +/- 0.0021 | g_im= -0.0266 +/- 0.0018 | g_im= -0.0893 +/- 0.0049 |
corr= [-1.00] | corr= [-0.52] | corr= [ 0.48] |
=====|=====|=====|
*****

```

```

*****
JP=0+ || eta:eta/1^S_0[-] kaon:kaon/1^S_0[+] pi:pi/1^S_0[+]

```

```

sqrt(s)_pole = (0.11651 +/- 0.0093712)
+ (i/2)*(-0.056317 +/- 0.020323) [-0.92]

```

```

=====|=====|=====|
eta:eta/1^S_0 | kaon:kaon/1^S_0 | pi:pi/1^S_0 |
=====|=====|=====|
k_re= 0.0094 +/- 0.0043 | k_re= -0.0103 +/- 0.0047 | k_re= -0.0187 +/- 0.0085 |
k_im= -0.0874 +/- 0.0020 | k_im= 0.0795 +/- 0.0021 | k_im= 0.0439 +/- 0.0019 |
corr= [ 0.86] | corr= [ 0.85] | corr= [ 0.44] |
=====|=====|=====|
|g|= 0.0787 +/- 0.0028 | |g|= 0.2292 +/- 0.0093 | |g|= 0.0775 +/- 0.0071 |
arg(g)/pi= 0.2768 +/- 0.0222 | arg(g)/pi= -0.7815 +/- 0.0104 | arg(g)/pi= 0.0554 +/- 0.0745 |
=====|=====|=====|
g_re= 0.0508 +/- 0.0031 | g_re= -0.1773 +/- 0.0075 | g_re= 0.0763 +/- 0.0041 |
g_im= 0.0601 +/- 0.0053 | g_im= -0.1453 +/- 0.0093 | g_im= 0.0134 +/- 0.0190 |
corr= [-0.78] | corr= [ 0.26] | corr= [ 0.86] |
=====|=====|=====|
*****

```

```

*****
JP=0+ || eta:eta/1^S_0[-] kaon:kaon/1^S_0[+] pi:pi/1^S_0[-]

```

```

sqrt(s)_pole = (0.23603 +/- 0.010868)
+ (i/2)*(-0.093602 +/- 0.052979) [ 0.09]

```

```

=====|=====|=====|
eta:eta/1^S_0 | kaon:kaon/1^S_0 | pi:pi/1^S_0 |
=====|=====|=====|
k_re= 0.0662 +/- 0.0102 | k_re= -0.0734 +/- 0.0089 | k_re= 0.0971 +/- 0.0065 |
k_im= -0.0417 +/- 0.0195 | k_im= 0.0376 +/- 0.0189 | k_im= -0.0285 +/- 0.0157 |
corr= [-0.52] | corr= [-0.42] | corr= [-0.10] |
=====|=====|=====|
|g|= 0.1200 +/- 0.0167 | |g|= 0.2706 +/- 0.0618 | |g|= 0.2636 +/- 0.0937 |
arg(g)/pi= 0.2523 +/- 0.0719 | arg(g)/pi= -0.5256 +/- 0.1227 | arg(g)/pi= 0.8881 +/- 0.0663 |
=====|=====|=====|
g_re= 0.0842 +/- 0.0171 | g_re= -0.0217 +/- 0.1012 | g_re= -0.2475 +/- 0.1002 |
g_im= 0.0855 +/- 0.0269 | g_im= -0.2697 +/- 0.0668 | g_im= 0.0907 +/- 0.0418 |
corr= [-0.50] | corr= [-0.63] | corr= [ 0.10] |
=====|=====|=====|
*****

```

```

*****
JP=0+ || eta:eta/1^S_0[-] kaon:kaon/1^S_0[+] pi:pi/1^S_0[-]

```

```

sqrt(s)_pole = (0.098964 +/- 0.015174)
+ (i/2)*(+1.4552e-13 +/- 4.4657e-11) [-0.03]

```

```

=====|=====|=====|
eta:eta/1^S_0 | kaon:kaon/1^S_0 | pi:pi/1^S_0 |
=====|=====|=====|
k_re= -0.0000 +/- 0.0000 | k_re= 0.0000 +/- 0.0000 | k_re= -0.0000 +/- 0.0000 |
k_im= -0.0911 +/- 0.0041 | k_im= 0.0834 +/- 0.0045 | k_im= -0.0482 +/- 0.0078 |
corr= [ 0.03] | corr= [ 0.03] | corr= [ 0.03] |
=====|=====|=====|
|g|= 0.0680 +/- 0.0117 | |g|= 0.1282 +/- 0.0161 | |g|= 0.0326 +/- 0.0171 |
arg(g)/pi= 0.5000 +/- 0.0000 | arg(g)/pi= -0.5000 +/- 0.0000 | arg(g)/pi= -0.5000 +/- 0.0000 |
=====|=====|=====|
g_re= 0.0000 +/- 0.0000 | g_re= 0.0000 +/- 0.0000 | g_re= 0.0000 +/- 0.0000 |
g_im= 0.0680 +/- 0.0117 | g_im= -0.1282 +/- 0.0161 | g_im= -0.0326 +/- 0.0171 |
corr= [-1.00] | corr= [ 0.85] | corr= [-0.83] |
=====|=====|=====|
*****

```

```

*****
JP=0+ || eta:eta/1^S_0[-] kaon:kaon/1^S_0[+] pi:pi/1^S_0[-]

```

```

sqrt(s)_pole = ( 0.1873 +/- 0.013178)

```

```

+ (i/2)*(-0.14531 +/- 0.032573) [ 0.71]

eta:eta/1^S_0 | kaon:kaon/1^S_0 | pi:pi/1^S_0 |
=====|=====|=====|
k_re= 0.0462 +/- 0.0045 | k_re= -0.0506 +/- 0.0047 | k_re= 0.0707 +/- 0.0062 |
k_im= -0.0736 +/- 0.0112 | k_im= 0.0672 +/- 0.0116 | k_im= -0.0481 +/- 0.0106 |
corr= [-0.01] | corr= [ 0.17] | corr= [ 0.61] |
=====|=====|=====|
|g|= 0.0968 +/- 0.0424 | |g|= 0.3295 +/- 0.0844 | |g|= 0.2282 +/- 0.0716 |
arg(g)/pi= -0.1033 +/- 0.0899 | arg(g)/pi= -0.9487 +/- 0.0639 | arg(g)/pi= 0.2855 +/- 0.1359 |
=====|=====|=====|
g_re= 0.0918 +/- 0.0434 | g_re= -0.3253 +/- 0.0763 | g_re= 0.1423 +/- 0.0582 |
g_im= -0.0309 +/- 0.0257 | g_im= -0.0529 +/- 0.0752 | g_im= 0.1783 +/- 0.1059 |
corr= [-0.06] | corr= [ 0.71] | corr= [-0.51] |
=====|=====|=====|
*****

```

```

*****
JP=0+ || eta:eta/1^S_0[-] kaon:kaon/1^S_0[-] pi:pi/1^S_0[-]

```

```

sqrt(s)_pole = (0.12726 +/- 0.0044819)
+ (i/2)*(-3.171e-17 +/- 6.1485e-14) [ 0.02]

```

```

eta:eta/1^S_0 | kaon:kaon/1^S_0 | pi:pi/1^S_0 |
=====|=====|=====|
k_re= 0.0000 +/- 0.0000 | k_re= 0.0000 +/- 0.0000 | k_re= 0.0000 +/- 0.0000 |
k_im= -0.0818 +/- 0.0017 | k_im= -0.0732 +/- 0.0019 | k_im= -0.0268 +/- 0.0053 |
corr= [-0.02] | corr= [-0.02] | corr= [-0.02] |
=====|=====|=====|
|g|= 0.0353 +/- 0.0017 | |g|= 0.0144 +/- 0.0032 | |g|= 0.0923 +/- 0.0020 |
arg(g)/pi= 0.5000 +/- 0.0000 | arg(g)/pi= -0.5000 +/- 0.0000 | arg(g)/pi= -0.5000 +/- 0.0000 |
=====|=====|=====|
g_re= 0.0000 +/- 0.0000 | g_re= 0.0000 +/- 0.0000 | g_re= 0.0000 +/- 0.0000 |
g_im= 0.0353 +/- 0.0017 | g_im= -0.0144 +/- 0.0032 | g_im= -0.0923 +/- 0.0020 |
corr= [-1.00] | corr= [-0.92] | corr= [ 0.31] |
=====|=====|=====|
*****

```

# k\_inv\_poly\_clcccc\_noCM

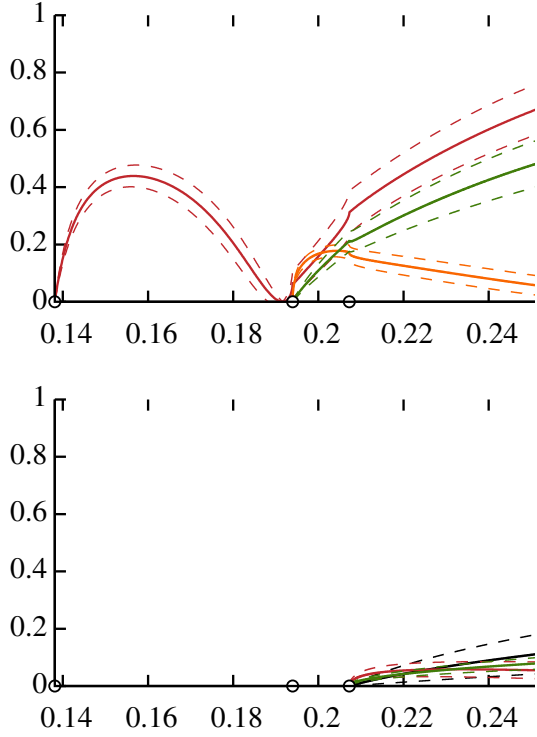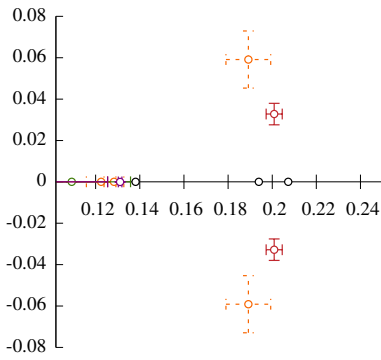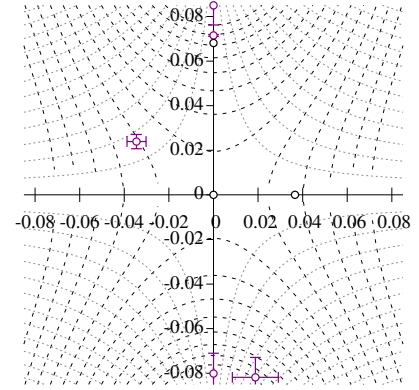

## parameter values

minimised with  $\text{chisq}/\text{nDoF} = 48.58 / (57 - 7) = 0.97$

|                                               |                      |      |       |       |      |       |       |       |
|-----------------------------------------------|----------------------|------|-------|-------|------|-------|-------|-------|
| JP0+_c_eta:eta/1^S_0 eta:eta/1^S_0_order0     | -1.4904 +/- 0.76003  | 1.00 | 0.94  | -0.26 | 0.52 | 0.34  | -0.39 | -0.46 |
| JP0+_c_eta:eta/1^S_0 kaon:kaon/1^S_0_order0   | -0.75307 +/- 0.34193 | 1.00 | -0.31 | 0.75  | 0.26 | -0.41 | -0.40 |       |
| JP0+_c_eta:eta/1^S_0 pi:pi/1^S_0_order0       | 0.45490 +/- 0.12681  |      | 1.00  | -0.27 | 0.64 | -0.13 | -0.50 |       |
| JP0+_c_kaon:kaon/1^S_0 kaon:kaon/1^S_0_order0 | -0.68465 +/- 0.18458 |      |       | 1.00  | 0.00 | -0.35 | -0.16 |       |
| JP0+_c_kaon:kaon/1^S_0 pi:pi/1^S_0_order0     | -0.69786 +/- 0.14159 |      |       |       | 1.00 | -0.73 | -0.93 |       |
| JP0+_c_kaon:kaon/1^S_0 pi:pi/1^S_0_order1     | 0.37477 +/- 0.10791  |      |       |       |      | 1.00  | 0.68  |       |
| JP0+_c_pi:pi/1^S_0 pi:pi/1^S_0_order0         | 0.18775 +/- 0.090049 |      |       |       |      |       | 1.00  |       |

## pole singularities

\*\*\*\*\*  
JP=0+ || eta:eta/1^S\_0[+] kaon:kaon/1^S\_0[+] pi:pi/1^S\_0[+]

$\text{sqrt}(s)_{\text{pole}} = (0.1311 \pm 0.00082249) + (i/2)*(-1.073e-12 \pm 3.1144e-10) [-0.01]$

| eta:eta/1^S_0                | kaon:kaon/1^S_0              | pi:pi/1^S_0                  |
|------------------------------|------------------------------|------------------------------|
| k_re= -0.0000 +/- 0.0000     | k_re= -0.0000 +/- 0.0000     | k_re= -0.0000 +/- 0.0000     |
| k_im= 0.0803 +/- 0.0003      | k_im= 0.0715 +/- 0.0004      | k_im= 0.0217 +/- 0.0012      |
| corr= [ 0.01]                | corr= [ 0.01]                | corr= [ 0.01]                |
| g = 0.0288 +/- 0.0198        | g = 0.0656 +/- 0.0111        | g = 0.0917 +/- 0.0018        |
| arg(g)/pi= 0.0000 +/- 0.0000 | arg(g)/pi= 1.0000 +/- 0.0000 | arg(g)/pi= 1.0000 +/- 0.0000 |
| g_re= 0.0288 +/- 0.0198      | g_re= -0.0656 +/- 0.0111     | g_re= -0.0917 +/- 0.0018     |
| g_im= 0.0000 +/- 0.0000      | g_im= 0.0000 +/- 0.0000      | g_im= 0.0000 +/- 0.0000      |
| corr= [-1.00]                | corr= [-0.91]                | corr= [ 0.17]                |

\*\*\*\*\*

\*\*\*\*\*  
JP=0+ || eta:eta/1^S\_0[+] kaon:kaon/1^S\_0[+] pi:pi/1^S\_0[+]

$\text{sqrt}(s)_{\text{pole}} = (0.09312 \pm 0.032311) + (i/2)*(2.7966e-15 \pm 8.3367e-13) [-0.02]$

| eta:eta/1^S_0 | kaon:kaon/1^S_0 | pi:pi/1^S_0 |
|---------------|-----------------|-------------|
|---------------|-----------------|-------------|

| eta:eta/1^S_0                | kaon:kaon/1^S_0               | pi:pi/1^S_0                  |
|------------------------------|-------------------------------|------------------------------|
| k_re= 0.0000 +/- 0.0000      | k_re= 0.0000 +/- 0.0000       | k_re= 0.0000 +/- 0.0000      |
| k_im= 0.0926 +/- 0.0081      | k_im= 0.0851 +/- 0.0088       | k_im= 0.0510 +/- 0.0148      |
| corr= [ 0.02]                | corr= [ 0.02]                 | corr= [ 0.02]                |
| g = 0.0709 +/- 0.0304        | g = 0.0447 +/- 0.0290         | g = 0.0038 +/- 0.0153        |
| arg(g)/pi= 0.0000 +/- 0.0000 | arg(g)/pi= -0.0000 +/- 0.0000 | arg(g)/pi= 1.0000 +/- 0.0000 |
| g_re= 0.0709 +/- 0.0304      | g_re= 0.0447 +/- 0.0290       | g_re= -0.0038 +/- 0.0153     |
| g_im= 0.0000 +/- 0.0000      | g_im= -0.0000 +/- 0.0000      | g_im= 0.0000 +/- 0.0000      |
| corr= [-1.00]                | corr= [ 0.21]                 | corr= [-0.98]                |

JP=0+ || eta:eta/1^S\_0[+] kaon:kaon/1^S\_0[+] pi:pi/1^S\_0[-]

sqrt(s)\_pole = ( 0.2009 +/- 0.003639)  
+ (i/2)\*(-0.032771 +/- 0.0051933) [-0.13]

| eta:eta/1^S_0                | kaon:kaon/1^S_0               | pi:pi/1^S_0                   |
|------------------------------|-------------------------------|-------------------------------|
| k_re= -0.0232 +/- 0.0038     | k_re= -0.0345 +/- 0.0043      | k_re= 0.0733 +/- 0.0025       |
| k_im= 0.0355 +/- 0.0037      | k_im= 0.0239 +/- 0.0032       | k_im= -0.0112 +/- 0.0017      |
| corr= [ 0.35]                | corr= [ 0.23]                 | corr= [-0.08]                 |
| g = 0.0876 +/- 0.0194        | g = 0.1355 +/- 0.0112         | g = 0.1058 +/- 0.0105         |
| arg(g)/pi= 0.0899 +/- 0.0361 | arg(g)/pi= -0.8298 +/- 0.0178 | arg(g)/pi= -0.3924 +/- 0.0152 |
| g_re= 0.0842 +/- 0.0196      | g_re= -0.1166 +/- 0.0098      | g_re= 0.0351 +/- 0.0070       |
| g_im= 0.0244 +/- 0.0095      | g_im= -0.0690 +/- 0.0094      | g_im= -0.0998 +/- 0.0094      |
| corr= [ 0.14]                | corr= [ 0.41]                 | corr= [-0.66]                 |

JP=0+ || eta:eta/1^S\_0[+] kaon:kaon/1^S\_0[+] pi:pi/1^S\_0[-]

sqrt(s)\_pole = (0.093257 +/- 0.032178)  
+ (i/2)\*(+5.9586e-18 +/- 1.7847e-15) [-0.02]

| eta:eta/1^S_0                | kaon:kaon/1^S_0               | pi:pi/1^S_0                   |
|------------------------------|-------------------------------|-------------------------------|
| k_re= 0.0000 +/- 0.0000      | k_re= 0.0000 +/- 0.0000       | k_re= -0.0000 +/- 0.0000      |
| k_im= 0.0926 +/- 0.0081      | k_im= 0.0850 +/- 0.0088       | k_im= -0.0509 +/- 0.0147      |
| corr= [ 0.02]                | corr= [ 0.02]                 | corr= [ 0.02]                 |
| g = 0.0697 +/- 0.0295        | g = 0.0476 +/- 0.0288         | g = 0.0029 +/- 0.0114         |
| arg(g)/pi= 0.0000 +/- 0.0000 | arg(g)/pi= -0.0000 +/- 0.0000 | arg(g)/pi= -0.0000 +/- 0.0000 |
| g_re= 0.0697 +/- 0.0295      | g_re= 0.0476 +/- 0.0288       | g_re= 0.0029 +/- 0.0114       |
| g_im= 0.0000 +/- 0.0000      | g_im= -0.0000 +/- 0.0000      | g_im= -0.0000 +/- 0.0000      |
| corr= [-1.00]                | corr= [ 0.51]                 | corr= [-0.98]                 |

JP=0+ || eta:eta/1^S\_0[+] kaon:kaon/1^S\_0[-] pi:pi/1^S\_0[+]

sqrt(s)\_pole = ( 0.1092 +/- 0.026593)  
+ (i/2)\*(+5.075e-16 +/- 1.5183e-13) [-0.01]

| eta:eta/1^S_0                | kaon:kaon/1^S_0              | pi:pi/1^S_0                  |
|------------------------------|------------------------------|------------------------------|
| k_re= 0.0000 +/- 0.0000      | k_re= -0.0000 +/- 0.0000     | k_re= 0.0000 +/- 0.0000      |
| k_im= 0.0881 +/- 0.0082      | k_im= -0.0801 +/- 0.0091     | k_im= 0.0423 +/- 0.0172      |
| corr= [ 0.01]                | corr= [ 0.01]                | corr= [ 0.02]                |
| g = 0.0920 +/- 0.0183        | g = 0.0176 +/- 0.0090        | g = 0.0541 +/- 0.0275        |
| arg(g)/pi= 0.0000 +/- 0.0000 | arg(g)/pi= 1.0000 +/- 0.0000 | arg(g)/pi= 1.0000 +/- 0.0000 |
| g_re= 0.0920 +/- 0.0183      | g_re= -0.0176 +/- 0.0090     | g_re= -0.0541 +/- 0.0275     |
| g_im= 0.0000 +/- 0.0000      | g_im= 0.0000 +/- 0.0000      | g_im= 0.0000 +/- 0.0000      |
| corr= [-1.00]                | corr= [-0.93]                | corr= [-0.63]                |

JP=0+ || eta:eta/1^S\_0[+] kaon:kaon/1^S\_0[-] pi:pi/1^S\_0[-]

sqrt(s)\_pole = (0.12181 +/- 0.031756)  
+ (i/2)\*(-0.10108 +/- 0.027114) [-0.55]

| eta:eta/1^S_0                 | kaon:kaon/1^S_0              | pi:pi/1^S_0                   |
|-------------------------------|------------------------------|-------------------------------|
| k_re= -0.0172 +/- 0.0092      | k_re= 0.0188 +/- 0.0103      | k_re= 0.0302 +/- 0.0170       |
| k_im= 0.0893 +/- 0.0084       | k_im= -0.0818 +/- 0.0089     | k_im= -0.0511 +/- 0.0089      |
| corr= [ 0.79]                 | corr= [ 0.79]                | corr= [ 0.68]                 |
| g = 0.1135 +/- 0.0459         | g = 0.0656 +/- 0.0200        | g = 0.1062 +/- 0.0400         |
| arg(g)/pi= -0.1923 +/- 0.1004 | arg(g)/pi= 0.5215 +/- 0.0528 | arg(g)/pi= -0.6405 +/- 0.0411 |
| g_re= 0.0934 +/- 0.0542       | g_re= -0.0044 +/- 0.0114     | g_re= -0.0454 +/- 0.0233      |
| g_im= -0.0645 +/- 0.0212      | g_im= 0.0654 +/- 0.0197      | g_im= -0.0960 +/- 0.0353      |
| corr= [ 0.03]                 | corr= [-0.43]                | corr= [ 0.76]                 |

JP=0+ || eta:eta/1^S\_0[-] kaon:kaon/1^S\_0[+] pi:pi/1^S\_0[+]

sqrt(s)\_pole = ( 0.1283 +/- 0.0044961)  
+ (i/2)\*(+7.2508e-15 +/- 2.1634e-12) [-0.01]

| eta:eta/1^S_0                | kaon:kaon/1^S_0              | pi:pi/1^S_0                  |
|------------------------------|------------------------------|------------------------------|
| k_re= -0.0000 +/- 0.0000     | k_re= 0.0000 +/- 0.0000      | k_re= 0.0000 +/- 0.0000      |
| k_im= -0.0814 +/- 0.0018     | k_im= 0.0727 +/- 0.0020      | k_im= 0.0256 +/- 0.0056      |
| corr= [ 0.01]                | corr= [ 0.01]                | corr= [ 0.01]                |
| g = 0.0096 +/- 0.0095        | g = 0.0884 +/- 0.0093        | g = 0.0879 +/- 0.0027        |
| arg(g)/pi= 0.0000 +/- 0.0000 | arg(g)/pi= 1.0000 +/- 0.0000 | arg(g)/pi= 1.0000 +/- 0.0000 |
| g_re= 0.0096 +/- 0.0095      | g_re= -0.0884 +/- 0.0093     | g_re= -0.0879 +/- 0.0027     |
| g_im= 0.0000 +/- 0.0000      | g_im= 0.0000 +/- 0.0000      | g_im= 0.0000 +/- 0.0000      |
| corr= [-1.00]                | corr= [ 0.79]                | corr= [ 0.13]                |

\*\*\*\*\*

\*\*\*\*\*

JP=0+ || eta:eta/1^S\_0[-] kaon:kaon/1^S\_0[+] pi:pi/1^S\_0[-]

sqrt(s)\_pole = (0.18918 +/- 0.010151)  
+ (i/2)\*(-0.05912 +/- 0.013788) [ 0.13]

| eta:eta/1^S_0                 | kaon:kaon/1^S_0               | pi:pi/1^S_0                   |
|-------------------------------|-------------------------------|-------------------------------|
| k_re= 0.0268 +/- 0.0062       | k_re= -0.0332 +/- 0.0074      | k_re= 0.0664 +/- 0.0068       |
| k_im= -0.0522 +/- 0.0078      | k_im= 0.0421 +/- 0.0081       | k_im= -0.0211 +/- 0.0049      |
| corr= [ 0.32]                 | corr= [ 0.38]                 | corr= [ 0.24]                 |
| g = 0.0706 +/- 0.0124         | g = 0.1800 +/- 0.0113         | g = 0.1242 +/- 0.0140         |
| arg(g)/pi= -0.0822 +/- 0.1012 | arg(g)/pi= -0.8957 +/- 0.0457 | arg(g)/pi= -0.4217 +/- 0.0413 |
| g_re= 0.0682 +/- 0.0142       | g_re= -0.1704 +/- 0.0130      | g_re= 0.0302 +/- 0.0166       |
| g_im= -0.0180 +/- 0.0213      | g_im= -0.0579 +/- 0.0250      | g_im= -0.1204 +/- 0.0134      |
| corr= [ 0.43]                 | corr= [-0.45]                 | corr= [-0.11]                 |

\*\*\*\*\*

\*\*\*\*\*

JP=0+ || eta:eta/1^S\_0[-] kaon:kaon/1^S\_0[-] pi:pi/1^S\_0[-]

sqrt(s)\_pole = (0.12249 +/- 0.0066945)  
+ (i/2)\*(+1.5948e-18 +/- 4.7803e-16) [ 0.03]

| eta:eta/1^S_0                | kaon:kaon/1^S_0               | pi:pi/1^S_0                  |
|------------------------------|-------------------------------|------------------------------|
| k_re= -0.0000 +/- 0.0000     | k_re= -0.0000 +/- 0.0000      | k_re= -0.0000 +/- 0.0000     |
| k_im= -0.0836 +/- 0.0025     | k_im= -0.0752 +/- 0.0027      | k_im= -0.0319 +/- 0.0064     |
| corr= [-0.03]                | corr= [-0.03]                 | corr= [-0.03]                |
| g = 0.0278 +/- 0.0046        | g = 0.0414 +/- 0.0058         | g = 0.1062 +/- 0.0019        |
| arg(g)/pi= 0.5000 +/- 0.0000 | arg(g)/pi= -0.5000 +/- 0.0000 | arg(g)/pi= 0.5000 +/- 0.0000 |
| g_re= 0.0000 +/- 0.0000      | g_re= 0.0000 +/- 0.0000       | g_re= -0.0000 +/- 0.0000     |
| g_im= 0.0278 +/- 0.0046      | g_im= -0.0414 +/- 0.0058      | g_im= 0.1062 +/- 0.0019      |
| corr= [-1.00]                | corr= [-0.86]                 | corr= [-0.60]                |

\*\*\*\*\*

# k\_inv\_poly\_ccclcc\_noCM

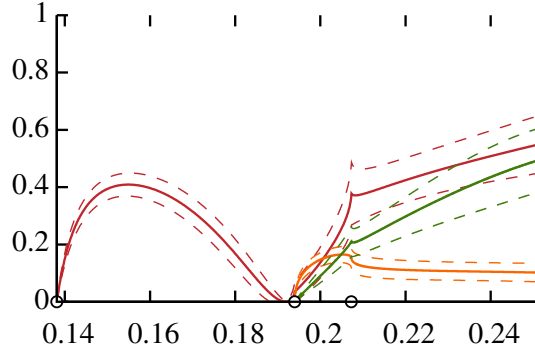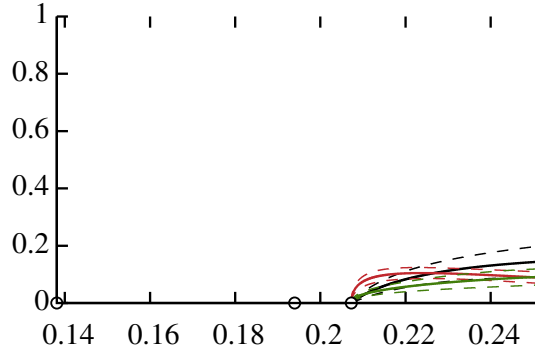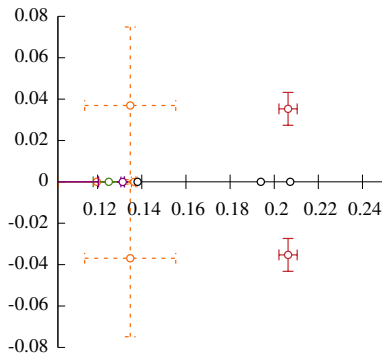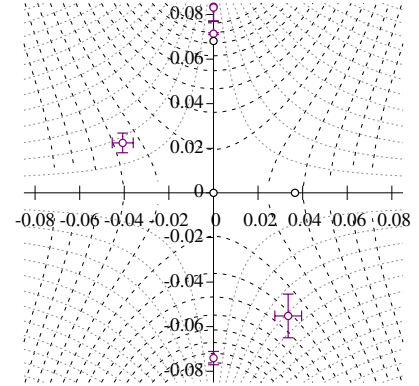

## parameter values

minimised with  $\text{chisq}/\text{nDoF} = 49.97 / (57 - 7) = 1.00$

|                                               |                        |      |      |       |       |       |       |       |
|-----------------------------------------------|------------------------|------|------|-------|-------|-------|-------|-------|
| JPO+_c_eta:eta/1^S_0 eta:eta/1^S_0_order0     | -0.82356 +/- 0.20214   | 1.00 | 0.90 | -0.49 | 0.17  | -0.11 | -0.15 | 0.02  |
| JPO+_c_eta:eta/1^S_0 kaon:kaon/1^S_0_order0   | -0.53391 +/- 0.15528   |      | 1.00 | -0.68 | 0.49  | -0.39 | -0.44 | 0.21  |
| JPO+_c_eta:eta/1^S_0 pi:pi/1^S_0_order0       | 0.50181 +/- 0.082744   |      |      | 1.00  | -0.59 | 0.53  | 0.81  | -0.64 |
| JPO+_c_kaon:kaon/1^S_0 kaon:kaon/1^S_0_order0 | -1.5940 +/- 0.49116    |      |      |       | 1.00  | -0.98 | -0.86 | 0.43  |
| JPO+_c_kaon:kaon/1^S_0 kaon:kaon/1^S_0_order1 | 0.77322 +/- 0.3513     |      |      |       |       | 1.00  | 0.82  | -0.38 |
| JPO+_c_kaon:kaon/1^S_0 pi:pi/1^S_0_order0     | -0.14325 +/- 0.14701   |      |      |       |       |       | 1.00  | -0.76 |
| JPO+_c_pi:pi/1^S_0 pi:pi/1^S_0_order0         | -0.015359 +/- 0.061282 |      |      |       |       |       |       | 1.00  |

## pole singularities

\*\*\*\*\*  
JP=0+ || eta:eta/1^S\_0[+] kaon:kaon/1^S\_0[+] pi:pi/1^S\_0[+]

$\text{sqrt}(s)_{\text{pole}} = (0.13136 \pm 0.00081309) + (i/2)*(-9.6645e-13 \pm 2.7586e-10) [-0.01]$

| eta:eta/1^S_0                | kaon:kaon/1^S_0              | pi:pi/1^S_0                  |
|------------------------------|------------------------------|------------------------------|
| k_re= -0.0000 +/- 0.0000     | k_re= -0.0000 +/- 0.0000     | k_re= -0.0000 +/- 0.0000     |
| k_im= 0.0802 +/- 0.0003      | k_im= 0.0714 +/- 0.0004      | k_im= 0.0213 +/- 0.0013      |
| corr= [ 0.01]                | corr= [ 0.01]                | corr= [ 0.01]                |
| g = 0.0398 +/- 0.0133        | g = 0.0548 +/- 0.0186        | g = 0.0897 +/- 0.0021        |
| arg(g)/pi= 0.0000 +/- 0.0000 | arg(g)/pi= 1.0000 +/- 0.0000 | arg(g)/pi= 1.0000 +/- 0.0000 |
| g_re= 0.0398 +/- 0.0133      | g_re= -0.0548 +/- 0.0186     | g_re= -0.0897 +/- 0.0021     |
| g_im= 0.0000 +/- 0.0000      | g_im= 0.0000 +/- 0.0000      | g_im= 0.0000 +/- 0.0000      |
| corr= [-1.00]                | corr= [-0.94]                | corr= [ 0.56]                |

\*\*\*\*\*  
JP=0+ || eta:eta/1^S\_0[+] kaon:kaon/1^S\_0[+] pi:pi/1^S\_0[+]

$\text{sqrt}(s)_{\text{pole}} = (0.098693 \pm 0.021563) + (i/2)*(+1.4381e-12 \pm 4.275e-10) [-0.06]$

| eta:eta/1^S_0 | kaon:kaon/1^S_0 | pi:pi/1^S_0 |
|---------------|-----------------|-------------|
|---------------|-----------------|-------------|



| eta:eta/1^S_0                | kaon:kaon/1^S_0               | pi:pi/1^S_0                  |
|------------------------------|-------------------------------|------------------------------|
| k_re= 0.0000 +/- 0.0000      | k_re= 0.0000 +/- 0.0000       | k_re= 0.0000 +/- 0.0000      |
| k_im= 0.0911 +/- 0.0058      | k_im= 0.0835 +/- 0.0064       | k_im= 0.0483 +/- 0.0110      |
| corr= [ 0.06]                | corr= [ 0.06]                 | corr= [ 0.06]                |
| g = 0.0502 +/- 0.0243        | g = 0.0833 +/- 0.0248         | g = 0.0138 +/- 0.0122        |
| arg(g)/pi= 0.0000 +/- 0.0000 | arg(g)/pi= -0.0000 +/- 0.0000 | arg(g)/pi= 1.0000 +/- 0.0000 |
| g_re= 0.0502 +/- 0.0243      | g_re= 0.0833 +/- 0.0248       | g_re= -0.0138 +/- 0.0122     |
| g_im= 0.0000 +/- 0.0000      | g_im= -0.0000 +/- 0.0000      | g_im= 0.0000 +/- 0.0000      |
| corr= [-1.00]                | corr= [ 0.22]                 | corr= [-0.54]                |

JP=0+ || eta:eta/1^S\_0[+] kaon:kaon/1^S\_0[+] pi:pi/1^S\_0[-]

sqrt(s)\_pole = (0.099977 +/- 0.020432)  
+ (i/2)\*(+4.7996e-14 +/- 1.4384e-11) [-0.06]

| eta:eta/1^S_0                | kaon:kaon/1^S_0               | pi:pi/1^S_0                   |
|------------------------------|-------------------------------|-------------------------------|
| k_re= 0.0000 +/- 0.0000      | k_re= 0.0000 +/- 0.0000       | k_re= -0.0000 +/- 0.0000      |
| k_im= 0.0908 +/- 0.0056      | k_im= 0.0831 +/- 0.0062       | k_im= -0.0476 +/- 0.0107      |
| corr= [ 0.06]                | corr= [ 0.06]                 | corr= [ 0.06]                 |
| g = 0.0444 +/- 0.0221        | g = 0.0915 +/- 0.0226         | g = 0.0095 +/- 0.0089         |
| arg(g)/pi= 0.0000 +/- 0.0000 | arg(g)/pi= -0.0000 +/- 0.0000 | arg(g)/pi= -0.0000 +/- 0.0000 |
| g_re= 0.0444 +/- 0.0221      | g_re= 0.0915 +/- 0.0226       | g_re= 0.0095 +/- 0.0089       |
| g_im= 0.0000 +/- 0.0000      | g_im= -0.0000 +/- 0.0000      | g_im= -0.0000 +/- 0.0000      |
| corr= [-1.00]                | corr= [ 0.47]                 | corr= [-0.74]                 |

JP=0+ || eta:eta/1^S\_0[+] kaon:kaon/1^S\_0[+] pi:pi/1^S\_0[-]

sqrt(s)\_pole = (0.20627 +/- 0.0041458)  
+ (i/2)\*(-0.035272 +/- 0.007938) [-0.05]

| eta:eta/1^S_0                | kaon:kaon/1^S_0               | pi:pi/1^S_0                   |
|------------------------------|-------------------------------|-------------------------------|
| k_re= -0.0287 +/- 0.0050     | k_re= -0.0407 +/- 0.0047      | k_re= 0.0770 +/- 0.0028       |
| k_im= 0.0317 +/- 0.0048      | k_im= 0.0224 +/- 0.0044       | k_im= -0.0118 +/- 0.0026      |
| corr= [ 0.04]                | corr= [ 0.00]                 | corr= [-0.04]                 |
| g = 0.1504 +/- 0.0162        | g = 0.1403 +/- 0.0225         | g = 0.1262 +/- 0.0188         |
| arg(g)/pi= 0.1269 +/- 0.0354 | arg(g)/pi= -0.7990 +/- 0.0516 | arg(g)/pi= -0.3299 +/- 0.0305 |
| g_re= 0.1386 +/- 0.0179      | g_re= -0.1133 +/- 0.0211      | g_re= 0.0643 +/- 0.0116       |
| g_im= 0.0584 +/- 0.0148      | g_im= -0.0829 +/- 0.0240      | g_im= -0.1086 +/- 0.0192      |
| corr= [-0.23]                | corr= [ 0.03]                 | corr= [-0.25]                 |

JP=0+ || eta:eta/1^S\_0[+] kaon:kaon/1^S\_0[-] pi:pi/1^S\_0[+]

sqrt(s)\_pole = (0.12504 +/- 0.0070406)  
+ (i/2)\*(+1.2868e-13 +/- 3.8537e-11) [-0.01]

| eta:eta/1^S_0                | kaon:kaon/1^S_0              | pi:pi/1^S_0                  |
|------------------------------|------------------------------|------------------------------|
| k_re= 0.0000 +/- 0.0000      | k_re= -0.0000 +/- 0.0000     | k_re= 0.0000 +/- 0.0000      |
| k_im= 0.0827 +/- 0.0027      | k_im= -0.0741 +/- 0.0030     | k_im= 0.0293 +/- 0.0075      |
| corr= [ 0.01]                | corr= [ 0.01]                | corr= [ 0.01]                |
| g = 0.0756 +/- 0.0088        | g = 0.0113 +/- 0.0077        | g = 0.0871 +/- 0.0053        |
| arg(g)/pi= 0.0000 +/- 0.0000 | arg(g)/pi= 1.0000 +/- 0.0000 | arg(g)/pi= 1.0000 +/- 0.0000 |
| g_re= 0.0756 +/- 0.0088      | g_re= -0.0113 +/- 0.0077     | g_re= -0.0871 +/- 0.0053     |
| g_im= 0.0000 +/- 0.0000      | g_im= 0.0000 +/- 0.0000      | g_im= 0.0000 +/- 0.0000      |
| corr= [-1.00]                | corr= [-0.95]                | corr= [-0.99]                |

JP=0+ || eta:eta/1^S\_0[+] kaon:kaon/1^S\_0[-] pi:pi/1^S\_0[-]

sqrt(s)\_pole = (0.17789 +/- 0.013277)  
+ (i/2)\*(-0.083221 +/- 0.018563) [ 0.48]

| eta:eta/1^S_0                 | kaon:kaon/1^S_0              | pi:pi/1^S_0                   |
|-------------------------------|------------------------------|-------------------------------|
| k_re= -0.0289 +/- 0.0052      | k_re= 0.0335 +/- 0.0060      | k_re= 0.0604 +/- 0.0081       |
| k_im= 0.0640 +/- 0.0092       | k_im= -0.0552 +/- 0.0098     | k_im= -0.0306 +/- 0.0073      |
| corr= [ 0.25]                 | corr= [ 0.37]                | corr= [ 0.56]                 |
| g = 0.1798 +/- 0.0165         | g = 0.0602 +/- 0.0064        | g = 0.1303 +/- 0.0117         |
| arg(g)/pi= -0.0595 +/- 0.0444 | arg(g)/pi= 0.7256 +/- 0.0496 | arg(g)/pi= -0.4945 +/- 0.0358 |
| g_re= 0.1766 +/- 0.0187       | g_re= -0.0392 +/- 0.0073     | g_re= 0.0023 +/- 0.0148       |
| g_im= -0.0334 +/- 0.0235      | g_im= 0.0457 +/- 0.0087      | g_im= -0.1303 +/- 0.0116      |
| corr= [ 0.52]                 | corr= [ 0.40]                | corr= [-0.48]                 |

JP=0+ || eta:eta/1^S\_0[-] kaon:kaon/1^S\_0[+] pi:pi/1^S\_0[+]

sqrt(s)\_pole = (0.24822 +/- 0.027871)  
+ (i/2)\*(-0.14961 +/- 0.093191) [-0.89]

| eta:eta/1^S_0                | kaon:kaon/1^S_0               | pi:pi/1^S_0                  |
|------------------------------|-------------------------------|------------------------------|
| k_re= 0.0809 +/- 0.0263      | k_re= -0.0865 +/- 0.0243      | k_re= -0.1057 +/- 0.0181     |
| k_im= -0.0573 +/- 0.0238     | k_im= 0.0537 +/- 0.0246       | k_im= 0.0439 +/- 0.0248      |
| corr= [-0.92]                | corr= [-0.92]                 | corr= [-0.91]                |
| g = 0.1107 +/- 0.0164        | g = 0.2442 +/- 0.0504         | g = 0.1021 +/- 0.0341        |
| arg(g)/pi= 0.4274 +/- 0.0309 | arg(g)/pi= -0.4991 +/- 0.0182 | arg(g)/pi= 0.9825 +/- 0.0509 |
| g_re= 0.0250 +/- 0.0108      | g_re= 0.0007 +/- 0.0141       | g_re= -0.1019 +/- 0.0347     |
| g_im= 0.1078 +/- 0.0164      | g_im= -0.2442 +/- 0.0504      | g_im= 0.0056 +/- 0.0149      |
| corr= [ 0.10]                | corr= [-0.98]                 | corr= [ 0.73]                |

\*\*\*\*\*

\*\*\*\*\*

JP=0+ || eta:eta/1^S\_0[-] kaon:kaon/1^S\_0[+] pi:pi/1^S\_0[+]

sqrt(s)\_pole = (0.11969 +/- 0.017513)  
+ (i/2)\*(+6.8186e-16 +/- 2.0343e-13) [-0.07]

| eta:eta/1^S_0                | kaon:kaon/1^S_0              | pi:pi/1^S_0                  |
|------------------------------|------------------------------|------------------------------|
| k_re= -0.0000 +/- 0.0000     | k_re= 0.0000 +/- 0.0000      | k_re= 0.0000 +/- 0.0000      |
| k_im= -0.0846 +/- 0.0062     | k_im= 0.0763 +/- 0.0069      | k_im= 0.0345 +/- 0.0152      |
| corr= [ 0.07]                | corr= [ 0.07]                | corr= [ 0.07]                |
| g = 0.0191 +/- 0.0126        | g = 0.1269 +/- 0.0127        | g = 0.0497 +/- 0.0417        |
| arg(g)/pi= 0.0000 +/- 0.0000 | arg(g)/pi= 1.0000 +/- 0.0000 | arg(g)/pi= 1.0000 +/- 0.0000 |
| g_re= 0.0191 +/- 0.0126      | g_re= -0.1269 +/- 0.0127     | g_re= -0.0497 +/- 0.0417     |
| g_im= 0.0000 +/- 0.0000      | g_im= 0.0000 +/- 0.0000      | g_im= 0.0000 +/- 0.0000      |
| corr= [-1.00]                | corr= [ 0.75]                | corr= [-0.96]                |

\*\*\*\*\*

\*\*\*\*\*

JP=0+ || eta:eta/1^S\_0[-] kaon:kaon/1^S\_0[+] pi:pi/1^S\_0[-]

sqrt(s)\_pole = (0.13477 +/- 0.020642)  
+ (i/2)\*(-0.036887 +/- 0.037938) [-0.92]

| eta:eta/1^S_0                 | kaon:kaon/1^S_0              | pi:pi/1^S_0                   |
|-------------------------------|------------------------------|-------------------------------|
| k_re= 0.0078 +/- 0.0097       | k_re= -0.0088 +/- 0.0111     | k_re= 0.0220 +/- 0.0261       |
| k_im= -0.0797 +/- 0.0069      | k_im= 0.0709 +/- 0.0074      | k_im= -0.0283 +/- 0.0052      |
| corr= [ 0.91]                 | corr= [ 0.91]                | corr= [ 0.17]                 |
| g = 0.0522 +/- 0.0073         | g = 0.1428 +/- 0.0281        | g = 0.0840 +/- 0.0171         |
| arg(g)/pi= -0.2722 +/- 0.0457 | arg(g)/pi= 0.8868 +/- 0.0963 | arg(g)/pi= -0.4497 +/- 0.1689 |
| g_re= 0.0342 +/- 0.0076       | g_re= -0.1338 +/- 0.0406     | g_re= 0.0132 +/- 0.0414       |
| g_im= -0.0394 +/- 0.0072      | g_im= 0.0497 +/- 0.0318      | g_im= -0.0830 +/- 0.0237      |
| corr= [ 0.02]                 | corr= [ 0.92]                | corr= [ 0.99]                 |

\*\*\*\*\*

\*\*\*\*\*

JP=0+ || eta:eta/1^S\_0[-] kaon:kaon/1^S\_0[-] pi:pi/1^S\_0[-]

sqrt(s)\_pole = (0.13658 +/- 0.0012692)  
+ (i/2)\*(-6.2058e-17 +/- 1.8503e-14) [-0.04]

| eta:eta/1^S_0                | kaon:kaon/1^S_0               | pi:pi/1^S_0                  |
|------------------------------|-------------------------------|------------------------------|
| k_re= 0.0000 +/- 0.0000      | k_re= 0.0000 +/- 0.0000       | k_re= 0.0000 +/- 0.0000      |
| k_im= -0.0780 +/- 0.0006     | k_im= -0.0689 +/- 0.0006      | k_im= -0.0103 +/- 0.0042     |
| corr= [ 0.04]                | corr= [ 0.04]                 | corr= [ 0.04]                |
| g = 0.0213 +/- 0.0036        | g = 0.0098 +/- 0.0066         | g = 0.0729 +/- 0.0134        |
| arg(g)/pi= 0.5000 +/- 0.0000 | arg(g)/pi= -0.5000 +/- 0.0000 | arg(g)/pi= 0.5000 +/- 0.0000 |
| g_re= 0.0000 +/- 0.0000      | g_re= 0.0000 +/- 0.0000       | g_re= -0.0000 +/- 0.0000     |
| g_im= 0.0213 +/- 0.0036      | g_im= -0.0098 +/- 0.0066      | g_im= 0.0729 +/- 0.0134      |
| corr= [-1.00]                | corr= [-0.87]                 | corr= [ 0.56]                |

\*\*\*\*\*

# k\_inv\_poly\_llcccc\_noCM

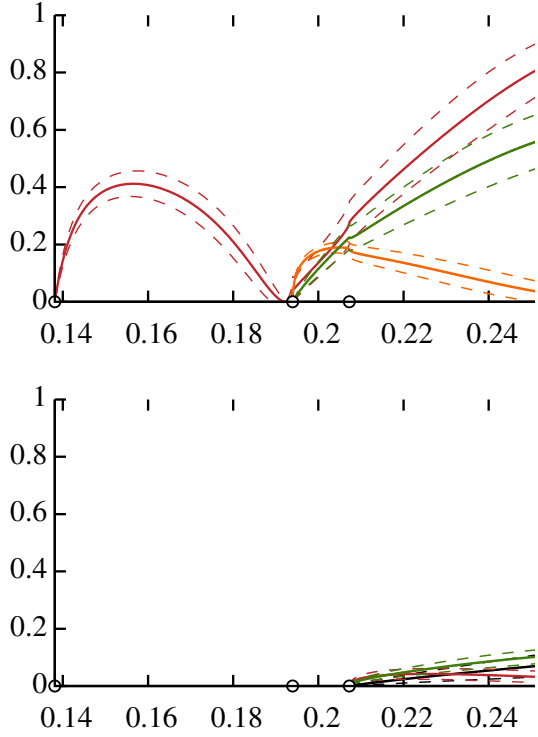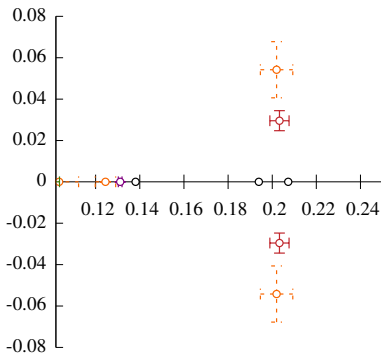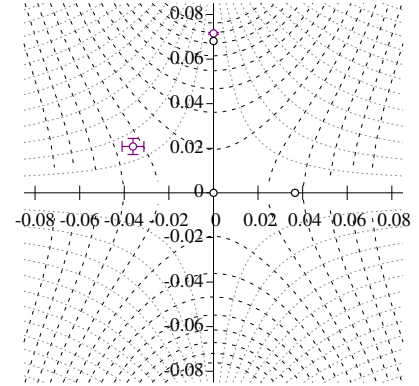

## parameter values

minimised with  $\text{chisq}/\text{nDoF} = 47.39 / (57 - 8) = 0.97$

|                                               |                      |      |       |       |       |       |       |       |       |
|-----------------------------------------------|----------------------|------|-------|-------|-------|-------|-------|-------|-------|
| JP0+_c_eta:eta/1^S_0 eta:eta/1^S_0_order0     | -2.4294 +/- 0.86726  | 1.00 | 0.86  | 0.01  | 0.17  | 0.25  | -0.06 | -0.13 | -0.11 |
| JP0+_c_eta:eta/1^S_0 kaon:kaon/1^S_0_order0   | -1.1833 +/- 0.31432  | 1.00 | -0.08 | 0.61  | 0.18  | -0.17 | -0.16 | -0.02 |       |
| JP0+_c_eta:eta/1^S_0 pi:pi/1^S_0_order0       | 0.51449 +/- 0.17904  |      | 1.00  | -0.10 | 0.57  | 0.18  | 0.16  | -0.50 |       |
| JP0+_c_kaon:kaon/1^S_0 kaon:kaon/1^S_0_order0 | -0.82296 +/- 0.18717 |      |       | 1.00  | -0.08 | -0.25 | -0.04 | 0.04  |       |
| JP0+_c_kaon:kaon/1^S_0 pi:pi/1^S_0_order0     | -0.91816 +/- 0.1314  |      |       |       | 1.00  | -0.56 | -0.61 | 0.15  |       |
| JP0+_c_kaon:kaon/1^S_0 pi:pi/1^S_0_order1     | 0.57724 +/- 0.11202  |      |       |       |       | 1.00  | 0.67  | -0.50 |       |
| JP0+_c_pi:pi/1^S_0 pi:pi/1^S_0_order0         | 0.49371 +/- 0.13915  |      |       |       |       |       | 1.00  | -0.83 |       |
| JP0+_c_pi:pi/1^S_0 pi:pi/1^S_0_order1         | -0.22607 +/- 0.13551 |      |       |       |       |       |       | 1.00  |       |

## pole singularities

\*\*\*\*\*  
JP=0+ || eta:eta/1^S\_0[+] kaon:kaon/1^S\_0[+] pi:pi/1^S\_0[+]

$\text{sqrt}(s)_{\text{pole}} = (0.13113 \pm 0.0008526) + (i/2) * (1.5112e-12 \pm 4.4495e-10) [0.04]$

| eta:eta/1^S_0                | kaon:kaon/1^S_0              | pi:pi/1^S_0                  |
|------------------------------|------------------------------|------------------------------|
| k_re= 0.0000 +/- 0.0000      | k_re= 0.0000 +/- 0.0000      | k_re= 0.0000 +/- 0.0000      |
| k_im= 0.0803 +/- 0.0003      | k_im= 0.0715 +/- 0.0004      | k_im= 0.0217 +/- 0.0013      |
| corr= [-0.04]                | corr= [-0.04]                | corr= [-0.04]                |
| g = 0.0331 +/- 0.0106        | g = 0.0725 +/- 0.0073        | g = 0.0894 +/- 0.0021        |
| arg(g)/pi= 0.0000 +/- 0.0000 | arg(g)/pi= 1.0000 +/- 0.0000 | arg(g)/pi= 1.0000 +/- 0.0000 |
| g_re= 0.0331 +/- 0.0106      | g_re= -0.0725 +/- 0.0073     | g_re= -0.0894 +/- 0.0021     |
| g_im= 0.0000 +/- 0.0000      | g_im= 0.0000 +/- 0.0000      | g_im= 0.0000 +/- 0.0000      |
| corr= [-1.00]                | corr= [-0.77]                | corr= [-0.10]                |

\*\*\*\*\*  
JP=0+ || eta:eta/1^S\_0[+] kaon:kaon/1^S\_0[+] pi:pi/1^S\_0[-]

$\text{sqrt}(s)_{\text{pole}} = (0.2033 \pm 0.0043477) + (i/2) * (-0.029575 \pm 0.0048465) [0.06]$

| eta:eta/1^S_0 | kaon:kaon/1^S_0 | pi:pi/1^S_0 |
|---------------|-----------------|-------------|
|---------------|-----------------|-------------|

```

=====|=====|=====|
k_re= -0.0236 +/- 0.0042 | k_re= -0.0361 +/- 0.0049 | k_re= 0.0749 +/- 0.0029 |
k_im= 0.0319 +/- 0.0048 | k_im= 0.0208 +/- 0.0036 | k_im= -0.0100 +/- 0.0017 |
corr= [ 0.52] | corr= [ 0.46] | corr= [ 0.14] |
=====|=====|=====|
|g|= 0.0732 +/- 0.0135 | |g|= 0.1353 +/- 0.0089 | |g|= 0.1034 +/- 0.0100 |
arg(g)/pi= 0.1351 +/- 0.0319 | arg(g)/pi= -0.7953 +/- 0.0248 | arg(g)/pi= -0.3660 +/- 0.0272 |
=====|=====|=====|
g_re= 0.0667 +/- 0.0131 | g_re= -0.1083 +/- 0.0099 | g_re= 0.0423 +/- 0.0109 |
g_im= 0.0301 +/- 0.0079 | g_im= -0.0811 +/- 0.0097 | g_im= -0.0944 +/- 0.0077 |
corr= [ 0.36] | corr= [-0.18] | corr= [-0.50] |
=====|=====|=====|

```

```

*****
JP=0+ || eta:eta/1^S_0[+] kaon:kaon/1^S_0[-] pi:pi/1^S_0[+]

```

```

sqrt(s)_pole = (0.082516 +/- 0.021108)
+ (i/2)*(+5.1525e-19 +/- 1.5405e-16) [-0.01]

```

```

=====|=====|=====|
eta:eta/1^S_0 | kaon:kaon/1^S_0 | pi:pi/1^S_0 |
=====|=====|=====|
k_re= 0.0000 +/- 0.0000 | k_re= -0.0000 +/- 0.0000 | k_re= 0.0000 +/- 0.0000 |
k_im= 0.0951 +/- 0.0046 | k_im= -0.0878 +/- 0.0050 | k_im= 0.0554 +/- 0.0079 |
corr= [ 0.02] | corr= [ 0.02] | corr= [ 0.02] |
=====|=====|=====|
|g|= 0.0691 +/- 0.0223 | |g|= 0.0198 +/- 0.0053 | |g|= 0.0288 +/- 0.0162 |
arg(g)/pi= 0.0000 +/- 0.0000 | arg(g)/pi= 1.0000 +/- 0.0000 | arg(g)/pi= 1.0000 +/- 0.0000 |
=====|=====|=====|
g_re= 0.0691 +/- 0.0223 | g_re= -0.0198 +/- 0.0053 | g_re= -0.0288 +/- 0.0162 |
g_im= 0.0000 +/- 0.0000 | g_im= 0.0000 +/- 0.0000 | g_im= 0.0000 +/- 0.0000 |
corr= [-1.00] | corr= [ 0.56] | corr= [ 0.18] |
=====|=====|=====|

```

```

*****
JP=0+ || eta:eta/1^S_0[+] kaon:kaon/1^S_0[-] pi:pi/1^S_0[-]

```

```

sqrt(s)_pole = (0.08398 +/- 0.013701)
+ (i/2)*(-0.079298 +/- 0.02859) [-0.60]

```

```

=====|=====|=====|
eta:eta/1^S_0 | kaon:kaon/1^S_0 | pi:pi/1^S_0 |
=====|=====|=====|
k_re= -0.0086 +/- 0.0041 | k_re= 0.0092 +/- 0.0045 | k_re= 0.0139 +/- 0.0067 |
k_im= 0.0972 +/- 0.0023 | k_im= -0.0901 +/- 0.0024 | k_im= -0.0599 +/- 0.0034 |
corr= [ 0.30] | corr= [ 0.29] | corr= [ 0.12] |
=====|=====|=====|
|g|= 0.0655 +/- 0.0152 | |g|= 0.0411 +/- 0.0082 | |g|= 0.0654 +/- 0.0172 |
arg(g)/pi= -0.2637 +/- 0.0455 | arg(g)/pi= 0.4614 +/- 0.0801 | arg(g)/pi= -0.6805 +/- 0.1022 |
=====|=====|=====|
g_re= 0.0443 +/- 0.0144 | g_re= 0.0050 +/- 0.0104 | g_re= -0.0351 +/- 0.0247 |
g_im= -0.0483 +/- 0.0106 | g_im= 0.0408 +/- 0.0082 | g_im= -0.0552 +/- 0.0112 |
corr= [-0.50] | corr= [ 0.01] | corr= [ 0.12] |
=====|=====|=====|

```

```

*****
JP=0+ || eta:eta/1^S_0[-] kaon:kaon/1^S_0[+] pi:pi/1^S_0[+]

```

```

sqrt(s)_pole = (0.12444 +/- 0.0046238)
+ (i/2)*(+2.4689e-16 +/- 7.3684e-14) [-0.00]

```

```

=====|=====|=====|
eta:eta/1^S_0 | kaon:kaon/1^S_0 | pi:pi/1^S_0 |
=====|=====|=====|
k_re= -0.0000 +/- 0.0000 | k_re= 0.0000 +/- 0.0000 | k_re= 0.0000 +/- 0.0000 |
k_im= -0.0829 +/- 0.0017 | k_im= 0.0744 +/- 0.0019 | k_im= 0.0300 +/- 0.0048 |
corr= [ 0.00] | corr= [ 0.00] | corr= [ 0.00] |
=====|=====|=====|
|g|= 0.0189 +/- 0.0060 | |g|= 0.0975 +/- 0.0057 | |g|= 0.0862 +/- 0.0039 |
arg(g)/pi= 0.0000 +/- 0.0000 | arg(g)/pi= 1.0000 +/- 0.0000 | arg(g)/pi= 1.0000 +/- 0.0000 |
=====|=====|=====|
g_re= 0.0189 +/- 0.0060 | g_re= -0.0975 +/- 0.0057 | g_re= -0.0862 +/- 0.0039 |
g_im= 0.0000 +/- 0.0000 | g_im= 0.0000 +/- 0.0000 | g_im= 0.0000 +/- 0.0000 |
corr= [-1.00] | corr= [ 0.43] | corr= [-0.38] |
=====|=====|=====|

```

```

*****
JP=0+ || eta:eta/1^S_0[-] kaon:kaon/1^S_0[+] pi:pi/1^S_0[-]

```

```

sqrt(s)_pole = (0.20197 +/- 0.0073459)
+ (i/2)*(-0.05421 +/- 0.01356) [ 0.15]

```

```

=====|=====|=====|
eta:eta/1^S_0 | kaon:kaon/1^S_0 | pi:pi/1^S_0 |
=====|=====|=====|
k_re= 0.0324 +/- 0.0063 | k_re= -0.0413 +/- 0.0065 | k_re= 0.0747 +/- 0.0048 |
k_im= -0.0422 +/- 0.0073 | k_im= 0.0331 +/- 0.0071 | k_im= -0.0183 +/- 0.0046 |
corr= [ 0.08] | corr= [ 0.14] | corr= [ 0.16] |
=====|=====|=====|
|g|= 0.0738 +/- 0.0158 | |g|= 0.1730 +/- 0.0124 | |g|= 0.1243 +/- 0.0145 |
arg(g)/pi= 0.0454 +/- 0.0644 | arg(g)/pi= -0.8138 +/- 0.0303 | arg(g)/pi= -0.3456 +/- 0.0315 |
=====|=====|=====|
g_re= 0.0731 +/- 0.0168 | g_re= -0.1442 +/- 0.0161 | g_re= 0.0580 +/- 0.0143 |
g_im= 0.0105 +/- 0.0138 | g_im= -0.0956 +/- 0.0129 | g_im= -0.1100 +/- 0.0125 |
corr= [-0.45] | corr= [-0.40] | corr= [-0.30] |
=====|=====|=====|

```

```

*****
JP=0+ || eta:eta/1^S_0[-] kaon:kaon/1^S_0[-] pi:pi/1^S_0[-]

```

```

sqrt(s)_pole = (0.10349 +/- 0.0087698)

```

+ (i/2)\*(+2.2238e-14 +/- 6.6569e-12) [ 0.04]

| eta:eta/1^S_0                | kaon:kaon/1^S_0               | pi:pi/1^S_0                  |
|------------------------------|-------------------------------|------------------------------|
| =====                        | =====                         | =====                        |
| k_re= -0.0000 +/- 0.0000     | k_re= -0.0000 +/- 0.0000      | k_re= -0.0000 +/- 0.0000     |
| k_im= -0.0898 +/- 0.0025     | k_im= -0.0820 +/- 0.0028      | k_im= -0.0457 +/- 0.0050     |
| corr= [-0.04]                | corr= [-0.04]                 | corr= [-0.04]                |
| =====                        | =====                         | =====                        |
| g = 0.0246 +/- 0.0053        | g = 0.0433 +/- 0.0034         | g = 0.0996 +/- 0.0078        |
| arg(g)/pi= 0.5000 +/- 0.0000 | arg(g)/pi= -0.5000 +/- 0.0000 | arg(g)/pi= 0.5000 +/- 0.0000 |
| =====                        | =====                         | =====                        |
| g_re= 0.0000 +/- 0.0000      | g_re= 0.0000 +/- 0.0000       | g_re= -0.0000 +/- 0.0000     |
| g_im= 0.0246 +/- 0.0053      | g_im= -0.0433 +/- 0.0034      | g_im= 0.0996 +/- 0.0078      |
| corr= [-1.00]                | corr= [-0.43]                 | corr= [ 0.39]                |
| =====                        | =====                         | =====                        |

\*\*\*\*\*

# k\_inv\_poly\_lcclcc\_noCM

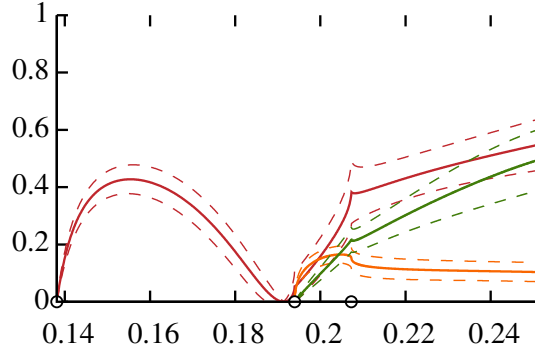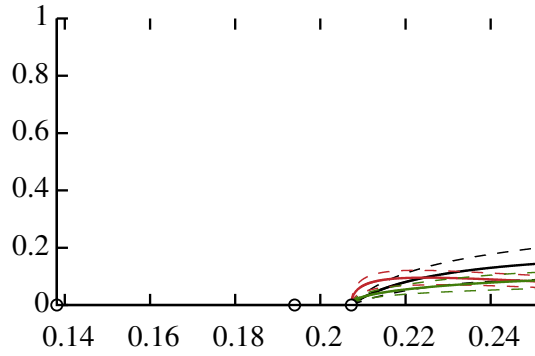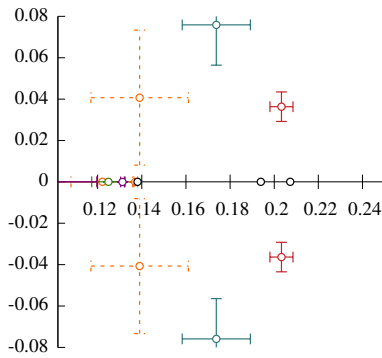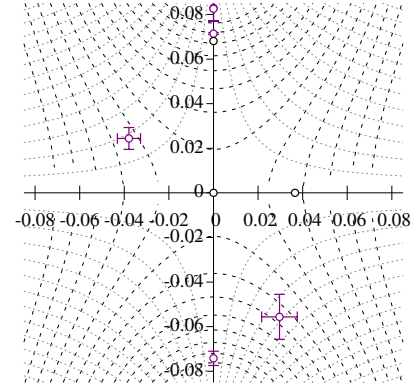

## parameter values

minimised with chisq/nDoF = 49.49 / (57 - 8) = 1.01

|                                               |                        |      |       |       |       |       |       |       |       |
|-----------------------------------------------|------------------------|------|-------|-------|-------|-------|-------|-------|-------|
| JPO+_c_eta:eta/1^S_0 eta:eta/1^S_0_order0     | -0.85933 +/- 0.2303    | 1.00 | 0.88  | -0.27 | -0.09 | 0.16  | 0.06  | 0.18  | -0.24 |
| JPO+_c_eta:eta/1^S_0 kaon:kaon/1^S_0_order0   | -0.53774 +/- 0.15497   | 1.00 | -0.56 | 0.31  | -0.19 | -0.29 | 0.08  | 0.03  |       |
| JPO+_c_eta:eta/1^S_0 pi:pi/1^S_0_order0       | 0.47608 +/- 0.092484   | 1.00 | -0.57 | 0.50  | 0.82  | 0.01  | -0.51 |       |       |
| JPO+_c_kaon:kaon/1^S_0 kaon:kaon/1^S_0_order0 | -1.5170 +/- 0.46447    | 1.00 | -0.97 | -0.83 | -0.17 | 0.48  |       |       |       |
| JPO+_c_kaon:kaon/1^S_0 kaon:kaon/1^S_0_order1 | 0.71829 +/- 0.33785    |      |       |       |       | 1.00  | 0.78  | 0.20  | -0.47 |
| JPO+_c_kaon:kaon/1^S_0 pi:pi/1^S_0_order0     | -0.16339 +/- 0.13886   |      |       |       |       | 1.00  | -0.13 | -0.44 |       |
| JPO+_c_pi:pi/1^S_0 pi:pi/1^S_0_order0         | -0.071467 +/- 0.088953 |      |       |       |       | 1.00  | -0.75 |       |       |
| JPO+_c_pi:pi/1^S_0 pi:pi/1^S_0_order1         | 0.089283 +/- 0.12146   |      |       |       |       |       | 1.00  |       |       |

## pole singularities

\*\*\*\*\*  
JP=0+ || eta:eta/1^S\_0[+] kaon:kaon/1^S\_0[+] pi:pi/1^S\_0[+]

sqrt(s)\_pole = (0.13126 +/- 0.00084395)  
+ (i/2)\*(-2.2446e-14 +/- 5.9616e-12) [-0.04]

| eta:eta/1^S_0                | kaon:kaon/1^S_0              | pi:pi/1^S_0                  |
|------------------------------|------------------------------|------------------------------|
| k_re= -0.0000 +/- 0.0000     | k_re= -0.0000 +/- 0.0000     | k_re= -0.0000 +/- 0.0000     |
| k_im= 0.0802 +/- 0.0003      | k_im= 0.0714 +/- 0.0004      | k_im= 0.0215 +/- 0.0013      |
| corr= [ 0.04]                | corr= [ 0.04]                | corr= [ 0.04]                |
| g = 0.0380 +/- 0.0152        | g = 0.0551 +/- 0.0193        | g = 0.0912 +/- 0.0026        |
| arg(g)/pi= 0.0000 +/- 0.0000 | arg(g)/pi= 1.0000 +/- 0.0000 | arg(g)/pi= 1.0000 +/- 0.0000 |
| g_re= 0.0380 +/- 0.0152      | g_re= -0.0551 +/- 0.0193     | g_re= -0.0912 +/- 0.0026     |
| g_im= 0.0000 +/- 0.0000      | g_im= 0.0000 +/- 0.0000      | g_im= 0.0000 +/- 0.0000      |
| corr= [-1.00]                | corr= [-0.94]                | corr= [ 0.25]                |

\*\*\*\*\*  
JP=0+ || eta:eta/1^S\_0[+] kaon:kaon/1^S\_0[+] pi:pi/1^S\_0[+]

sqrt(s)\_pole = (0.10059 +/- 0.019146)  
+ (i/2)\*(+6.8761e-17 +/- 2.0476e-14) [-0.06]

| eta:eta/1^S_0 | kaon:kaon/1^S_0 | pi:pi/1^S_0 |
|---------------|-----------------|-------------|
|---------------|-----------------|-------------|

```

=====|=====|=====|
k_re= 0.0000 +/- 0.0000 | k_re= 0.0000 +/- 0.0000 | k_re= 0.0000 +/- 0.0000 |
k_im= 0.0906 +/- 0.0053 | k_im= 0.0829 +/- 0.0058 | k_im= 0.0473 +/- 0.0102 |
corr= [ 0.06] | corr= [ 0.06] | corr= [ 0.06] |
=====|=====|=====|
|g|= 0.0544 +/- 0.0243 | |g|= 0.0831 +/- 0.0244 | |g|= 0.0138 +/- 0.0135 |
arg(g)/pi= 0.0000 +/- 0.0000 | arg(g)/pi= -0.0000 +/- 0.0000 | arg(g)/pi= 1.0000 +/- 0.0000 |
=====|=====|=====|
g_re= 0.0544 +/- 0.0243 | g_re= 0.0831 +/- 0.0244 | g_re= -0.0138 +/- 0.0135 |
g_im= 0.0000 +/- 0.0000 | g_im= -0.0000 +/- 0.0000 | g_im= 0.0000 +/- 0.0000 |
corr= [-1.00] | corr= [-0.12] | corr= [-0.66] |
=====|=====|=====|

```

```

*****
JP=0+ || eta:eta/1^S_0[+] kaon:kaon/1^S_0[+] pi:pi/1^S_0[-]

```

```

sqrt(s)_pole = (0.20327 +/- 0.0052176)
+ (i/2)*(-0.036341 +/- 0.0071189) [ 0.21]

```

```

=====|=====|=====|
eta:eta/1^S_0 | kaon:kaon/1^S_0 | pi:pi/1^S_0 |
=====|=====|=====|
k_re= -0.0266 +/- 0.0046 | k_re= -0.0379 +/- 0.0052 | k_re= 0.0750 +/- 0.0035 |
k_im= 0.0347 +/- 0.0058 | k_im= 0.0244 +/- 0.0049 | k_im= -0.0123 +/- 0.0024 |
corr= [ 0.36] | corr= [ 0.41] | corr= [ 0.26] |
=====|=====|=====|
|g|= 0.1462 +/- 0.0182 | |g|= 0.1413 +/- 0.0233 | |g|= 0.1213 +/- 0.0151 |
arg(g)/pi= 0.1074 +/- 0.0414 | arg(g)/pi= -0.8289 +/- 0.0607 | arg(g)/pi= -0.3647 +/- 0.0546 |
=====|=====|=====|
g_re= 0.1379 +/- 0.0171 | g_re= -0.1214 +/- 0.0230 | g_re= 0.0500 +/- 0.0208 |
g_im= 0.0484 +/- 0.0200 | g_im= -0.0723 +/- 0.0272 | g_im= -0.1105 +/- 0.0152 |
corr= [ 0.12] | corr= [-0.07] | corr= [ 0.15] |
=====|=====|=====|

```

```

*****
JP=0+ || eta:eta/1^S_0[+] kaon:kaon/1^S_0[+] pi:pi/1^S_0[-]

```

```

sqrt(s)_pole = (0.10171 +/- 0.017945)
+ (i/2)*(+1.4669e-13 +/- 4.3677e-11) [-0.06]

```

```

=====|=====|=====|
eta:eta/1^S_0 | kaon:kaon/1^S_0 | pi:pi/1^S_0 |
=====|=====|=====|
k_re= 0.0000 +/- 0.0000 | k_re= 0.0000 +/- 0.0000 | k_re= -0.0000 +/- 0.0000 |
k_im= 0.0903 +/- 0.0051 | k_im= 0.0826 +/- 0.0055 | k_im= -0.0467 +/- 0.0098 |
corr= [ 0.06] | corr= [ 0.06] | corr= [ 0.06] |
=====|=====|=====|
|g|= 0.0489 +/- 0.0230 | |g|= 0.0909 +/- 0.0201 | |g|= 0.0087 +/- 0.0092 |
arg(g)/pi= 0.0000 +/- 0.0000 | arg(g)/pi= -0.0000 +/- 0.0000 | arg(g)/pi= -0.0000 +/- 0.0000 |
=====|=====|=====|
g_re= 0.0489 +/- 0.0230 | g_re= 0.0909 +/- 0.0201 | g_re= 0.0087 +/- 0.0092 |
g_im= 0.0000 +/- 0.0000 | g_im= -0.0000 +/- 0.0000 | g_im= -0.0000 +/- 0.0000 |
corr= [-1.00] | corr= [ 0.12] | corr= [-0.80] |
=====|=====|=====|

```

```

*****
JP=0+ || eta:eta/1^S_0[+] kaon:kaon/1^S_0[-] pi:pi/1^S_0[+]

```

```

sqrt(s)_pole = (0.12489 +/- 0.00756)
+ (i/2)*(+2.2947e-13 +/- 6.8655e-11) [-0.01]

```

```

=====|=====|=====|
eta:eta/1^S_0 | kaon:kaon/1^S_0 | pi:pi/1^S_0 |
=====|=====|=====|
k_re= 0.0000 +/- 0.0000 | k_re= -0.0000 +/- 0.0000 | k_re= 0.0000 +/- 0.0000 |
k_im= 0.0827 +/- 0.0029 | k_im= -0.0742 +/- 0.0032 | k_im= 0.0295 +/- 0.0080 |
corr= [ 0.01] | corr= [ 0.01] | corr= [ 0.01] |
=====|=====|=====|
|g|= 0.0767 +/- 0.0101 | |g|= 0.0112 +/- 0.0076 | |g|= 0.0876 +/- 0.0064 |
arg(g)/pi= 0.0000 +/- 0.0000 | arg(g)/pi= 1.0000 +/- 0.0000 | arg(g)/pi= 1.0000 +/- 0.0000 |
=====|=====|=====|
g_re= 0.0767 +/- 0.0101 | g_re= -0.0112 +/- 0.0076 | g_re= -0.0876 +/- 0.0064 |
g_im= 0.0000 +/- 0.0000 | g_im= 0.0000 +/- 0.0000 | g_im= 0.0000 +/- 0.0000 |
corr= [-1.00] | corr= [-0.93] | corr= [-0.98] |
=====|=====|=====|

```

```

*****
JP=0+ || eta:eta/1^S_0[+] kaon:kaon/1^S_0[-] pi:pi/1^S_0[-]

```

```

sqrt(s)_pole = (0.17374 +/- 0.015441)
+ (i/2)*(-0.075908 +/- 0.01949) [ 0.18]

```

```

=====|=====|=====|
eta:eta/1^S_0 | kaon:kaon/1^S_0 | pi:pi/1^S_0 |
=====|=====|=====|
k_re= -0.0254 +/- 0.0068 | k_re= 0.0296 +/- 0.0080 | k_re= 0.0570 +/- 0.0102 |
k_im= 0.0648 +/- 0.0095 | k_im= -0.0556 +/- 0.0101 | k_im= -0.0289 +/- 0.0075 |
corr= [ 0.35] | corr= [ 0.41] | corr= [ 0.37] |
=====|=====|=====|
|g|= 0.1712 +/- 0.0204 | |g|= 0.0585 +/- 0.0070 | |g|= 0.1191 +/- 0.0169 |
arg(g)/pi= -0.0578 +/- 0.0432 | arg(g)/pi= 0.7391 +/- 0.0457 | arg(g)/pi= -0.4992 +/- 0.0315 |
=====|=====|=====|
g_re= 0.1684 +/- 0.0222 | g_re= -0.0399 +/- 0.0066 | g_re= 0.0003 +/- 0.0118 |
g_im= -0.0309 +/- 0.0215 | g_im= 0.0427 +/- 0.0087 | g_im= -0.1191 +/- 0.0169 |
corr= [ 0.44] | corr= [ 0.20] | corr= [-0.57] |
=====|=====|=====|

```

```

*****
JP=0+ || eta:eta/1^S_0[-] kaon:kaon/1^S_0[+] pi:pi/1^S_0[+]

```

```

sqrt(s)_pole = (0.12217 +/- 0.014219)

```

```

+ (i/2)*(+2.1753e-15 +/- 6.4251e-13) [-0.06]

eta:eta/1^S_0 | kaon:kaon/1^S_0 | pi:pi/1^S_0 |
=====|=====|=====|
k_re= -0.0000 +/- 0.0000 | k_re= 0.0000 +/- 0.0000 | k_re= 0.0000 +/- 0.0000 |
k_im= -0.0837 +/- 0.0052 | k_im= 0.0753 +/- 0.0058 | k_im= 0.0322 +/- 0.0135 |
corr= [ 0.06] | corr= [ 0.06] | corr= [ 0.06] |
=====|=====|=====|
|g|= 0.0174 +/- 0.0133 | |g|= 0.1236 +/- 0.0224 | |g|= 0.0580 +/- 0.0394 |
arg(g)/pi= 0.0000 +/- 0.0000 | arg(g)/pi= 1.0000 +/- 0.0000 | arg(g)/pi= 1.0000 +/- 0.0000 |
=====|=====|=====|
g_re= 0.0174 +/- 0.0133 | g_re= -0.1236 +/- 0.0224 | g_re= -0.0580 +/- 0.0394 |
g_im= 0.0000 +/- 0.0000 | g_im= 0.0000 +/- 0.0000 | g_im= 0.0000 +/- 0.0000 |
corr= [-1.00] | corr= [ 0.87] | corr= [-0.95] |
=====|=====|=====|
*****

```

```

*****
JP=0+ || eta:eta/1^S_0[-] kaon:kaon/1^S_0[+] pi:pi/1^S_0[-]

sqrt(s)_pole = (0.13905 +/- 0.022117)
+ (i/2)*(-0.040701 +/- 0.03264) [-0.90]

```

```

eta:eta/1^S_0 | kaon:kaon/1^S_0 | pi:pi/1^S_0 |
=====|=====|=====|
k_re= 0.0091 +/- 0.0094 | k_re= -0.0102 +/- 0.0108 | k_re= 0.0262 +/- 0.0251 |
k_im= -0.0781 +/- 0.0079 | k_im= 0.0691 +/- 0.0086 | k_im= -0.0270 +/- 0.0054 |
corr= [ 0.91] | corr= [ 0.91] | corr= [ 0.15] |
=====|=====|=====|
|g|= 0.0531 +/- 0.0116 | |g|= 0.1503 +/- 0.0412 | |g|= 0.0857 +/- 0.0223 |
arg(g)/pi= -0.2611 +/- 0.0417 | arg(g)/pi= 0.9024 +/- 0.0745 | arg(g)/pi= -0.4649 +/- 0.1368 |
=====|=====|=====|
g_re= 0.0362 +/- 0.0092 | g_re= -0.1433 +/- 0.0490 | g_re= 0.0094 +/- 0.0342 |
g_im= -0.0389 +/- 0.0099 | g_im= 0.0454 +/- 0.0232 | g_im= -0.0851 +/- 0.0262 |
corr= [-0.47] | corr= [ 0.81] | corr= [ 0.99] |
=====|=====|=====|
*****

```

```

*****
JP=0+ || eta:eta/1^S_0[-] kaon:kaon/1^S_0[-] pi:pi/1^S_0[-]

sqrt(s)_pole = (0.13699 +/- 0.001094)
+ (i/2)*(-3.961e-14 +/- 1.1809e-11) [-0.02]

```

```

eta:eta/1^S_0 | kaon:kaon/1^S_0 | pi:pi/1^S_0 |
=====|=====|=====|
k_re= 0.0000 +/- 0.0000 | k_re= 0.0000 +/- 0.0000 | k_re= 0.0000 +/- 0.0000 |
k_im= -0.0778 +/- 0.0005 | k_im= -0.0687 +/- 0.0005 | k_im= -0.0088 +/- 0.0043 |
corr= [ 0.02] | corr= [ 0.02] | corr= [ 0.02] |
=====|=====|=====|
|g|= 0.0188 +/- 0.0045 | |g|= 0.0098 +/- 0.0064 | |g|= 0.0677 +/- 0.0150 |
arg(g)/pi= 0.5000 +/- 0.0000 | arg(g)/pi= -0.5000 +/- 0.0000 | arg(g)/pi= 0.5000 +/- 0.0000 |
=====|=====|=====|
g_re= 0.0000 +/- 0.0000 | g_re= 0.0000 +/- 0.0000 | g_re= -0.0000 +/- 0.0000 |
g_im= 0.0188 +/- 0.0045 | g_im= -0.0098 +/- 0.0064 | g_im= 0.0677 +/- 0.0150 |
corr= [-1.00] | corr= [-0.72] | corr= [ 0.58] |
=====|=====|=====|
*****

```



# k\_lcclcc

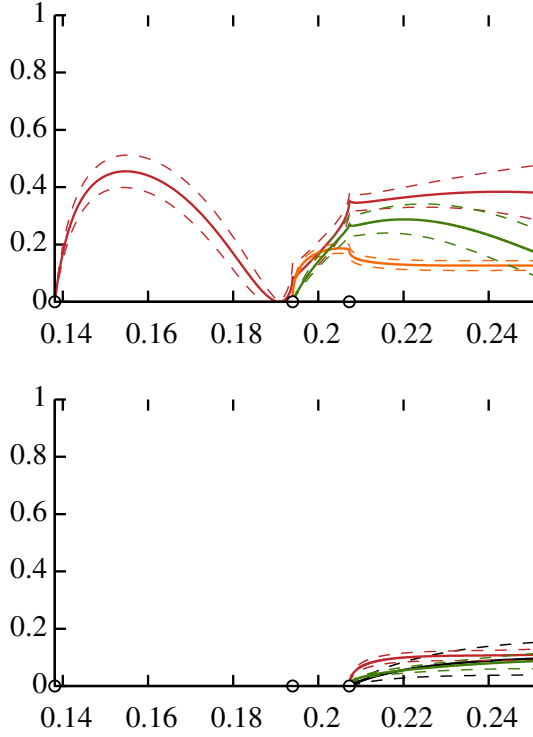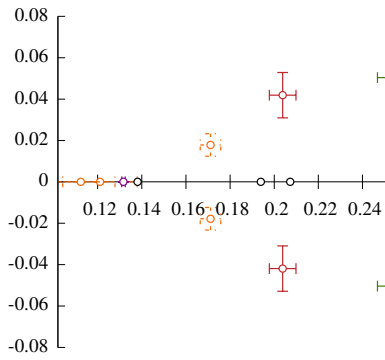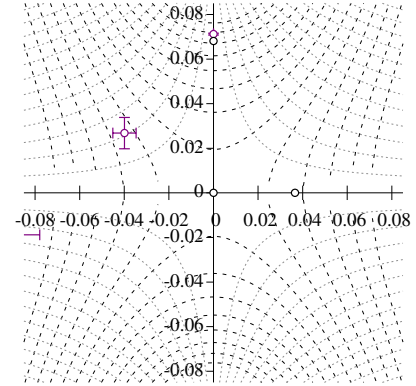

## parameter values

minimised with  $\chi^2/\text{nDoF} = 48.90 / (57 - 8) = 1.00$

|                                                   |                      |       |       |       |       |       |       |       |      |
|---------------------------------------------------|----------------------|-------|-------|-------|-------|-------|-------|-------|------|
| JPO+_gamma_eta:eta/1^S_0 eta:eta/1^S_0_order0     | 2.4833 +/- 0.70886   | 1.00  | 0.67  | -0.61 | 0.22  | -0.23 | -0.10 | 0.07  | 0.02 |
| JPO+_gamma_eta:eta/1^S_0 kaon:kaon/1^S_0_order0   | 2.6146 +/- 0.37004   | 1.00  | -0.59 | 0.83  | 0.07  | -0.66 | 0.31  | -0.02 |      |
| JPO+_gamma_eta:eta/1^S_0 pi:pi/1^S_0_order0       | -3.2149 +/- 0.45591  | 1.00  | -0.37 | 0.32  | 0.47  | -0.44 | -0.35 |       |      |
| JPO+_gamma_kaon:kaon/1^S_0 kaon:kaon/1^S_0_order0 | -0.79204 +/- 0.32572 | 1.00  | 0.01  | -0.80 | 0.39  | -0.04 |       |       |      |
| JPO+_gamma_kaon:kaon/1^S_0 kaon:kaon/1^S_0_order1 | 1.6846 +/- 0.30194   | 1.00  | -0.34 | 0.19  | -0.33 |       |       |       |      |
| JPO+_gamma_kaon:kaon/1^S_0 pi:pi/1^S_0_order0     | -3.0891 +/- 0.35715  | 1.00  | -0.73 | 0.11  |       |       |       |       |      |
| JPO+_gamma_pi:pi/1^S_0 pi:pi/1^S_0_order0         | 2.0352 +/- 0.52595   | 1.00  | -0.49 |       |       |       |       |       |      |
| JPO+_gamma_pi:pi/1^S_0 pi:pi/1^S_0_order1         | 0.24406 +/- 0.39933  | 1.00  |       |       |       |       |       |       |      |
| JPO+_gamma_eta:eta/1^S_0 eta:eta/1^S_0_order1     | 0.0000 +/- 0         | FIXED |       |       |       |       |       |       |      |
| JPO+_gamma_eta:eta/1^S_0 kaon:kaon/1^S_0_order1   | 0.0000 +/- 0         | FIXED |       |       |       |       |       |       |      |
| JPO+_gamma_eta:eta/1^S_0 pi:pi/1^S_0_order1       | 0.0000 +/- 0         | FIXED |       |       |       |       |       |       |      |
| JPO+_gamma_kaon:kaon/1^S_0 pi:pi/1^S_0_order1     | 0.0000 +/- 0         | FIXED |       |       |       |       |       |       |      |

## pole singularities

\*\*\*\*\*  
JP=0+ || eta:eta/1^S\_0[+] kaon:kaon/1^S\_0[+] pi:pi/1^S\_0[+]

$\sqrt{s}_{\text{pole}} = (0.13171 \pm 0.00078231) + (i/2) * (2.9462e-13 \pm 7.8504e-11) [-0.08]$

| eta:eta/1^S_0                | kaon:kaon/1^S_0              | pi:pi/1^S_0                  |
|------------------------------|------------------------------|------------------------------|
| k_re= 0.0000 +/- 0.0000      | k_re= 0.0000 +/- 0.0000      | k_re= 0.0000 +/- 0.0000      |
| k_im= 0.0800 +/- 0.0003      | k_im= 0.0712 +/- 0.0004      | k_im= 0.0208 +/- 0.0012      |
| corr= [ 0.08]                | corr= [ 0.08]                | corr= [ 0.08]                |
| g = 0.0519 +/- 0.0096        | g = 0.1458 +/- 0.0112        | g = 0.0922 +/- 0.0043        |
| arg(g)/pi= 0.0000 +/- 0.0000 | arg(g)/pi= 1.0000 +/- 0.0000 | arg(g)/pi= 1.0000 +/- 0.0000 |
| g_re= 0.0519 +/- 0.0096      | g_re= -0.1458 +/- 0.0112     | g_re= -0.0922 +/- 0.0043     |
| g_im= 0.0000 +/- 0.0000      | g_im= 0.0000 +/- 0.0000      | g_im= 0.0000 +/- 0.0000      |
| corr= [-1.00]                | corr= [ 0.11]                | corr= [-0.67]                |

\*\*\*\*\*

\*\*\*\*\*  
JP=0+ || eta:eta/1^S\_0[+] kaon:kaon/1^S\_0[+] pi:pi/1^S\_0[-]

```

sqrt(s)_pole = (0.20383 +/- 0.0060096)
+ (i/2)*(-0.041908 +/- 0.010943) [ 0.41]

=====
eta:eta/1^S_0 | kaon:kaon/1^S_0 | pi:pi/1^S_0 |
=====
k_re= -0.0293 +/- 0.0048 | k_re= -0.0399 +/- 0.0052 | k_re= 0.0755 +/- 0.0039 |
k_im= 0.0364 +/- 0.0075 | k_im= 0.0268 +/- 0.0070 | k_im= -0.0141 +/- 0.0038 |
corr= [ 0.10] | corr= [ 0.32] | corr= [ 0.42] |
=====
|g|= 0.1713 +/- 0.0202 | |g|= 0.1761 +/- 0.0264 | |g|= 0.1435 +/- 0.0248 |
arg(g)/pi= 0.0326 +/- 0.0765 | arg(g)/pi= 0.2286 +/- 0.0639 | arg(g)/pi= 0.6096 +/- 0.0800 |
=====
g_re= 0.1704 +/- 0.0209 | g_re= 0.1326 +/- 0.0296 | g_re= -0.0484 +/- 0.0352 |
g_im= 0.0175 +/- 0.0408 | g_im= 0.1159 +/- 0.0327 | g_im= 0.1351 +/- 0.0259 |
corr= [-0.25] | corr= [-0.28] | corr= [ 0.21] |
=====
*****

*****
JP=0+ || eta:eta/1^S_0[+] kaon:kaon/1^S_0[-] pi:pi/1^S_0[+]

sqrt(s)_pole = (0.25909 +/- 0.012313)
+ (i/2)*(-0.050389 +/- 0.017542) [-0.16]

=====
eta:eta/1^S_0 | kaon:kaon/1^S_0 | pi:pi/1^S_0 |
=====
k_re= -0.0794 +/- 0.0099 | k_re= 0.0870 +/- 0.0091 | k_re= -0.1099 +/- 0.0073 |
k_im= 0.0206 +/- 0.0068 | k_im= -0.0188 +/- 0.0063 | k_im= 0.0149 +/- 0.0051 |
corr= [-0.05] | corr= [-0.08] | corr= [-0.13] |
=====
|g|= 0.0867 +/- 0.0197 | |g|= 0.1642 +/- 0.0078 | |g|= 0.0868 +/- 0.0172 |
arg(g)/pi= -0.4707 +/- 0.0837 | arg(g)/pi= -0.5824 +/- 0.0199 | arg(g)/pi= 0.9504 +/- 0.0619 |
=====
g_re= 0.0080 +/- 0.0214 | g_re= -0.0420 +/- 0.0114 | g_re= -0.0858 +/- 0.0189 |
g_im= -0.0863 +/- 0.0211 | g_im= -0.1587 +/- 0.0059 | g_im= 0.0135 +/- 0.0149 |
corr= [ 0.72] | corr= [ 0.58] | corr= [ 0.69] |
=====
*****

*****
JP=0+ || eta:eta/1^S_0[-] kaon:kaon/1^S_0[+] pi:pi/1^S_0[+]

sqrt(s)_pole = (0.11238 +/- 0.015472)
+ (i/2)*(+2.7737e-13 +/- 3.5275e-11) [-0.05]

=====
eta:eta/1^S_0 | kaon:kaon/1^S_0 | pi:pi/1^S_0 |
=====
k_re= -0.0000 +/- 0.0000 | k_re= 0.0000 +/- 0.0000 | k_re= 0.0000 +/- 0.0000 |
k_im= -0.0871 +/- 0.0050 | k_im= 0.0790 +/- 0.0055 | k_im= 0.0401 +/- 0.0108 |
corr= [ 0.05] | corr= [ 0.05] | corr= [ 0.05] |
=====
|g|= 0.0277 +/- 0.0165 | |g|= 0.0828 +/- 0.0261 | |g|= 0.1919 +/- 0.0636 |
arg(g)/pi= 0.0000 +/- 0.0000 | arg(g)/pi= 1.0000 +/- 0.0000 | arg(g)/pi= 1.0000 +/- 0.0000 |
=====
g_re= 0.0277 +/- 0.0165 | g_re= -0.0828 +/- 0.0261 | g_re= -0.1919 +/- 0.0636 |
g_im= 0.0000 +/- 0.0000 | g_im= 0.0000 +/- 0.0000 | g_im= 0.0000 +/- 0.0000 |
corr= [-1.00] | corr= [-0.87] | corr= [ 0.96] |
=====
*****

*****
JP=0+ || eta:eta/1^S_0[-] kaon:kaon/1^S_0[+] pi:pi/1^S_0[-]

sqrt(s)_pole = (0.17114 +/- 0.0046381)
+ (i/2)*(-0.017839 +/- 0.0054471) [-0.59]

=====
eta:eta/1^S_0 | kaon:kaon/1^S_0 | pi:pi/1^S_0 |
=====
k_re= 0.0065 +/- 0.0023 | k_re= -0.0082 +/- 0.0031 | k_re= 0.0509 +/- 0.0040 |
k_im= -0.0590 +/- 0.0031 | k_im= 0.0466 +/- 0.0038 | k_im= -0.0075 +/- 0.0021 |
corr= [ 0.67] | corr= [ 0.69] | corr= [-0.51] |
=====
|g|= 0.0535 +/- 0.0095 | |g|= 0.2089 +/- 0.0105 | |g|= 0.0631 +/- 0.0086 |
arg(g)/pi= -0.1838 +/- 0.0276 | arg(g)/pi= -0.0012 +/- 0.0139 | arg(g)/pi= 0.5119 +/- 0.0214 |
=====
g_re= 0.0448 +/- 0.0096 | g_re= 0.2089 +/- 0.0105 | g_re= -0.0024 +/- 0.0040 |
g_im= -0.0292 +/- 0.0045 | g_im= -0.0008 +/- 0.0092 | g_im= 0.0630 +/- 0.0087 |
corr= [-0.51] | corr= [-0.72] | corr= [ 0.78] |
=====
*****

*****
JP=0+ || eta:eta/1^S_0[-] kaon:kaon/1^S_0[-] pi:pi/1^S_0[+]

sqrt(s)_pole = (0.12107 +/- 0.016873)
+ (i/2)*(+1.769e-14 +/- 5.0552e-12) [-0.02]

=====
eta:eta/1^S_0 | kaon:kaon/1^S_0 | pi:pi/1^S_0 |
=====
k_re= -0.0000 +/- 0.0000 | k_re= -0.0000 +/- 0.0000 | k_re= 0.0000 +/- 0.0000 |
k_im= -0.0841 +/- 0.0061 | k_im= -0.0758 +/- 0.0067 | k_im= 0.0332 +/- 0.0153 |
corr= [ 0.01] | corr= [ 0.01] | corr= [ 0.01] |
=====
|g|= 0.0392 +/- 0.0175 | |g|= 0.0093 +/- 0.0037 | |g|= 0.1879 +/- 0.0796 |
arg(g)/pi= 0.0000 +/- 0.0000 | arg(g)/pi= -0.0000 +/- 0.0000 | arg(g)/pi= 1.0000 +/- 0.0000 |
=====
g_re= 0.0392 +/- 0.0175 | g_re= 0.0093 +/- 0.0037 | g_re= -0.1879 +/- 0.0796 |
g_im= 0.0000 +/- 0.0000 | g_im= -0.0000 +/- 0.0000 | g_im= 0.0000 +/- 0.0000 |
corr= [-1.00] | corr= [-0.80] | corr= [ 0.93] |
=====
*****

```

# k\_lcclcl

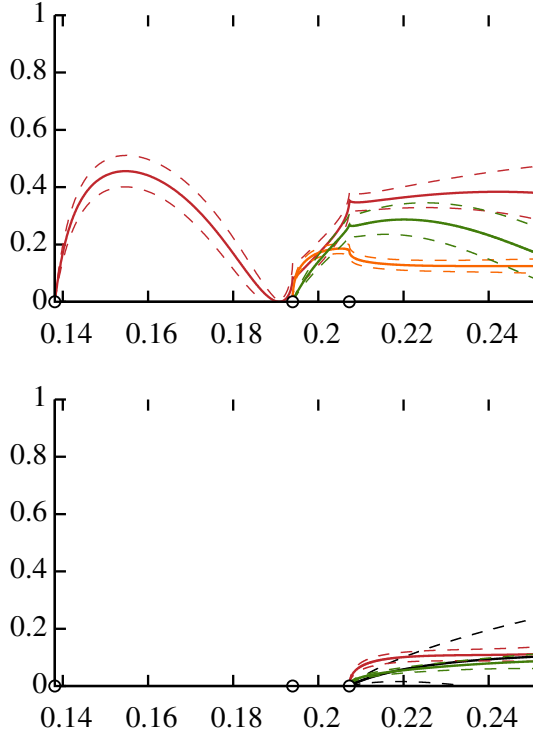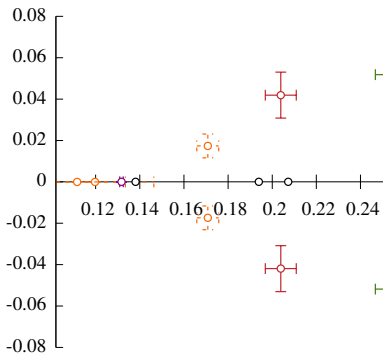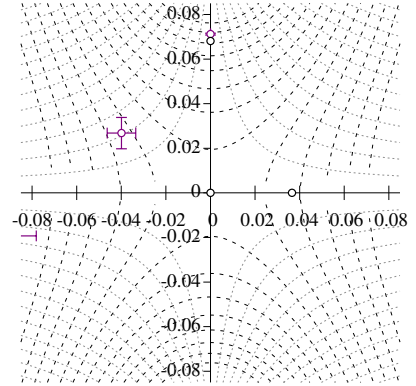

## parameter values

minimised with chisq/nDoF = 48.90 / (57 - 9) = 1.02

|                                                    |                       |       |       |       |       |       |       |      |       |      |
|----------------------------------------------------|-----------------------|-------|-------|-------|-------|-------|-------|------|-------|------|
| JPO+ _gamma_eta:eta/1^S_0 eta:eta/1^S_0_order0     | 2.6064 +/- 1.1457     | 1.00  | -0.78 | 0.49  | -0.42 | -0.22 | 0.21  | 0.06 | -0.15 | 0.18 |
| JPO+ _gamma_eta:eta/1^S_0 eta:eta/1^S_0_order1     | -0.047216 +/- 0.87011 | 1.00  | -0.11 | 0.07  | 0.41  | -0.43 | -0.13 | 0.23 | -0.22 |      |
| JPO+ _gamma_eta:eta/1^S_0 kaon:kaon/1^S_0_order0   | 2.6536 +/- 0.35688    | 1.00  | -0.57 | 0.68  | 0.10  | -0.61 | 0.24  | 0.00 |       |      |
| JPO+ _gamma_eta:eta/1^S_0 pi:pi/1^S_0_order0       | -3.2723 +/- 0.44931   | 1.00  | -0.27 | 0.28  | 0.43  | -0.40 | -0.36 |      |       |      |
| JPO+ _gamma_kaon:kaon/1^S_0 kaon:kaon/1^S_0_order0 | -0.78010 +/- 0.34229  | 1.00  | -0.18 | -0.76 | 0.41  | -0.12 |       |      |       |      |
| JPO+ _gamma_kaon:kaon/1^S_0 kaon:kaon/1^S_0_order1 | 1.6796 +/- 0.33522    | 1.00  | -0.25 | 0.06  | -0.20 |       |       |      |       |      |
| JPO+ _gamma_kaon:kaon/1^S_0 pi:pi/1^S_0_order0     | -3.1063 +/- 0.34548   | 1.00  | -0.25 | -0.73 | 0.12  |       |       |      |       |      |
| JPO+ _gamma_pi:pi/1^S_0 pi:pi/1^S_0_order0         | 2.0517 +/- 0.52859    | 1.00  | -0.51 |       |       |       |       |      |       |      |
| JPO+ _gamma_pi:pi/1^S_0 pi:pi/1^S_0_order1         | 0.26165 +/- 0.40833   | 1.00  |       |       |       |       |       |      |       |      |
| JPO+ _gamma_eta:eta/1^S_0 kaon:kaon/1^S_0_order0   | 0.0000 +/- 0          | FIXED |       |       |       |       |       |      |       |      |
| JPO+ _gamma_eta:eta/1^S_0 pi:pi/1^S_0_order1       | 0.0000 +/- 0          | FIXED |       |       |       |       |       |      |       |      |
| JPO+ _gamma_kaon:kaon/1^S_0 pi:pi/1^S_0_order1     | 0.0000 +/- 0          | FIXED |       |       |       |       |       |      |       |      |

## pole singularities

JP=0+ || eta:eta/1^S\_0[+] kaon:kaon/1^S\_0[+] pi:pi/1^S\_0[+]

sqrt(s)\_pole = (0.13172 +/- 0.00079127)  
+ (i/2)\*(+1.9671e-13 +/- 6.8917e-12) [ 0.36]

| eta:eta/1^S_0                | kaon:kaon/1^S_0              | pi:pi/1^S_0                  |
|------------------------------|------------------------------|------------------------------|
| k_re= 0.0000 +/- 0.0000      | k_re= 0.0000 +/- 0.0000      | k_re= 0.0000 +/- 0.0000      |
| k_im= 0.0800 +/- 0.0003      | k_im= 0.0712 +/- 0.0004      | k_im= 0.0208 +/- 0.0013      |
| corr= [-0.36]                | corr= [-0.36]                | corr= [-0.36]                |
| g = 0.0514 +/- 0.0130        | g = 0.1459 +/- 0.0124        | g = 0.0923 +/- 0.0049        |
| arg(g)/pi= 0.0000 +/- 0.0000 | arg(g)/pi= 1.0000 +/- 0.0000 | arg(g)/pi= 1.0000 +/- 0.0000 |
| g_re= 0.0514 +/- 0.0130      | g_re= -0.1459 +/- 0.0124     | g_re= -0.0923 +/- 0.0049     |
| g_im= 0.0000 +/- 0.0000      | g_im= 0.0000 +/- 0.0000      | g_im= 0.0000 +/- 0.0000      |
| corr= [-1.00]                | corr= [ 0.40]                | corr= [-0.72]                |

JP=0+ || eta:eta/1^S\_0[+] kaon:kaon/1^S\_0[+] pi:pi/1^S\_0[-]

```

sqrt(s)_pole = (0.20391 +/- 0.0070146)
+ (i/2)*(-0.041925 +/- 0.011097) [ 0.27]

=====
eta:eta/1^S_0 | kaon:kaon/1^S_0 | pi:pi/1^S_0 |
=====
k_re= -0.0294 +/- 0.0060 | k_re= -0.0399 +/- 0.0064 | k_re= 0.0756 +/- 0.0046 |
k_im= 0.0363 +/- 0.0078 | k_im= 0.0268 +/- 0.0070 | k_im= -0.0141 +/- 0.0038 |
corr= [ 0.24] | corr= [ 0.34] | corr= [ 0.30] |
=====
|g|= 0.1730 +/- 0.0339 | |g|= 0.1751 +/- 0.0314 | |g|= 0.1436 +/- 0.0298 |
arg(g)/pi= 0.0332 +/- 0.0869 | arg(g)/pi= 0.2301 +/- 0.0751 | arg(g)/pi= 0.6107 +/- 0.0901 |
=====
g_re= 0.1720 +/- 0.0326 | g_re= 0.1313 +/- 0.0370 | g_re= -0.0490 +/- 0.0413 |
g_im= 0.0180 +/- 0.0481 | g_im= 0.1158 +/- 0.0363 | g_im= 0.1350 +/- 0.0290 |
corr= [ 0.22] | corr= [-0.27] | corr= [ 0.07] |
=====
*****

*****
JP=0+ || eta:eta/1^S_0[+] kaon:kaon/1^S_0[-] pi:pi/1^S_0[+]

sqrt(s)_pole = (0.25913 +/- 0.012387)
+ (i/2)*(-0.051824 +/- 0.020665) [ 0.07]

=====
eta:eta/1^S_0 | kaon:kaon/1^S_0 | pi:pi/1^S_0 |
=====
k_re= -0.0795 +/- 0.0097 | k_re= 0.0871 +/- 0.0090 | k_re= -0.1099 +/- 0.0072 |
k_im= 0.0211 +/- 0.0083 | k_im= -0.0193 +/- 0.0076 | k_im= 0.0153 +/- 0.0061 |
corr= [ 0.12] | corr= [ 0.11] | corr= [ 0.08] |
=====
|g|= 0.0868 +/- 0.0234 | |g|= 0.1639 +/- 0.0085 | |g|= 0.0848 +/- 0.0301 |
arg(g)/pi= -0.4629 +/- 0.1478 | arg(g)/pi= -0.5829 +/- 0.0185 | arg(g)/pi= 0.9484 +/- 0.0670 |
=====
g_re= 0.0101 +/- 0.0406 | g_re= -0.0422 +/- 0.0105 | g_re= -0.0837 +/- 0.0317 |
g_im= -0.0863 +/- 0.0229 | g_im= -0.1583 +/- 0.0073 | g_im= 0.0137 +/- 0.0147 |
corr= [-0.03] | corr= [ 0.40] | corr= [ 0.55] |
=====
*****

*****
JP=0+ || eta:eta/1^S_0[-] kaon:kaon/1^S_0[+] pi:pi/1^S_0[+]

sqrt(s)_pole = (0.11161 +/- 0.021887)
+ (i/2)*(-5.2411e-12 +/- 1.538e-09) [-0.06]

=====
eta:eta/1^S_0 | kaon:kaon/1^S_0 | pi:pi/1^S_0 |
=====
k_re= 0.0000 +/- 0.0000 | k_re= -0.0000 +/- 0.0000 | k_re= -0.0000 +/- 0.0000 |
k_im= -0.0873 +/- 0.0070 | k_im= 0.0793 +/- 0.0077 | k_im= 0.0407 +/- 0.0149 |
corr= [ 0.06] | corr= [ 0.06] | corr= [ 0.06] |
=====
|g|= 0.0289 +/- 0.0281 | |g|= 0.0798 +/- 0.0466 | |g|= 0.1964 +/- 0.1068 |
arg(g)/pi= 0.0000 +/- 0.0000 | arg(g)/pi= 1.0000 +/- 0.0000 | arg(g)/pi= 1.0000 +/- 0.0000 |
=====
g_re= 0.0289 +/- 0.0281 | g_re= -0.0798 +/- 0.0466 | g_re= -0.1964 +/- 0.1068 |
g_im= 0.0000 +/- 0.0000 | g_im= 0.0000 +/- 0.0000 | g_im= 0.0000 +/- 0.0000 |
corr= [-1.00] | corr= [-0.95] | corr= [ 0.97] |
=====
*****

*****
JP=0+ || eta:eta/1^S_0[-] kaon:kaon/1^S_0[+] pi:pi/1^S_0[-]

sqrt(s)_pole = (0.17081 +/- 0.0049893)
+ (i/2)*(-0.017359 +/- 0.0057429) [-0.67]

=====
eta:eta/1^S_0 | kaon:kaon/1^S_0 | pi:pi/1^S_0 |
=====
k_re= 0.0063 +/- 0.0024 | k_re= -0.0079 +/- 0.0033 | k_re= 0.0506 +/- 0.0043 |
k_im= -0.0592 +/- 0.0033 | k_im= 0.0468 +/- 0.0040 | k_im= -0.0073 +/- 0.0022 |
corr= [ 0.74] | corr= [ 0.75] | corr= [-0.59] |
=====
|g|= 0.0537 +/- 0.0105 | |g|= 0.2099 +/- 0.0126 | |g|= 0.0623 +/- 0.0092 |
arg(g)/pi= -0.1813 +/- 0.0295 | arg(g)/pi= -0.0025 +/- 0.0187 | arg(g)/pi= 0.5135 +/- 0.0231 |
=====
g_re= 0.0452 +/- 0.0105 | g_re= 0.2099 +/- 0.0126 | g_re= -0.0026 +/- 0.0043 |
g_im= -0.0289 +/- 0.0049 | g_im= -0.0016 +/- 0.0124 | g_im= 0.0623 +/- 0.0093 |
corr= [-0.53] | corr= [-0.84] | corr= [ 0.63] |
=====
*****

*****
JP=0+ || eta:eta/1^S_0[-] kaon:kaon/1^S_0[-] pi:pi/1^S_0[+]

sqrt(s)_pole = (0.11975 +/- 0.026638)
+ (i/2)*(-1.2414e-14 +/- 6.1932e-12) [ 0.01]

=====
eta:eta/1^S_0 | kaon:kaon/1^S_0 | pi:pi/1^S_0 |
=====
k_re= 0.0000 +/- 0.0000 | k_re= 0.0000 +/- 0.0000 | k_re= -0.0000 +/- 0.0000 |
k_im= -0.0846 +/- 0.0094 | k_im= -0.0763 +/- 0.0104 | k_im= 0.0344 +/- 0.0230 |
corr= [-0.01] | corr= [-0.01] | corr= [-0.01] |
=====
|g|= 0.0403 +/- 0.0289 | |g|= 0.0088 +/- 0.0060 | |g|= 0.1944 +/- 0.1368 |
arg(g)/pi= 0.0000 +/- 0.0000 | arg(g)/pi= -0.0000 +/- 0.0000 | arg(g)/pi= 1.0000 +/- 0.0000 |
=====
g_re= 0.0403 +/- 0.0289 | g_re= 0.0088 +/- 0.0060 | g_re= -0.1944 +/- 0.1368 |
g_im= 0.0000 +/- 0.0000 | g_im= -0.0000 +/- 0.0000 | g_im= 0.0000 +/- 0.0000 |
corr= [-1.00] | corr= [-0.92] | corr= [ 0.96] |
=====
*****

```

# k\_qcclcc

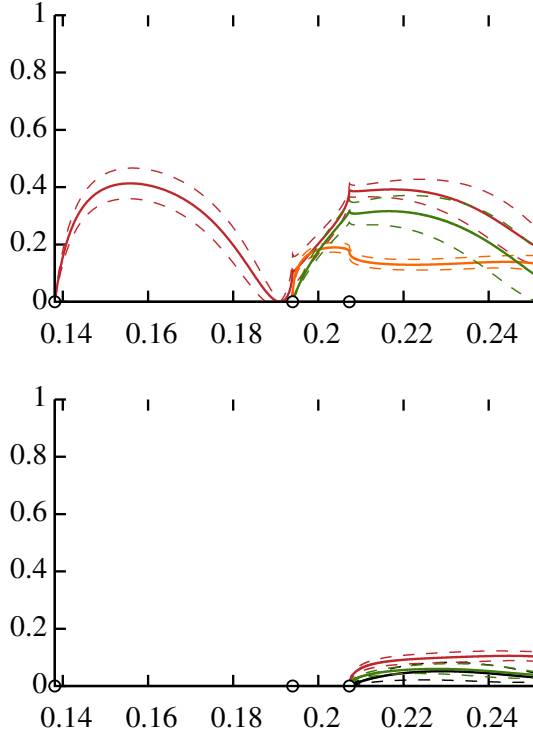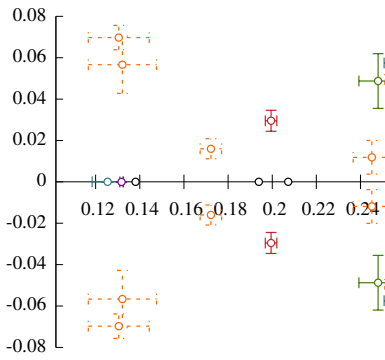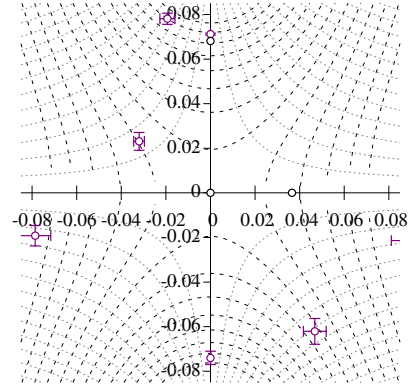

## parameter values

minimised with  $\chi^2/\text{nDoF} = 47.45 / (57 - 9) = 0.99$

|                                                                                                                      |                      |       |       |       |       |       |       |       |       |      |
|----------------------------------------------------------------------------------------------------------------------|----------------------|-------|-------|-------|-------|-------|-------|-------|-------|------|
| JPO+ $\gamma_{\eta} : \eta \rightarrow 1^1 S_0   \eta \rightarrow 1^1 S_0$ order0                                    | 2.7706 +/- 0.60523   | 1.00  | 0.52  | -0.59 | 0.01  | -0.31 | 0.09  | -0.00 | 0.03  | 0.02 |
| JPO+ $\gamma_{\eta} : \eta \rightarrow 1^1 S_0   \text{kaon} : \text{kaon} \rightarrow 1^1 S_0$ order0               | 2.8630 +/- 0.31619   | 1.00  | -0.39 | 0.80  | 0.16  | -0.62 | 0.18  | 0.07  | -0.12 |      |
| JPO+ $\gamma_{\eta} : \eta \rightarrow 1^1 S_0   \pi : \pi \rightarrow 1^1 S_0$ order0                               | -3.5560 +/- 0.43676  | 1.00  | -0.11 | 0.37  | 0.28  | -0.36 | -0.19 | -0.08 |       |      |
| JPO+ $\gamma_{\text{kaon}} : \text{kaon} \rightarrow 1^1 S_0   \text{kaon} : \text{kaon} \rightarrow 1^1 S_0$ order0 | -0.62261 +/- 0.32071 | 1.00  | 0.12  | -0.77 | 0.25  | 0.07  | -0.17 |       |       |      |
| JPO+ $\gamma_{\text{kaon}} : \text{kaon} \rightarrow 1^1 S_0   \text{kaon} : \text{kaon} \rightarrow 1^1 S_0$ order1 | 1.7956 +/- 0.33073   | 1.00  | -0.43 | 0.13  | -0.06 | -0.15 |       |       |       |      |
| JPO+ $\gamma_{\text{kaon}} : \text{kaon} \rightarrow 1^1 S_0   \pi : \pi \rightarrow 1^1 S_0$ order0                 | -3.5452 +/- 0.3603   | 1.00  | -0.60 | -0.08 | 0.21  |       |       |       |       |      |
| JPO+ $\gamma_{\pi} : \pi \rightarrow 1^1 S_0   \pi : \pi \rightarrow 1^1 S_0$ order0                                 | 5.4068 +/- 0.56911   | 1.00  | -0.51 | 0.24  |       |       |       |       |       |      |
| JPO+ $\gamma_{\pi} : \pi \rightarrow 1^1 S_0   \pi : \pi \rightarrow 1^1 S_0$ order1                                 | -5.3248 +/- 0.71239  | 1.00  | -0.78 |       |       |       |       |       |       |      |
| JPO+ $\gamma_{\pi} : \pi \rightarrow 1^1 S_0   \pi : \pi \rightarrow 1^1 S_0$ order2                                 | 2.5887 +/- 0.40471   | 1.00  |       |       |       |       |       |       |       |      |
| JPO+ $\gamma_{\eta} : \eta \rightarrow 1^1 S_0   \eta \rightarrow 1^1 S_0$ order1                                    | 0.0000 +/- 0         | FIXED |       |       |       |       |       |       |       |      |
| JPO+ $\gamma_{\eta} : \eta \rightarrow 1^1 S_0   \eta \rightarrow 1^1 S_0$ order2                                    | 0.0000 +/- 0         | FIXED |       |       |       |       |       |       |       |      |
| JPO+ $\gamma_{\eta} : \eta \rightarrow 1^1 S_0   \text{kaon} : \text{kaon} \rightarrow 1^1 S_0$ order1               | 0.0000 +/- 0         | FIXED |       |       |       |       |       |       |       |      |
| JPO+ $\gamma_{\eta} : \eta \rightarrow 1^1 S_0   \text{kaon} : \text{kaon} \rightarrow 1^1 S_0$ order2               | 0.0000 +/- 0         | FIXED |       |       |       |       |       |       |       |      |
| JPO+ $\gamma_{\eta} : \eta \rightarrow 1^1 S_0   \pi : \pi \rightarrow 1^1 S_0$ order1                               | 0.0000 +/- 0         | FIXED |       |       |       |       |       |       |       |      |
| JPO+ $\gamma_{\eta} : \eta \rightarrow 1^1 S_0   \pi : \pi \rightarrow 1^1 S_0$ order2                               | 0.0000 +/- 0         | FIXED |       |       |       |       |       |       |       |      |
| JPO+ $\gamma_{\text{kaon}} : \text{kaon} \rightarrow 1^1 S_0   \text{kaon} : \text{kaon} \rightarrow 1^1 S_0$ order1 | 0.0000 +/- 0         | FIXED |       |       |       |       |       |       |       |      |
| JPO+ $\gamma_{\text{kaon}} : \text{kaon} \rightarrow 1^1 S_0   \pi : \pi \rightarrow 1^1 S_0$ order1                 | 0.0000 +/- 0         | FIXED |       |       |       |       |       |       |       |      |
| JPO+ $\gamma_{\text{kaon}} : \text{kaon} \rightarrow 1^1 S_0   \pi : \pi \rightarrow 1^1 S_0$ order2                 | 0.0000 +/- 0         | FIXED |       |       |       |       |       |       |       |      |

## pole singularities

\*\*\*\*\*  
JP=0+ ||  $\eta \rightarrow 1^1 S_0$  |  $\text{kaon} : \text{kaon} \rightarrow 1^1 S_0$  |  $\pi : \pi \rightarrow 1^1 S_0$  |

$\sqrt{s}_{\text{pole}} = (0.13174 \pm 0.00078917) + (i/2) \times (-1.9272e-13 \pm 1.2397e-11) [-1.00]$

| $\eta \rightarrow 1^1 S_0$           | $\text{kaon} : \text{kaon} \rightarrow 1^1 S_0$ | $\pi : \pi \rightarrow 1^1 S_0$      |
|--------------------------------------|-------------------------------------------------|--------------------------------------|
| $k_{\text{re}} = -0.0000 \pm 0.0000$ | $k_{\text{re}} = -0.0000 \pm 0.0000$            | $k_{\text{re}} = -0.0000 \pm 0.0000$ |
| $k_{\text{im}} = 0.0800 \pm 0.0003$  | $k_{\text{im}} = 0.0712 \pm 0.0004$             | $k_{\text{im}} = 0.0208 \pm 0.0013$  |
| $\text{corr} = [1.00]$               | $\text{corr} = [1.00]$                          | $\text{corr} = [1.00]$               |
| $ g  = 0.0588 \pm 0.0088$            | $ g  = 0.1539 \pm 0.0111$                       | $ g  = 0.0894 \pm 0.0043$            |
| $\arg(g)/\pi = 0.0000 \pm 0.0000$    | $\arg(g)/\pi = 1.0000 \pm 0.0000$               | $\arg(g)/\pi = 1.0000 \pm 0.0000$    |
| $g_{\text{re}} = 0.0588 \pm 0.0088$  | $g_{\text{re}} = -0.1539 \pm 0.0111$            | $g_{\text{re}} = -0.0894 \pm 0.0043$ |
| $g_{\text{im}} = 0.0000 \pm 0.0000$  | $g_{\text{im}} = 0.0000 \pm 0.0000$             | $g_{\text{im}} = 0.0000 \pm 0.0000$  |
| $\text{corr} = [-1.00]$              | $\text{corr} = [-0.11]$                         | $\text{corr} = [-0.58]$              |

```
*****

JP=0+ || eta:eta/1^S_0[+] kaon:kaon/1^S_0[+] pi:pi/1^S_0[-]

sqrt(s)_pole = (0.12983 +/- 0.007648)
               + (i/2)*(-0.092943 +/- 0.012442) [-0.44]

=====
eta:eta/1^S_0 | kaon:kaon/1^S_0 | pi:pi/1^S_0 |
=====
k_re= -0.0176 +/- 0.0031 | k_re= -0.0193 +/- 0.0034 | k_re= 0.0325 +/- 0.0051 |
k_im= 0.0859 +/- 0.0023 | k_im= 0.0781 +/- 0.0025 | k_im= -0.0464 +/- 0.0031 |
corr= [ 0.40] | corr= [ 0.37] | corr= [ 0.06] |
=====
|g|= 0.1331 +/- 0.0161 | |g|= 0.1647 +/- 0.0113 | |g|= 0.0589 +/- 0.0057 |
arg(g)/pi= 0.2194 +/- 0.0206 | arg(g)/pi= 0.9379 +/- 0.0329 | arg(g)/pi= -0.8554 +/- 0.0306 |
=====
g_re= 0.1027 +/- 0.0120 | g_re= -0.1616 +/- 0.0105 | g_re= -0.0529 +/- 0.0057 |
g_im= 0.0847 +/- 0.0138 | g_im= 0.0319 +/- 0.0176 | g_im= -0.0258 +/- 0.0057 |
corr= [ 0.60] | corr= [-0.15] | corr= [ 0.01] |
=====
*****
```

```
*****

JP=0+ || eta:eta/1^S_0[+] kaon:kaon/1^S_0[+] pi:pi/1^S_0[-]

sqrt(s)_pole = (0.19949 +/- 0.0026266)
               + (i/2)*(-0.029535 +/- 0.0050716) [ 0.56]

=====
eta:eta/1^S_0 | kaon:kaon/1^S_0 | pi:pi/1^S_0 |
=====
k_re= -0.0206 +/- 0.0021 | k_re= -0.0320 +/- 0.0024 | k_re= 0.0723 +/- 0.0017 |
k_im= 0.0357 +/- 0.0039 | k_im= 0.0231 +/- 0.0040 | k_im= -0.0102 +/- 0.0018 |
corr= [-0.20] | corr= [ 0.32] | corr= [ 0.56] |
=====
|g|= 0.1242 +/- 0.0105 | |g|= 0.1473 +/- 0.0140 | |g|= 0.1014 +/- 0.0065 |
arg(g)/pi= 0.0352 +/- 0.0334 | arg(g)/pi= 0.2198 +/- 0.0270 | arg(g)/pi= 0.5987 +/- 0.0324 |
=====
g_re= 0.1234 +/- 0.0099 | g_re= 0.1136 +/- 0.0118 | g_re= -0.0309 +/- 0.0104 |
g_im= 0.0137 +/- 0.0135 | g_im= 0.0938 +/- 0.0146 | g_im= 0.0966 +/- 0.0064 |
corr= [ 0.41] | corr= [ 0.16] | corr= [ 0.13] |
=====
*****
```

```
*****

JP=0+ || eta:eta/1^S_0[+] kaon:kaon/1^S_0[-] pi:pi/1^S_0[+]

sqrt(s)_pole = (0.24796 +/- 0.0086701)
               + (i/2)*(-0.048729 +/- 0.013232) [-0.55]

=====
eta:eta/1^S_0 | kaon:kaon/1^S_0 | pi:pi/1^S_0 |
=====
k_re= -0.0703 +/- 0.0079 | k_re= 0.0786 +/- 0.0070 | k_re= -0.1033 +/- 0.0053 |
k_im= 0.0215 +/- 0.0049 | k_im= -0.0192 +/- 0.0046 | k_im= 0.0146 +/- 0.0038 |
corr= [-0.43] | corr= [-0.47] | corr= [-0.53] |
=====
|g|= 0.0841 +/- 0.0092 | |g|= 0.1484 +/- 0.0064 | |g|= 0.0565 +/- 0.0144 |
arg(g)/pi= -0.3826 +/- 0.1028 | arg(g)/pi= -0.5901 +/- 0.0204 | arg(g)/pi= 0.9135 +/- 0.0324 |
=====
g_re= 0.0303 +/- 0.0281 | g_re= -0.0414 +/- 0.0095 | g_re= -0.0544 +/- 0.0137 |
g_im= -0.0784 +/- 0.0057 | g_im= -0.1425 +/- 0.0063 | g_im= 0.0151 +/- 0.0073 |
corr= [ 0.43] | corr= [-0.10] | corr= [-0.59] |
=====
*****
```

```
*****

JP=0+ || eta:eta/1^S_0[+] kaon:kaon/1^S_0[-] pi:pi/1^S_0[-]

sqrt(s)_pole = (0.12541 +/- 0.0070143)
               + (i/2)*(+3.1819e-17 +/- 7.1552e-13) [-0.04]

=====
eta:eta/1^S_0 | kaon:kaon/1^S_0 | pi:pi/1^S_0 |
=====
k_re= 0.0000 +/- 0.0000 | k_re= -0.0000 +/- 0.0000 | k_re= 0.0000 +/- 0.0000 |
k_im= 0.0825 +/- 0.0027 | k_im= -0.0740 +/- 0.0030 | k_im= -0.0289 +/- 0.0076 |
corr= [ 0.04] | corr= [ 0.04] | corr= [ 0.05] |
=====
|g|= 0.1037 +/- 0.0306 | |g|= 0.0163 +/- 0.0013 | |g|= 0.0835 +/- 0.0043 |
arg(g)/pi= 0.5000 +/- 0.0000 | arg(g)/pi= 0.5000 +/- 0.0000 | arg(g)/pi= -0.5000 +/- 0.0000 |
=====
g_re= 0.0000 +/- 0.0000 | g_re= -0.0000 +/- 0.0000 | g_re= 0.0000 +/- 0.0000 |
g_im= 0.1037 +/- 0.0306 | g_im= 0.0163 +/- 0.0013 | g_im= -0.0835 +/- 0.0043 |
corr= [-1.00] | corr= [-0.15] | corr= [-0.76] |
=====
*****
```

```
*****

JP=0+ || eta:eta/1^S_0[+] kaon:kaon/1^S_0[-] pi:pi/1^S_0[-]

sqrt(s)_pole = (0.18661 +/- 0.0067307)
               + (i/2)*(-0.12467 +/- 0.020559) [-0.02]

=====
eta:eta/1^S_0 | kaon:kaon/1^S_0 | pi:pi/1^S_0 |
=====
k_re= -0.0421 +/- 0.0052 | k_re= 0.0468 +/- 0.0051 | k_re= 0.0689 +/- 0.0043 |
k_im= 0.0691 +/- 0.0054 | k_im= -0.0621 +/- 0.0058 | k_im= -0.0422 +/- 0.0061 |
corr= [-0.40] | corr= [-0.38] | corr= [-0.21] |
=====
|g|= 0.1847 +/- 0.0244 | |g|= 0.0670 +/- 0.0069 | |g|= 0.0657 +/- 0.0088 |
arg(g)/pi= 0.0754 +/- 0.0145 | arg(g)/pi= -0.3569 +/- 0.0532 | arg(g)/pi= 0.6762 +/- 0.0492 |
=====
*****
```

```

g_re= 0.1796 +/- 0.0226 | g_re= 0.0291 +/- 0.0113 | g_re= -0.0346 +/- 0.0055 |
g_im= 0.0434 +/- 0.0125 | g_im= -0.0604 +/- 0.0067 | g_im= 0.0559 +/- 0.0123 |
corr= [ 0.82] | corr= [ 0.22] | corr= [ 0.65] |
*****

*****
JP=0+ || eta:eta/1^S_0[+] kaon:kaon/1^S_0[-] pi:pi/1^S_0[-]

sqrt(s)_pole = (0.25773 +/- 0.0070572)
+ (i/2)*(-0.057453 +/- 0.0074957) [-0.12]

eta:eta/1^S_0 | kaon:kaon/1^S_0 | pi:pi/1^S_0 |
=====|=====|=====|
k_re= -0.0788 +/- 0.0056 | k_re= 0.0863 +/- 0.0052 | k_re= 0.1092 +/- 0.0042 |
k_im= 0.0235 +/- 0.0030 | k_im= -0.0214 +/- 0.0027 | k_im= -0.0170 +/- 0.0022 |
corr= [ 0.12] | corr= [ 0.06] | corr= [-0.06] |
=====|=====|=====|
|g|= 0.0137 +/- 0.7028 | |g|= 0.0356 +/- 1.8712 | |g|= 0.0167 +/- 0.9258 |
arg(g)/pi= -0.4669 +/- 1.6864 | arg(g)/pi= -0.5992 +/- 0.0977 | arg(g)/pi= -0.5659 +/- 0.0732 |
=====|=====|=====|
g_re= 0.0014 +/- 0.0190 | g_re= -0.0109 +/- 0.5819 | g_re= -0.0034 +/- 0.1915 |
g_im= -0.0136 +/- 0.7062 | g_im= -0.0338 +/- 1.7785 | g_im= -0.0164 +/- 0.9057 |
corr= [-0.16] | corr= [ 1.00] | corr= [ 1.00] |
=====|=====|=====|
*****

*****
JP=0+ || eta:eta/1^S_0[-] kaon:kaon/1^S_0[+] pi:pi/1^S_0[+]

sqrt(s)_pole = (0.13048 +/- 0.013821)
+ (i/2)*(-0.069735 +/- 0.0059076) [-0.32]

eta:eta/1^S_0 | kaon:kaon/1^S_0 | pi:pi/1^S_0 |
=====|=====|=====|
k_re= 0.0136 +/- 0.0028 | k_re= -0.0151 +/- 0.0032 | k_re= -0.0283 +/- 0.0078 |
k_im= -0.0835 +/- 0.0049 | k_im= 0.0754 +/- 0.0053 | k_im= 0.0402 +/- 0.0058 |
corr= [ 0.89] | corr= [ 0.90] | corr= [ 0.91] |
=====|=====|=====|
|g|= 0.0401 +/- 0.0093 | |g|= 0.0762 +/- 0.0218 | |g|= 0.1389 +/- 0.0157 |
arg(g)/pi= 0.3178 +/- 0.0453 | arg(g)/pi= -0.9080 +/- 0.1015 | arg(g)/pi= -0.7703 +/- 0.0100 |
=====|=====|=====|
g_re= 0.0217 +/- 0.0026 | g_re= -0.0730 +/- 0.0142 | g_re= -0.1043 +/- 0.0127 |
g_im= 0.0337 +/- 0.0106 | g_im= -0.0217 +/- 0.0294 | g_im= -0.0918 +/- 0.0103 |
corr= [ 0.20] | corr= [ 0.97] | corr= [ 0.86] |
=====|=====|=====|
*****

*****
JP=0+ || eta:eta/1^S_0[-] kaon:kaon/1^S_0[+] pi:pi/1^S_0[+]

sqrt(s)_pole = (0.24147 +/- 0.012921)
+ (i/2)*(-0.10573 +/- 0.01586) [-0.34]

eta:eta/1^S_0 | kaon:kaon/1^S_0 | pi:pi/1^S_0 |
=====|=====|=====|
k_re= 0.0716 +/- 0.0097 | k_re= -0.0783 +/- 0.0093 | k_re= -0.1006 +/- 0.0077 |
k_im= -0.0446 +/- 0.0053 | k_im= 0.0407 +/- 0.0051 | k_im= 0.0317 +/- 0.0044 |
corr= [ 0.06] | corr= [-0.04] | corr= [-0.25] |
=====|=====|=====|
|g|= 0.1546 +/- 0.0091 | |g|= 0.1028 +/- 0.0089 | |g|= 0.0710 +/- 0.0116 |
arg(g)/pi= 0.4609 +/- 0.0409 | arg(g)/pi= 0.7123 +/- 0.0468 | arg(g)/pi= -0.0469 +/- 0.0363 |
=====|=====|=====|
g_re= 0.0189 +/- 0.0206 | g_re= -0.0636 +/- 0.0155 | g_re= 0.0702 +/- 0.0118 |
g_im= 0.1534 +/- 0.0072 | g_im= 0.0808 +/- 0.0082 | g_im= -0.0104 +/- 0.0079 |
corr= [ 0.71] | corr= [ 0.44] | corr= [ 0.04] |
=====|=====|=====|
*****

*****
JP=0+ || eta:eta/1^S_0[-] kaon:kaon/1^S_0[+] pi:pi/1^S_0[-]

sqrt(s)_pole = (0.25594 +/- 0.010139)
+ (i/2)*(-0.10466 +/- 0.012764) [-0.34]

eta:eta/1^S_0 | kaon:kaon/1^S_0 | pi:pi/1^S_0 |
=====|=====|=====|
k_re= 0.0815 +/- 0.0075 | k_re= -0.0880 +/- 0.0071 | k_re= 0.1089 +/- 0.0059 |
k_im= -0.0411 +/- 0.0042 | k_im= 0.0381 +/- 0.0040 | k_im= -0.0307 +/- 0.0035 |
corr= [-0.06] | corr= [-0.13] | corr= [-0.27] |
=====|=====|=====|
|g|= 0.1357 +/- 0.0117 | |g|= 0.0809 +/- 0.0105 | |g|= 0.0604 +/- 0.0098 |
arg(g)/pi= 0.4059 +/- 0.0255 | arg(g)/pi= 0.6157 +/- 0.0894 | arg(g)/pi= 0.5061 +/- 0.0299 |
=====|=====|=====|
g_re= 0.0395 +/- 0.0131 | g_re= -0.0288 +/- 0.0228 | g_re= -0.0012 +/- 0.0057 |
g_im= 0.1298 +/- 0.0092 | g_im= 0.0756 +/- 0.0103 | g_im= 0.0603 +/- 0.0097 |
corr= [ 0.67] | corr= [ 0.31] | corr= [-0.32] |
=====|=====|=====|
*****

*****
JP=0+ || eta:eta/1^S_0[-] kaon:kaon/1^S_0[+] pi:pi/1^S_0[-]

sqrt(s)_pole = (0.17222 +/- 0.0048561)
+ (i/2)*(-0.016004 +/- 0.0048476) [-0.58]

eta:eta/1^S_0 | kaon:kaon/1^S_0 | pi:pi/1^S_0 |
=====|=====|=====|
k_re= 0.0059 +/- 0.0021 | k_re= -0.0076 +/- 0.0029 | k_re= 0.0517 +/- 0.0041 |
k_im= -0.0581 +/- 0.0034 | k_im= 0.0454 +/- 0.0042 | k_im= -0.0067 +/- 0.0018 |
corr= [ 0.69] | corr= [ 0.72] | corr= [-0.49] |
=====|=====|=====|

```

|                                    |                                   |                                   |
|------------------------------------|-----------------------------------|-----------------------------------|
| $ g  = 0.0562 \pm 0.0094$          | $ g  = 0.2120 \pm 0.0096$         | $ g  = 0.0593 \pm 0.0080$         |
| $\arg(g)/\pi = -0.1709 \pm 0.0217$ | $\arg(g)/\pi = 0.0050 \pm 0.0156$ | $\arg(g)/\pi = 0.5227 \pm 0.0185$ |
| $g_{re} = 0.0483 \pm 0.0091$       | $g_{re} = 0.2120 \pm 0.0097$      | $g_{re} = -0.0042 \pm 0.0030$     |
| $g_{im} = -0.0288 \pm 0.0043$      | $g_{im} = 0.0033 \pm 0.0103$      | $g_{im} = 0.0591 \pm 0.0082$      |
| $corr = [-0.60]$                   | $corr = [-0.71]$                  | $corr = [0.75]$                   |

\*\*\*\*\*

\*\*\*\*\*

JP=0+ || eta:eta/1^S\_0[-] kaon:kaon/1^S\_0[-] pi:pi/1^S\_0[+]

$\sqrt{s}_{pole} = (0.24513 \pm 0.0084416)$   
 $+ (i/2)*(-0.011868 \pm 0.0081487) [0.46]$

|                                   |                                   |                                    |  |             |  |
|-----------------------------------|-----------------------------------|------------------------------------|--|-------------|--|
| eta:eta/1^S_0                     |                                   | kaon:kaon/1^S_0                    |  | pi:pi/1^S_0 |  |
| $k_{re} = 0.0656 \pm 0.0077$      | $k_{re} = 0.0750 \pm 0.0068$      | $k_{re} = -0.1013 \pm 0.0051$      |  |             |  |
| $k_{im} = -0.0055 \pm 0.0040$     | $k_{im} = -0.0048 \pm 0.0035$     | $k_{im} = 0.0036 \pm 0.0025$       |  |             |  |
| $corr = [0.53]$                   | $corr = [0.51]$                   | $corr = [0.47]$                    |  |             |  |
| $ g  = 0.0874 \pm 0.0098$         | $ g  = 0.1026 \pm 0.0073$         | $ g  = 0.0997 \pm 0.0082$          |  |             |  |
| $\arg(g)/\pi = 0.4541 \pm 0.0847$ | $\arg(g)/\pi = 0.3328 \pm 0.0493$ | $\arg(g)/\pi = -0.2199 \pm 0.0237$ |  |             |  |
| $g_{re} = 0.0126 \pm 0.0223$      | $g_{re} = 0.0514 \pm 0.0141$      | $g_{re} = 0.0768 \pm 0.0058$       |  |             |  |
| $g_{im} = 0.0865 \pm 0.0117$      | $g_{im} = 0.0887 \pm 0.0104$      | $g_{im} = -0.0635 \pm 0.0094$      |  |             |  |
| $corr = [-0.67]$                  | $corr = [-0.61]$                  | $corr = [-0.20]$                   |  |             |  |

\*\*\*\*\*

\*\*\*\*\*

JP=0+ || eta:eta/1^S\_0[-] kaon:kaon/1^S\_0[-] pi:pi/1^S\_0[+]

$\sqrt{s}_{pole} = (0.13214 \pm 0.01546)$   
 $+ (i/2)*(-0.056617 \pm 0.013843) [-0.94]$

|                                   |                                   |                                    |  |             |  |
|-----------------------------------|-----------------------------------|------------------------------------|--|-------------|--|
| eta:eta/1^S_0                     |                                   | kaon:kaon/1^S_0                    |  | pi:pi/1^S_0 |  |
| $k_{re} = 0.0114 \pm 0.0047$      | $k_{re} = 0.0127 \pm 0.0054$      | $k_{re} = -0.0261 \pm 0.0121$      |  |             |  |
| $k_{im} = -0.0819 \pm 0.0050$     | $k_{im} = -0.0735 \pm 0.0054$     | $k_{im} = 0.0359 \pm 0.0044$       |  |             |  |
| $corr = [0.97]$                   | $corr = [0.97]$                   | $corr = [0.92]$                    |  |             |  |
| $ g  = 0.0483 \pm 0.0053$         | $ g  = 0.0104 \pm 0.0035$         | $ g  = 0.1523 \pm 0.0234$          |  |             |  |
| $\arg(g)/\pi = 0.2642 \pm 0.0308$ | $\arg(g)/\pi = 0.1288 \pm 0.0806$ | $\arg(g)/\pi = -0.7503 \pm 0.0035$ |  |             |  |
| $g_{re} = 0.0326 \pm 0.0021$      | $g_{re} = 0.0096 \pm 0.0024$      | $g_{re} = -0.1078 \pm 0.0167$      |  |             |  |
| $g_{im} = 0.0357 \pm 0.0068$      | $g_{im} = 0.0041 \pm 0.0037$      | $g_{im} = -0.1076 \pm 0.0165$      |  |             |  |
| $corr = [0.10]$                   | $corr = [0.83]$                   | $corr = [0.99]$                    |  |             |  |

\*\*\*\*\*

\*\*\*\*\*

JP=0+ || eta:eta/1^S\_0[-] kaon:kaon/1^S\_0[-] pi:pi/1^S\_0[-]

$\sqrt{s}_{pole} = (0.25843 \pm 0.007402)$   
 $+ (i/2)*(-0.0495 \pm 0.0028793) [0.28]$

|                                   |                                   |                                   |  |             |  |
|-----------------------------------|-----------------------------------|-----------------------------------|--|-------------|--|
| eta:eta/1^S_0                     |                                   | kaon:kaon/1^S_0                   |  | pi:pi/1^S_0 |  |
| $k_{re} = 0.0788 \pm 0.0058$      | $k_{re} = 0.0865 \pm 0.0054$      | $k_{re} = 0.1095 \pm 0.0043$      |  |             |  |
| $k_{im} = -0.0203 \pm 0.0016$     | $k_{im} = -0.0185 \pm 0.0014$     | $k_{im} = -0.0146 \pm 0.0009$     |  |             |  |
| $corr = [0.73]$                   | $corr = [0.66]$                   | $corr = [0.44]$                   |  |             |  |
| $ g  = 0.0376 \pm 0.0090$         | $ g  = 0.0821 \pm 0.0037$         | $ g  = 0.0697 \pm 0.0038$         |  |             |  |
| $\arg(g)/\pi = 0.4688 \pm 0.1759$ | $\arg(g)/\pi = 0.4305 \pm 0.0581$ | $\arg(g)/\pi = 0.3875 \pm 0.0207$ |  |             |  |
| $g_{re} = 0.0037 \pm 0.0203$      | $g_{re} = 0.0178 \pm 0.0144$      | $g_{re} = 0.0241 \pm 0.0052$      |  |             |  |
| $g_{im} = 0.0374 \pm 0.0100$      | $g_{im} = 0.0802 \pm 0.0054$      | $g_{im} = 0.0654 \pm 0.0028$      |  |             |  |
| $corr = [-0.57]$                  | $corr = [-0.74]$                  | $corr = [0.45]$                   |  |             |  |

\*\*\*\*\*



# k\_lccclcc\_noCM

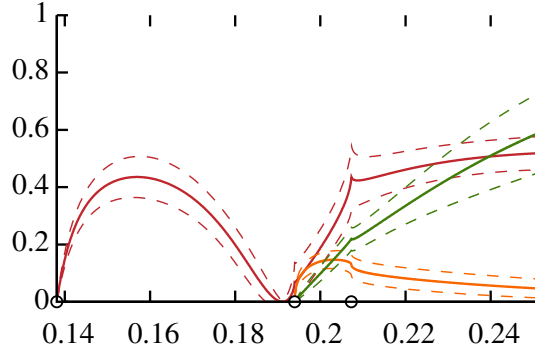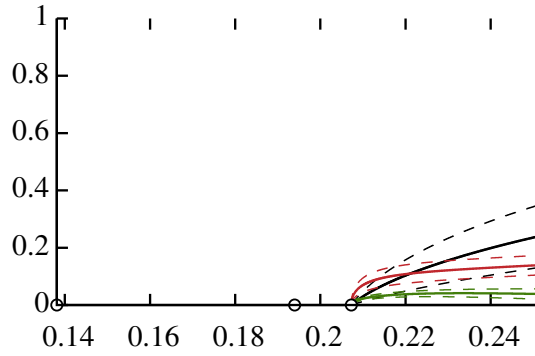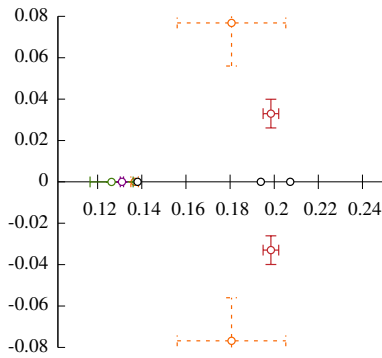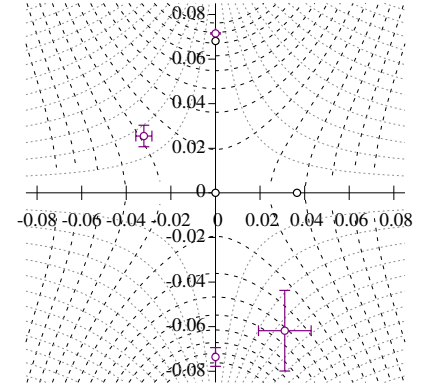

## parameter values

minimised with  $\text{chisq}/\text{nDoF} = 50.67 / (57 - 8) = 1.03$

|                                                   |                      |       |       |       |       |       |      |       |       |
|---------------------------------------------------|----------------------|-------|-------|-------|-------|-------|------|-------|-------|
| JPO+_gamma_eta:eta/1^S_0 eta:eta/1^S_0_order0     | -0.23422 +/- 0.18522 | 1.00  | 0.21  | -0.83 | 0.18  | -0.28 | 0.50 | 0.41  | -0.16 |
| JPO+_gamma_eta:eta/1^S_0 kaon:kaon/1^S_0_order0   | 0.24572 +/- 0.17058  | 1.00  | -0.54 | 0.07  | -0.09 | 0.05  | 0.25 | -0.15 |       |
| JPO+_gamma_eta:eta/1^S_0 pi:pi/1^S_0_order0       | -1.5503 +/- 0.42569  | 1.00  | -0.39 | 0.48  | -0.38 | -0.67 | 0.43 |       |       |
| JPO+_gamma_kaon:kaon/1^S_0 kaon:kaon/1^S_0_order0 | 0.90384 +/- 1.3446   | 1.00  | -0.98 | 0.01  | 0.08  | 0.04  |      |       |       |
| JPO+_gamma_kaon:kaon/1^S_0 kaon:kaon/1^S_0_order1 | -1.6812 +/- 1.1897   | 1.00  | -0.08 | -0.15 | -0.00 |       |      |       |       |
| JPO+_gamma_kaon:kaon/1^S_0 pi:pi/1^S_0_order0     | -1.3651 +/- 0.15966  | 1.00  | -0.07 | 0.21  |       |       |      |       |       |
| JPO+_gamma_pi:pi/1^S_0 pi:pi/1^S_0_order0         | 1.9054 +/- 1.1305    | 1.00  | -0.07 | -0.94 |       |       |      |       |       |
| JPO+_gamma_pi:pi/1^S_0 pi:pi/1^S_0_order1         | -0.51864 +/- 0.82934 | 1.00  |       |       |       |       |      |       |       |
| JPO+_gamma_eta:eta/1^S_0 eta:eta/1^S_0_order1     | 0.0000 +/- 0         | FIXED |       |       |       |       |      |       |       |
| JPO+_gamma_eta:eta/1^S_0 kaon:kaon/1^S_0_order1   | 0.0000 +/- 0         | FIXED |       |       |       |       |      |       |       |
| JPO+_gamma_eta:eta/1^S_0 pi:pi/1^S_0_order1       | 0.0000 +/- 0         | FIXED |       |       |       |       |      |       |       |
| JPO+_gamma_kaon:kaon/1^S_0 pi:pi/1^S_0_order1     | 0.0000 +/- 0         | FIXED |       |       |       |       |      |       |       |

## pole singularities

\*\*\*\*\*  
JP=0+ || eta:eta/1^S\_0[+] kaon:kaon/1^S\_0[+] pi:pi/1^S\_0[+]

$\text{sqrt}(s)_{\text{pole}} = (0.13102 \pm 0.00073957) + (i/2)*(+5.2217e-17 \pm 1.5498e-14) [-0.00]$

| eta:eta/1^S_0                | kaon:kaon/1^S_0               | pi:pi/1^S_0                   |
|------------------------------|-------------------------------|-------------------------------|
| k_re= 0.0000 +/- 0.0000      | k_re= 0.0000 +/- 0.0000       | k_re= 0.0000 +/- 0.0000       |
| k_im= 0.0803 +/- 0.0003      | k_im= 0.0715 +/- 0.0003       | k_im= 0.0219 +/- 0.0011       |
| corr= [ 0.00]                | corr= [ 0.00]                 | corr= [ 0.00]                 |
| g = 0.0583 +/- 0.0124        | g = 0.0209 +/- 0.0241         | g = 0.0913 +/- 0.0037         |
| arg(g)/pi= 0.0000 +/- 0.0000 | arg(g)/pi= -0.0000 +/- 0.0000 | arg(g)/pi= -0.0000 +/- 0.0000 |
| g_re= 0.0583 +/- 0.0124      | g_re= 0.0209 +/- 0.0241       | g_re= 0.0913 +/- 0.0037       |
| g_im= 0.0000 +/- 0.0000      | g_im= -0.0000 +/- 0.0000      | g_im= -0.0000 +/- 0.0000      |
| corr= [-1.00]                | corr= [-0.99]                 | corr= [-0.89]                 |

\*\*\*\*\*

\*\*\*\*\*  
JP=0+ || eta:eta/1^S\_0[+] kaon:kaon/1^S\_0[+] pi:pi/1^S\_0[-]

```

sqrt(s)_pole = (0.19852 +/- 0.0035389)
+ (i/2)*(-0.032997 +/- 0.0069252) [ 0.30]

=====
eta:eta/1^S_0 | kaon:kaon/1^S_0 | pi:pi/1^S_0 |
=====
k_re= -0.0217 +/- 0.0034 | k_re= -0.0321 +/- 0.0036 | k_re= 0.0717 +/- 0.0024 |
k_im= 0.0378 +/- 0.0046 | k_im= 0.0255 +/- 0.0048 | k_im= -0.0114 +/- 0.0024 |
corr= [-0.09] | corr= [ 0.14] | corr= [ 0.30] |
=====
|g|= 0.1219 +/- 0.0244 | |g|= 0.1228 +/- 0.0208 | |g|= 0.1022 +/- 0.0138 |
arg(g)/pi= 0.0515 +/- 0.0341 | arg(g)/pi= 0.1371 +/- 0.0242 | arg(g)/pi= 0.5883 +/- 0.0339 |
=====
g_re= 0.1203 +/- 0.0245 | g_re= 0.1116 +/- 0.0204 | g_re= -0.0280 +/- 0.0093 |
g_im= 0.0196 +/- 0.0130 | g_im= 0.0513 +/- 0.0102 | g_im= 0.0983 +/- 0.0149 |
corr= [ 0.09] | corr= [ 0.45] | corr= [ 0.29] |
=====
*****

*****
JP=0+ || eta:eta/1^S_0[+] kaon:kaon/1^S_0[-] pi:pi/1^S_0[+]

sqrt(s)_pole = (0.12632 +/- 0.0097708)
+ (i/2)*(-5.1799e-15 +/- 1.5562e-12) [ 0.01]

=====
eta:eta/1^S_0 | kaon:kaon/1^S_0 | pi:pi/1^S_0 |
=====
k_re= -0.0000 +/- 0.0000 | k_re= 0.0000 +/- 0.0000 | k_re= -0.0000 +/- 0.0000 |
k_im= 0.0822 +/- 0.0037 | k_im= -0.0736 +/- 0.0042 | k_im= 0.0279 +/- 0.0110 |
corr= [-0.01] | corr= [-0.01] | corr= [-0.01] |
=====
|g|= 0.0911 +/- 0.0378 | |g|= 0.0260 +/- 0.0459 | |g|= 0.0816 +/- 0.0127 |
arg(g)/pi= 0.0000 +/- 0.0000 | arg(g)/pi= -0.0000 +/- 0.0000 | arg(g)/pi= -0.0000 +/- 0.0000 |
=====
g_re= 0.0911 +/- 0.0378 | g_re= 0.0260 +/- 0.0459 | g_re= 0.0816 +/- 0.0127 |
g_im= 0.0000 +/- 0.0000 | g_im= -0.0000 +/- 0.0000 | g_im= -0.0000 +/- 0.0000 |
corr= [-1.00] | corr= [-0.96] | corr= [-0.83] |
=====
*****

*****
JP=0+ || eta:eta/1^S_0[+] kaon:kaon/1^S_0[-] pi:pi/1^S_0[-]

sqrt(s)_pole = (0.16824 +/- 0.031137)
+ (i/2)*(-0.091474 +/- 0.029155) [ 0.44]

=====
eta:eta/1^S_0 | kaon:kaon/1^S_0 | pi:pi/1^S_0 |
=====
k_re= -0.0274 +/- 0.0098 | k_re= 0.0311 +/- 0.0118 | k_re= 0.0549 +/- 0.0188 |
k_im= 0.0703 +/- 0.0173 | k_im= -0.0618 +/- 0.0181 | k_im= -0.0351 +/- 0.0133 |
corr= [ 0.60] | corr= [ 0.66] | corr= [ 0.68] |
=====
|g|= 0.2035 +/- 0.0450 | |g|= 0.0751 +/- 0.0177 | |g|= 0.1382 +/- 0.0266 |
arg(g)/pi= -0.0716 +/- 0.0964 | arg(g)/pi= -0.1670 +/- 0.1700 | arg(g)/pi= 0.4634 +/- 0.0778 |
=====
g_re= 0.1984 +/- 0.0545 | g_re= 0.0650 +/- 0.0305 | g_re= 0.0159 +/- 0.0313 |
g_im= -0.0454 +/- 0.0534 | g_im= -0.0376 +/- 0.0316 | g_im= 0.1372 +/- 0.0294 |
corr= [ 0.74] | corr= [ 0.76] | corr= [-0.76] |
=====
*****

*****
JP=0+ || eta:eta/1^S_0[-] kaon:kaon/1^S_0[+] pi:pi/1^S_0[+]

sqrt(s)_pole = (0.15955 +/- 0.060291)
+ (i/2)*(-0.12074 +/- 0.055488) [ 0.93]

=====
eta:eta/1^S_0 | kaon:kaon/1^S_0 | pi:pi/1^S_0 |
=====
k_re= 0.0305 +/- 0.0113 | k_re= -0.0338 +/- 0.0143 | k_re= -0.0527 +/- 0.0291 |
k_im= -0.0788 +/- 0.0313 | k_im= 0.0713 +/- 0.0327 | k_im= 0.0457 +/- 0.0281 |
corr= [ 0.89] | corr= [ 0.92] | corr= [ 0.96] |
=====
|g|= 0.0548 +/- 0.0184 | |g|= 0.1588 +/- 0.0260 | |g|= 0.0796 +/- 0.0363 |
arg(g)/pi= 0.3725 +/- 0.1343 | arg(g)/pi= 0.1380 +/- 0.0346 | arg(g)/pi= 0.0195 +/- 0.0565 |
=====
g_re= 0.0214 +/- 0.0245 | g_re= 0.1441 +/- 0.0289 | g_re= 0.0794 +/- 0.0356 |
g_im= 0.0505 +/- 0.0165 | g_im= 0.0667 +/- 0.0119 | g_im= 0.0049 +/- 0.0160 |
corr= [ 0.05] | corr= [-0.14] | corr= [ 0.84] |
=====
*****

*****
JP=0+ || eta:eta/1^S_0[-] kaon:kaon/1^S_0[+] pi:pi/1^S_0[-]

sqrt(s)_pole = (0.18065 +/- 0.024611)
+ (i/2)*(-0.076823 +/- 0.02085) [ 0.06]

=====
eta:eta/1^S_0 | kaon:kaon/1^S_0 | pi:pi/1^S_0 |
=====
k_re= 0.0283 +/- 0.0113 | k_re= -0.0333 +/- 0.0137 | k_re= 0.0617 +/- 0.0164 |
k_im= -0.0613 +/- 0.0144 | k_im= 0.0522 +/- 0.0145 | k_im= -0.0281 +/- 0.0080 |
corr= [ 0.68] | corr= [ 0.70] | corr= [ 0.42] |
=====
|g|= 0.0603 +/- 0.0219 | |g|= 0.1882 +/- 0.0432 | |g|= 0.0795 +/- 0.0515 |
arg(g)/pi= 0.0229 +/- 0.1659 | arg(g)/pi= 0.1078 +/- 0.0725 | arg(g)/pi= 0.7108 +/- 0.1378 |
=====
g_re= 0.0602 +/- 0.0237 | g_re= 0.1775 +/- 0.0542 | g_re= -0.0489 +/- 0.0098 |
g_im= 0.0043 +/- 0.0301 | g_im= 0.0625 +/- 0.0276 | g_im= 0.0627 +/- 0.0612 |
corr= [-0.81] | corr= [-0.89] | corr= [-0.50] |
=====
*****

```

```

*****
JP=0+  ||  eta:eta/1^S_0[-] kaon:kaon/1^S_0[-] pi:pi/1^S_0[-]

sqrt(s)_pole = (0.13679 +/- 0.0017116)
               + (i/2)*(+5.9472e-15 +/- 1.7877e-12) [-0.06]

=====
eta:eta/1^S_0 | kaon:kaon/1^S_0 | pi:pi/1^S_0 |
=====
k_re= -0.0000 +/- 0.0000 | k_re= -0.0000 +/- 0.0000 | k_re= -0.0000 +/- 0.0000 |
k_im= -0.0779 +/- 0.0008 | k_im= -0.0688 +/- 0.0009 | k_im= -0.0096 +/- 0.0061 |
corr= [ 0.06] | corr= [ 0.06] | corr= [ 0.06] |
=====
|g|= 0.0157 +/- 0.0073 | |g|= 0.0190 +/- 0.0088 | |g|= 0.0698 +/- 0.0205 |
arg(g)/pi= 0.5000 +/- 0.0000 | arg(g)/pi= 0.5000 +/- 0.0000 | arg(g)/pi= -0.5000 +/- 0.0000 |
=====
g_re= 0.0000 +/- 0.0000 | g_re= -0.0000 +/- 0.0000 | g_re= 0.0000 +/- 0.0000 |
g_im= 0.0157 +/- 0.0073 | g_im= 0.0190 +/- 0.0088 | g_im= -0.0698 +/- 0.0205 |
corr= [-1.00] | corr= [-0.53] | corr= [ 0.81] |
=====
*****

```

# k\_llclcc\_noCM

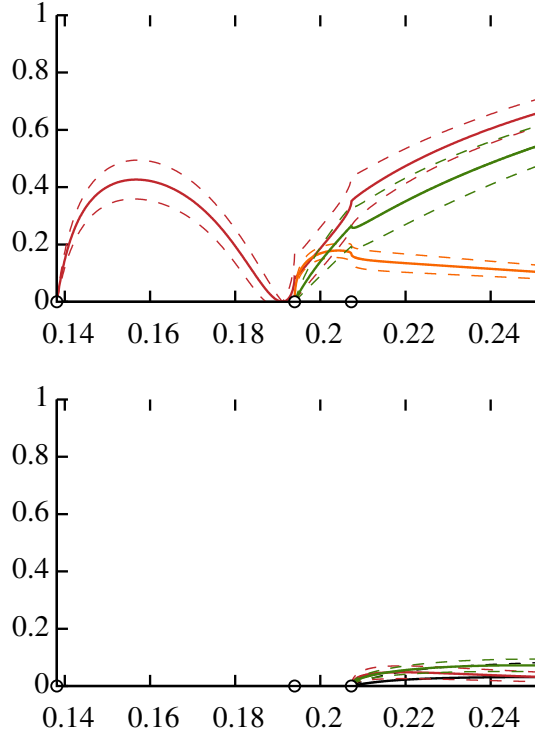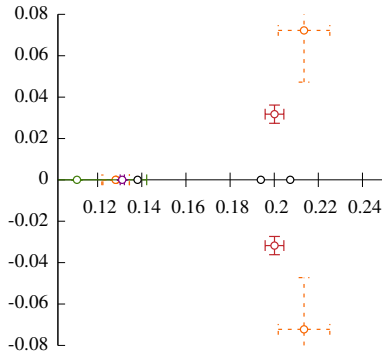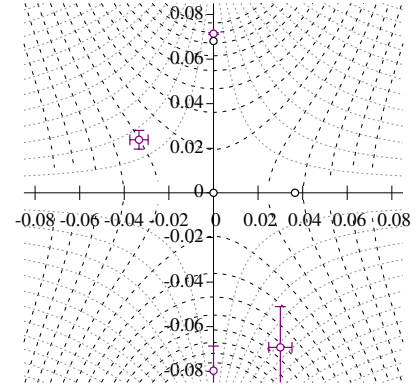

## parameter values

minimised with chisq/nDoF = 46.11 / (57 - 9) = 0.96

|                                                   |                      |       |       |       |       |       |       |       |      |       |
|---------------------------------------------------|----------------------|-------|-------|-------|-------|-------|-------|-------|------|-------|
| JPO+_gamma_eta:eta/1^S_0 eta:eta/1^S_0_order0     | -0.18324 +/- 0.28051 | 1.00  | -0.42 | 0.33  | -0.66 | -0.53 | -0.40 | 0.09  | 0.13 | -0.14 |
| JPO+_gamma_eta:eta/1^S_0 kaon:kaon/1^S_0_order0   | -0.20925 +/- 0.08904 | 1.00  | -0.50 | -0.10 | 0.30  | -0.08 | 0.30  | 0.08  | 0.05 |       |
| JPO+_gamma_eta:eta/1^S_0 pi:pi/1^S_0_order0       | -1.1452 +/- 0.26641  | 1.00  | -0.25 | -0.20 | -0.43 | 0.02  | -0.30 | -0.02 |      |       |
| JPO+_gamma_kaon:kaon/1^S_0 kaon:kaon/1^S_0_order0 | -0.18715 +/- 0.18954 | 1.00  | 0.03  | 0.24  | 0.01  | -0.06 | 0.11  |       |      |       |
| JPO+_gamma_kaon:kaon/1^S_0 kaon:kaon/1^S_0_order1 | -0.84889 +/- 0.24817 | 1.00  | 0.04  | 0.14  | -0.15 | 0.12  |       |       |      |       |
| JPO+_gamma_kaon:kaon/1^S_0 pi:pi/1^S_0_order0     | 0.38634 +/- 0.31091  | 1.00  | -0.81 | -0.04 | 0.15  |       |       |       |      |       |
| JPO+_gamma_kaon:kaon/1^S_0 pi:pi/1^S_0_order1     | -1.6799 +/- 0.2665   | 1.00  | -0.10 | 0.08  |       |       |       |       |      |       |
| JPO+_gamma_pi:pi/1^S_0 pi:pi/1^S_0_order0         | 1.3111 +/- 0.65271   | 1.00  | -0.90 |       |       |       |       |       |      |       |
| JPO+_gamma_pi:pi/1^S_0 pi:pi/1^S_0_order1         | -0.33354 +/- 0.57855 | 1.00  |       |       |       |       |       |       |      |       |
| JPO+_gamma_eta:eta/1^S_0 eta:eta/1^S_0_order1     | 0.0000 +/- 0         | FIXED |       |       |       |       |       |       |      |       |
| JPO+_gamma_eta:eta/1^S_0 kaon:kaon/1^S_0_order1   | 0.0000 +/- 0         | FIXED |       |       |       |       |       |       |      |       |
| JPO+_gamma_eta:eta/1^S_0 pi:pi/1^S_0_order1       | 0.0000 +/- 0         | FIXED |       |       |       |       |       |       |      |       |

## pole singularities

JP=0+ || eta:eta/1^S\_0[+] kaon:kaon/1^S\_0[+] pi:pi/1^S\_0[+]

sqrt(s)\_pole = (0.13116 +/- 0.00096653)  
+ (i/2)\*(+7.999e-16 +/- 1.7314e-13) [-0.08]

| eta:eta/1^S_0                | kaon:kaon/1^S_0               | pi:pi/1^S_0                   |
|------------------------------|-------------------------------|-------------------------------|
| k_re= 0.0000 +/- 0.0000      | k_re= 0.0000 +/- 0.0000       | k_re= 0.0000 +/- 0.0000       |
| k_im= 0.0803 +/- 0.0004      | k_im= 0.0714 +/- 0.0004       | k_im= 0.0217 +/- 0.0015       |
| corr= [ 0.08]                | corr= [ 0.08]                 | corr= [ 0.08]                 |
| g = 0.0660 +/- 0.0161        | g = 0.0757 +/- 0.0559         | g = 0.0897 +/- 0.0034         |
| arg(g)/pi= 0.0000 +/- 0.0000 | arg(g)/pi= -0.0000 +/- 0.0000 | arg(g)/pi= -0.0000 +/- 0.0000 |
| g_re= 0.0660 +/- 0.0161      | g_re= 0.0757 +/- 0.0559       | g_re= 0.0897 +/- 0.0034       |
| g_im= 0.0000 +/- 0.0000      | g_im= -0.0000 +/- 0.0000      | g_im= -0.0000 +/- 0.0000      |
| corr= [-1.00]                | corr= [-0.97]                 | corr= [-0.53]                 |

JP=0+ || eta:eta/1^S\_0[+] kaon:kaon/1^S\_0[+] pi:pi/1^S\_0[-]

```

sqrt(s)_pole = (0.20015 +/- 0.0042337)
+ (i/2)*(-0.031742 +/- 0.0044008) [ 0.40]

=====
eta:eta/1^S_0 | kaon:kaon/1^S_0 | pi:pi/1^S_0 |
=====
k_re= -0.0222 +/- 0.0029 | k_re= -0.0334 +/- 0.0041 | k_re= 0.0728 +/- 0.0028 |
k_im= 0.0358 +/- 0.0049 | k_im= 0.0238 +/- 0.0042 | k_im= -0.0109 +/- 0.0016 |
corr= [ 0.52] | corr= [ 0.66] | corr= [ 0.47] |
=====
|g|= 0.0977 +/- 0.0251 | |g|= 0.1424 +/- 0.0200 | |g|= 0.1051 +/- 0.0061 |
arg(g)/pi= 0.1469 +/- 0.0498 | arg(g)/pi= 0.1902 +/- 0.0268 | arg(g)/pi= 0.6124 +/- 0.0296 |
=====
g_re= 0.0875 +/- 0.0224 | g_re= 0.1177 +/- 0.0134 | g_re= -0.0363 +/- 0.0095 |
g_im= 0.0435 +/- 0.0191 | g_im= 0.0801 +/- 0.0191 | g_im= 0.0986 +/- 0.0064 |
corr= [ 0.46] | corr= [ 0.68] | corr= [ 0.26] |
=====
*****

*****
JP=0+ || eta:eta/1^S_0[+] kaon:kaon/1^S_0[-] pi:pi/1^S_0[+]

sqrt(s)_pole = (0.11062 +/- 0.031638)
+ (i/2)*(+2.8356e-17 +/- 8.4787e-15) [ 0.02]

=====
eta:eta/1^S_0 | kaon:kaon/1^S_0 | pi:pi/1^S_0 |
=====
k_re= 0.0000 +/- 0.0000 | k_re= -0.0000 +/- 0.0000 | k_re= 0.0000 +/- 0.0000 |
k_im= 0.0876 +/- 0.0100 | k_im= -0.0797 +/- 0.0110 | k_im= 0.0413 +/- 0.0212 |
corr= [-0.01] | corr= [-0.01] | corr= [-0.01] |
=====
|g|= 0.0760 +/- 0.0182 | |g|= 0.0201 +/- 0.0077 | |g|= 0.0702 +/- 0.0283 |
arg(g)/pi= 0.0000 +/- 0.0000 | arg(g)/pi= -0.0000 +/- 0.0000 | arg(g)/pi= -0.0000 +/- 0.0000 |
=====
g_re= 0.0760 +/- 0.0182 | g_re= 0.0201 +/- 0.0077 | g_re= 0.0702 +/- 0.0283 |
g_im= 0.0000 +/- 0.0000 | g_im= -0.0000 +/- 0.0000 | g_im= -0.0000 +/- 0.0000 |
corr= [-1.00] | corr= [-0.61] | corr= [-0.00] |
=====
*****

*****
JP=0+ || eta:eta/1^S_0[+] kaon:kaon/1^S_0[-] pi:pi/1^S_0[-]

sqrt(s)_pole = ( 0.1575 +/- 0.027535)
+ (i/2)*(-0.10551 +/- 0.041861) [ 0.86]

=====
eta:eta/1^S_0 | kaon:kaon/1^S_0 | pi:pi/1^S_0 |
=====
k_re= -0.0269 +/- 0.0045 | k_re= 0.0300 +/- 0.0052 | k_re= 0.0498 +/- 0.0124 |
k_im= 0.0772 +/- 0.0170 | k_im= -0.0693 +/- 0.0183 | k_im= -0.0417 +/- 0.0183 |
corr= [ 0.10] | corr= [ 0.33] | corr= [ 0.85] |
=====
|g|= 0.1262 +/- 0.0233 | |g|= 0.0593 +/- 0.0091 | |g|= 0.1344 +/- 0.0141 |
arg(g)/pi= -0.0714 +/- 0.1015 | arg(g)/pi= -0.3441 +/- 0.1427 | arg(g)/pi= 0.5071 +/- 0.0333 |
=====
g_re= 0.1231 +/- 0.0287 | g_re= 0.0279 +/- 0.0252 | g_re= -0.0030 +/- 0.0140 |
g_im= -0.0281 +/- 0.0366 | g_im= -0.0523 +/- 0.0124 | g_im= 0.1344 +/- 0.0141 |
corr= [ 0.67] | corr= [ 0.68] | corr= [ 0.09] |
=====
*****

*****
JP=0+ || eta:eta/1^S_0[-] kaon:kaon/1^S_0[+] pi:pi/1^S_0[+]

sqrt(s)_pole = ( 0.1771 +/- 0.017475)
+ (i/2)*(-0.093898 +/- 0.017647) [-0.48]

=====
eta:eta/1^S_0 | kaon:kaon/1^S_0 | pi:pi/1^S_0 |
=====
k_re= 0.0312 +/- 0.0097 | k_re= -0.0357 +/- 0.0110 | k_re= -0.0608 +/- 0.0119 |
k_im= -0.0665 +/- 0.0073 | k_im= 0.0582 +/- 0.0071 | k_im= 0.0342 +/- 0.0049 |
corr= [ 0.68] | corr= [ 0.63] | corr= [-0.07] |
=====
|g|= 0.0844 +/- 0.0154 | |g|= 0.1636 +/- 0.0195 | |g|= 0.0822 +/- 0.0079 |
arg(g)/pi= 0.3351 +/- 0.0491 | arg(g)/pi= 0.2374 +/- 0.0339 | arg(g)/pi= -0.1033 +/- 0.0573 |
=====
g_re= 0.0418 +/- 0.0130 | g_re= 0.1201 +/- 0.0113 | g_re= 0.0779 +/- 0.0110 |
g_im= 0.0733 +/- 0.0154 | g_im= 0.1110 +/- 0.0236 | g_im= -0.0262 +/- 0.0126 |
corr= [ 0.10] | corr= [ 0.21] | corr= [ 0.75] |
=====
*****

*****
JP=0+ || eta:eta/1^S_0[-] kaon:kaon/1^S_0[+] pi:pi/1^S_0[-]

sqrt(s)_pole = (0.12816 +/- 0.0062633)
+ (i/2)*(+3.7033e-18 +/- 1.1069e-15) [-0.01]

=====
eta:eta/1^S_0 | kaon:kaon/1^S_0 | pi:pi/1^S_0 |
=====
k_re= -0.0000 +/- 0.0000 | k_re= 0.0000 +/- 0.0000 | k_re= -0.0000 +/- 0.0000 |
k_im= -0.0815 +/- 0.0025 | k_im= 0.0728 +/- 0.0028 | k_im= -0.0257 +/- 0.0078 |
corr= [ 0.01] | corr= [ 0.01] | corr= [ 0.01] |
=====
|g|= 0.0387 +/- 0.0097 | |g|= 0.0095 +/- 0.0236 | |g|= 0.0987 +/- 0.0069 |
arg(g)/pi= 0.5000 +/- 0.0000 | arg(g)/pi= 0.5000 +/- 0.0000 | arg(g)/pi= -0.5000 +/- 0.0000 |
=====
g_re= 0.0000 +/- 0.0000 | g_re= -0.0000 +/- 0.0000 | g_re= 0.0000 +/- 0.0000 |
g_im= 0.0387 +/- 0.0097 | g_im= 0.0095 +/- 0.0236 | g_im= -0.0987 +/- 0.0069 |
corr= [-1.00] | corr= [-0.98] | corr= [-0.34] |
=====
*****

```

```

*****
JP=0+  ||  eta:eta/1^S_0[-] kaon:kaon/1^S_0[+] pi:pi/1^S_0[-]

sqrt(s)_pole = (0.21351 +/- 0.011673)
               + (i/2)*(-0.072229 +/- 0.02501) [-0.07]

=====
eta:eta/1^S_0 | kaon:kaon/1^S_0 | pi:pi/1^S_0 |
=====
k_re= 0.0458 +/- 0.0107 | k_re= -0.0542 +/- 0.0101 | k_re= 0.0827 +/- 0.0074 |
k_im= -0.0421 +/- 0.0103 | k_im= 0.0356 +/- 0.0101 | k_im= -0.0233 +/- 0.0078 |
corr= [-0.10] | corr= [-0.10] | corr= [-0.09] |
=====
|g|= 0.0952 +/- 0.0175 | |g|= 0.1895 +/- 0.0213 | |g|= 0.1060 +/- 0.0109 |
arg(g)/pi= 0.2040 +/- 0.0585 | arg(g)/pi= 0.2628 +/- 0.0271 | arg(g)/pi= 0.6893 +/- 0.0416 |
=====
g_re= 0.0763 +/- 0.0196 | g_re= 0.1285 +/- 0.0151 | g_re= -0.0594 +/- 0.0108 |
g_im= 0.0569 +/- 0.0151 | g_im= 0.1393 +/- 0.0221 | g_im= 0.0878 +/- 0.0139 |
corr= [-0.08] | corr= [ 0.26] | corr= [ 0.36] |
=====

```

```

*****
JP=0+  ||  eta:eta/1^S_0[-] kaon:kaon/1^S_0[-] pi:pi/1^S_0[-]

sqrt(s)_pole = (0.12839 +/- 0.0060217)
               + (i/2)*(+2.2404e-14 +/- 6.699e-12) [-0.02]

=====
eta:eta/1^S_0 | kaon:kaon/1^S_0 | pi:pi/1^S_0 |
=====
k_re= -0.0000 +/- 0.0000 | k_re= -0.0000 +/- 0.0000 | k_re= -0.0000 +/- 0.0000 |
k_im= -0.0814 +/- 0.0024 | k_im= -0.0727 +/- 0.0027 | k_im= -0.0255 +/- 0.0076 |
corr= [ 0.02] | corr= [ 0.02] | corr= [ 0.02] |
=====
|g|= 0.0369 +/- 0.0080 | |g|= 0.0026 +/- 0.0061 | |g|= 0.1014 +/- 0.0069 |
arg(g)/pi= 0.5000 +/- 0.0000 | arg(g)/pi= 0.5000 +/- 0.0000 | arg(g)/pi= -0.5000 +/- 0.0000 |
=====
g_re= 0.0000 +/- 0.0000 | g_re= -0.0000 +/- 0.0000 | g_re= 0.0000 +/- 0.0000 |
g_im= 0.0369 +/- 0.0080 | g_im= 0.0026 +/- 0.0061 | g_im= -0.1014 +/- 0.0069 |
corr= [-1.00] | corr= [-0.98] | corr= [ 0.28] |
=====

```

# k\_sigma\_pole\_cccccc

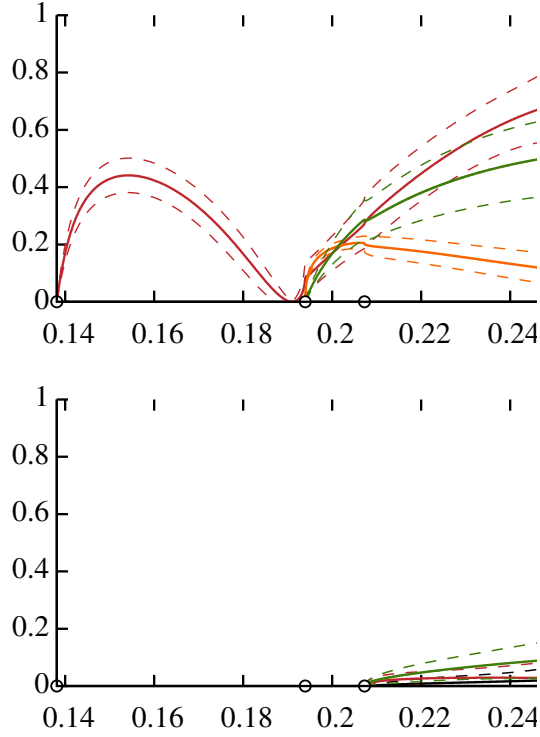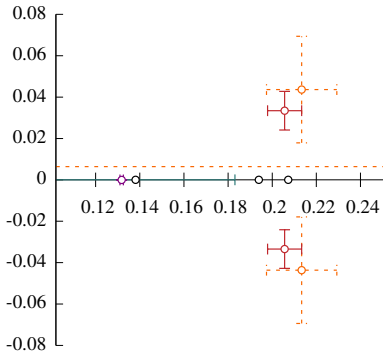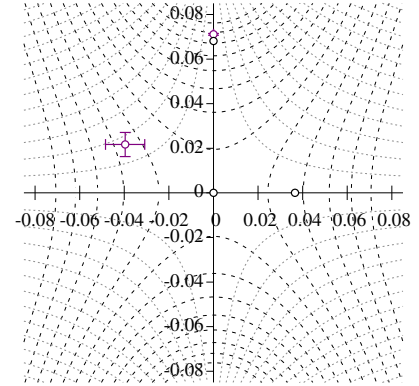

## parameter values

minimised with chisq/nDoF = 43.01 / (57 - 10) = 0.92

|                                                   |                        |      |       |       |       |       |       |       |       |       |       |
|---------------------------------------------------|------------------------|------|-------|-------|-------|-------|-------|-------|-------|-------|-------|
| JPO+_g_eta:eta/1^S_0_pole0                        | -0.18420 +/- 0.2049    | 1.00 | 0.54  | -0.59 | -0.99 | 0.98  | 0.96  | 0.57  | -0.08 | -0.48 | 0.01  |
| JPO+_g_kaon:kaon/1^S_0_pole0                      | 0.35487 +/- 0.063106   | 1.00 | -0.05 | -0.56 | 0.47  | 0.55  | 0.97  | 0.21  | -0.53 | -0.05 |       |
| JPO+_g_pi:pi/1^S_0_pole0                          | 0.20742 +/- 0.02861    |      | 1.00  | 0.57  | -0.60 | -0.62 | -0.10 | 0.62  | 0.61  | 0.10  |       |
| JPO+_gamma_eta:eta/1^S_0 eta:eta/1^S_0_order0     | 1.1320 +/- 2.4267      |      |       | 1.00  | -0.98 | -0.59 | -0.97 | -0.59 | 0.08  | 0.50  | -0.01 |
| JPO+_gamma_eta:eta/1^S_0 kaon:kaon/1^S_0_order0   | -2.3389 +/- 2.2518     |      |       |       | 1.00  | 0.94  | 0.52  | -0.11 | -0.46 | 0.01  |       |
| JPO+_gamma_eta:eta/1^S_0 pi:pi/1^S_0_order0       | -0.40581 +/- 1.5209    |      |       |       |       | 1.00  | 0.58  | -0.16 | -0.60 | -0.02 |       |
| JPO+_gamma_kaon:kaon/1^S_0 kaon:kaon/1^S_0_order0 | 4.0875 +/- 1.4686      |      |       |       |       |       | 1.00  | 0.27  | -0.48 | 0.01  |       |
| JPO+_gamma_kaon:kaon/1^S_0 pi:pi/1^S_0_order0     | 0.19605 +/- 0.48623    |      |       |       |       |       |       | 1.00  | 0.67  | 0.23  |       |
| JPO+_gamma_pi:pi/1^S_0 pi:pi/1^S_0_order0         | -0.41101 +/- 0.65552   |      |       |       |       |       |       |       | 1.00  | 0.19  |       |
| JPO+_m_pole0                                      | 0.13181 +/- 0.00074754 |      |       |       |       |       |       |       |       | 1.00  |       |

## pole singularities

\*\*\*\*\*  
JP=0+ || eta:eta/1^S\_0[+] kaon:kaon/1^S\_0[+] pi:pi/1^S\_0[+]

sqrt(s)\_pole = (0.13181 +/- 0.00075932)  
+ (i/2)\*(-6.9527e-15 +/- 2.3792e-12) [-0.10]

| eta:eta/1^S_0                | kaon:kaon/1^S_0              | pi:pi/1^S_0                  |
|------------------------------|------------------------------|------------------------------|
| k_re= -0.0000 +/- 0.0000     | k_re= -0.0000 +/- 0.0000     | k_re= -0.0000 +/- 0.0000     |
| k_im= 0.0800 +/- 0.0003      | k_im= 0.0711 +/- 0.0004      | k_im= 0.0206 +/- 0.0012      |
| corr= [ 0.10]                | corr= [ 0.10]                | corr= [ 0.10]                |
| g = 0.0814 +/- 0.0882        | g = 0.1569 +/- 0.0344        | g = 0.0917 +/- 0.0047        |
| arg(g)/pi= 0.0000 +/- 0.0000 | arg(g)/pi= 1.0000 +/- 0.0000 | arg(g)/pi= 1.0000 +/- 0.0000 |
| g_re= 0.0814 +/- 0.0882      | g_re= -0.1569 +/- 0.0344     | g_re= -0.0917 +/- 0.0047     |
| g_im= 0.0000 +/- 0.0000      | g_im= 0.0000 +/- 0.0000      | g_im= 0.0000 +/- 0.0000      |
| corr= [-1.00]                | corr= [-0.86]                | corr= [ 0.03]                |

\*\*\*\*\*

\*\*\*\*\*  
JP=0+ || eta:eta/1^S\_0[+] kaon:kaon/1^S\_0[+] pi:pi/1^S\_0[-]

sqrt(s)\_pole = ( 0.2056 +/- 0.0077181)  
+ (i/2)\*(-0.033423 +/- 0.0093446) [-0.22]

| eta:eta/1^S_0                | kaon:kaon/1^S_0               | pi:pi/1^S_0                   |
|------------------------------|-------------------------------|-------------------------------|
| k_re= -0.0273 +/- 0.0087     | k_re= -0.0396 +/- 0.0088      | k_re= 0.0765 +/- 0.0052       |
| k_im= 0.0314 +/- 0.0070      | k_im= 0.0217 +/- 0.0054       | k_im= -0.0112 +/- 0.0031      |
| corr= [ 0.47]                | corr= [ 0.24]                 | corr= [-0.15]                 |
| g = 0.0664 +/- 0.0469        | g = 0.1725 +/- 0.0366         | g = 0.1248 +/- 0.0331         |
| arg(g)/pi= 0.2636 +/- 0.1627 | arg(g)/pi= -0.7142 +/- 0.0612 | arg(g)/pi= -0.3273 +/- 0.0647 |
| g_re= 0.0449 +/- 0.0509      | g_re= -0.1075 +/- 0.0240      | g_re= 0.0644 +/- 0.0356       |
| g_im= 0.0489 +/- 0.0277      | g_im= -0.1349 +/- 0.0431      | g_im= -0.1069 +/- 0.0217      |
| corr= [ 0.43]                | corr= [-0.02]                 | corr= [-0.60]                 |

\*\*\*\*\*

JP=0+ || eta:eta/1^S\_0[+] kaon:kaon/1^S\_0[-] pi:pi/1^S\_0[-]

sqrt(s)\_pole = (0.07985 +/- 0.10329)  
+ (i/2)\*(+1.0098e-14 +/- 9.8776e-13) [ 0.02]

| eta:eta/1^S_0                | kaon:kaon/1^S_0              | pi:pi/1^S_0                   |
|------------------------------|------------------------------|-------------------------------|
| k_re= 0.0000 +/- 0.0000      | k_re= -0.0000 +/- 0.0000     | k_re= -0.0000 +/- 0.0000      |
| k_im= 0.0956 +/- 0.0214      | k_im= -0.0883 +/- 0.0231     | k_im= -0.0562 +/- 0.0363      |
| corr= [-0.02]                | corr= [-0.02]                | corr= [-0.02]                 |
| g = 0.0258 +/- 0.0201        | g = 0.0165 +/- 0.0897        | g = 0.0641 +/- 0.3458         |
| arg(g)/pi= 0.5000 +/- 0.0003 | arg(g)/pi= 0.5000 +/- 0.0132 | arg(g)/pi= -0.5000 +/- 0.0131 |
| g_re= 0.0000 +/- 0.0000      | g_re= 0.0000 +/- 0.0007      | g_re= -0.0000 +/- 0.0026      |
| g_im= 0.0258 +/- 0.0201      | g_im= 0.0165 +/- 0.0897      | g_im= -0.0641 +/- 0.3458      |
| corr= [-0.42]                | corr= [-0.51]                | corr= [-0.51]                 |

\*\*\*\*\*

JP=0+ || eta:eta/1^S\_0[-] kaon:kaon/1^S\_0[+] pi:pi/1^S\_0[-]

sqrt(s)\_pole = (0.21334 +/- 0.01591)  
+ (i/2)\*(-0.043642 +/- 0.025732) [-0.33]

| eta:eta/1^S_0                | kaon:kaon/1^S_0               | pi:pi/1^S_0                   |
|------------------------------|-------------------------------|-------------------------------|
| k_re= 0.0381 +/- 0.0186      | k_re= -0.0491 +/- 0.0166      | k_re= 0.0818 +/- 0.0104       |
| k_im= -0.0306 +/- 0.0125     | k_im= 0.0237 +/- 0.0113       | k_im= -0.0142 +/- 0.0081      |
| corr= [ 0.06]                | corr= [-0.12]                 | corr= [-0.30]                 |
| g = 0.0704 +/- 0.0687        | g = 0.1934 +/- 0.0466         | g = 0.1324 +/- 0.0330         |
| arg(g)/pi= 0.2230 +/- 0.2338 | arg(g)/pi= -0.7006 +/- 0.1243 | arg(g)/pi= -0.2694 +/- 0.1288 |
| g_re= 0.0538 +/- 0.0507      | g_re= -0.1139 +/- 0.0529      | g_re= 0.0877 +/- 0.0570       |
| g_im= 0.0454 +/- 0.0695      | g_im= -0.1563 +/- 0.0712      | g_im= -0.0991 +/- 0.0265      |
| corr= [ 0.35]                | corr= [-0.59]                 | corr= [ 0.49]                 |



# k\_sigma\_pole\_lccccc

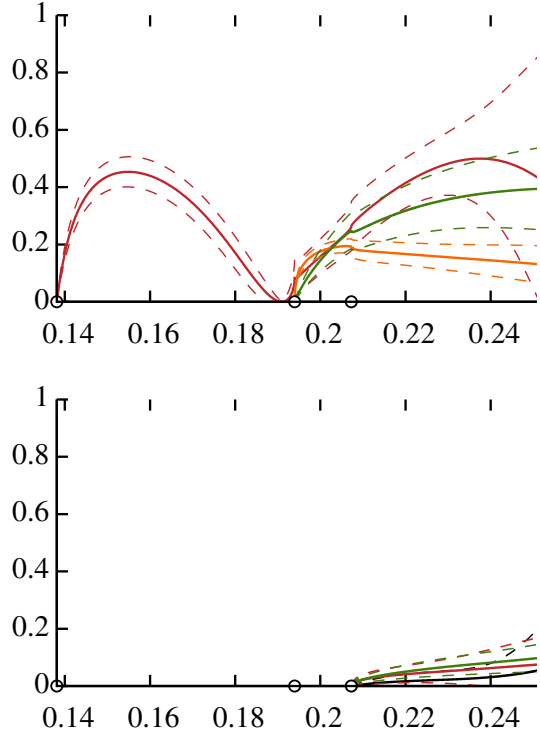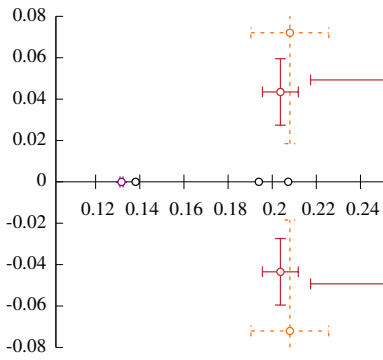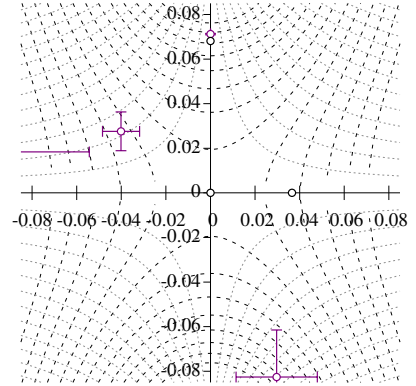

## parameter values

minimised with chisq/nDoF = 42.09 / (57 - 11) = 0.92

|                                               |                        |      |       |       |       |       |       |      |       |       |       |      |
|-----------------------------------------------|------------------------|------|-------|-------|-------|-------|-------|------|-------|-------|-------|------|
| JPO+_g_eta:eta/1^S_0_pole0                    | -0.23773 +/- 0.17567   | 1.00 | 0.57  | -0.62 | -0.99 | 0.97  | 0.96  | 0.61 | 0.02  | -0.24 | -0.23 | 0.07 |
| JPO+_g_kaon:kaon/1^S_0_pole0                  | 0.32291 +/- 0.055163   | 1.00 | -0.10 | -0.59 | 0.46  | 0.54  | 0.96  | 0.35 | -0.27 | -0.13 | 0.01  |      |
| JPO+_g_pi:pi/1^S_0_pole0                      | 0.20469 +/- 0.027226   | 1.00 | 0.61  | -0.65 | -0.68 | -0.17 | 0.49  | 0.46 | 0.15  | 0.06  |       |      |
| JPO+_gamma_eta:eta/1^S_0_eta:eta/1^S_0_order0 | 1.8785 +/- 2.6217      | 1.00 | -0.98 | -0.97 | -0.63 | -0.04 | 0.24  | 0.23 | -0.07 |       |       |      |
| JPO+_gamma_eta:eta/1^S_0 kaon:kaon/1^S_0_orde | -2.8635 +/- 1.6516     | 1.00 | 0.94  | 0.52  | -0.05 | -0.20 | -0.26 | 0.07 |       |       |       |      |
| JPO+_gamma_eta:eta/1^S_0 pi:pi/1^S_0_order0   | -0.70754 +/- 1.2603    | 1.00 | 0.57  | -0.05 | -0.35 | -0.20 | 0.04  |      |       |       |       |      |
| JPO+_gamma_kaon:kaon/1^S_0 kaon:kaon/1^S_0_or | 3.2928 +/- 1.2475      | 1.00 | 0.39  | -0.22 | -0.16 | 0.07  |       |      |       |       |       |      |
| JPO+_gamma_kaon:kaon/1^S_0 pi:pi/1^S_0_order0 | 0.16769 +/- 0.42788    | 1.00 | 0.39  | 0.21  | 0.19  |       |       |      |       |       |       |      |
| JPO+_gamma_pi:pi/1^S_0 pi:pi/1^S_0_order0     | -0.84937 +/- 0.58298   |      |       |       |       |       |       |      |       |       |       |      |
| JPO+_gamma_pi:pi/1^S_0 pi:pi/1^S_0_order1     | 0.67490 +/- 0.49776    |      |       |       |       |       |       |      |       |       |       |      |
| JPO+_m_pole0                                  | 0.13173 +/- 0.00074613 |      |       |       |       |       |       |      |       |       |       |      |
| JPO+_gamma_eta:eta/1^S_0 eta:eta/1^S_0_order1 | 0.0000 +/- 0           |      |       |       |       |       |       |      |       |       |       |      |
| JPO+_gamma_eta:eta/1^S_0 kaon:kaon/1^S_0_orde | 0.0000 +/- 0           |      |       |       |       |       |       |      |       |       |       |      |
| JPO+_gamma_eta:eta/1^S_0 pi:pi/1^S_0_order1   | 0.0000 +/- 0           |      |       |       |       |       |       |      |       |       |       |      |
| JPO+_gamma_kaon:kaon/1^S_0 kaon:kaon/1^S_0_or | 0.0000 +/- 0           |      |       |       |       |       |       |      |       |       |       |      |
| JPO+_gamma_kaon:kaon/1^S_0 pi:pi/1^S_0_order1 | 0.0000 +/- 0           |      |       |       |       |       |       |      |       |       |       |      |

## pole singularities

\*\*\*\*\*  
JP=0+ || eta:eta/1^S\_0[+] kaon:kaon/1^S\_0[+] pi:pi/1^S\_0[+]

sqrt(s)\_pole = (0.13173 +/- 0.00070979)  
+ (i/2)\*(-8.5784e-15 +/- 1.718e-12) [ 0.43]

| eta:eta/1^S_0                | kaon:kaon/1^S_0              | pi:pi/1^S_0                  |
|------------------------------|------------------------------|------------------------------|
| k_re= -0.0000 +/- 0.0000     | k_re= -0.0000 +/- 0.0000     | k_re= -0.0000 +/- 0.0000     |
| k_im= 0.0800 +/- 0.0003      | k_im= 0.0712 +/- 0.0003      | k_im= 0.0208 +/- 0.0011      |
| corr= [-0.43]                | corr= [-0.43]                | corr= [-0.43]                |
| g = 0.1064 +/- 0.0710        | g = 0.1445 +/- 0.0321        | g = 0.0916 +/- 0.0045        |
| arg(g)/pi= 0.0000 +/- 0.0000 | arg(g)/pi= 1.0000 +/- 0.0000 | arg(g)/pi= 1.0000 +/- 0.0000 |
| g_re= 0.1064 +/- 0.0710      | g_re= -0.1445 +/- 0.0321     | g_re= -0.0916 +/- 0.0045     |
| g_im= 0.0000 +/- 0.0000      | g_im= 0.0000 +/- 0.0000      | g_im= 0.0000 +/- 0.0000      |
| corr= [-1.00]                | corr= [-0.91]                | corr= [-0.10]                |

```

*****
JP=0+ || eta:eta/1^S_0[+] kaon:kaon/1^S_0[+] pi:pi/1^S_0[-]

sqrt(s)_pole = (0.20371 +/- 0.0081359)
               + (i/2)*(-0.043457 +/- 0.016059) [ 0.07]

eta:eta/1^S_0 | kaon:kaon/1^S_0 | pi:pi/1^S_0 |
=====|=====|=====|
k_re= -0.0298 +/- 0.0084 | k_re= -0.0401 +/- 0.0083 | k_re= 0.0755 +/- 0.0054 |
k_im= 0.0371 +/- 0.0090 | k_im= 0.0276 +/- 0.0087 | k_im= -0.0147 +/- 0.0054 |
corr= [ 0.02] | corr= [ 0.05] | corr= [ 0.07] |
=====|=====|=====|
|g|= 0.0803 +/- 0.0424 | |g|= 0.1867 +/- 0.0397 | |g|= 0.1445 +/- 0.0444 |
arg(g)/pi= 0.2104 +/- 0.1260 | arg(g)/pi= -0.7778 +/- 0.0873 | arg(g)/pi= -0.4005 +/- 0.1068 |
-----|-----|-----|
g_re= 0.0634 +/- 0.0485 | g_re= -0.1430 +/- 0.0474 | g_re= 0.0444 +/- 0.0455 |
g_im= 0.0493 +/- 0.0214 | g_im= -0.1200 +/- 0.0442 | g_im= -0.1375 +/- 0.0474 |
corr= [ 0.16] | corr= [-0.27] | corr= [ 0.21] |
=====|=====|=====|
*****

*****
JP=0+ || eta:eta/1^S_0[+] kaon:kaon/1^S_0[+] pi:pi/1^S_0[-]

sqrt(s)_pole = (0.25878 +/- 0.041399)
               + (i/2)*(-0.049251 +/- 0.069505) [-0.78]

eta:eta/1^S_0 | kaon:kaon/1^S_0 | pi:pi/1^S_0 |
=====|=====|=====|
k_re= -0.0791 +/- 0.0360 | k_re= -0.0867 +/- 0.0324 | k_re= 0.1097 +/- 0.0249 |
k_im= 0.0201 +/- 0.0236 | k_im= 0.0184 +/- 0.0227 | k_im= -0.0145 +/- 0.0197 |
corr= [-0.75] | corr= [-0.76] | corr= [-0.78] |
=====|=====|=====|
|g|= 0.0490 +/- 0.0491 | |g|= 0.1195 +/- 0.0512 | |g|= 0.1750 +/- 0.0792 |
arg(g)/pi= 0.2975 +/- 0.5108 | arg(g)/pi= -0.1869 +/- 0.2336 | arg(g)/pi= 0.2505 +/- 0.0976 |
-----|-----|-----|
g_re= 0.0291 +/- 0.0817 | g_re= 0.0995 +/- 0.0743 | g_re= 0.1236 +/- 0.0498 |
g_im= 0.0395 +/- 0.0440 | g_im= -0.0662 +/- 0.0693 | g_im= 0.1240 +/- 0.0817 |
corr= [-0.35] | corr= [ 0.56] | corr= [ 0.42] |
=====|=====|=====|
*****

*****
JP=0+ || eta:eta/1^S_0[+] kaon:kaon/1^S_0[-] pi:pi/1^S_0[-]

sqrt(s)_pole = (0.13763 +/- 0.055083)
               + (i/2)*(-0.14242 +/- 0.061371) [ 0.22]

eta:eta/1^S_0 | kaon:kaon/1^S_0 | pi:pi/1^S_0 |
=====|=====|=====|
k_re= -0.0274 +/- 0.0165 | k_re= 0.0297 +/- 0.0182 | k_re= 0.0434 +/- 0.0265 |
k_im= 0.0896 +/- 0.0202 | k_im= -0.0826 +/- 0.0211 | k_im= -0.0564 +/- 0.0217 |
corr= [ 0.53] | corr= [ 0.55] | corr= [ 0.53] |
=====|=====|=====|
|g|= 0.0768 +/- 0.1549 | |g|= 0.0473 +/- 0.0149 | |g|= 0.1189 +/- 0.0353 |
arg(g)/pi= 0.2105 +/- 0.6263 | arg(g)/pi= -0.4706 +/- 0.1242 | arg(g)/pi= 0.5390 +/- 0.0402 |
-----|-----|-----|
g_re= 0.0606 +/- 0.2119 | g_re= 0.0044 +/- 0.0191 | g_re= -0.0145 +/- 0.0154 |
g_im= 0.0472 +/- 0.0436 | g_im= -0.0471 +/- 0.0142 | g_im= 0.1180 +/- 0.0351 |
corr= [-0.53] | corr= [-0.41] | corr= [-0.21] |
=====|=====|=====|
*****

*****
JP=0+ || eta:eta/1^S_0[-] kaon:kaon/1^S_0[+] pi:pi/1^S_0[-]

sqrt(s)_pole = (0.20799 +/- 0.017616)
               + (i/2)*(-0.072048 +/- 0.053587) [ 0.05]

eta:eta/1^S_0 | kaon:kaon/1^S_0 | pi:pi/1^S_0 |
=====|=====|=====|
k_re= 0.0419 +/- 0.0180 | k_re= -0.0499 +/- 0.0164 | k_re= 0.0792 +/- 0.0112 |
k_im= -0.0447 +/- 0.0209 | k_im= 0.0375 +/- 0.0216 | k_im= -0.0236 +/- 0.0171 |
corr= [-0.37] | corr= [-0.31] | corr= [-0.06] |
=====|=====|=====|
|g|= 0.0760 +/- 0.0741 | |g|= 0.2198 +/- 0.0884 | |g|= 0.1552 +/- 0.0555 |
arg(g)/pi= 0.0298 +/- 0.2220 | arg(g)/pi= -0.8310 +/- 0.1350 | arg(g)/pi= -0.3889 +/- 0.1154 |
-----|-----|-----|
g_re= 0.0757 +/- 0.0734 | g_re= -0.1896 +/- 0.0877 | g_re= 0.0531 +/- 0.0563 |
g_im= 0.0071 +/- 0.0540 | g_im= -0.1113 +/- 0.0939 | g_im= -0.1458 +/- 0.0555 |
corr= [ 0.17] | corr= [-0.02] | corr= [ 0.01] |
=====|=====|=====|
*****

```

# k\_sigma\_pole\_ccclcc

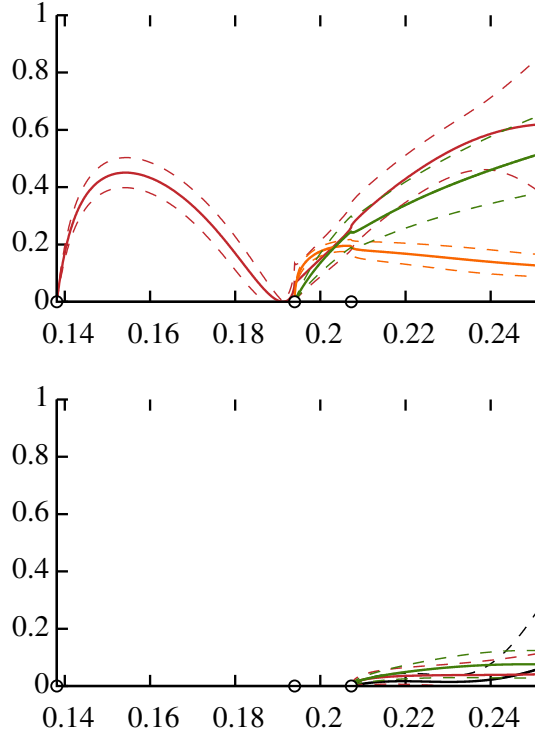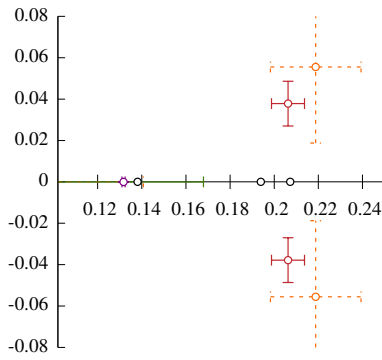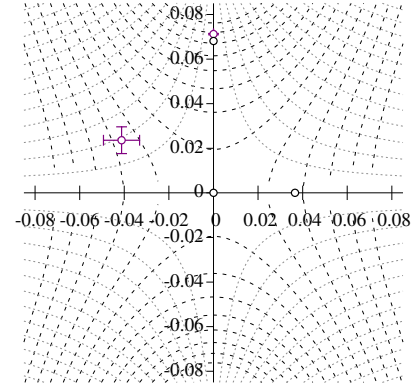

## parameter values

minimised with chisq/nDoF = 42.02 / (57 - 11) = 0.91

|                                               |                        |       |       |       |       |       |       |       |      |       |       |       |
|-----------------------------------------------|------------------------|-------|-------|-------|-------|-------|-------|-------|------|-------|-------|-------|
| JPO+_g_eta:eta/1^S_0_pole0                    | -0.26840 +/- 0.17387   | 1.00  | 0.57  | -0.73 | -0.99 | 0.88  | 0.95  | 0.29  | 0.20 | 0.10  | -0.53 | -0.03 |
| JPO+_g_kaon:kaon/1^S_0_pole0                  | 0.21784 +/- 0.072849   | 1.00  | -0.16 | -0.58 | 0.24  | 0.54  | 0.53  | 0.26  | 0.45 | -0.50 | -0.02 |       |
| JPO+_g_pi:pi/1^S_0_pole0                      | 0.19244 +/- 0.029297   | 1.00  | 0.72  | -0.75 | -0.76 | -0.08 | -0.10 | 0.31  | 0.64 | 0.11  |       |       |
| JPO+_gamma_eta:eta/1^S_0_eta:eta/1^S_0_order0 | 2.2975 +/- 2.8829      | 1.00  | -0.89 | -0.96 | -0.28 | -0.22 | -0.10 | 0.54  | 0.03 |       |       |       |
| JPO+_gamma_eta:eta/1^S_0 kaon:kaon/1^S_0_orde | -2.2210 +/- 1.0807     | 1.00  | 0.86  | 0.06  | 0.20  | -0.15 | -0.42 | -0.05 |      |       |       |       |
| JPO+_gamma_eta:eta/1^S_0 pi:pi/1^S_0_order0   | -0.77240 +/- 1.2384    | 1.00  | 0.22  | 0.24  | 0.00  | -0.65 | -0.06 |       |      |       |       |       |
| JPO+_gamma_kaon:kaon/1^S_0 kaon:kaon/1^S_0_or | -1.6187 +/- 1.3914     | 1.00  | -0.65 | 0.52  | -0.16 | 0.03  |       |       |      |       |       |       |
| JPO+_gamma_kaon:kaon/1^S_0 kaon:kaon/1^S_0_or | 2.4137 +/- 0.96671     | 1.00  | -0.14 | -0.23 | -0.00 |       |       |       |      |       |       |       |
| JPO+_gamma_kaon:kaon/1^S_0 pi:pi/1^S_0_order0 | -0.70162 +/- 0.40644   | 1.00  | 0.42  | 0.19  |       |       |       |       |      |       |       |       |
| JPO+_gamma_pi:pi/1^S_0 pi:pi/1^S_0_order0     | -0.25036 +/- 0.52797   | 1.00  | 0.18  |       |       |       |       |       |      |       |       |       |
| JPO+_m_pole0                                  | 0.13173 +/- 0.00074241 | 1.00  |       |       |       |       |       |       |      |       |       |       |
| JPO+_gamma_eta:eta/1^S_0 eta:eta/1^S_0_order1 | 0.0000 +/- 0           | FIXED |       |       |       |       |       |       |      |       |       |       |
| JPO+_gamma_eta:eta/1^S_0 kaon:kaon/1^S_0_orde | 0.0000 +/- 0           | FIXED |       |       |       |       |       |       |      |       |       |       |
| JPO+_gamma_eta:eta/1^S_0 pi:pi/1^S_0_order1   | 0.0000 +/- 0           | FIXED |       |       |       |       |       |       |      |       |       |       |
| JPO+_gamma_kaon:kaon/1^S_0 pi:pi/1^S_0_order1 | 0.0000 +/- 0           | FIXED |       |       |       |       |       |       |      |       |       |       |
| JPO+_gamma_pi:pi/1^S_0 pi:pi/1^S_0_order1     | 0.0000 +/- 0           | FIXED |       |       |       |       |       |       |      |       |       |       |

## pole singularities

\*\*\*\*\*  
JP=0+ || eta:eta/1^S\_0[+] kaon:kaon/1^S\_0[+] pi:pi/1^S\_0[+]

sqrt(s)\_pole = (0.13173 +/- 0.00071217)  
+ (i/2)\*(-2.3263e-13 +/- 1.4984e-11) [ 0.66]

| eta:eta/1^S_0                | kaon:kaon/1^S_0              | pi:pi/1^S_0                  |
|------------------------------|------------------------------|------------------------------|
| k_re= -0.0000 +/- 0.0000     | k_re= -0.0000 +/- 0.0000     | k_re= -0.0000 +/- 0.0000     |
| k_im= 0.0800 +/- 0.0003      | k_im= 0.0712 +/- 0.0003      | k_im= 0.0208 +/- 0.0011      |
| corr= [-0.66]                | corr= [-0.66]                | corr= [-0.66]                |
| g = 0.1296 +/- 0.0700        | g = 0.1052 +/- 0.0427        | g = 0.0930 +/- 0.0044        |
| arg(g)/pi= 0.0000 +/- 0.0000 | arg(g)/pi= 1.0000 +/- 0.0000 | arg(g)/pi= 1.0000 +/- 0.0000 |
| g_re= 0.1296 +/- 0.0700      | g_re= -0.1052 +/- 0.0427     | g_re= -0.0930 +/- 0.0044     |
| g_im= 0.0000 +/- 0.0000      | g_im= 0.0000 +/- 0.0000      | g_im= 0.0000 +/- 0.0000      |
| corr= [-1.00]                | corr= [-0.92]                | corr= [-0.30]                |

\*\*\*\*\*

```

*****
JP=0+ || eta:eta/1^S_0[+] kaon:kaon/1^S_0[+] pi:pi/1^S_0[-]

sqrt(s)_pole = (0.20626 +/- 0.0074652)
               + (i/2)*(-0.037816 +/- 0.010824) [-0.13]

eta:eta/1^S_0 | kaon:kaon/1^S_0 | pi:pi/1^S_0 |
=====|=====|=====|
k_re= -0.0297 +/- 0.0082 | k_re= -0.0412 +/- 0.0081 | k_re= 0.0771 +/- 0.0050 |
k_im= 0.0328 +/- 0.0070 | k_im= 0.0236 +/- 0.0060 | k_im= -0.0127 +/- 0.0036 |
corr= [ 0.30] | corr= [ 0.16] | corr= [-0.08] |
=====|=====|=====|
|g|= 0.0843 +/- 0.0349 | |g|= 0.1718 +/- 0.0336 | |g|= 0.1339 +/- 0.0345 |
arg(g)/pi= 0.2844 +/- 0.1138 | arg(g)/pi= -0.7451 +/- 0.0528 | arg(g)/pi= -0.3395 +/- 0.0595 |
=====|=====|=====|
g_re= 0.0528 +/- 0.0374 | g_re= -0.1196 +/- 0.0298 | g_re= 0.0647 +/- 0.0327 |
g_im= 0.0657 +/- 0.0270 | g_im= -0.1233 +/- 0.0325 | g_im= -0.1173 +/- 0.0272 |
corr= [ 0.23] | corr= [ 0.16] | corr= [-0.49] |
=====|=====|=====|
*****

```

```

*****
JP=0+ || eta:eta/1^S_0[+] kaon:kaon/1^S_0[-] pi:pi/1^S_0[+]

sqrt(s)_pole = (0.077324 +/- 0.090641)
               + (i/2)*(-2.0303e-13 +/- 4.5604e-11) [ 0.09]

eta:eta/1^S_0 | kaon:kaon/1^S_0 | pi:pi/1^S_0 |
=====|=====|=====|
k_re= -0.0000 +/- 0.0000 | k_re= 0.0000 +/- 0.0000 | k_re= -0.0000 +/- 0.0000 |
k_im= 0.0961 +/- 0.0181 | k_im= -0.0889 +/- 0.0196 | k_im= 0.0571 +/- 0.0305 |
corr= [-0.11] | corr= [-0.11] | corr= [-0.12] |
=====|=====|=====|
|g|= 0.2611 +/- 0.0608 | |g|= 0.0155 +/- 0.0134 | |g|= 0.0570 +/- 0.0296 |
arg(g)/pi= 0.0000 +/- 0.0000 | arg(g)/pi= 1.0000 +/- 0.0000 | arg(g)/pi= 1.0000 +/- 0.0000 |
=====|=====|=====|
g_re= 0.2611 +/- 0.0608 | g_re= -0.0155 +/- 0.0134 | g_re= -0.0570 +/- 0.0296 |
g_im= 0.0000 +/- 0.0000 | g_im= 0.0000 +/- 0.0000 | g_im= 0.0000 +/- 0.0000 |
corr= [-1.00] | corr= [-0.85] | corr= [-0.90] |
=====|=====|=====|
*****

```

```

*****
JP=0+ || eta:eta/1^S_0[+] kaon:kaon/1^S_0[-] pi:pi/1^S_0[-]

sqrt(s)_pole = (0.10933 +/- 0.049539)
               + (i/2)*(-0.11699 +/- 0.11075) [ 0.49]

eta:eta/1^S_0 | kaon:kaon/1^S_0 | pi:pi/1^S_0 |
=====|=====|=====|
k_re= -0.0169 +/- 0.0126 | k_re= 0.0183 +/- 0.0134 | k_re= 0.0274 +/- 0.0178 |
k_im= 0.0943 +/- 0.0205 | k_im= -0.0872 +/- 0.0221 | k_im= -0.0582 +/- 0.0310 |
corr= [-0.25] | corr= [-0.22] | corr= [ 0.04] |
=====|=====|=====|
|g|= 0.2031 +/- 0.0549 | |g|= 0.0338 +/- 0.0103 | |g|= 0.0949 +/- 0.0529 |
arg(g)/pi= 0.0704 +/- 0.1507 | arg(g)/pi= 0.5279 +/- 0.2806 | arg(g)/pi= -0.6934 +/- 0.2989 |
=====|=====|=====|
g_re= 0.1981 +/- 0.0490 | g_re= -0.0030 +/- 0.0301 | g_re= -0.0542 +/- 0.0906 |
g_im= 0.0445 +/- 0.0992 | g_im= 0.0337 +/- 0.0093 | g_im= -0.0779 +/- 0.0503 |
corr= [ 0.12] | corr= [-0.26] | corr= [-0.37] |
=====|=====|=====|
*****

```

```

*****
JP=0+ || eta:eta/1^S_0[-] kaon:kaon/1^S_0[+] pi:pi/1^S_0[+]

sqrt(s)_pole = (0.24325 +/- 0.018233)
               + (i/2)*(-0.089961 +/- 0.12807) [ 0.74]

eta:eta/1^S_0 | kaon:kaon/1^S_0 | pi:pi/1^S_0 |
=====|=====|=====|
k_re= 0.0710 +/- 0.0104 | k_re= -0.0782 +/- 0.0087 | k_re= -0.1012 +/- 0.0088 |
k_im= -0.0385 +/- 0.0498 | k_im= 0.0350 +/- 0.0472 | k_im= 0.0270 +/- 0.0383 |
corr= [-0.46] | corr= [-0.12] | corr= [ 0.58] |
=====|=====|=====|
|g|= 0.1365 +/- 1.4589 | |g|= 0.0893 +/- 0.9938 | |g|= 0.0082 +/- 0.1422 |
arg(g)/pi= -0.4749 +/- 0.2970 | arg(g)/pi= 0.5908 +/- 0.1824 | arg(g)/pi= 0.5127 +/- 1.6784 |
=====|=====|=====|
g_re= 0.0107 +/- 0.1047 | g_re= -0.0251 +/- 0.2591 | g_re= -0.0003 +/- 0.0403 |
g_im= -0.1361 +/- 1.4607 | g_im= 0.0857 +/- 0.9608 | g_im= 0.0082 +/- 0.1431 |
corr= [-0.33] | corr= [-0.98] | corr= [ 0.49] |
=====|=====|=====|
*****

```

```

*****
JP=0+ || eta:eta/1^S_0[-] kaon:kaon/1^S_0[+] pi:pi/1^S_0[-]

sqrt(s)_pole = ( 0.2188 +/- 0.020541)
               + (i/2)*(-0.0555 +/- 0.036711) [-0.14]

eta:eta/1^S_0 | kaon:kaon/1^S_0 | pi:pi/1^S_0 |
=====|=====|=====|
k_re= 0.0461 +/- 0.0205 | k_re= -0.0558 +/- 0.0187 | k_re= 0.0856 +/- 0.0131 |
k_im= -0.0330 +/- 0.0172 | k_im= 0.0272 +/- 0.0157 | k_im= -0.0177 +/- 0.0115 |
corr= [ 0.01] | corr= [-0.04] | corr= [-0.12] |
=====|=====|=====|
|g|= 0.0986 +/- 0.1009 | |g|= 0.2047 +/- 0.0739 | |g|= 0.1430 +/- 0.0453 |
arg(g)/pi= 0.1465 +/- 0.4302 | arg(g)/pi= -0.7103 +/- 0.1622 | arg(g)/pi= -0.2419 +/- 0.1558 |
=====|=====|=====|
g_re= 0.0884 +/- 0.1001 | g_re= -0.1256 +/- 0.0896 | g_re= 0.1036 +/- 0.0633 |
g_im= 0.0438 +/- 0.1338 | g_im= -0.1616 +/- 0.0912 | g_im= -0.0985 +/- 0.0542 |
=====|=====|=====|

```

```

corr= [-0.13] | corr= [-0.35] | corr= [ 0.42] |
*****

*****
JP=0+ || eta:eta/1^S_0[-] kaon:kaon/1^S_0[+] pi:pi/1^S_0[-]

sqrt(s)_pole = (0.24441 +/- 0.012943)
+ (i/2)*(-0.091676 +/- 0.14974) [ 0.13]

=====
eta:eta/1^S_0 | kaon:kaon/1^S_0 | pi:pi/1^S_0 |
=====
k_re= 0.0720 +/- 0.0186 | k_re= -0.0791 +/- 0.0145 | k_re= 0.1020 +/- 0.0080 |
k_im= -0.0389 +/- 0.0544 | k_im= 0.0354 +/- 0.0524 | k_im= -0.0275 +/- 0.0440 |
corr= [-0.83] | corr= [-0.75] | corr= [-0.30] |
=====
|g|= 0.1589 +/- 0.0718 | |g|= 0.0833 +/- 0.1437 | |g|= 0.0337 +/- 0.2208 |
arg(g)/pi= -0.4350 +/- 0.1136 | arg(g)/pi= 0.7049 +/- 0.7029 | arg(g)/pi= -0.2231 +/- 1.0135 |
=====
g_re= 0.0322 +/- 0.0559 | g_re= -0.0500 +/- 0.1493 | g_re= 0.0258 +/- 0.1830 |
g_im= -0.1556 +/- 0.0724 | g_im= 0.0667 +/- 0.1795 | g_im= -0.0218 +/- 0.1637 |
corr= [-0.00] | corr= [ 0.31] | corr= [-0.61] |
=====

*****
JP=0+ || eta:eta/1^S_0[-] kaon:kaon/1^S_0[-] pi:pi/1^S_0[-]

sqrt(s)_pole = (0.080578 +/- 0.060153)
+ (i/2)*(+4.2956e-14 +/- 1.2028e-11) [ 0.06]

=====
eta:eta/1^S_0 | kaon:kaon/1^S_0 | pi:pi/1^S_0 |
=====
k_re= -0.0000 +/- 0.0000 | k_re= -0.0000 +/- 0.0000 | k_re= -0.0000 +/- 0.0000 |
k_im= -0.0955 +/- 0.0127 | k_im= -0.0882 +/- 0.0137 | k_im= -0.0560 +/- 0.0216 |
corr= [-0.06] | corr= [-0.06] | corr= [-0.06] |
=====
|g|= 0.0087 +/- 0.0095 | |g|= 0.0176 +/- 0.0197 | |g|= 0.0677 +/- 0.0680 |
arg(g)/pi= 0.5000 +/- 0.0000 | arg(g)/pi= -0.5000 +/- 0.0000 | arg(g)/pi= 0.5000 +/- 0.0000 |
=====
g_re= 0.0000 +/- 0.0000 | g_re= 0.0000 +/- 0.0000 | g_re= -0.0000 +/- 0.0000 |
g_im= 0.0087 +/- 0.0095 | g_im= -0.0176 +/- 0.0197 | g_im= 0.0677 +/- 0.0680 |
corr= [-1.00] | corr= [-0.10] | corr= [ 0.43] |
=====

*****
JP=0+ || eta:eta/1^S_0[-] kaon:kaon/1^S_0[-] pi:pi/1^S_0[-]

sqrt(s)_pole = (0.24672 +/- 0.014889)
+ (i/2)*(-0.10273 +/- 0.14672) [-0.61]

=====
eta:eta/1^S_0 | kaon:kaon/1^S_0 | pi:pi/1^S_0 |
=====
k_re= 0.0749 +/- 0.0240 | k_re= 0.0816 +/- 0.0199 | k_re= 0.1036 +/- 0.0112 |
k_im= -0.0423 +/- 0.0490 | k_im= -0.0388 +/- 0.0480 | k_im= -0.0306 +/- 0.0422 |
corr= [-0.92] | corr= [-0.90] | corr= [-0.78] |
=====
|g|= 0.1239 +/- 0.0457 | |g|= 0.0271 +/- 0.0415 | |g|= 0.0848 +/- 0.0665 |
arg(g)/pi= -0.4492 +/- 0.2296 | arg(g)/pi= -0.5790 +/- 0.2636 | arg(g)/pi= 0.0964 +/- 0.1242 |
=====
g_re= 0.0197 +/- 0.0815 | g_re= -0.0067 +/- 0.0232 | g_re= 0.0810 +/- 0.0662 |
g_im= -0.1223 +/- 0.0585 | g_im= -0.0263 +/- 0.0411 | g_im= 0.0253 +/- 0.0337 |
corr= [ 0.95] | corr= [ 0.23] | corr= [ 0.26] |
=====

```

# k\_sigma\_pole\_llcccc

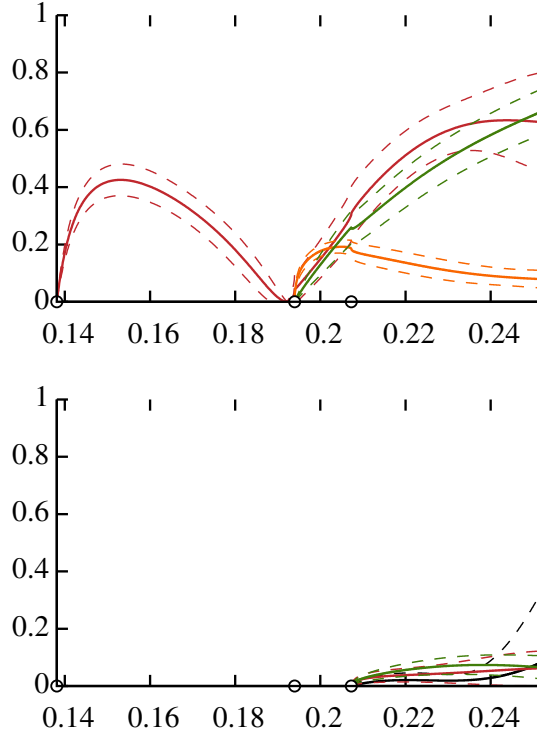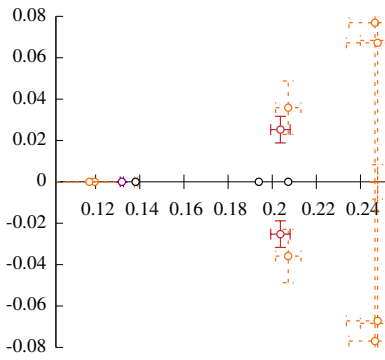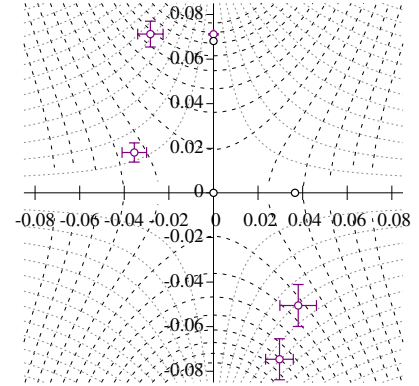

## parameter values

minimised with chisq/nDoF = 40.51 / (57 - 12) = 0.90

|                                               |                        |       |       |       |       |       |       |       |       |       |       |       |       |
|-----------------------------------------------|------------------------|-------|-------|-------|-------|-------|-------|-------|-------|-------|-------|-------|-------|
| JP0+_g_eta:eta/1^S_0_pole0                    | -0.27654 +/- 0.13506   | 1.00  | 0.48  | -0.63 | -0.99 | 0.85  | 0.91  | 0.48  | 0.01  | 0.02  | -0.09 | -0.27 | -0.03 |
| JP0+_g_kaon:kaon/1^S_0_pole0                  | 0.25176 +/- 0.069067   | 1.00  | 0.02  | -0.49 | 0.07  | 0.40  | 0.95  | 0.17  | 0.16  | -0.14 | -0.12 | -0.01 |       |
| JP0+_g_pi:pi/1^S_0_pole0                      | 0.20033 +/- 0.02774    | 1.00  | 0.62  | -0.69 | -0.72 | -0.01 | 0.09  | 0.23  | 0.36  | 0.22  | 0.11  |       |       |
| JP0+_gamma_eta:eta/1^S_0_eta:eta/1^S_0_order0 | 2.5594 +/- 2.3523      | 1.00  | -0.87 | -0.92 | -0.50 | -0.00 | -0.02 | 0.10  | 0.29  | 0.03  |       |       |       |
| JP0+_gamma_eta:eta/1^S_0 kaon:kaon/1^S_0_orde | -2.7417 +/- 1.0656     | 1.00  | 0.83  | 0.10  | -0.11 | -0.07 | -0.03 | -0.31 | -0.07 |       |       |       |       |
| JP0+_gamma_eta:eta/1^S_0 pi:pi/1^S_0_order0   | -0.83787 +/- 1.0448    | 1.00  | 0.38  | 0.04  | -0.14 | -0.24 | -0.32 | -0.09 |       |       |       |       |       |
| JP0+_gamma_kaon:kaon/1^S_0 kaon:kaon/1^S_0_or | 1.8514 +/- 1.269       | 1.00  | 0.17  | 0.22  | -0.09 | -0.10 | 0.05  |       |       |       |       |       |       |
| JP0+_gamma_kaon:kaon/1^S_0 pi:pi/1^S_0_order0 | 2.6856 +/- 0.80636     | 1.00  | -0.78 | 0.33  | -0.14 | 0.06  |       |       |       |       |       |       |       |
| JP0+_gamma_kaon:kaon/1^S_0 pi:pi/1^S_0_order1 | -2.6978 +/- 0.75592    | 1.00  | -0.19 | 0.36  | 0.07  |       |       |       |       |       |       |       |       |
| JP0+_gamma_pi:pi/1^S_0 pi:pi/1^S_0_order0     | 1.5634 +/- 0.65022     | 1.00  | -0.59 | 0.16  |       |       |       |       |       |       |       |       |       |
| JP0+_gamma_pi:pi/1^S_0 pi:pi/1^S_0_order1     | -1.5530 +/- 0.6674     | 1.00  | -0.01 |       |       |       |       |       |       |       |       |       |       |
| JP0+_m_pole0                                  | 0.13190 +/- 0.00073828 | 1.00  |       |       |       |       |       |       |       |       |       |       |       |
| JP0+_gamma_eta:eta/1^S_0_eta:eta/1^S_0_order1 | 0.0000 +/- 0           | FIXED |       |       |       |       |       |       |       |       |       |       |       |
| JP0+_gamma_eta:eta/1^S_0 kaon:kaon/1^S_0_orde | 0.0000 +/- 0           | FIXED |       |       |       |       |       |       |       |       |       |       |       |
| JP0+_gamma_eta:eta/1^S_0 pi:pi/1^S_0_order1   | 0.0000 +/- 0           | FIXED |       |       |       |       |       |       |       |       |       |       |       |
| JP0+_gamma_kaon:kaon/1^S_0 kaon:kaon/1^S_0_or | 0.0000 +/- 0           | FIXED |       |       |       |       |       |       |       |       |       |       |       |

## pole singularities

\*\*\*\*\*  
JP=0+ || eta:eta/1^S\_0[+] kaon:kaon/1^S\_0[+] pi:pi/1^S\_0[+]

sqrt(s)\_pole = ( 0.1319 +/- 0.00073442)  
+ (i/2)\*(+1.721e-13 +/- 5.9191e-11) [ 0.07]

| eta:eta/1^S_0                | kaon:kaon/1^S_0              | pi:pi/1^S_0                  |
|------------------------------|------------------------------|------------------------------|
| k_re= 0.0000 +/- 0.0000      | k_re= 0.0000 +/- 0.0000      | k_re= 0.0000 +/- 0.0000      |
| k_im= 0.0799 +/- 0.0003      | k_im= 0.0711 +/- 0.0003      | k_im= 0.0205 +/- 0.0012      |
| corr= [-0.07]                | corr= [-0.07]                | corr= [-0.07]                |
| g = 0.1275 +/- 0.0529        | g = 0.1161 +/- 0.0347        | g = 0.0924 +/- 0.0043        |
| arg(g)/pi= 0.0000 +/- 0.0000 | arg(g)/pi= 1.0000 +/- 0.0000 | arg(g)/pi= 1.0000 +/- 0.0000 |
| g_re= 0.1275 +/- 0.0529      | g_re= -0.1161 +/- 0.0347     | g_re= -0.0924 +/- 0.0043     |
| g_im= 0.0000 +/- 0.0000      | g_im= 0.0000 +/- 0.0000      | g_im= 0.0000 +/- 0.0000      |
| corr= [-1.00]                | corr= [-0.89]                | corr= [-0.21]                |

\*\*\*\*\*  
JP=0+ || eta:eta/1^S\_0[+] kaon:kaon/1^S\_0[+] pi:pi/1^S\_0[-]

sqrt(s)\_pole = ( 0.1527 +/- 0.011728)  
+ (i/2)\*(-0.10567 +/- 0.020211) [ 0.00]

| eta:eta/1^S_0                | kaon:kaon/1^S_0               | pi:pi/1^S_0                   |
|------------------------------|-------------------------------|-------------------------------|
| k_re= -0.0255 +/- 0.0052     | k_re= -0.0283 +/- 0.0057      | k_re= 0.0470 +/- 0.0073       |
| k_im= 0.0791 +/- 0.0054      | k_im= 0.0712 +/- 0.0058       | k_im= -0.0429 +/- 0.0066      |
| corr= [ 0.14]                | corr= [ 0.15]                 | corr= [ 0.11]                 |
| g = 0.1853 +/- 0.0602        | g = 0.0558 +/- 0.0575         | g = 0.0841 +/- 0.0129         |
| arg(g)/pi= 0.0535 +/- 0.0677 | arg(g)/pi= -0.7983 +/- 0.2553 | arg(g)/pi= -0.8127 +/- 0.0382 |
| g_re= 0.1827 +/- 0.0544      | g_re= -0.0450 +/- 0.0570      | g_re= -0.0700 +/- 0.0133      |
| g_im= 0.0310 +/- 0.0471      | g_im= -0.0330 +/- 0.0453      | g_im= -0.0467 +/- 0.0096      |
| corr= [ 0.81]                | corr= [ 0.19]                 | corr= [ 0.14]                 |

\*\*\*\*\*

\*\*\*\*\*  
JP=0+ || eta:eta/1^S\_0[+] kaon:kaon/1^S\_0[+] pi:pi/1^S\_0[-]

sqrt(s)\_pole = (0.20371 +/- 0.0044099)  
+ (i/2)\*(-0.025273 +/- 0.0064347) [-0.03]

| eta:eta/1^S_0                | kaon:kaon/1^S_0               | pi:pi/1^S_0                   |
|------------------------------|-------------------------------|-------------------------------|
| k_re= -0.0217 +/- 0.0053     | k_re= -0.0355 +/- 0.0055      | k_re= 0.0751 +/- 0.0030       |
| k_im= 0.0296 +/- 0.0054      | k_im= 0.0181 +/- 0.0043       | k_im= -0.0086 +/- 0.0022      |
| corr= [ 0.30]                | corr= [ 0.21]                 | corr= [-0.00]                 |
| g = 0.0676 +/- 0.0227        | g = 0.1255 +/- 0.0149         | g = 0.0936 +/- 0.0122         |
| arg(g)/pi= 0.2583 +/- 0.0777 | arg(g)/pi= -0.7806 +/- 0.0391 | arg(g)/pi= -0.3362 +/- 0.0335 |
| g_re= 0.0465 +/- 0.0236      | g_re= -0.0968 +/- 0.0124      | g_re= 0.0461 +/- 0.0126       |
| g_im= 0.0490 +/- 0.0152      | g_im= -0.0798 +/- 0.0174      | g_im= -0.0814 +/- 0.0094      |
| corr= [ 0.37]                | corr= [ 0.03]                 | corr= [-0.43]                 |

\*\*\*\*\*

\*\*\*\*\*  
JP=0+ || eta:eta/1^S\_0[+] kaon:kaon/1^S\_0[-] pi:pi/1^S\_0[-]

sqrt(s)\_pole = (0.18676 +/- 0.010304)  
+ (i/2)\*(-0.082029 +/- 0.025824) [ 0.11]

| eta:eta/1^S_0                 | kaon:kaon/1^S_0              | pi:pi/1^S_0                    |
|-------------------------------|------------------------------|--------------------------------|
| k_re= -0.0324 +/- 0.0080      | k_re= 0.0380 +/- 0.0082      | k_re= 0.0661 +/- 0.0067        |
| k_im= 0.0591 +/- 0.0086       | k_im= -0.0505 +/- 0.0094     | k_im= -0.0290 +/- 0.0086       |
| corr= [-0.23]                 | corr= [-0.20]                | corr= [ 0.01]                  |
| g = 0.0030 +/- 0.0633         | g = 0.0033 +/- 1.0739        | g = 0.0051 +/- 1.6317          |
| arg(g)/pi= 0.1041 +/- 15.2771 | arg(g)/pi= 0.7408 +/- 8.6084 | arg(g)/pi= -0.3646 +/- 10.6740 |
| g_re= 0.0028 +/- 0.0370       | g_re= -0.0023 +/- 0.6718     | g_re= 0.0021 +/- 0.8267        |
| g_im= 0.0009 +/- 0.1509       | g_im= 0.0024 +/- 0.8426      | g_im= -0.0046 +/- 1.4169       |
| corr= [ 0.13]                 | corr= [-1.00]                | corr= [-1.00]                  |

\*\*\*\*\*

\*\*\*\*\*  
JP=0+ || eta:eta/1^S\_0[+] kaon:kaon/1^S\_0[-] pi:pi/1^S\_0[-]

sqrt(s)\_pole = (0.14956 +/- 0.014686)  
+ (i/2)\*(-0.11817 +/- 0.033083) [ 0.38]

| eta:eta/1^S_0                | kaon:kaon/1^S_0              | pi:pi/1^S_0                   |
|------------------------------|------------------------------|-------------------------------|
| k_re= -0.0269 +/- 0.0059     | k_re= 0.0296 +/- 0.0062      | k_re= 0.0467 +/- 0.0076       |
| k_im= 0.0821 +/- 0.0085      | k_im= -0.0746 +/- 0.0092     | k_im= -0.0473 +/- 0.0110      |
| corr= [-0.20]                | corr= [-0.15]                | corr= [ 0.18]                 |
| g = 0.1849 +/- 0.0424        | g = 0.0194 +/- 0.0162        | g = 0.0771 +/- 0.0185         |
| arg(g)/pi= 0.0633 +/- 0.0694 | arg(g)/pi= 0.7760 +/- 0.1628 | arg(g)/pi= -0.6862 +/- 0.1033 |
| g_re= 0.1812 +/- 0.0366      | g_re= -0.0148 +/- 0.0081     | g_re= -0.0426 +/- 0.0208      |
| g_im= 0.0365 +/- 0.0456      | g_im= 0.0125 +/- 0.0171      | g_im= -0.0643 +/- 0.0231      |
| corr= [ 0.66]                | corr= [-0.73]                | corr= [-0.36]                 |

\*\*\*\*\*

\*\*\*\*\*  
JP=0+ || eta:eta/1^S\_0[-] kaon:kaon/1^S\_0[+] pi:pi/1^S\_0[+]

sqrt(s)\_pole = (0.18766 +/- 0.010406)  
+ (i/2)\*(-0.11808 +/- 0.025938) [ 0.27]

| eta:eta/1^S_0                | kaon:kaon/1^S_0               | pi:pi/1^S_0                   |
|------------------------------|-------------------------------|-------------------------------|
| k_re= 0.0412 +/- 0.0062      | k_re= -0.0461 +/- 0.0063      | k_re= -0.0691 +/- 0.0060      |
| k_im= -0.0672 +/- 0.0083     | k_im= 0.0600 +/- 0.0088       | k_im= 0.0401 +/- 0.0083       |
| corr= [-0.19]                | corr= [-0.12]                 | corr= [ 0.15]                 |
| g = 0.0559 +/- 0.0317        | g = 0.1640 +/- 0.0187         | g = 0.1235 +/- 0.0162         |
| arg(g)/pi= 0.2874 +/- 0.0832 | arg(g)/pi= -0.7984 +/- 0.0594 | arg(g)/pi= -0.8599 +/- 0.0435 |
| g_re= 0.0346 +/- 0.0142      | g_re= -0.1322 +/- 0.0165      | g_re= -0.1117 +/- 0.0102      |
| g_im= 0.0439 +/- 0.0318      | g_im= -0.0971 +/- 0.0319      | g_im= -0.0526 +/- 0.0210      |

```

corr= [ 0.68] | corr= [-0.36] | corr= [ 0.58] |
*****

*****
JP=0+ || eta:eta/1^S_0[-] kaon:kaon/1^S_0[+] pi:pi/1^S_0[+]

sqrt(s)_pole = (0.24775 +/- 0.014146)
+ (i/2)*(-0.067175 +/- 0.075505) [-0.72]

eta:eta/1^S_0 | kaon:kaon/1^S_0 | pi:pi/1^S_0 |
=====
k_re= 0.0718 +/- 0.0173 | k_re= -0.0796 +/- 0.0145 | k_re= -0.1034 +/- 0.0093 |
k_im= -0.0289 +/- 0.0276 | k_im= 0.0261 +/- 0.0263 | k_im= 0.0201 +/- 0.0220 |
corr= [-0.86] | corr= [-0.84] | corr= [-0.78] |
=====
|g|= 0.1403 +/- 0.0253 | |g|= 0.0705 +/- 0.0295 | |g|= 0.0382 +/- 0.0236 |
arg(g)/pi= -0.4232 +/- 0.1200 | arg(g)/pi= 0.6895 +/- 0.1168 | arg(g)/pi= -0.4490 +/- 0.2101 |
=====
g_re= 0.0335 +/- 0.0459 | g_re= -0.0396 +/- 0.0294 | g_re= 0.0061 +/- 0.0228 |
g_im= -0.1363 +/- 0.0365 | g_im= 0.0584 +/- 0.0260 | g_im= -0.0377 +/- 0.0260 |
corr= [ 0.95] | corr= [-0.19] | corr= [ 0.60] |
=====

*****
JP=0+ || eta:eta/1^S_0[-] kaon:kaon/1^S_0[+] pi:pi/1^S_0[-]

sqrt(s)_pole = (0.24656 +/- 0.01178)
+ (i/2)*(-0.076943 +/- 0.077046) [-0.48]

eta:eta/1^S_0 | kaon:kaon/1^S_0 | pi:pi/1^S_0 |
=====
k_re= 0.0719 +/- 0.0148 | k_re= -0.0795 +/- 0.0123 | k_re= 0.1029 +/- 0.0078 |
k_im= -0.0330 +/- 0.0281 | k_im= 0.0298 +/- 0.0269 | k_im= -0.0230 +/- 0.0225 |
corr= [-0.80] | corr= [-0.76] | corr= [-0.60] |
=====
|g|= 0.1360 +/- 0.0375 | |g|= 0.0745 +/- 0.0399 | |g|= 0.0377 +/- 0.0171 |
arg(g)/pi= -0.4610 +/- 0.1132 | arg(g)/pi= 0.5131 +/- 0.1389 | arg(g)/pi= 0.3521 +/- 0.1751 |
=====
g_re= 0.0166 +/- 0.0437 | g_re= -0.0031 +/- 0.0335 | g_re= 0.0169 +/- 0.0183 |
g_im= -0.1350 +/- 0.0429 | g_im= 0.0744 +/- 0.0391 | g_im= 0.0337 +/- 0.0196 |
corr= [ 0.96] | corr= [-0.61] | corr= [-0.29] |
=====

*****
JP=0+ || eta:eta/1^S_0[-] kaon:kaon/1^S_0[+] pi:pi/1^S_0[-]

sqrt(s)_pole = (0.11717 +/- 0.020393)
+ (i/2)*(+1.0552e-14 +/- 5.0007e-12) [ 0.05]

eta:eta/1^S_0 | kaon:kaon/1^S_0 | pi:pi/1^S_0 |
=====
k_re= -0.0000 +/- 0.0000 | k_re= 0.0000 +/- 0.0000 | k_re= -0.0000 +/- 0.0000 |
k_im= -0.0855 +/- 0.0070 | k_im= 0.0773 +/- 0.0077 | k_im= -0.0366 +/- 0.0162 |
corr= [-0.05] | corr= [-0.05] | corr= [-0.05] |
=====
|g|= 0.0191 +/- 0.0072 | |g|= 0.0370 +/- 0.0493 | |g|= 0.0744 +/- 0.0159 |
arg(g)/pi= 0.5000 +/- 0.0000 | arg(g)/pi= 0.5000 +/- 0.0000 | arg(g)/pi= 0.5000 +/- 0.0000 |
=====
g_re= 0.0000 +/- 0.0000 | g_re= -0.0000 +/- 0.0000 | g_re= -0.0000 +/- 0.0000 |
g_im= 0.0191 +/- 0.0072 | g_im= 0.0370 +/- 0.0493 | g_im= 0.0744 +/- 0.0159 |
corr= [-1.00] | corr= [-0.91] | corr= [ 0.31] |
=====

*****
JP=0+ || eta:eta/1^S_0[-] kaon:kaon/1^S_0[+] pi:pi/1^S_0[-]

sqrt(s)_pole = (0.20728 +/- 0.0057319)
+ (i/2)*(-0.03585 +/- 0.012892) [-0.07]

eta:eta/1^S_0 | kaon:kaon/1^S_0 | pi:pi/1^S_0 |
=====
k_re= 0.0298 +/- 0.0075 | k_re= -0.0418 +/- 0.0066 | k_re= 0.0777 +/- 0.0038 |
k_im= -0.0311 +/- 0.0072 | k_im= 0.0222 +/- 0.0068 | k_im= -0.0120 +/- 0.0042 |
corr= [-0.13] | corr= [-0.13] | corr= [-0.08] |
=====
|g|= 0.0517 +/- 0.0221 | |g|= 0.1331 +/- 0.0138 | |g|= 0.0858 +/- 0.0087 |
arg(g)/pi= 0.1287 +/- 0.1309 | arg(g)/pi= -0.7971 +/- 0.0430 | arg(g)/pi= -0.2909 +/- 0.0360 |
=====
g_re= 0.0475 +/- 0.0209 | g_re= -0.1069 +/- 0.0117 | g_re= 0.0524 +/- 0.0081 |
g_im= 0.0203 +/- 0.0224 | g_im= -0.0792 +/- 0.0194 | g_im= -0.0679 +/- 0.0102 |
corr= [ 0.12] | corr= [-0.14] | corr= [ 0.17] |
=====

*****
JP=0+ || eta:eta/1^S_0[-] kaon:kaon/1^S_0[-] pi:pi/1^S_0[+]

sqrt(s)_pole = ( 0.2563 +/- 0.016386)
+ (i/2)*(-0.068357 +/- 0.076289) [-0.74]

eta:eta/1^S_0 | kaon:kaon/1^S_0 | pi:pi/1^S_0 |
=====
k_re= 0.0785 +/- 0.0175 | k_re= 0.0859 +/- 0.0151 | k_re= -0.1085 +/- 0.0105 |
k_im= -0.0279 +/- 0.0270 | k_im= -0.0255 +/- 0.0258 | k_im= 0.0202 +/- 0.0219 |
corr= [-0.85] | corr= [-0.83] | corr= [-0.78] |
=====
|g|= 0.1268 +/- 0.0285 | |g|= 0.0462 +/- 0.0143 | |g|= 0.0723 +/- 0.0257 |
arg(g)/pi= -0.4518 +/- 0.1516 | arg(g)/pi= -0.2197 +/- 0.1414 | arg(g)/pi= -0.4632 +/- 0.0419 |
=====

```



```

-----|-----|-----|
g_re= 0.0191 +/- 0.0554 | g_re= 0.0356 +/- 0.0170 | g_re= 0.0083 +/- 0.0095 |
g_im= -0.1253 +/- 0.0372 | g_im= -0.0294 +/- 0.0184 | g_im= -0.0719 +/- 0.0257 |
corr= [ 0.99] | corr= [ 0.34] | corr= [-0.13] |
*****

```

```

*****
JP=0+ || eta:eta/1^S_0[-] kaon:kaon/1^S_0[-] pi:pi/1^S_0[-]

```

```

sqrt(s)_pole = (0.11957 +/- 0.019536)
+ (i/2)*(+1.7407e-15 +/- 4.7187e-13) [ 0.08]

```

```

eta:eta/1^S_0 | kaon:kaon/1^S_0 | pi:pi/1^S_0 |
-----|-----|-----|
k_re= -0.0000 +/- 0.0000 | k_re= -0.0000 +/- 0.0000 | k_re= -0.0000 +/- 0.0000 |
k_im= -0.0847 +/- 0.0069 | k_im= -0.0764 +/- 0.0076 | k_im= -0.0345 +/- 0.0168 |
corr= [-0.08] | corr= [-0.08] | corr= [-0.08] |
-----|-----|-----|
|g|= 0.0222 +/- 0.0087 | |g|= 0.0061 +/- 0.0071 | |g|= 0.0676 +/- 0.0164 |
arg(g)/pi= 0.5000 +/- 0.0000 | arg(g)/pi= 0.5000 +/- 0.0000 | arg(g)/pi= 0.5000 +/- 0.0000 |
-----|-----|-----|
g_re= 0.0000 +/- 0.0000 | g_re= -0.0000 +/- 0.0000 | g_re= -0.0000 +/- 0.0000 |
g_im= 0.0222 +/- 0.0087 | g_im= 0.0061 +/- 0.0071 | g_im= 0.0676 +/- 0.0164 |
corr= [-1.00] | corr= [-0.84] | corr= [ 0.29] |
*****

```

```

*****
JP=0+ || eta:eta/1^S_0[-] kaon:kaon/1^S_0[-] pi:pi/1^S_0[-]

```

```

sqrt(s)_pole = (0.24723 +/- 0.017058)
+ (i/2)*(-0.094404 +/- 0.091964) [-0.71]

```

```

eta:eta/1^S_0 | kaon:kaon/1^S_0 | pi:pi/1^S_0 |
-----|-----|-----|
k_re= 0.0743 +/- 0.0206 | k_re= 0.0813 +/- 0.0177 | k_re= 0.1037 +/- 0.0115 |
k_im= -0.0392 +/- 0.0304 | k_im= -0.0359 +/- 0.0299 | k_im= -0.0281 +/- 0.0263 |
corr= [-0.87] | corr= [-0.85] | corr= [-0.78] |
-----|-----|-----|
|g|= 0.1223 +/- 0.0327 | |g|= 0.0425 +/- 0.0243 | |g|= 0.0654 +/- 0.0251 |
arg(g)/pi= -0.4550 +/- 0.1569 | arg(g)/pi= -0.4830 +/- 0.1204 | arg(g)/pi= 0.2464 +/- 0.0952 |
-----|-----|-----|
g_re= 0.0173 +/- 0.0552 | g_re= 0.0023 +/- 0.0164 | g_re= 0.0468 +/- 0.0195 |
g_im= -0.1211 +/- 0.0408 | g_im= -0.0424 +/- 0.0241 | g_im= 0.0457 +/- 0.0252 |
corr= [ 0.99] | corr= [-0.24] | corr= [ 0.26] |
*****

```

```

*****
JP=0+ || eta:eta/1^S_0[-] kaon:kaon/1^S_0[-] pi:pi/1^S_0[-]

```

```

sqrt(s)_pole = (0.18684 +/- 0.0099448)
+ (i/2)*(-0.082053 +/- 0.02436) [ 0.12]

```

```

eta:eta/1^S_0 | kaon:kaon/1^S_0 | pi:pi/1^S_0 |
-----|-----|-----|
k_re= 0.0324 +/- 0.0075 | k_re= 0.0380 +/- 0.0078 | k_re= 0.0662 +/- 0.0065 |
k_im= -0.0591 +/- 0.0082 | k_im= -0.0504 +/- 0.0090 | k_im= -0.0290 +/- 0.0082 |
corr= [-0.21] | corr= [-0.18] | corr= [ 0.03] |
-----|-----|-----|
|g|= 0.0026 +/- 0.0124 | |g|= 0.0610 +/- 0.2185 | |g|= 0.0890 +/- 0.3170 |
arg(g)/pi= 0.1826 +/- 2.0806 | arg(g)/pi= 0.7039 +/- 0.0408 | arg(g)/pi= -0.3333 +/- 0.0923 |
-----|-----|-----|
g_re= 0.0022 +/- 0.0154 | g_re= -0.0365 +/- 0.1309 | g_re= 0.0445 +/- 0.1581 |
g_im= 0.0014 +/- 0.0144 | g_im= 0.0489 +/- 0.1751 | g_im= -0.0771 +/- 0.2760 |
corr= [-0.37] | corr= [-1.00] | corr= [-0.98] |
*****

```

# k\_sigma\_pole\_sccccc\_Adler\_L0

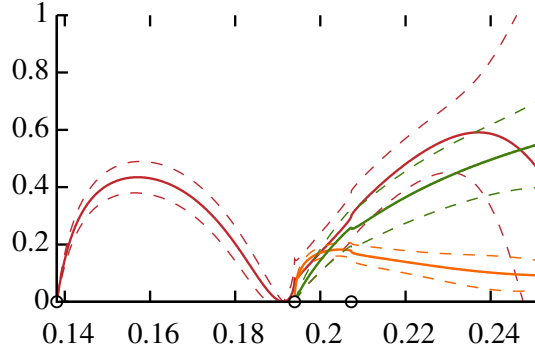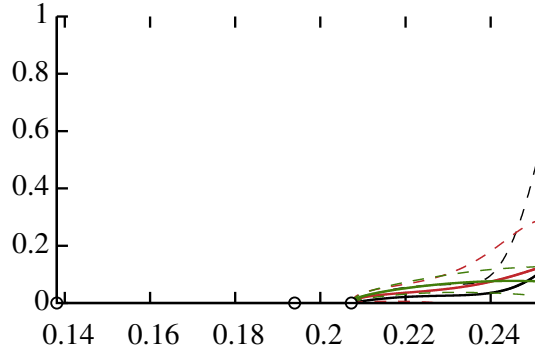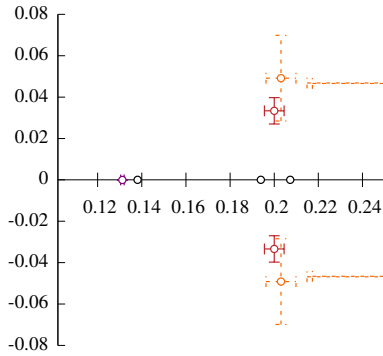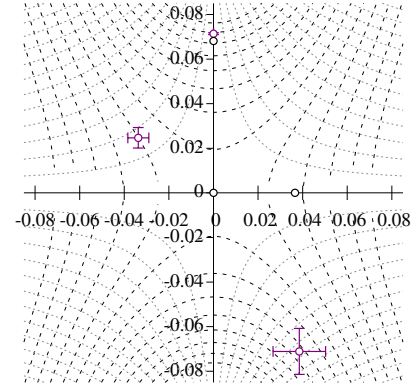

## parameter values

minimised with chisq/nDoF = 45.74 / (57 - 10) = 0.97

|                                               |                        |      |       |       |       |       |      |       |       |       |       |
|-----------------------------------------------|------------------------|------|-------|-------|-------|-------|------|-------|-------|-------|-------|
| JPO+_g_eta:eta/1^S_0_pole0                    | 1.3159 +/- 0.85844     | 1.00 | -0.57 | 0.19  | 0.99  | 0.89  | 0.97 | -0.61 | -0.52 | 0.15  | -0.05 |
| JPO+_g_kaon:kaon/1^S_0_pole0                  | 1.5849 +/- 0.60536     | 1.00 | 0.54  | -0.61 | -0.18 | -0.50 | 0.99 | 0.91  | -0.02 | 0.14  |       |
| JPO+_g_pi:pi/1^S_0_pole0                      | 1.2460 +/- 0.14335     |      |       | 1.00  | 0.14  | 0.49  | 0.25 | 0.48  | 0.58  | 0.42  | 0.10  |
| JPO+_gamma_eta:eta/1^S_0_eta:eta/1^S_0_order0 | 55.103 +/- 70.511      |      |       |       | 1.00  | 0.88  | 0.97 | -0.65 | -0.56 | 0.15  | -0.06 |
| JPO+_gamma_eta:eta/1^S_0 kaon:kaon/1^S_0_orde | 73.664 +/- 35.974      |      |       |       |       | 1.00  | 0.90 | -0.24 | -0.15 | 0.21  | 0.02  |
| JPO+_gamma_eta:eta/1^S_0 pi:pi/1^S_0_order0   | 29.442 +/- 33.14       |      |       |       |       |       | 1.00 | -0.54 | -0.45 | 0.22  | -0.03 |
| JPO+_gamma_kaon:kaon/1^S_0 kaon:kaon/1^S_0_or | 73.114 +/- 66.756      |      |       |       |       |       |      | 1.00  | 0.92  | -0.01 | 0.17  |
| JPO+_gamma_kaon:kaon/1^S_0 pi:pi/1^S_0_order0 | 10.915 +/- 24.647      |      |       |       |       |       |      |       | 1.00  | 0.34  | 0.19  |
| JPO+_gamma_pi:pi/1^S_0 pi:pi/1^S_0_order1     | 13.284 +/- 12.359      |      |       |       |       |       |      |       |       | 1.00  | 0.08  |
| JPO+_m_pole0                                  | 0.13122 +/- 0.00078344 |      |       |       |       |       |      |       |       |       | 1.00  |
| JPO+_gamma_eta:eta/1^S_0_eta:eta/1^S_0_order1 | 0.0000 +/- 0           |      |       |       |       |       |      |       |       |       | FIXED |
| JPO+_gamma_eta:eta/1^S_0 kaon:kaon/1^S_0_orde | 0.0000 +/- 0           |      |       |       |       |       |      |       |       |       | FIXED |
| JPO+_gamma_eta:eta/1^S_0 pi:pi/1^S_0_order1   | 0.0000 +/- 0           |      |       |       |       |       |      |       |       |       | FIXED |
| JPO+_gamma_kaon:kaon/1^S_0 kaon:kaon/1^S_0_or | 0.0000 +/- 0           |      |       |       |       |       |      |       |       |       | FIXED |
| JPO+_gamma_kaon:kaon/1^S_0 pi:pi/1^S_0_order1 | 0.0000 +/- 0           |      |       |       |       |       |      |       |       |       | FIXED |
| JPO+_gamma_pi:pi/1^S_0 pi:pi/1^S_0_order0     | 0.0000 +/- 0           |      |       |       |       |       |      |       |       |       | FIXED |

## pole singularities

\*\*\*\*\*

JP=0+ || eta:eta/1^S\_0[+] kaon:kaon/1^S\_0[+] pi:pi/1^S\_0[+]

sqrt(s)\_pole = (0.13122 +/- 0.00077243)  
+ (i/2)\*(-1.7152e-14 +/- 3.7531e-12) [-0.15]

| eta:eta/1^S_0                | kaon:kaon/1^S_0               | pi:pi/1^S_0                   |
|------------------------------|-------------------------------|-------------------------------|
| k_re= -0.0000 +/- 0.0000     | k_re= -0.0000 +/- 0.0000      | k_re= -0.0000 +/- 0.0000      |
| k_im= 0.0802 +/- 0.0003      | k_im= 0.0714 +/- 0.0004       | k_im= 0.0216 +/- 0.0012       |
| corr= [ 0.15]                | corr= [ 0.15]                 | corr= [ 0.15]                 |
| g = 0.0941 +/- 0.0620        | g = 0.1133 +/- 0.0385         | g = 0.0891 +/- 0.0035         |
| arg(g)/pi= 0.0000 +/- 0.0000 | arg(g)/pi= -0.0000 +/- 0.0000 | arg(g)/pi= -0.0000 +/- 0.0000 |
| g_re= 0.0941 +/- 0.0620      | g_re= 0.1133 +/- 0.0385       | g_re= 0.0891 +/- 0.0035       |
| g_im= 0.0000 +/- 0.0000      | g_im= -0.0000 +/- 0.0000      | g_im= -0.0000 +/- 0.0000      |
| corr= [-1.00]                | corr= [-0.86]                 | corr= [-0.16]                 |

\*\*\*\*\*

```

*****
JP=0+ || eta:eta/1^S_0[+] kaon:kaon/1^S_0[+] pi:pi/1^S_0[-]
*** not found on all cfigs ***
sqrt(s)_pole = (0.07243 +/- 0.0044552)
               + (i/2)*(-7.5255e-13 +/- 2.0772e-11) [-0.21]

eta:eta/1^S_0 | kaon:kaon/1^S_0 | pi:pi/1^S_0 |
=====|=====|=====|
k_re= -0.0000 +/- 0.0000 | k_re= -0.0000 +/- 0.0000 | k_re= 0.0000 +/- 0.0000 |
k_im= 0.0971 +/- 0.0008 | k_im= 0.0900 +/- 0.0009 | k_im= -0.0588 +/- 0.0014 |
corr= [ 0.21] | corr= [ 0.21] | corr= [ 0.21] |
=====|=====|=====|
|g|= 0.4152 +/- 10.6602 | |g|= 0.4161 +/- 10.6482 | |g|= 0.4101 +/- 10.7230 |
arg(g)/pi= 0.2322 +/- 0.6495 | arg(g)/pi= 0.2315 +/- 0.6717 | arg(g)/pi= 0.2357 +/- 0.5270 |
=====|=====|=====|
g_re= 0.3095 +/- 7.3839 | g_re= 0.3108 +/- 7.3701 | g_re= 0.3027 +/- 7.4570 |
g_im= 0.2767 +/- 7.7354 | g_im= 0.2767 +/- 7.7354 | g_im= 0.2767 +/- 7.7354 |
corr= [ 1.00] | corr= [ 1.00] | corr= [ 1.00] |
=====|=====|=====|
*****

*****
JP=0+ || eta:eta/1^S_0[+] kaon:kaon/1^S_0[+] pi:pi/1^S_0[-]

sqrt(s)_pole = (0.20002 +/- 0.0044556)
               + (i/2)*(-0.033386 +/- 0.006384) [ 0.14]

eta:eta/1^S_0 | kaon:kaon/1^S_0 | pi:pi/1^S_0 |
=====|=====|=====|
k_re= -0.0229 +/- 0.0040 | k_re= -0.0337 +/- 0.0047 | k_re= 0.0728 +/- 0.0030 |
k_im= 0.0365 +/- 0.0050 | k_im= 0.0247 +/- 0.0046 | k_im= -0.0115 +/- 0.0022 |
corr= [ 0.28] | corr= [ 0.35] | corr= [ 0.19] |
=====|=====|=====|
|g|= 0.0693 +/- 0.0250 | |g|= 0.1472 +/- 0.0093 | |g|= 0.1077 +/- 0.0118 |
arg(g)/pi= 0.2167 +/- 0.1115 | arg(g)/pi= 0.1937 +/- 0.0481 | arg(g)/pi= 0.5958 +/- 0.0416 |
=====|=====|=====|
g_re= 0.0538 +/- 0.0303 | g_re= 0.1208 +/- 0.0125 | g_re= -0.0319 +/- 0.0138 |
g_im= 0.0436 +/- 0.0173 | g_im= 0.0842 +/- 0.0206 | g_im= 0.1028 +/- 0.0120 |
corr= [-0.09] | corr= [-0.65] | corr= [ 0.11] |
=====|=====|=====|
*****

*****
JP=0+ || eta:eta/1^S_0[+] kaon:kaon/1^S_0[-] pi:pi/1^S_0[-]

sqrt(s)_pole = (0.16644 +/- 0.026826)
               + (i/2)*(-0.13163 +/- 0.017964) [ 0.01]

eta:eta/1^S_0 | kaon:kaon/1^S_0 | pi:pi/1^S_0 |
=====|=====|=====|
k_re= -0.0350 +/- 0.0105 | k_re= 0.0385 +/- 0.0118 | k_re= 0.0577 +/- 0.0154 |
k_im= 0.0783 +/- 0.0104 | k_im= -0.0711 +/- 0.0103 | k_im= -0.0475 +/- 0.0071 |
corr= [ 0.80] | corr= [ 0.79] | corr= [ 0.62] |
=====|=====|=====|
|g|= 0.0383 +/- 0.1137 | |g|= 0.0690 +/- 0.1973 | |g|= 0.1145 +/- 0.3300 |
arg(g)/pi= 0.3925 +/- 0.6895 | arg(g)/pi= 0.6851 +/- 0.0609 | arg(g)/pi= -0.3976 +/- 0.0477 |
=====|=====|=====|
g_re= 0.0127 +/- 0.0749 | g_re= -0.0379 +/- 0.1107 | g_re= 0.0362 +/- 0.1075 |
g_im= 0.0361 +/- 0.1190 | g_im= 0.0576 +/- 0.1639 | g_im= -0.1086 +/- 0.3125 |
corr= [-0.06] | corr= [-0.99] | corr= [-0.99] |
=====|=====|=====|
*****

*****
JP=0+ || eta:eta/1^S_0[-] kaon:kaon/1^S_0[+] pi:pi/1^S_0[-]

sqrt(s)_pole = (0.25955 +/- 0.044672)
               + (i/2)*(-0.046829 +/- 0.034117) [-0.56]

eta:eta/1^S_0 | kaon:kaon/1^S_0 | pi:pi/1^S_0 |
=====|=====|=====|
k_re= 0.0795 +/- 0.0363 | k_re= -0.0872 +/- 0.0333 | k_re= 0.1101 +/- 0.0264 |
k_im= -0.0191 +/- 0.0114 | k_im= 0.0174 +/- 0.0109 | k_im= -0.0138 +/- 0.0095 |
corr= [-0.26] | corr= [-0.35] | corr= [-0.50] |
=====|=====|=====|
|g|= 0.0956 +/- 0.0441 | |g|= 0.0182 +/- 0.0510 | |g|= 0.0783 +/- 0.0622 |
arg(g)/pi= -0.2560 +/- 0.2975 | arg(g)/pi= -0.2547 +/- 2.1247 | arg(g)/pi= -0.7157 +/- 0.0836 |
=====|=====|=====|
g_re= 0.0663 +/- 0.0520 | g_re= 0.0127 +/- 0.0632 | g_re= -0.0491 +/- 0.0470 |
g_im= -0.0689 +/- 0.0850 | g_im= -0.0130 +/- 0.1154 | g_im= -0.0610 +/- 0.0457 |
corr= [ 0.70] | corr= [ 0.85] | corr= [ 0.83] |
=====|=====|=====|
*****

*****
JP=0+ || eta:eta/1^S_0[-] kaon:kaon/1^S_0[+] pi:pi/1^S_0[-]

sqrt(s)_pole = (0.20306 +/- 0.0067955)
               + (i/2)*(-0.04916 +/- 0.020712) [ 0.30]

eta:eta/1^S_0 | kaon:kaon/1^S_0 | pi:pi/1^S_0 |
=====|=====|=====|
k_re= 0.0315 +/- 0.0075 | k_re= -0.0410 +/- 0.0066 | k_re= 0.0753 +/- 0.0043 |
k_im= -0.0397 +/- 0.0100 | k_im= 0.0304 +/- 0.0105 | k_im= -0.0166 +/- 0.0070 |
corr= [-0.41] | corr= [-0.23] | corr= [ 0.22] |
=====|=====|=====|
|g|= 0.0532 +/- 0.0290 | |g|= 0.1581 +/- 0.0193 | |g|= 0.1091 +/- 0.0185 |
arg(g)/pi= 0.1155 +/- 0.1365 | arg(g)/pi= 0.1775 +/- 0.0589 | arg(g)/pi= 0.6466 +/- 0.0336 |
=====|=====|=====|
g_re= 0.0498 +/- 0.0285 | g_re= 0.1341 +/- 0.0228 | g_re= -0.0485 +/- 0.0127 |
g_im= 0.0189 +/- 0.0235 | g_im= 0.0837 +/- 0.0266 | g_im= 0.0977 +/- 0.0177 |
=====|=====|=====|

```

```

corr= [ 0.14] | corr= [-0.37] | corr= [-0.33] |
*****

```

```

*****
JP=0+ || eta:eta/1^S_0[-] kaon:kaon/1^S_0[-] pi:pi/1^S_0[-]

```

```

sqrt(s)_pole = ( 0.2599 +/- 0.042568)
               + (i/2)*(-0.046599 +/- 0.035345) [-0.47]

```

| eta:eta/1^S_0                 |  | kaon:kaon/1^S_0              |  | pi:pi/1^S_0                   |  |
|-------------------------------|--|------------------------------|--|-------------------------------|--|
| k_re= 0.0798 +/- 0.0345       |  | k_re= 0.0874 +/- 0.0316      |  | k_re= 0.1103 +/- 0.0251       |  |
| k_im= -0.0190 +/- 0.0124      |  | k_im= -0.0173 +/- 0.0117     |  | k_im= -0.0137 +/- 0.0100      |  |
| corr= [-0.20]                 |  | corr= [-0.28]                |  | corr= [-0.42]                 |  |
| -----                         |  |                              |  |                               |  |
| g = 0.0875 +/- 0.0503         |  | g = 0.0089 +/- 0.0259        |  | g = 0.0863 +/- 0.0521         |  |
| arg(g)/pi= -0.2394 +/- 0.1070 |  | arg(g)/pi= 0.8965 +/- 2.1130 |  | arg(g)/pi= -0.7157 +/- 0.1416 |  |
| -----                         |  |                              |  |                               |  |
| g_re= 0.0639 +/- 0.0260       |  | g_re= -0.0084 +/- 0.0135     |  | g_re= -0.0541 +/- 0.0327      |  |
| g_im= -0.0598 +/- 0.0522      |  | g_im= 0.0028 +/- 0.0629      |  | g_im= -0.0672 +/- 0.0558      |  |
| corr= [-0.67]                 |  | corr= [-0.20]                |  | corr= [ 0.23]                 |  |

```

*****
JP=0+ || eta:eta/1^S_0[-] kaon:kaon/1^S_0[-] pi:pi/1^S_0[-]

```

```

sqrt(s)_pole = (0.16927 +/- 0.024819)
               + (i/2)*(-0.12975 +/- 0.03023) [ 0.46]

```

| eta:eta/1^S_0                |  | kaon:kaon/1^S_0              |  | pi:pi/1^S_0                   |  |
|------------------------------|--|------------------------------|--|-------------------------------|--|
| k_re= 0.0357 +/- 0.0086      |  | k_re= 0.0394 +/- 0.0097      |  | k_re= 0.0591 +/- 0.0133       |  |
| k_im= -0.0769 +/- 0.0130     |  | k_im= -0.0696 +/- 0.0133     |  | k_im= -0.0464 +/- 0.0114      |  |
| corr= [ 0.51]                |  | corr= [ 0.56]                |  | corr= [ 0.60]                 |  |
| -----                        |  |                              |  |                               |  |
| g = 0.0150 +/- 0.0134        |  | g = 0.0661 +/- 0.0341        |  | g = 0.1263 +/- 0.0175         |  |
| arg(g)/pi= 0.3320 +/- 0.8678 |  | arg(g)/pi= 0.7512 +/- 0.0560 |  | arg(g)/pi= -0.3894 +/- 0.0795 |  |
| -----                        |  |                              |  |                               |  |
| g_re= 0.0076 +/- 0.0313      |  | g_re= -0.0469 +/- 0.0200     |  | g_re= 0.0430 +/- 0.0305       |  |
| g_im= 0.0129 +/- 0.0295      |  | g_im= 0.0466 +/- 0.0300      |  | g_im= -0.1188 +/- 0.0193      |  |
| corr= [-0.89]                |  | corr= [-0.86]                |  | corr= [ 0.34]                 |  |

# k\_sigma\_pole\_ssssss\_noCM

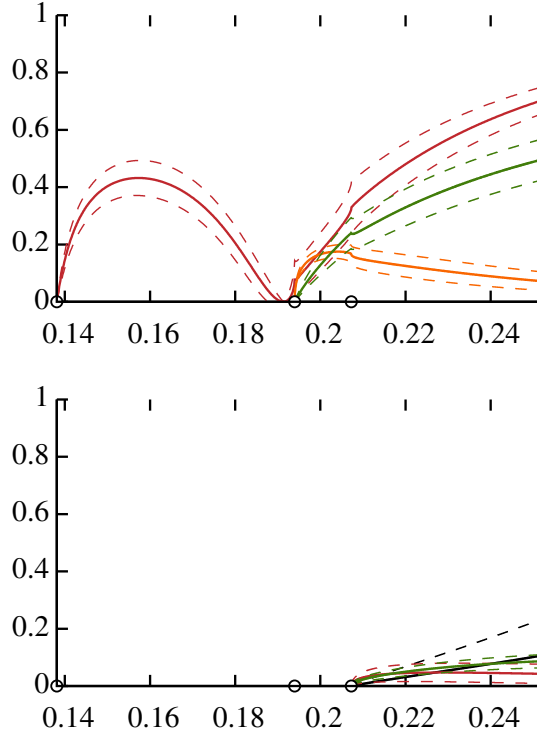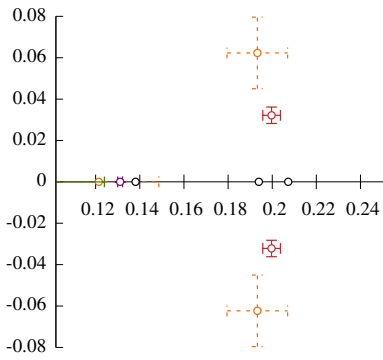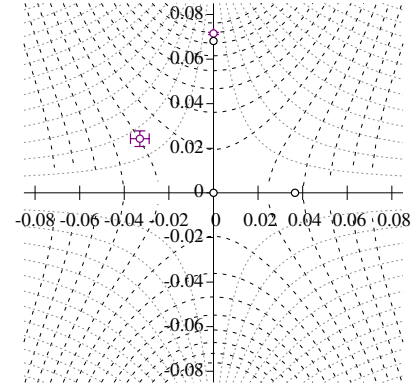

## parameter values

minimised with  $\chi^2/\text{nDoF} = 48.27 / (57 - 10) = 1.03$

|                                                   |                          |       |       |       |       |       |      |       |      |       |      |
|---------------------------------------------------|--------------------------|-------|-------|-------|-------|-------|------|-------|------|-------|------|
| JPO+_g_eta:eta/1^S_0_pole0                        | -0.018558 +/- 0.0569     | 1.00  | 0.80  | 0.46  | 0.14  | 0.16  | 0.34 | -0.13 | 0.24 | 0.29  | 0.04 |
| JPO+_g_kaon:kaon/1^S_0_pole0                      | 0.050495 +/- 0.020008    | 1.00  | 0.17  | 0.17  | -0.08 | 0.34  | 0.18 | 0.11  | 0.01 | -0.04 |      |
| JPO+_g_pi:pi/1^S_0_pole0                          | 0.098283 +/- 0.04665     | 1.00  | 0.04  | -0.21 | 0.13  | 0.33  | 0.62 | 0.57  | 0.01 |       |      |
| JPO+_gamma_eta:eta/1^S_0_eta:eta/1^S_0_order1     | -0.27476 +/- 0.34043     | 1.00  | -0.43 | 0.36  | -0.30 | -0.22 | 0.13 | 0.01  |      |       |      |
| JPO+_gamma_eta:eta/1^S_0 kaon:kaon/1^S_0_order1   | 0.17088 +/- 0.19008      | 1.00  | -0.48 | -0.21 | -0.11 | -0.21 | 0.00 |       |      |       |      |
| JPO+_gamma_eta:eta/1^S_0 pi:pi/1^S_0_order1       | 0.80024 +/- 0.30087      | 1.00  | -0.24 | 0.33  | 0.60  | 0.01  |      |       |      |       |      |
| JPO+_gamma_kaon:kaon/1^S_0 kaon:kaon/1^S_0_order1 | -0.90483 +/- 0.24397     | 1.00  | 0.21  | -0.10 | -0.00 |       |      |       |      |       |      |
| JPO+_gamma_kaon:kaon/1^S_0 pi:pi/1^S_0_order1     | -1.1702 +/- 0.14678      | 1.00  | 0.45  | -0.01 |       |       |      |       |      |       |      |
| JPO+_gamma_pi:pi/1^S_0 pi:pi/1^S_0_order1         | 0.97940 +/- 0.31971      | 1.00  | 0.01  |       |       |       |      |       |      |       |      |
| JPO+_m_pole0                                      | -5.1943e-05 +/- 0.098939 | 1.00  |       |       |       |       |      |       |      |       |      |
| JPO+_gamma_eta:eta/1^S_0_eta:eta/1^S_0_order0     | 0.0000 +/- 0             | FIXED |       |       |       |       |      |       |      |       |      |
| JPO+_gamma_eta:eta/1^S_0 kaon:kaon/1^S_0_order0   | 0.0000 +/- 0             | FIXED |       |       |       |       |      |       |      |       |      |
| JPO+_gamma_eta:eta/1^S_0 pi:pi/1^S_0_order0       | 0.0000 +/- 0             | FIXED |       |       |       |       |      |       |      |       |      |
| JPO+_gamma_kaon:kaon/1^S_0 kaon:kaon/1^S_0_order0 | 0.0000 +/- 0             | FIXED |       |       |       |       |      |       |      |       |      |
| JPO+_gamma_kaon:kaon/1^S_0 pi:pi/1^S_0_order0     | 0.0000 +/- 0             | FIXED |       |       |       |       |      |       |      |       |      |
| JPO+_gamma_pi:pi/1^S_0 pi:pi/1^S_0_order0         | 0.0000 +/- 0             | FIXED |       |       |       |       |      |       |      |       |      |

## pole singularities

\*\*\*\*\*  
JP=0+ || eta:eta/1^S\_0[+] kaon:kaon/1^S\_0[+] pi:pi/1^S\_0[+]

sqrt(s)\_pole = (0.13108 +/- 0.0010987)  
+ (i/2)\*(+3.0758e-13 +/- 9.2315e-11) [ 0.06]

| eta:eta/1^S_0                | kaon:kaon/1^S_0              | pi:pi/1^S_0                  |
|------------------------------|------------------------------|------------------------------|
| k_re= 0.0000 +/- 0.0000      | k_re= 0.0000 +/- 0.0000      | k_re= 0.0000 +/- 0.0000      |
| k_im= 0.0803 +/- 0.0004      | k_im= 0.0715 +/- 0.0005      | k_im= 0.0218 +/- 0.0017      |
| corr= [-0.06]                | corr= [-0.06]                | corr= [-0.06]                |
| g = 0.0305 +/- 0.0316        | g = 0.0762 +/- 0.0224        | g = 0.0895 +/- 0.0037        |
| arg(g)/pi= 0.0000 +/- 0.0000 | arg(g)/pi= 1.0000 +/- 0.0000 | arg(g)/pi= 1.0000 +/- 0.0000 |
| g_re= 0.0305 +/- 0.0316      | g_re= -0.0762 +/- 0.0224     | g_re= -0.0895 +/- 0.0037     |
| g_im= 0.0000 +/- 0.0000      | g_im= 0.0000 +/- 0.0000      | g_im= 0.0000 +/- 0.0000      |
| corr= [-1.00]                | corr= [-0.44]                | corr= [-0.08]                |

\*\*\*\*\*  
JP=0+ || eta:eta/1^S\_0[+] kaon:kaon/1^S\_0[+] pi:pi/1^S\_0[-]

sqrt(s)\_pole = (0.19971 +/- 0.0040023)  
+ (i/2)\*(-0.032164 +/- 0.0039652) [ 0.16]

| eta:eta/1^S_0                | kaon:kaon/1^S_0               | pi:pi/1^S_0                   |
|------------------------------|-------------------------------|-------------------------------|
| k_re= -0.0221 +/- 0.0031     | k_re= -0.0330 +/- 0.0042      | k_re= 0.0725 +/- 0.0027       |
| k_im= 0.0364 +/- 0.0043      | k_im= 0.0243 +/- 0.0035       | k_im= -0.0111 +/- 0.0014      |
| corr= [ 0.56]                | corr= [ 0.61]                 | corr= [ 0.26]                 |
| g = 0.0803 +/- 0.0205        | g = 0.1366 +/- 0.0120         | g = 0.1037 +/- 0.0062         |
| arg(g)/pi= 0.1028 +/- 0.0722 | arg(g)/pi= -0.8187 +/- 0.0240 | arg(g)/pi= -0.3996 +/- 0.0267 |
| g_re= 0.0762 +/- 0.0208      | g_re= -0.1150 +/- 0.0111      | g_re= 0.0321 +/- 0.0091       |
| g_im= 0.0255 +/- 0.0179      | g_im= -0.0736 +/- 0.0113      | g_im= -0.0985 +/- 0.0056      |
| corr= [ 0.00]                | corr= [ 0.17]                 | corr= [-0.06]                 |

\*\*\*\*\*

\*\*\*\*\*  
JP=0+ || eta:eta/1^S\_0[+] kaon:kaon/1^S\_0[-] pi:pi/1^S\_0[+]

\*\*\* not found on all cfigs \*\*\*  
sqrt(s)\_pole = (0.075263 +/- 0.048698)  
+ (i/2)\*(-6.9186e-15 +/- 3.6069e-15) [ 0.89]

| eta:eta/1^S_0                | kaon:kaon/1^S_0              | pi:pi/1^S_0                  |
|------------------------------|------------------------------|------------------------------|
| k_re= -0.0000 +/- 0.0000     | k_re= 0.0000 +/- 0.0000      | k_re= -0.0000 +/- 0.0000     |
| k_im= 0.0966 +/- 0.0094      | k_im= -0.0894 +/- 0.0102     | k_im= 0.0579 +/- 0.0157      |
| corr= [ 0.77]                | corr= [ 0.79]                | corr= [ 0.89]                |
| g = 0.1752 +/- 7.6306        | g = 0.1380 +/- 7.7516        | g = 0.1326 +/- 7.6726        |
| arg(g)/pi= 0.2240 +/- 1.2998 | arg(g)/pi= 0.3066 +/- 3.5641 | arg(g)/pi= 0.3264 +/- 4.9909 |
| g_re= 0.1336 +/- 5.3565      | g_re= 0.0788 +/- 5.6948      | g_re= 0.0688 +/- 5.7570      |
| g_im= 0.1133 +/- 5.4814      | g_im= 0.1133 +/- 5.4814      | g_im= 0.1133 +/- 5.4814      |
| corr= [ 1.00]                | corr= [ 1.00]                | corr= [ 1.00]                |

\*\*\*\*\*

\*\*\*\*\*  
JP=0+ || eta:eta/1^S\_0[-] kaon:kaon/1^S\_0[+] pi:pi/1^S\_0[+]

sqrt(s)\_pole = ( 0.1214 +/- 0.027171)  
+ (i/2)\*(+8.8352e-15 +/- 3.622e-12) [-0.01]

| eta:eta/1^S_0                | kaon:kaon/1^S_0              | pi:pi/1^S_0                  |
|------------------------------|------------------------------|------------------------------|
| k_re= -0.0000 +/- 0.0000     | k_re= 0.0000 +/- 0.0000      | k_re= 0.0000 +/- 0.0000      |
| k_im= -0.0840 +/- 0.0098     | k_im= 0.0756 +/- 0.0109      | k_im= 0.0329 +/- 0.0248      |
| corr= [ 0.01]                | corr= [ 0.01]                | corr= [ 0.01]                |
| g = 0.0290 +/- 0.0397        | g = 0.0891 +/- 0.0252        | g = 0.0831 +/- 0.0111        |
| arg(g)/pi= 0.0000 +/- 0.0000 | arg(g)/pi= 1.0000 +/- 0.0000 | arg(g)/pi= 1.0000 +/- 0.0000 |
| g_re= 0.0290 +/- 0.0397      | g_re= -0.0891 +/- 0.0252     | g_re= -0.0831 +/- 0.0111     |
| g_im= 0.0000 +/- 0.0000      | g_im= 0.0000 +/- 0.0000      | g_im= 0.0000 +/- 0.0000      |
| corr= [-0.99]                | corr= [ 0.30]                | corr= [-0.69]                |

\*\*\*\*\*

\*\*\*\*\*  
JP=0+ || eta:eta/1^S\_0[-] kaon:kaon/1^S\_0[+] pi:pi/1^S\_0[-]

sqrt(s)\_pole = (0.19326 +/- 0.01372)  
+ (i/2)\*(-0.062301 +/- 0.017268) [ 0.14]

| eta:eta/1^S_0                | kaon:kaon/1^S_0               | pi:pi/1^S_0                   |
|------------------------------|-------------------------------|-------------------------------|
| k_re= 0.0299 +/- 0.0086      | k_re= -0.0369 +/- 0.0101      | k_re= 0.0693 +/- 0.0091       |
| k_im= -0.0504 +/- 0.0105     | k_im= 0.0408 +/- 0.0103       | k_im= -0.0217 +/- 0.0061      |
| corr= [ 0.41]                | corr= [ 0.45]                 | corr= [ 0.26]                 |
| g = 0.0749 +/- 0.0188        | g = 0.1740 +/- 0.0109         | g = 0.1225 +/- 0.0109         |
| arg(g)/pi= 0.0150 +/- 0.1170 | arg(g)/pi= -0.8702 +/- 0.0565 | arg(g)/pi= -0.3938 +/- 0.0560 |
| g_re= 0.0749 +/- 0.0192      | g_re= -0.1598 +/- 0.0126      | g_re= 0.0401 +/- 0.0211       |
| g_im= 0.0035 +/- 0.0273      | g_im= -0.0690 +/- 0.0302      | g_im= -0.1157 +/- 0.0117      |
| corr= [-0.32]                | corr= [-0.57]                 | corr= [ 0.33]                 |

\*\*\*\*\*

\*\*\*\*\*  
JP=0+ || eta:eta/1^S\_0[-] kaon:kaon/1^S\_0[-] pi:pi/1^S\_0[-]

sqrt(s)\_pole = (0.13495 +/- 0.015025)  
+ (i/2)\*(-0.12213 +/- 0.038736) [ 0.40]

| eta:eta/1^S_0                 | kaon:kaon/1^S_0              | pi:pi/1^S_0                   |
|-------------------------------|------------------------------|-------------------------------|
| k_re= 0.0235 +/- 0.0058       | k_re= 0.0257 +/- 0.0061      | k_re= 0.0396 +/- 0.0072       |
| k_im= -0.0876 +/- 0.0082      | k_im= -0.0803 +/- 0.0089     | k_im= -0.0521 +/- 0.0118      |
| corr= [-0.34]                 | corr= [-0.31]                | corr= [ 0.00]                 |
| g = 0.0424 +/- 0.0169         | g = 0.0488 +/- 0.0124        | g = 0.1364 +/- 0.0214         |
| arg(g)/pi= -0.3335 +/- 0.1118 | arg(g)/pi= 0.7119 +/- 0.1310 | arg(g)/pi= -0.4506 +/- 0.0312 |
| g_re= 0.0212 +/- 0.0140       | g_re= -0.0302 +/- 0.0133     | g_re= 0.0211 +/- 0.0131       |
| g_im= -0.0367 +/- 0.0177      | g_im= 0.0384 +/- 0.0196      | g_im= -0.1348 +/- 0.0216      |

```
corr= [-0.01]      |      corr= [ 0.59]      |      corr= [ 0.01]      |
*****
```

$$0.17 < a_t E_{\text{cm}} < 0.24$$



# k\_inv\_poly\_cccccc

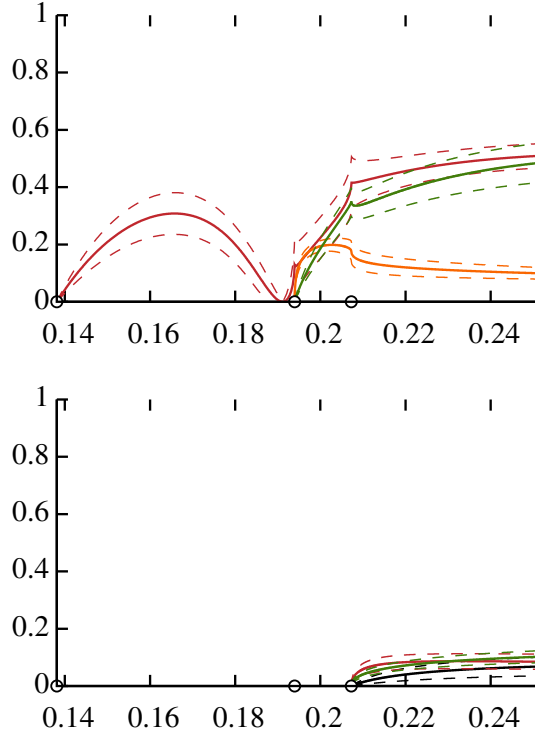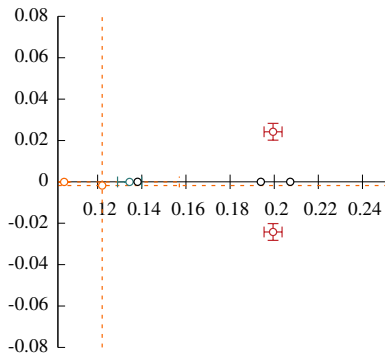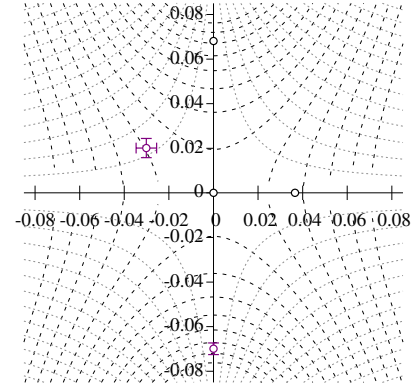

## parameter values

minimised with chisq/nDoF = 36.20 / (41 - 6) = 1.03

|                                               |                      |      |       |       |       |       |       |
|-----------------------------------------------|----------------------|------|-------|-------|-------|-------|-------|
| JPO+_c_eta:eta/1^S_0 eta:eta/1^S_0_order0     | -1.7000 +/- 0.55932  | 1.00 | 0.87  | -0.58 | 0.47  | -0.26 | -0.03 |
| JPO+_c_eta:eta/1^S_0 kaon:kaon/1^S_0_order0   | -1.0123 +/- 0.32672  | 1.00 | -0.63 | 0.84  | -0.57 | 0.13  |       |
| JPO+_c_eta:eta/1^S_0 pi:pi/1^S_0_order0       | 0.88559 +/- 0.23628  |      | 1.00  | -0.50 | 0.81  | -0.77 |       |
| JPO+_c_kaon:kaon/1^S_0 kaon:kaon/1^S_0_order0 | -0.89337 +/- 0.27262 |      |       | 1.00  | -0.75 | 0.25  |       |
| JPO+_c_kaon:kaon/1^S_0 pi:pi/1^S_0_order0     | 0.14114 +/- 0.19283  |      |       |       | 1.00  | -0.77 |       |
| JPO+_c_pi:pi/1^S_0 pi:pi/1^S_0_order0         | -0.64404 +/- 0.20345 |      |       |       |       | 1.00  |       |

## pole singularities

\*\*\*\*\*  
JP=0+ || eta:eta/1^S\_0[+] kaon:kaon/1^S\_0[+] pi:pi/1^S\_0[-]

sqrt(s)\_pole = (0.19948 +/- 0.0040978)  
+ (i/2)\*(-0.024235 +/- 0.0040586) [ 0.34]

| eta:eta/1^S_0                | kaon:kaon/1^S_0               | pi:pi/1^S_0                   |
|------------------------------|-------------------------------|-------------------------------|
| k_re= -0.0178 +/- 0.0029     | k_re= -0.0301 +/- 0.0046      | k_re= 0.0722 +/- 0.0028       |
| k_im= 0.0339 +/- 0.0052      | k_im= 0.0201 +/- 0.0043       | k_im= -0.0084 +/- 0.0015      |
| corr= [ 0.48]                | corr= [ 0.66]                 | corr= [ 0.41]                 |
| g = 0.1088 +/- 0.0169        | g = 0.1519 +/- 0.0092         | g = 0.0935 +/- 0.0079         |
| arg(g)/pi= 0.0624 +/- 0.0310 | arg(g)/pi= -0.7914 +/- 0.0331 | arg(g)/pi= -0.3743 +/- 0.0355 |
| g_re= 0.1067 +/- 0.0170      | g_re= -0.1205 +/- 0.0139      | g_re= 0.0360 +/- 0.0118       |
| g_im= 0.0212 +/- 0.0105      | g_im= -0.0926 +/- 0.0119      | g_im= -0.0864 +/- 0.0057      |
| corr= [ 0.07]                | corr= [-0.56]                 | corr= [-0.31]                 |

\*\*\*\*\*  
JP=0+ || eta:eta/1^S\_0[+] kaon:kaon/1^S\_0[-] pi:pi/1^S\_0[-]

sqrt(s)\_pole = (0.13446 +/- 0.0054616)  
+ (i/2)\*(-1.1716e-13 +/- 3.4956e-11) [-0.02]

| eta:eta/1^S_0            | kaon:kaon/1^S_0         | pi:pi/1^S_0             |
|--------------------------|-------------------------|-------------------------|
| k_re= -0.0000 +/- 0.0000 | k_re= 0.0000 +/- 0.0000 | k_re= 0.0000 +/- 0.0000 |

| eta:eta/1^S_0                | kaon:kaon/1^S_0               | pi:pi/1^S_0                  |
|------------------------------|-------------------------------|------------------------------|
| k_re= 0.0789 +/- 0.0023      | k_re= -0.0699 +/- 0.0026      | k_re= -0.0158 +/- 0.0116     |
| k_im= [ 0.02]                | k_im= [ 0.02]                 | k_im= [ 0.01]                |
| corr= [ 0.02]                | corr= [ 0.02]                 | corr= [ 0.01]                |
| g = 0.0847 +/- 0.0516        | g = 0.0303 +/- 0.0110         | g = 0.0774 +/- 0.0169        |
| arg(g)/pi= 0.5000 +/- 0.0000 | arg(g)/pi= -0.5000 +/- 0.0000 | arg(g)/pi= 0.5000 +/- 0.0000 |
| g_re= 0.0000 +/- 0.0000      | g_re= 0.0000 +/- 0.0000       | g_re= -0.0000 +/- 0.0000     |
| g_im= 0.0847 +/- 0.0516      | g_im= -0.0303 +/- 0.0110      | g_im= 0.0774 +/- 0.0169      |
| corr= [-1.00]                | corr= [ 0.93]                 | corr= [ 0.98]                |

JP=0+ || eta:eta/1^S\_0[-] kaon:kaon/1^S\_0[+] pi:pi/1^S\_0[+]

sqrt(s)\_pole = (0.12207 +/- 0.13575)  
+ (i/2)\*(-0.0017416 +/- 0.23134) [ 0.50]

| eta:eta/1^S_0                | kaon:kaon/1^S_0               | pi:pi/1^S_0                  |
|------------------------------|-------------------------------|------------------------------|
| k_re= 0.0002 +/- 0.0272      | k_re= -0.0002 +/- 0.0294      | k_re= -0.0003 +/- 0.0434     |
| k_im= -0.0837 +/- 0.0519     | k_im= 0.0753 +/- 0.0576       | k_im= 0.0315 +/- 0.1305      |
| corr= [-0.59]                | corr= [-0.59]                 | corr= [-0.51]                |
| g = 0.1244 +/- 0.9511        | g = 0.2336 +/- 1.3635         | g = 0.2617 +/- 1.6995        |
| arg(g)/pi= 0.0112 +/- 2.4950 | arg(g)/pi= -0.9997 +/- 1.5040 | arg(g)/pi= 0.0074 +/- 1.2790 |
| g_re= 0.1243 +/- 0.9192      | g_re= -0.2336 +/- 1.3627      | g_re= 0.2617 +/- 1.6947      |
| g_im= 0.0044 +/- 1.0050      | g_im= -0.0002 +/- 1.1049      | g_im= 0.0061 +/- 1.0593      |
| corr= [ 0.92]                | corr= [ 0.81]                 | corr= [ 0.21]                |

JP=0+ || eta:eta/1^S\_0[-] kaon:kaon/1^S\_0[+] pi:pi/1^S\_0[+]

sqrt(s)\_pole = (0.10521 +/- 0.12223)  
+ (i/2)\*(-0.099038 +/- 0.15227) [ 0.11]

| eta:eta/1^S_0                | kaon:kaon/1^S_0               | pi:pi/1^S_0                  |
|------------------------------|-------------------------------|------------------------------|
| k_re= 0.0139 +/- 0.0272      | k_re= -0.0151 +/- 0.0297      | k_re= -0.0233 +/- 0.0482     |
| k_im= -0.0937 +/- 0.0352     | k_im= 0.0864 +/- 0.0377       | k_im= 0.0561 +/- 0.0498      |
| corr= [ 0.40]                | corr= [ 0.41]                 | corr= [ 0.45]                |
| g = 0.1080 +/- 0.2669        | g = 0.3372 +/- 0.2764         | g = 0.2750 +/- 0.3593        |
| arg(g)/pi= 0.2961 +/- 0.4129 | arg(g)/pi= -0.7461 +/- 0.1699 | arg(g)/pi= 0.7010 +/- 0.6728 |
| g_re= 0.0646 +/- 0.2136      | g_re= -0.2355 +/- 0.2503      | g_re= -0.1623 +/- 0.4030     |
| g_im= 0.0866 +/- 0.2127      | g_im= -0.2413 +/- 0.2148      | g_im= 0.2220 +/- 0.5518      |
| corr= [ 0.59]                | corr= [ 0.41]                 | corr= [ 0.59]                |

JP=0+ || eta:eta/1^S\_0[-] kaon:kaon/1^S\_0[-] pi:pi/1^S\_0[+]

sqrt(s)\_pole = ( 0.1048 +/- 0.052226)  
+ (i/2)\*(-1.3794e-13 +/- 2.5358e-11) [ 0.04]

| eta:eta/1^S_0                | kaon:kaon/1^S_0              | pi:pi/1^S_0                   |
|------------------------------|------------------------------|-------------------------------|
| k_re= 0.0000 +/- 0.0000      | k_re= 0.0000 +/- 0.0000      | k_re= -0.0000 +/- 0.0000      |
| k_im= -0.0894 +/- 0.0152     | k_im= -0.0816 +/- 0.0167     | k_im= 0.0449 +/- 0.0303       |
| corr= [-0.03]                | corr= [-0.03]                | corr= [-0.03]                 |
| g = 0.0543 +/- 0.0326        | g = 0.0048 +/- 0.0169        | g = 0.2732 +/- 0.2677         |
| arg(g)/pi= 0.0000 +/- 0.0000 | arg(g)/pi= 1.0000 +/- 0.0000 | arg(g)/pi= -0.0000 +/- 0.0000 |
| g_re= 0.0543 +/- 0.0326      | g_re= -0.0048 +/- 0.0169     | g_re= 0.2732 +/- 0.2677       |
| g_im= 0.0000 +/- 0.0000      | g_im= 0.0000 +/- 0.0000      | g_im= -0.0000 +/- 0.0000      |
| corr= [-1.00]                | corr= [-0.99]                | corr= [ 0.58]                 |

# k\_inv\_poly\_lcccc

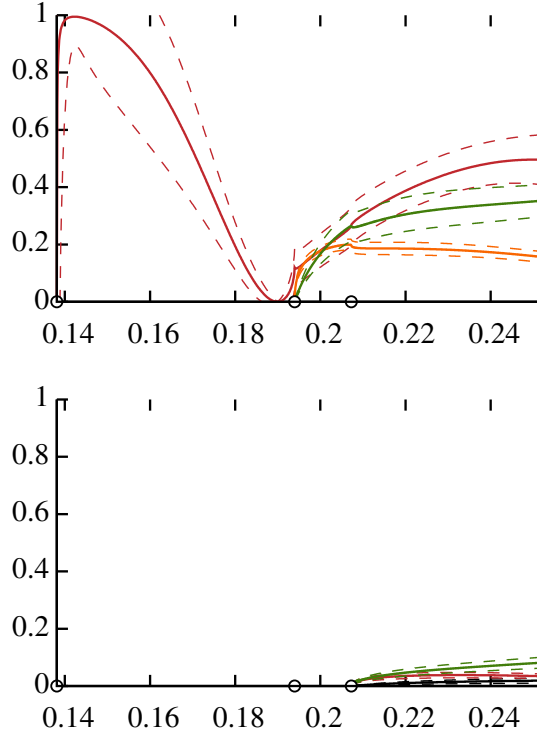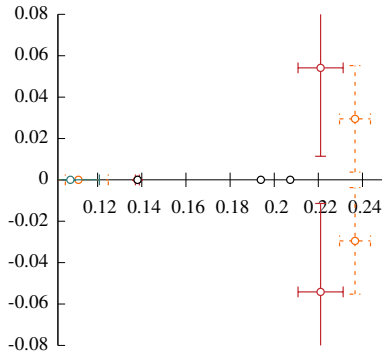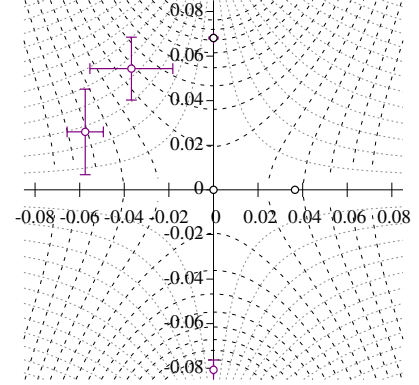

## parameter values

minimised with  $\text{chisq}/\text{nDoF} = 25.66 / (41 - 7) = 0.75$

|                                               |                      |      |      |      |       |       |       |       |
|-----------------------------------------------|----------------------|------|------|------|-------|-------|-------|-------|
| JP0+_c_eta:eta/1^S_0 eta:eta/1^S_0_order0     | -5.6765 +/- 1.0063   | 1.00 | 0.67 | 0.10 | -0.17 | 0.18  | -0.03 | -0.03 |
| JP0+_c_eta:eta/1^S_0 kaon:kaon/1^S_0_order0   | -2.7037 +/- 0.31246  | 1.00 | 0.01 | 0.61 | 0.00  | -0.03 | 0.01  |       |
| JP0+_c_eta:eta/1^S_0 pi:pi/1^S_0_order0       | 0.66572 +/- 0.54581  |      |      | 1.00 | -0.09 | 0.97  | -0.25 | -0.01 |
| JP0+_c_kaon:kaon/1^S_0 kaon:kaon/1^S_0_order0 | -1.5459 +/- 0.24186  |      |      |      | 1.00  | -0.20 | 0.00  | 0.03  |
| JP0+_c_kaon:kaon/1^S_0 pi:pi/1^S_0_order0     | -0.17490 +/- 0.28524 |      |      |      |       | 1.00  | -0.32 | 0.08  |
| JP0+_c_pi:pi/1^S_0 pi:pi/1^S_0_order0         | 1.3706 +/- 0.47352   |      |      |      |       |       | 1.00  | -0.96 |
| JP0+_c_pi:pi/1^S_0 pi:pi/1^S_0_order1         | -1.3503 +/- 0.37159  |      |      |      |       |       |       | 1.00  |

## pole singularities

\*\*\*\*\*

\*\*\*\*\*

JP=0+ || eta:eta/1^S\_0[+] kaon:kaon/1^S\_0[+] pi:pi/1^S\_0[-]

\*\*\* not found on all cfts \*\*\*

$\text{sqrt}(s)_{\text{pole}} = (0.13802 \pm 0.0008813) + (i/2) * (-2.7085e-12 \pm 6.0999e-09) [-0.01]$

| eta:eta/1^S_0                | kaon:kaon/1^S_0              | pi:pi/1^S_0                  |
|------------------------------|------------------------------|------------------------------|
| k_re= -0.0000 +/- 0.0000     | k_re= -0.0000 +/- 0.0000     | k_re= 0.0000 +/- 0.0000      |
| k_im= 0.0773 +/- 0.0004      | k_im= 0.0681 +/- 0.0004      | k_im= -0.0025 +/- 0.0110     |
| corr= [ 0.01]                | corr= [ 0.01]                | corr= [ 0.03]                |
| g = 0.5195 +/- 11.5999       | g = 0.4860 +/- 12.0163       | g = 0.4927 +/- 11.9406       |
| arg(g)/pi= 0.2563 +/- 0.2233 | arg(g)/pi= 0.2345 +/- 0.5888 | arg(g)/pi= 0.2392 +/- 0.4040 |
| g_re= 0.3600 +/- 8.3000      | g_re= 0.3600 +/- 8.3000      | g_re= 0.3600 +/- 8.3000      |
| g_im= 0.3745 +/- 8.1118      | g_im= 0.3265 +/- 8.7355      | g_im= 0.3364 +/- 8.6069      |
| corr= [ 1.00]                | corr= [ 1.00]                | corr= [ 1.00]                |

\*\*\*\*\*

\*\*\*\*\*

JP=0+ || eta:eta/1^S\_0[+] kaon:kaon/1^S\_0[+] pi:pi/1^S\_0[-]

$\text{sqrt}(s)_{\text{pole}} = (0.18197 \pm 0.026458) + (i/2) * (-0.087914 \pm 0.038523) [-0.25]$

| eta:eta/1^S_0                 | kaon:kaon/1^S_0               | pi:pi/1^S_0                   |
|-------------------------------|-------------------------------|-------------------------------|
| k_re= -0.0318 +/- 0.0168      | k_re= -0.0368 +/- 0.0186      | k_re= 0.0634 +/- 0.0180       |
| k_im= 0.0629 +/- 0.0138       | k_im= 0.0544 +/- 0.0141       | k_im= -0.0315 +/- 0.0120      |
| corr= [ 0.35]                 | corr= [ 0.30]                 | corr= [-0.09]                 |
| g = 0.1255 +/- 0.0517         | g = 0.2813 +/- 0.1040         | g = 0.2166 +/- 0.1154         |
| arg(g)/pi= -0.0052 +/- 0.0875 | arg(g)/pi= -0.9715 +/- 0.0687 | arg(g)/pi= -0.7570 +/- 0.1276 |
| g_re= 0.1254 +/- 0.0518       | g_re= -0.2801 +/- 0.1029      | g_re= -0.1565 +/- 0.0681      |
| g_im= -0.0021 +/- 0.0344      | g_im= -0.0251 +/- 0.0626      | g_im= -0.1497 +/- 0.1273      |
| corr= [ 0.05]                 | corr= [ 0.25]                 | corr= [ 0.36]                 |

JP=0+ || eta:eta/1^S\_0[+] kaon:kaon/1^S\_0[+] pi:pi/1^S\_0[-]

sqrt(s)\_pole = (0.22101 +/- 0.010224)  
+ (i/2)\*(-0.054117 +/- 0.042711) [ 0.40]

| eta:eta/1^S_0                | kaon:kaon/1^S_0               | pi:pi/1^S_0                   |
|------------------------------|-------------------------------|-------------------------------|
| k_re= -0.0477 +/- 0.0099     | k_re= -0.0575 +/- 0.0081      | k_re= 0.0869 +/- 0.0061       |
| k_im= 0.0314 +/- 0.0208      | k_im= 0.0260 +/- 0.0192       | k_im= -0.0172 +/- 0.0136      |
| corr= [-0.40]                | corr= [-0.14]                 | corr= [ 0.29]                 |
| g = 0.1045 +/- 0.0607        | g = 0.2198 +/- 0.1369         | g = 0.2169 +/- 0.1353         |
| arg(g)/pi= 0.4266 +/- 0.1348 | arg(g)/pi= -0.5143 +/- 0.1278 | arg(g)/pi= -0.1279 +/- 0.0951 |
| g_re= 0.0239 +/- 0.0414      | g_re= -0.0099 +/- 0.0863      | g_re= 0.1996 +/- 0.1218       |
| g_im= 0.1017 +/- 0.0627      | g_im= -0.2196 +/- 0.1382      | g_im= -0.0848 +/- 0.0876      |
| corr= [-0.11]                | corr= [-0.31]                 | corr= [-0.60]                 |

JP=0+ || eta:eta/1^S\_0[+] kaon:kaon/1^S\_0[-] pi:pi/1^S\_0[-]

sqrt(s)\_pole = (0.10763 +/- 0.01316)  
+ (i/2)\*(+1.3579e-12 +/- 4.0552e-10) [ 0.00]

| eta:eta/1^S_0                | kaon:kaon/1^S_0               | pi:pi/1^S_0                  |
|------------------------------|-------------------------------|------------------------------|
| k_re= 0.0000 +/- 0.0000      | k_re= -0.0000 +/- 0.0000      | k_re= -0.0000 +/- 0.0000     |
| k_im= 0.0886 +/- 0.0040      | k_im= -0.0807 +/- 0.0044      | k_im= -0.0433 +/- 0.0082     |
| corr= [-0.00]                | corr= [-0.00]                 | corr= [-0.00]                |
| g = 0.0214 +/- 0.0109        | g = 0.0185 +/- 0.0051         | g = 0.0893 +/- 0.0103        |
| arg(g)/pi= 0.5000 +/- 0.0000 | arg(g)/pi= -0.5000 +/- 0.0000 | arg(g)/pi= 0.5000 +/- 0.0000 |
| g_re= 0.0000 +/- 0.0000      | g_re= 0.0000 +/- 0.0000       | g_re= -0.0000 +/- 0.0000     |
| g_im= 0.0214 +/- 0.0109      | g_im= -0.0185 +/- 0.0051      | g_im= 0.0893 +/- 0.0103      |
| corr= [-1.00]                | corr= [ 0.07]                 | corr= [ 0.06]                |

JP=0+ || eta:eta/1^S\_0[-] kaon:kaon/1^S\_0[+] pi:pi/1^S\_0[+]

sqrt(s)\_pole = ( 0.1434 +/- 0.021454)  
+ (i/2)\*(-0.14308 +/- 0.033768) [-0.81]

| eta:eta/1^S_0                | kaon:kaon/1^S_0               | pi:pi/1^S_0                   |
|------------------------------|-------------------------------|-------------------------------|
| k_re= 0.0292 +/- 0.0112      | k_re= -0.0317 +/- 0.0120      | k_re= -0.0464 +/- 0.0141      |
| k_im= -0.0879 +/- 0.0038     | k_im= 0.0809 +/- 0.0039       | k_im= 0.0553 +/- 0.0055       |
| corr= [ 0.39]                | corr= [ 0.26]                 | corr= [-0.54]                 |
| g = 0.1084 +/- 0.0218        | g = 0.2890 +/- 0.0122         | g = 0.0691 +/- 0.0113         |
| arg(g)/pi= 0.1944 +/- 0.0267 | arg(g)/pi= -0.7489 +/- 0.0233 | arg(g)/pi= -0.9825 +/- 0.0513 |
| g_re= 0.0888 +/- 0.0159      | g_re= -0.2037 +/- 0.0149      | g_re= -0.0690 +/- 0.0111      |
| g_im= 0.0622 +/- 0.0175      | g_im= -0.2051 +/- 0.0194      | g_im= -0.0038 +/- 0.0114      |
| corr= [ 0.79]                | corr= [-0.52]                 | corr= [ 0.36]                 |

JP=0+ || eta:eta/1^S\_0[-] kaon:kaon/1^S\_0[+] pi:pi/1^S\_0[-]

sqrt(s)\_pole = (0.087565 +/- 0.017808)  
+ (i/2)\*(+1.5811e-15 +/- 2.1212e-12) [-0.04]

| eta:eta/1^S_0                | kaon:kaon/1^S_0               | pi:pi/1^S_0                  |
|------------------------------|-------------------------------|------------------------------|
| k_re= -0.0000 +/- 0.0000     | k_re= 0.0000 +/- 0.0000       | k_re= -0.0000 +/- 0.0000     |
| k_im= -0.0939 +/- 0.0042     | k_im= 0.0865 +/- 0.0045       | k_im= -0.0534 +/- 0.0073     |
| corr= [ 0.04]                | corr= [ 0.04]                 | corr= [ 0.04]                |
| g = 0.0367 +/- 0.0112        | g = 0.1136 +/- 0.0347         | g = 0.0546 +/- 0.0203        |
| arg(g)/pi= 0.5000 +/- 0.0000 | arg(g)/pi= -0.5000 +/- 0.0000 | arg(g)/pi= 0.5000 +/- 0.0000 |
| g_re= 0.0000 +/- 0.0000      | g_re= 0.0000 +/- 0.0000       | g_re= -0.0000 +/- 0.0000     |
| g_im= 0.0367 +/- 0.0112      | g_im= -0.1136 +/- 0.0347      | g_im= 0.0546 +/- 0.0203      |
| corr= [-1.00]                | corr= [ 0.12]                 | corr= [-0.23]                |

JP=0+ || eta:eta/1^S\_0[-] kaon:kaon/1^S\_0[+] pi:pi/1^S\_0[-]

```

sqrt(s)_pole = ( 0.2366 +/- 0.0070153)
               + (i/2)*(-0.029473 +/- 0.025749) [-0.44]

=====
eta:eta/1^S_0 | kaon:kaon/1^S_0 | pi:pi/1^S_0 |
=====
k_re= 0.0585 +/- 0.0081 | k_re= -0.0685 +/- 0.0066 | k_re= 0.0962 +/- 0.0044 |
k_im= -0.0149 +/- 0.0119 | k_im= 0.0127 +/- 0.0106 | k_im= -0.0091 +/- 0.0078 |
corr= [-0.58] | corr= [-0.54] | corr= [-0.47] |
=====
|g|= 0.0965 +/- 0.0201 | |g|= 0.2005 +/- 0.0338 | |g|= 0.1569 +/- 0.0296 |
arg(g)/pi= 0.3693 +/- 0.0475 | arg(g)/pi= -0.5370 +/- 0.0211 | arg(g)/pi= -0.0630 +/- 0.0310 |
=====
g_re= 0.0385 +/- 0.0170 | g_re= -0.0232 +/- 0.0118 | g_re= 0.1538 +/- 0.0269 |
g_im= 0.0885 +/- 0.0180 | g_im= -0.1992 +/- 0.0343 | g_im= -0.0308 +/- 0.0196 |
corr= [ 0.39] | corr= [-0.25] | corr= [-0.81] |
=====

```

```

*****
JP=0+ || eta:eta/1^S_0[-] kaon:kaon/1^S_0[-] pi:pi/1^S_0[-]

```

```

sqrt(s)_pole = (0.24876 +/- 0.014798)
               + (i/2)*(-0.14945 +/- 0.036142) [-0.89]

=====
eta:eta/1^S_0 | kaon:kaon/1^S_0 | pi:pi/1^S_0 |
=====
k_re= 0.0813 +/- 0.0126 | k_re= 0.0868 +/- 0.0118 | k_re= 0.1060 +/- 0.0093 |
k_im= -0.0572 +/- 0.0086 | k_im= -0.0535 +/- 0.0090 | k_im= -0.0439 +/- 0.0094 |
corr= [-0.88] | corr= [-0.89] | corr= [-0.90] |
=====
|g|= 0.0379 +/- 0.0082 | |g|= 0.0676 +/- 0.0074 | |g|= 0.1811 +/- 0.0256 |
arg(g)/pi= -0.3646 +/- 0.1125 | arg(g)/pi= 0.5063 +/- 0.0403 | arg(g)/pi= 0.0129 +/- 0.0095 |
=====
g_re= 0.0156 +/- 0.0150 | g_re= -0.0013 +/- 0.0086 | g_re= 0.1809 +/- 0.0254 |
g_im= -0.0345 +/- 0.0048 | g_im= 0.0676 +/- 0.0074 | g_im= 0.0073 +/- 0.0064 |
corr= [-0.18] | corr= [-0.14] | corr= [ 0.99] |
=====

```

```

*****
JP=0+ || eta:eta/1^S_0[-] kaon:kaon/1^S_0[-] pi:pi/1^S_0[-]

```

```

sqrt(s)_pole = (0.11127 +/- 0.01355)
               + (i/2)*(+1.2764e-16 +/- 1.9057e-13) [-0.02]

=====
eta:eta/1^S_0 | kaon:kaon/1^S_0 | pi:pi/1^S_0 |
=====
k_re= -0.0000 +/- 0.0000 | k_re= -0.0000 +/- 0.0000 | k_re= -0.0000 +/- 0.0000 |
k_im= -0.0874 +/- 0.0043 | k_im= -0.0794 +/- 0.0047 | k_im= -0.0409 +/- 0.0092 |
corr= [ 0.02] | corr= [ 0.02] | corr= [ 0.02] |
=====
|g|= 0.0116 +/- 0.0063 | |g|= 0.0124 +/- 0.0045 | |g|= 0.0936 +/- 0.0093 |
arg(g)/pi= 0.5000 +/- 0.0000 | arg(g)/pi= -0.5000 +/- 0.0000 | arg(g)/pi= 0.5000 +/- 0.0000 |
=====
g_re= 0.0000 +/- 0.0000 | g_re= 0.0000 +/- 0.0000 | g_re= -0.0000 +/- 0.0000 |
g_im= 0.0116 +/- 0.0063 | g_im= -0.0124 +/- 0.0045 | g_im= 0.0936 +/- 0.0093 |
corr= [-1.00] | corr= [-0.51] | corr= [ 0.46] |
=====

```

# k\_inv\_poly\_ccclcc

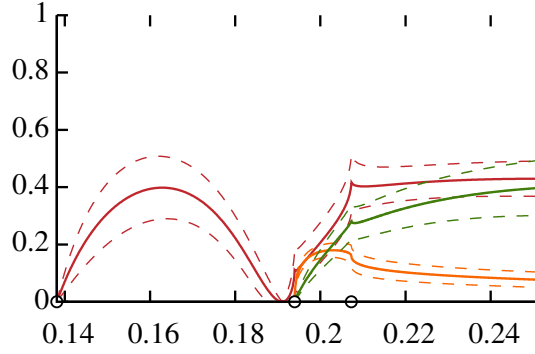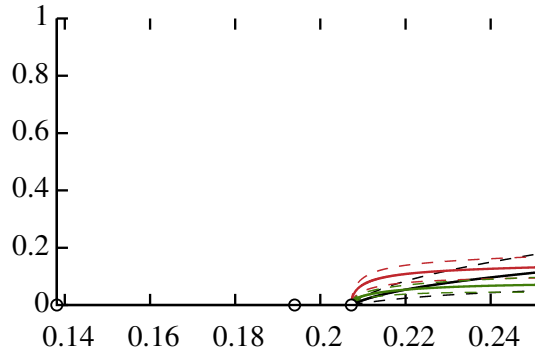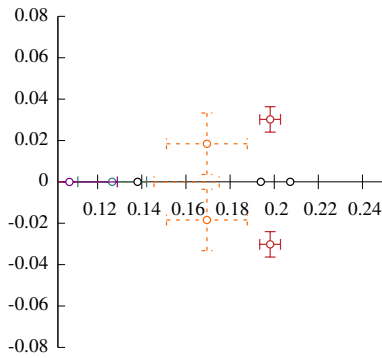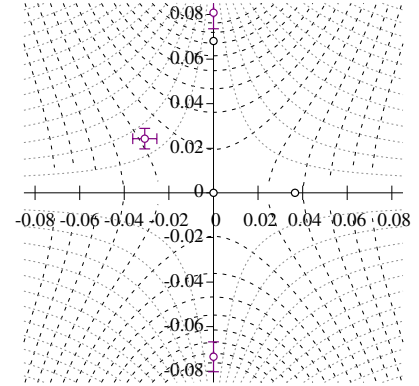

## parameter values

minimised with  $\text{chisq}/\text{nDoF} = 31.51 / (41 - 7) = 0.93$

|                                               |                      |      |       |       |       |       |       |      |
|-----------------------------------------------|----------------------|------|-------|-------|-------|-------|-------|------|
| JPO+_c_eta:eta/1^S_0 eta:eta/1^S_0_order0     | -1.2344 +/- 0.51916  | 1.00 | 0.92  | -0.73 | 0.57  | -0.36 | -0.43 | 0.14 |
| JPO+_c_eta:eta/1^S_0 kaon:kaon/1^S_0_order0   | -0.71450 +/- 0.30775 | 1.00 | -0.74 | 0.74  | -0.41 | -0.62 | 0.24  |      |
| JPO+_c_eta:eta/1^S_0 pi:pi/1^S_0_order0       | 0.75249 +/- 0.23366  |      | 1.00  | -0.51 | 0.28  | 0.81  | -0.74 |      |
| JPO+_c_kaon:kaon/1^S_0 kaon:kaon/1^S_0_order0 | -0.27993 +/- 0.4113  |      |       | 1.00  | -0.86 | -0.69 | 0.20  |      |
| JPO+_c_kaon:kaon/1^S_0 kaon:kaon/1^S_0_order1 | -0.44568 +/- 0.27612 |      |       |       | 1.00  | 0.40  | -0.03 |      |
| JPO+_c_kaon:kaon/1^S_0 pi:pi/1^S_0_order0     | 0.025023 +/- 0.1857  |      |       |       |       | 1.00  | -0.75 |      |
| JPO+_c_pi:pi/1^S_0 pi:pi/1^S_0_order0         | -0.63911 +/- 0.18992 |      |       |       |       |       | 1.00  |      |

## pole singularities

\*\*\*\*\*  
JP=0+ || eta:eta/1^S\_0| kaon:kaon/1^S\_0| pi:pi/1^S\_0|

$\text{sqrt}(s)_{\text{pole}} = (0.10724 \pm 0.021684) + (i/2)*(-2.2301e-13 \pm 6.1251e-11) [0.04]$

| eta:eta/1^S_0                | kaon:kaon/1^S_0               | pi:pi/1^S_0                   |
|------------------------------|-------------------------------|-------------------------------|
| k_re= -0.0000 +/- 0.0000     | k_re= -0.0000 +/- 0.0000      | k_re= -0.0000 +/- 0.0000      |
| k_im= 0.0887 +/- 0.0066      | k_im= 0.0808 +/- 0.0072       | k_im= 0.0435 +/- 0.0134       |
| corr= [-0.04]                | corr= [-0.04]                 | corr= [-0.04]                 |
| g = 0.0345 +/- 0.0371        | g = 0.1408 +/- 0.0317         | g = 0.1640 +/- 0.0374         |
| arg(g)/pi= 0.0000 +/- 0.0000 | arg(g)/pi= -0.0000 +/- 0.0000 | arg(g)/pi= -0.0000 +/- 0.0000 |
| g_re= 0.0345 +/- 0.0371      | g_re= 0.1408 +/- 0.0317       | g_re= 0.1640 +/- 0.0374       |
| g_im= 0.0000 +/- 0.0000      | g_im= -0.0000 +/- 0.0000      | g_im= -0.0000 +/- 0.0000      |
| corr= [-1.00]                | corr= [-0.65]                 | corr= [-0.81]                 |

\*\*\*\*\*

JP=0+ || eta:eta/1^S\_0| kaon:kaon/1^S\_0| pi:pi/1^S\_0|

$\text{sqrt}(s)_{\text{pole}} = (0.19817 \pm 0.0047054) + (i/2)*(-0.030188 \pm 0.0061231) [-0.01]$

| eta:eta/1^S_0 | kaon:kaon/1^S_0 | pi:pi/1^S_0 |
|---------------|-----------------|-------------|
|---------------|-----------------|-------------|

| eta:eta/1^S_0                 | kaon:kaon/1^S_0               | pi:pi/1^S_0                   |
|-------------------------------|-------------------------------|-------------------------------|
| k_re= -0.0201 +/- 0.0043      | k_re= -0.0308 +/- 0.0054      | k_re= 0.0714 +/- 0.0032       |
| k_im= 0.0372 +/- 0.0050       | k_im= 0.0243 +/- 0.0046       | k_im= -0.0105 +/- 0.0021      |
| corr= [ 0.38]                 | corr= [ 0.38]                 | corr= [ 0.05]                 |
| g = 0.1194 +/- 0.0250         | g = 0.1471 +/- 0.0113         | g = 0.1024 +/- 0.0136         |
| arg(g)/pi= -0.0147 +/- 0.0626 | arg(g)/pi= -0.8288 +/- 0.0383 | arg(g)/pi= -0.4176 +/- 0.0431 |
| g_re= 0.1193 +/- 0.0249       | g_re= -0.1263 +/- 0.0121      | g_re= 0.0262 +/- 0.0144       |
| g_im= -0.0055 +/- 0.0236      | g_im= -0.0753 +/- 0.0172      | g_im= -0.0990 +/- 0.0131      |
| corr= [-0.10]                 | corr= [-0.31]                 | corr= [-0.13]                 |

JP=0+ || eta:eta/1^S\_0 kaon:kaon/1^S\_0 pi:pi/1^S\_0

sqrt(s)\_pole = ( 0.1266 +/- 0.015579)  
+ (i/2)\*(+2.2083e-13 +/- 4.5357e-11) [ 0.02]

| eta:eta/1^S_0                | kaon:kaon/1^S_0               | pi:pi/1^S_0                  |
|------------------------------|-------------------------------|------------------------------|
| k_re= 0.0000 +/- 0.0000      | k_re= -0.0000 +/- 0.0000      | k_re= -0.0000 +/- 0.0000     |
| k_im= 0.0821 +/- 0.0060      | k_im= -0.0735 +/- 0.0067      | k_im= -0.0276 +/- 0.0178     |
| corr= [-0.02]                | corr= [-0.02]                 | corr= [-0.02]                |
| g = 0.1376 +/- 0.0850        | g = 0.0424 +/- 0.0101         | g = 0.0861 +/- 0.0045        |
| arg(g)/pi= 0.5000 +/- 0.0000 | arg(g)/pi= -0.5000 +/- 0.0000 | arg(g)/pi= 0.5000 +/- 0.0000 |
| g_re= 0.0000 +/- 0.0000      | g_re= 0.0000 +/- 0.0000       | g_re= -0.0000 +/- 0.0000     |
| g_im= 0.1376 +/- 0.0850      | g_im= -0.0424 +/- 0.0101      | g_im= 0.0861 +/- 0.0045      |
| corr= [-1.00]                | corr= [ 0.78]                 | corr= [ 0.88]                |

JP=0+ || eta:eta/1^S\_0 kaon:kaon/1^S\_0 pi:pi/1^S\_0

sqrt(s)\_pole = (0.08099 +/- 0.064535)  
+ (i/2)\*(+9.9221e-11 +/- 2.952e-08) [ 0.03]

| eta:eta/1^S_0                | kaon:kaon/1^S_0               | pi:pi/1^S_0                   |
|------------------------------|-------------------------------|-------------------------------|
| k_re= -0.0000 +/- 0.0000     | k_re= 0.0000 +/- 0.0000       | k_re= 0.0000 +/- 0.0000       |
| k_im= -0.0954 +/- 0.0135     | k_im= 0.0881 +/- 0.0146       | k_im= 0.0559 +/- 0.0230       |
| corr= [-0.03]                | corr= [-0.03]                 | corr= [-0.03]                 |
| g = 0.0330 +/- 0.0489        | g = 0.0671 +/- 0.0989         | g = 0.2993 +/- 0.3885         |
| arg(g)/pi= 0.0000 +/- 0.0000 | arg(g)/pi= -0.0000 +/- 0.0000 | arg(g)/pi= -0.0000 +/- 0.0000 |
| g_re= 0.0330 +/- 0.0489      | g_re= 0.0671 +/- 0.0989       | g_re= 0.2993 +/- 0.3885       |
| g_im= 0.0000 +/- 0.0000      | g_im= -0.0000 +/- 0.0000      | g_im= -0.0000 +/- 0.0000      |
| corr= [-0.99]                | corr= [-0.97]                 | corr= [ 0.82]                 |

JP=0+ || eta:eta/1^S\_0 kaon:kaon/1^S\_0 pi:pi/1^S\_0

sqrt(s)\_pole = ( 0.1695 +/- 0.018299)  
+ (i/2)\*(-0.018407 +/- 0.014859) [-0.30]

| eta:eta/1^S_0                 | kaon:kaon/1^S_0              | pi:pi/1^S_0                   |
|-------------------------------|------------------------------|-------------------------------|
| k_re= 0.0065 +/- 0.0061       | k_re= -0.0081 +/- 0.0081     | k_re= 0.0495 +/- 0.0156       |
| k_im= -0.0602 +/- 0.0124      | k_im= 0.0481 +/- 0.0152      | k_im= -0.0079 +/- 0.0060      |
| corr= [ 0.54]                 | corr= [ 0.60]                | corr= [-0.09]                 |
| g = 0.0729 +/- 0.0261         | g = 0.2041 +/- 0.0663        | g = 0.0634 +/- 0.0203         |
| arg(g)/pi= -0.1257 +/- 0.0402 | arg(g)/pi= 0.9957 +/- 0.0344 | arg(g)/pi= -0.4436 +/- 0.0669 |
| g_re= 0.0673 +/- 0.0266       | g_re= -0.2041 +/- 0.0660     | g_re= 0.0112 +/- 0.0114       |
| g_im= -0.0281 +/- 0.0075      | g_im= 0.0028 +/- 0.0228      | g_im= -0.0624 +/- 0.0214      |
| corr= [-0.48]                 | corr= [-0.78]                | corr= [ 0.44]                 |

JP=0+ || eta:eta/1^S\_0 kaon:kaon/1^S\_0 pi:pi/1^S\_0

sqrt(s)\_pole = (0.09367 +/- 0.081374)  
+ (i/2)\*(-9.1583e-12 +/- 2.7695e-09) [-0.02]

| eta:eta/1^S_0                | kaon:kaon/1^S_0              | pi:pi/1^S_0                   |
|------------------------------|------------------------------|-------------------------------|
| k_re= 0.0000 +/- 0.0000      | k_re= 0.0000 +/- 0.0000      | k_re= -0.0000 +/- 0.0000      |
| k_im= -0.0924 +/- 0.0203     | k_im= -0.0849 +/- 0.0221     | k_im= 0.0507 +/- 0.0369       |
| corr= [ 0.02]                | corr= [ 0.02]                | corr= [ 0.01]                 |
| g = 0.0534 +/- 0.0301        | g = 0.0088 +/- 0.0206        | g = 0.3185 +/- 0.4363         |
| arg(g)/pi= 0.0000 +/- 0.0000 | arg(g)/pi= 1.0000 +/- 0.0000 | arg(g)/pi= -0.0000 +/- 0.0000 |
| g_re= 0.0534 +/- 0.0301      | g_re= -0.0088 +/- 0.0206     | g_re= 0.3185 +/- 0.4363       |
| g_im= 0.0000 +/- 0.0000      | g_im= 0.0000 +/- 0.0000      | g_im= -0.0000 +/- 0.0000      |
| corr= [-1.00]                | corr= [-0.98]                | corr= [-0.57]                 |

# k\_inv\_poly\_cccccc\_noCM

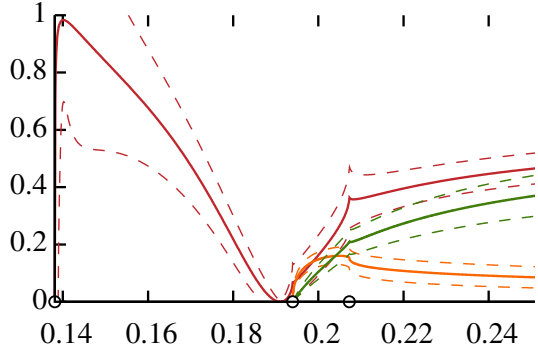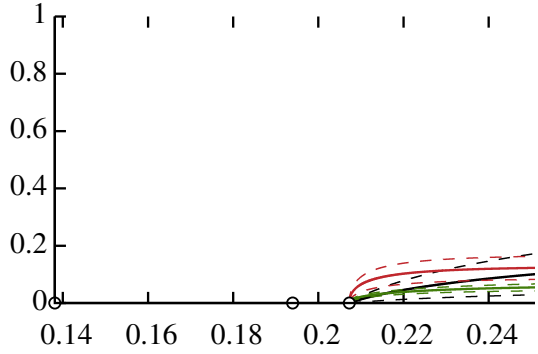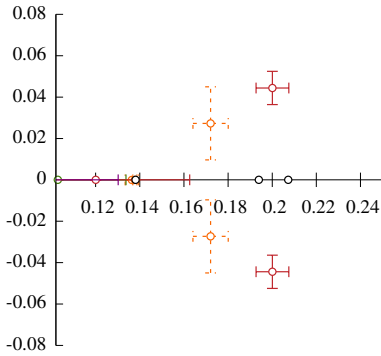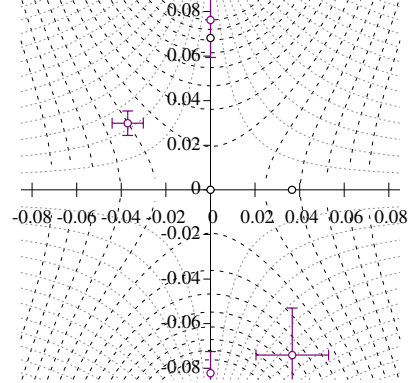

## parameter values

minimised with  $\text{chisq}/\text{nDoF} = 28.50 / (41 - 6) = 0.81$

|                                               |                       |      |       |       |       |       |      |
|-----------------------------------------------|-----------------------|------|-------|-------|-------|-------|------|
| JP0+_c_eta:eta/1^S_0 eta:eta/1^S_0_order0     | -1.2139 +/- 0.64711   | 1.00 | 0.95  | -0.79 | 0.68  | -0.58 | 0.46 |
| JP0+_c_eta:eta/1^S_0 kaon:kaon/1^S_0_order0   | -0.65140 +/- 0.36375  | 1.00 | -0.81 | 0.85  | -0.67 | 0.53  |      |
| JP0+_c_eta:eta/1^S_0 pi:pi/1^S_0_order0       | 0.72605 +/- 0.3459    |      | 1.00  | -0.67 | 0.91  | -0.88 |      |
| JP0+_c_kaon:kaon/1^S_0 kaon:kaon/1^S_0_order0 | -0.71086 +/- 0.22906  |      |       | 1.00  | -0.74 | 0.53  |      |
| JP0+_c_kaon:kaon/1^S_0 pi:pi/1^S_0_order0     | -0.083643 +/- 0.22939 |      |       |       | 1.00  | -0.91 |      |
| JP0+_c_pi:pi/1^S_0 pi:pi/1^S_0_order0         | -0.11888 +/- 0.25689  |      |       |       |       | 1.00  |      |

## pole singularities

\*\*\*\*\*  
JP=0+ || eta:eta/1^S\_0[+] kaon:kaon/1^S\_0[+] pi:pi/1^S\_0[+]

$\text{sqrt}(s)_{\text{pole}} = (0.091402 \pm 0.038816)$   
 $+ (i/2) * (2.183e-17 \pm 6.5277e-15) [-0.02]$

| eta:eta/1^S_0                | kaon:kaon/1^S_0               | pi:pi/1^S_0                  |
|------------------------------|-------------------------------|------------------------------|
| k_re= 0.0000 +/- 0.0000      | k_re= 0.0000 +/- 0.0000       | k_re= 0.0000 +/- 0.0000      |
| k_im= 0.0930 +/- 0.0096      | k_im= 0.0855 +/- 0.0104       | k_im= 0.0518 +/- 0.0173      |
| corr= [ 0.02]                | corr= [ 0.02]                 | corr= [ 0.02]                |
| g = 0.0641 +/- 0.0370        | g = 0.0328 +/- 0.0172         | g = 0.0431 +/- 0.0300        |
| arg(g)/pi= 0.0000 +/- 0.0000 | arg(g)/pi= -0.0000 +/- 0.0000 | arg(g)/pi= 1.0000 +/- 0.0000 |
| g_re= 0.0641 +/- 0.0370      | g_re= 0.0328 +/- 0.0172       | g_re= -0.0431 +/- 0.0300     |
| g_im= 0.0000 +/- 0.0000      | g_im= -0.0000 +/- 0.0000      | g_im= 0.0000 +/- 0.0000      |
| corr= [-1.00]                | corr= [ 0.64]                 | corr= [ 0.28]                |

\*\*\*\*\*  
JP=0+ || eta:eta/1^S\_0[+] kaon:kaon/1^S\_0[+] pi:pi/1^S\_0[-]

$\text{sqrt}(s)_{\text{pole}} = (0.2001 \pm 0.0074284)$   
 $+ (i/2) * (-0.044409 \pm 0.0080406) [-0.02]$

| eta:eta/1^S_0            | kaon:kaon/1^S_0          | pi:pi/1^S_0             |
|--------------------------|--------------------------|-------------------------|
| k_re= -0.0276 +/- 0.0060 | k_re= -0.0371 +/- 0.0070 | k_re= 0.0731 +/- 0.0050 |



```

k_im= 0.0402 +/- 0.0064 | k_im= 0.0299 +/- 0.0055 | k_im= -0.0152 +/- 0.0027 |
corr= [ 0.55] | corr= [ 0.51] | corr= [ 0.10] |
=====|=====|=====|
|g|= 0.1298 +/- 0.0286 | |g|= 0.1464 +/- 0.0240 | |g|= 0.1372 +/- 0.0197 |
arg(g)/pi= -0.0202 +/- 0.0641 | arg(g)/pi= -0.8306 +/- 0.0523 | arg(g)/pi= -0.4198 +/- 0.0586 |
-----|-----|-----|
g_re= 0.1295 +/- 0.0289 | g_re= -0.1262 +/- 0.0259 | g_re= 0.0342 +/- 0.0267 |
g_im= -0.0082 +/- 0.0258 | g_im= -0.0743 +/- 0.0221 | g_im= -0.1328 +/- 0.0177 |
corr= [ 0.20] | corr= [-0.09] | corr= [-0.23] |
*****

```

```

*****
JP=0+ || eta:eta/1^S_0[+] kaon:kaon/1^S_0[+] pi:pi/1^S_0[-]

```

```

sqrt(s)_pole = (0.12003 +/- 0.04258)
+ (i/2)*(+5.0073e-13 +/- 1.4874e-10) [-0.01]

```

```

eta:eta/1^S_0 | kaon:kaon/1^S_0 | pi:pi/1^S_0 |
=====|=====|=====|
k_re= 0.0000 +/- 0.0000 | k_re= 0.0000 +/- 0.0000 | k_re= -0.0000 +/- 0.0000 |
k_im= 0.0845 +/- 0.0152 | k_im= 0.0762 +/- 0.0168 | k_im= -0.0341 +/- 0.0380 |
corr= [ 0.01] | corr= [ 0.01] | corr= [ 0.01] |
-----|-----|-----|
|g|= 0.0881 +/- 0.0370 | |g|= 0.1149 +/- 0.1312 | |g|= 0.0794 +/- 0.1033 |
arg(g)/pi= 0.0000 +/- 0.0000 | arg(g)/pi= -0.0000 +/- 0.0000 | arg(g)/pi= -0.0000 +/- 0.0000 |
-----|-----|-----|
g_re= 0.0881 +/- 0.0370 | g_re= 0.1149 +/- 0.1312 | g_re= 0.0794 +/- 0.1033 |
g_im= 0.0000 +/- 0.0000 | g_im= -0.0000 +/- 0.0000 | g_im= -0.0000 +/- 0.0000 |
corr= [-1.00] | corr= [-0.75] | corr= [-0.85] |
*****

```

```

*****
JP=0+ || eta:eta/1^S_0[+] kaon:kaon/1^S_0[-] pi:pi/1^S_0[+]

```

```

sqrt(s)_pole = (0.10286 +/- 0.030912)
+ (i/2)*(+1.9012e-17 +/- 5.6753e-15) [-0.01]

```

```

eta:eta/1^S_0 | kaon:kaon/1^S_0 | pi:pi/1^S_0 |
=====|=====|=====|
k_re= 0.0000 +/- 0.0000 | k_re= -0.0000 +/- 0.0000 | k_re= 0.0000 +/- 0.0000 |
k_im= 0.0900 +/- 0.0089 | k_im= -0.0822 +/- 0.0097 | k_im= 0.0461 +/- 0.0174 |
corr= [ 0.01] | corr= [ 0.01] | corr= [ 0.01] |
-----|-----|-----|
|g|= 0.0723 +/- 0.0215 | |g|= 0.0179 +/- 0.0079 | |g|= 0.0695 +/- 0.0276 |
arg(g)/pi= 0.0000 +/- 0.0000 | arg(g)/pi= 1.0000 +/- 0.0000 | arg(g)/pi= 1.0000 +/- 0.0000 |
-----|-----|-----|
g_re= 0.0723 +/- 0.0215 | g_re= -0.0179 +/- 0.0079 | g_re= -0.0695 +/- 0.0276 |
g_im= 0.0000 +/- 0.0000 | g_im= 0.0000 +/- 0.0000 | g_im= 0.0000 +/- 0.0000 |
corr= [-1.00] | corr= [-0.80] | corr= [ 0.06] |
*****

```

```

*****
JP=0+ || eta:eta/1^S_0[+] kaon:kaon/1^S_0[-] pi:pi/1^S_0[-]

```

```

sqrt(s)_pole = (0.16013 +/- 0.039504)
+ (i/2)*(-0.13598 +/- 0.063728) [ 0.29]

```

```

eta:eta/1^S_0 | kaon:kaon/1^S_0 | pi:pi/1^S_0 |
=====|=====|=====|
k_re= -0.0335 +/- 0.0150 | k_re= 0.0367 +/- 0.0163 | k_re= 0.0546 +/- 0.0210 |
k_im= 0.0813 +/- 0.0202 | k_im= -0.0741 +/- 0.0211 | k_im= -0.0499 +/- 0.0213 |
corr= [ 0.22] | corr= [ 0.26] | corr= [ 0.36] |
-----|-----|-----|
|g|= 0.1802 +/- 0.0585 | |g|= 0.0815 +/- 0.0274 | |g|= 0.1523 +/- 0.0482 |
arg(g)/pi= -0.1707 +/- 0.1629 | arg(g)/pi= 0.6411 +/- 0.1184 | arg(g)/pi= -0.5317 +/- 0.0788 |
-----|-----|-----|
g_re= 0.1549 +/- 0.0737 | g_re= -0.0349 +/- 0.0279 | g_re= -0.0151 +/- 0.0362 |
g_im= -0.0921 +/- 0.0806 | g_im= 0.0736 +/- 0.0299 | g_im= -0.1516 +/- 0.0494 |
corr= [ 0.44] | corr= [ 0.19] | corr= [-0.28] |
*****

```

```

*****
JP=0+ || eta:eta/1^S_0[-] kaon:kaon/1^S_0[+] pi:pi/1^S_0[+]

```

```

sqrt(s)_pole = (0.13778 +/- 0.00090723)
+ (i/2)*(-5.7589e-12 +/- 1.6864e-09) [-0.05]

```

```

eta:eta/1^S_0 | kaon:kaon/1^S_0 | pi:pi/1^S_0 |
=====|=====|=====|
k_re= 0.0000 +/- 0.0000 | k_re= -0.0000 +/- 0.0000 | k_re= -0.0000 +/- 0.0000 |
k_im= -0.0774 +/- 0.0004 | k_im= 0.0683 +/- 0.0005 | k_im= 0.0049 +/- 0.0064 |
corr= [ 0.05] | corr= [ 0.05] | corr= [ 0.05] |
-----|-----|-----|
|g|= 0.0069 +/- 0.0067 | |g|= 0.0312 +/- 0.0262 | |g|= 0.0503 +/- 0.0308 |
arg(g)/pi= 0.0000 +/- 0.0001 | arg(g)/pi= -0.0000 +/- 0.0001 | arg(g)/pi= -0.0000 +/- 0.0001 |
-----|-----|-----|
g_re= 0.0069 +/- 0.0067 | g_re= 0.0312 +/- 0.0262 | g_re= 0.0503 +/- 0.0308 |
g_im= 0.0000 +/- 0.0000 | g_im= -0.0000 +/- 0.0000 | g_im= -0.0000 +/- 0.0000 |
corr= [-1.00] | corr= [-0.52] | corr= [-0.13] |
*****

```

```

*****
JP=0+ || eta:eta/1^S_0[-] kaon:kaon/1^S_0[+] pi:pi/1^S_0[-]

```

```

sqrt(s)_pole = (0.17208 +/- 0.0080123)
+ (i/2)*(-0.027313 +/- 0.01764) [-0.31]

```

| eta:eta/1^S_0                 |  | kaon:kaon/1^S_0               |  | pi:pi/1^S_0                   |  |
|-------------------------------|--|-------------------------------|--|-------------------------------|--|
| k_re= 0.0100 +/- 0.0067       |  | k_re= -0.0125 +/- 0.0084      |  | k_re= 0.0521 +/- 0.0068       |  |
| k_im= -0.0590 +/- 0.0053      |  | k_im= 0.0470 +/- 0.0064       |  | k_im= -0.0113 +/- 0.0069      |  |
| corr= [ 0.23]                 |  | corr= [ 0.18]                 |  | corr= [-0.32]                 |  |
| -----                         |  |                               |  |                               |  |
| g = 0.0603 +/- 0.0149         |  | g = 0.1655 +/- 0.0063         |  | g = 0.0859 +/- 0.0268         |  |
| arg(g)/pi= -0.2039 +/- 0.0409 |  | arg(g)/pi= -0.9950 +/- 0.0171 |  | arg(g)/pi= -0.5540 +/- 0.0319 |  |
| -----                         |  |                               |  |                               |  |
| g_re= 0.0483 +/- 0.0148       |  | g_re= -0.1655 +/- 0.0063      |  | g_re= -0.0145 +/- 0.0089      |  |
| g_im= -0.0360 +/- 0.0078      |  | g_im= -0.0026 +/- 0.0089      |  | g_im= -0.0847 +/- 0.0268      |  |
| corr= [-0.52]                 |  | corr= [ 0.26]                 |  | corr= [ 0.29]                 |  |

\*\*\*\*\*  
JP=0+ || eta:eta/1^S\_0[-] kaon:kaon/1^S\_0[-] pi:pi/1^S\_0[-]

sqrt(s)\_pole = (0.13644 +/- 0.0030804)  
+ (i/2)\*(-1.0005e-15 +/- 2.994e-13) [-0.02]

| eta:eta/1^S_0                |  | kaon:kaon/1^S_0               |  | pi:pi/1^S_0                  |  |
|------------------------------|--|-------------------------------|--|------------------------------|--|
| k_re= 0.0000 +/- 0.0000      |  | k_re= 0.0000 +/- 0.0000       |  | k_re= 0.0000 +/- 0.0000      |  |
| k_im= -0.0780 +/- 0.0013     |  | k_im= -0.0689 +/- 0.0015      |  | k_im= -0.0107 +/- 0.0097     |  |
| corr= [ 0.02]                |  | corr= [ 0.02]                 |  | corr= [ 0.02]                |  |
| -----                        |  |                               |  |                              |  |
| g = 0.0264 +/- 0.0064        |  | g = 0.0136 +/- 0.0111         |  | g = 0.0737 +/- 0.0296        |  |
| arg(g)/pi= 0.5000 +/- 0.0000 |  | arg(g)/pi= -0.5000 +/- 0.0000 |  | arg(g)/pi= 0.5000 +/- 0.0000 |  |
| -----                        |  |                               |  |                              |  |
| g_re= 0.0000 +/- 0.0000      |  | g_re= 0.0000 +/- 0.0000       |  | g_re= -0.0000 +/- 0.0000     |  |
| g_im= 0.0264 +/- 0.0064      |  | g_im= -0.0136 +/- 0.0111      |  | g_im= 0.0737 +/- 0.0296      |  |
| corr= [-1.00]                |  | corr= [-0.82]                 |  | corr= [-0.07]                |  |

# k\_inv\_poly\_clcccc\_noCM

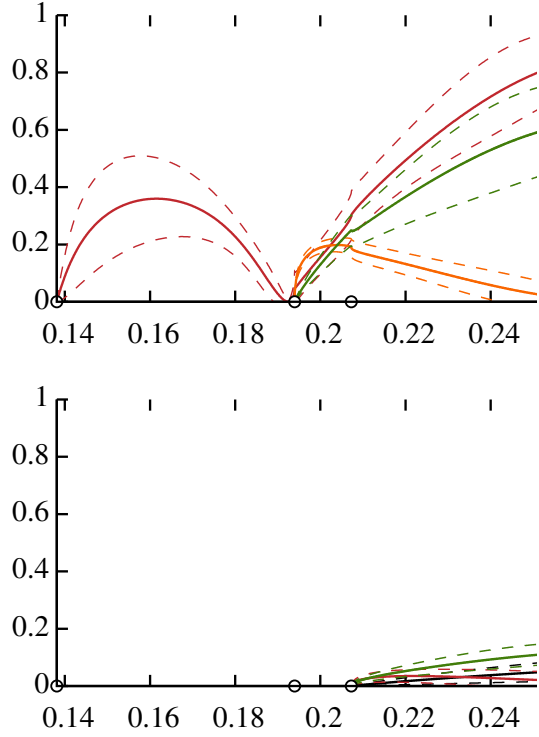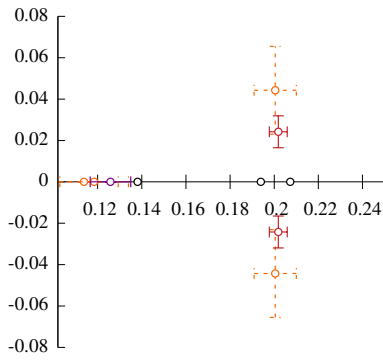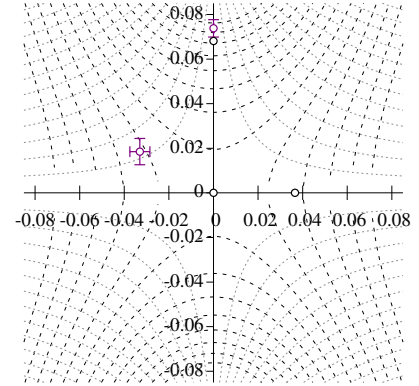

## parameter values

minimised with  $\chi^2/\text{nDoF} = 25.49 / (41 - 7) = 0.75$

|                                               |                      |      |       |       |       |       |       |       |
|-----------------------------------------------|----------------------|------|-------|-------|-------|-------|-------|-------|
| JP0+_c_eta:eta/1^S_0 eta:eta/1^S_0_order0     | -3.6898 +/- 1.4024   | 1.00 | 0.77  | 0.16  | -0.07 | 0.29  | -0.18 | -0.38 |
| JP0+_c_eta:eta/1^S_0 kaon:kaon/1^S_0_order0   | -1.7632 +/- 0.46229  | 1.00 | -0.07 | 0.56  | 0.05  | -0.11 | -0.11 |       |
| JP0+_c_eta:eta/1^S_0 pi:pi/1^S_0_order0       | 0.62404 +/- 0.48031  |      | 1.00  | -0.35 | 0.81  | -0.40 | -0.92 |       |
| JP0+_c_kaon:kaon/1^S_0 kaon:kaon/1^S_0_order0 | -1.0701 +/- 0.32583  |      |       | 1.00  | -0.39 | 0.16  | 0.35  |       |
| JP0+_c_kaon:kaon/1^S_0 pi:pi/1^S_0_order0     | -0.86398 +/- 0.48354 |      |       |       | 1.00  | -0.84 | -0.83 |       |
| JP0+_c_kaon:kaon/1^S_0 pi:pi/1^S_0_order1     | 0.59482 +/- 0.278    |      |       |       |       | 1.00  | 0.47  |       |
| JP0+_c_pi:pi/1^S_0 pi:pi/1^S_0_order0         | 0.20433 +/- 0.17784  |      |       |       |       |       | 1.00  |       |

## pole singularities

\*\*\*\*\*  
JP=0+ || eta:eta/1^S\_0[+] kaon:kaon/1^S\_0[+] pi:pi/1^S\_0[+]

$\sqrt{s}_{\text{pole}} = (0.1258 \pm 0.0091935) + (i/2) * (5.8084e-14 \pm 1.7369e-11) [0.07]$

| eta:eta/1^S_0                | kaon:kaon/1^S_0              | pi:pi/1^S_0                  |
|------------------------------|------------------------------|------------------------------|
| k_re= 0.0000 +/- 0.0000      | k_re= 0.0000 +/- 0.0000      | k_re= 0.0000 +/- 0.0000      |
| k_im= 0.0824 +/- 0.0035      | k_im= 0.0738 +/- 0.0039      | k_im= 0.0285 +/- 0.0102      |
| corr= [-0.07]                | corr= [-0.07]                | corr= [-0.07]                |
| g = 0.0299 +/- 0.0182        | g = 0.0751 +/- 0.0082        | g = 0.0984 +/- 0.0056        |
| arg(g)/pi= 0.0000 +/- 0.0000 | arg(g)/pi= 1.0000 +/- 0.0000 | arg(g)/pi= 1.0000 +/- 0.0000 |
| g_re= 0.0299 +/- 0.0182      | g_re= -0.0751 +/- 0.0082     | g_re= -0.0984 +/- 0.0056     |
| g_im= 0.0000 +/- 0.0000      | g_im= 0.0000 +/- 0.0000      | g_im= 0.0000 +/- 0.0000      |
| corr= [-1.00]                | corr= [-0.26]                | corr= [0.39]                 |

\*\*\*\*\*

\*\*\*\*\*  
JP=0+ || eta:eta/1^S\_0[+] kaon:kaon/1^S\_0[+] pi:pi/1^S\_0[-]

$\sqrt{s}_{\text{pole}} = (0.20186 \pm 0.0040414) + (i/2) * (-0.024208 \pm 0.0077167) [0.36]$

| eta:eta/1^S_0 | kaon:kaon/1^S_0 | pi:pi/1^S_0 |
|---------------|-----------------|-------------|
|---------------|-----------------|-------------|

| eta:eta/1^S_0                | kaon:kaon/1^S_0               | pi:pi/1^S_0                   |
|------------------------------|-------------------------------|-------------------------------|
| k_re= -0.0196 +/- 0.0043     | k_re= -0.0330 +/- 0.0045      | k_re= 0.0738 +/- 0.0027       |
| k_im= 0.0312 +/- 0.0063      | k_im= 0.0185 +/- 0.0059       | k_im= -0.0083 +/- 0.0027      |
| corr= [-0.08]                | corr= [ 0.27]                 | corr= [ 0.37]                 |
| g = 0.0662 +/- 0.0173        | g = 0.1298 +/- 0.0136         | g = 0.0923 +/- 0.0135         |
| arg(g)/pi= 0.1311 +/- 0.0704 | arg(g)/pi= -0.8079 +/- 0.0287 | arg(g)/pi= -0.3691 +/- 0.0344 |
| g_re= 0.0607 +/- 0.0197      | g_re= -0.1069 +/- 0.0158      | g_re= 0.0369 +/- 0.0086       |
| g_im= 0.0265 +/- 0.0113      | g_im= -0.0736 +/- 0.0085      | g_im= -0.0846 +/- 0.0144      |
| corr= [-0.28]                | corr= [-0.06]                 | corr= [ 0.05]                 |

JP=0+ || eta:eta/1^S\_0 kaon:kaon/1^S\_0 pi:pi/1^S\_0

sqrt(s)\_pole = (0.076021 +/- 0.012567)  
+ (i/2)\*(-0.059474 +/- 0.058933) [-0.52]

| eta:eta/1^S_0                 | kaon:kaon/1^S_0              | pi:pi/1^S_0                   |
|-------------------------------|------------------------------|-------------------------------|
| k_re= -0.0058 +/- 0.0062      | k_re= 0.0062 +/- 0.0067      | k_re= 0.0094 +/- 0.0098       |
| k_im= 0.0977 +/- 0.0024       | k_im= -0.0907 +/- 0.0026     | k_im= -0.0603 +/- 0.0044      |
| corr= [-0.41]                 | corr= [-0.43]                | corr= [-0.56]                 |
| g = 0.0654 +/- 0.0154         | g = 0.0474 +/- 0.0095        | g = 0.0580 +/- 0.0150         |
| arg(g)/pi= -0.3105 +/- 0.0812 | arg(g)/pi= 0.5320 +/- 0.1780 | arg(g)/pi= -0.5646 +/- 0.2354 |
| g_re= 0.0367 +/- 0.0154       | g_re= -0.0048 +/- 0.0267     | g_re= -0.0117 +/- 0.0429      |
| g_im= -0.0542 +/- 0.0167      | g_im= 0.0472 +/- 0.0090      | g_im= -0.0568 +/- 0.0149      |
| corr= [ 0.12]                 | corr= [-0.07]                | corr= [-0.25]                 |

JP=0+ || eta:eta/1^S\_0 kaon:kaon/1^S\_0 pi:pi/1^S\_0

sqrt(s)\_pole = (0.11841 +/- 0.015558)  
+ (i/2)\*(+1.1296e-17 +/- 3.3792e-15) [ 0.05]

| eta:eta/1^S_0                | kaon:kaon/1^S_0              | pi:pi/1^S_0                  |
|------------------------------|------------------------------|------------------------------|
| k_re= -0.0000 +/- 0.0000     | k_re= 0.0000 +/- 0.0000      | k_re= 0.0000 +/- 0.0000      |
| k_im= -0.0851 +/- 0.0054     | k_im= 0.0768 +/- 0.0060      | k_im= 0.0355 +/- 0.0130      |
| corr= [-0.05]                | corr= [-0.05]                | corr= [-0.05]                |
| g = 0.0210 +/- 0.0087        | g = 0.0930 +/- 0.0055        | g = 0.0905 +/- 0.0069        |
| arg(g)/pi= 0.0000 +/- 0.0000 | arg(g)/pi= 1.0000 +/- 0.0000 | arg(g)/pi= 1.0000 +/- 0.0000 |
| g_re= 0.0210 +/- 0.0087      | g_re= -0.0930 +/- 0.0055     | g_re= -0.0905 +/- 0.0069     |
| g_im= 0.0000 +/- 0.0000      | g_im= 0.0000 +/- 0.0000      | g_im= 0.0000 +/- 0.0000      |
| corr= [-1.00]                | corr= [ 0.09]                | corr= [-0.75]                |

JP=0+ || eta:eta/1^S\_0 kaon:kaon/1^S\_0 pi:pi/1^S\_0

sqrt(s)\_pole = (0.20047 +/- 0.009567)  
+ (i/2)\*(-0.044271 +/- 0.021227) [ 0.63]

| eta:eta/1^S_0                | kaon:kaon/1^S_0               | pi:pi/1^S_0                   |
|------------------------------|-------------------------------|-------------------------------|
| k_re= 0.0278 +/- 0.0066      | k_re= -0.0374 +/- 0.0067      | k_re= 0.0734 +/- 0.0060       |
| k_im= -0.0399 +/- 0.0133     | k_im= 0.0297 +/- 0.0135       | k_im= -0.0151 +/- 0.0075      |
| corr= [-0.23]                | corr= [ 0.22]                 | corr= [ 0.61]                 |
| g = 0.0720 +/- 0.0244        | g = 0.1642 +/- 0.0284         | g = 0.1092 +/- 0.0224         |
| arg(g)/pi= 0.0752 +/- 0.1138 | arg(g)/pi= -0.8253 +/- 0.0593 | arg(g)/pi= -0.3471 +/- 0.0597 |
| g_re= 0.0700 +/- 0.0284      | g_re= -0.1401 +/- 0.0390      | g_re= 0.0504 +/- 0.0141       |
| g_im= 0.0169 +/- 0.0214      | g_im= -0.0857 +/- 0.0149      | g_im= -0.0968 +/- 0.0269      |
| corr= [-0.68]                | corr= [-0.70]                 | corr= [ 0.35]                 |

JP=0+ || eta:eta/1^S\_0 kaon:kaon/1^S\_0 pi:pi/1^S\_0

sqrt(s)\_pole = (0.11379 +/- 0.015537)  
+ (i/2)\*(+7.3193e-14 +/- 2.1908e-11) [ 0.04]

| eta:eta/1^S_0                | kaon:kaon/1^S_0               | pi:pi/1^S_0                  |
|------------------------------|-------------------------------|------------------------------|
| k_re= -0.0000 +/- 0.0000     | k_re= -0.0000 +/- 0.0000      | k_re= -0.0000 +/- 0.0000     |
| k_im= -0.0866 +/- 0.0051     | k_im= -0.0785 +/- 0.0056      | k_im= -0.0391 +/- 0.0113     |
| corr= [-0.04]                | corr= [-0.04]                 | corr= [-0.04]                |
| g = 0.0290 +/- 0.0118        | g = 0.0489 +/- 0.0086         | g = 0.1041 +/- 0.0082        |
| arg(g)/pi= 0.5000 +/- 0.0000 | arg(g)/pi= -0.5000 +/- 0.0000 | arg(g)/pi= 0.5000 +/- 0.0000 |
| g_re= 0.0000 +/- 0.0000      | g_re= 0.0000 +/- 0.0000       | g_re= -0.0000 +/- 0.0000     |
| g_im= 0.0290 +/- 0.0118      | g_im= -0.0489 +/- 0.0086      | g_im= 0.1041 +/- 0.0082      |
| corr= [-1.00]                | corr= [-0.76]                 | corr= [ 0.66]                |

# k\_inv\_poly\_ccclcc\_noCM

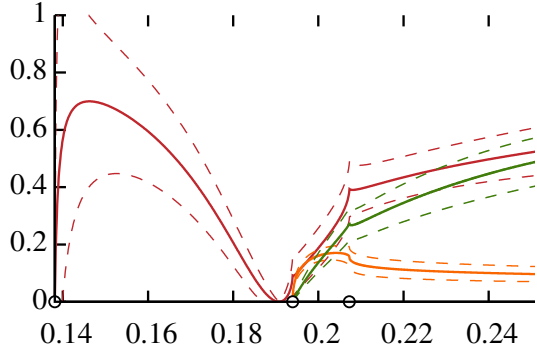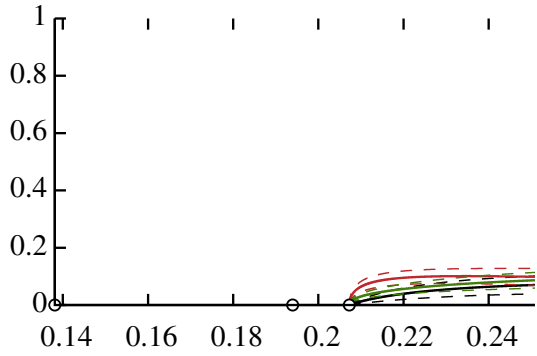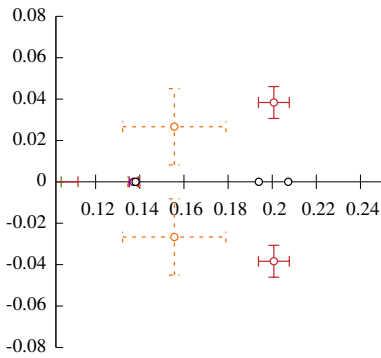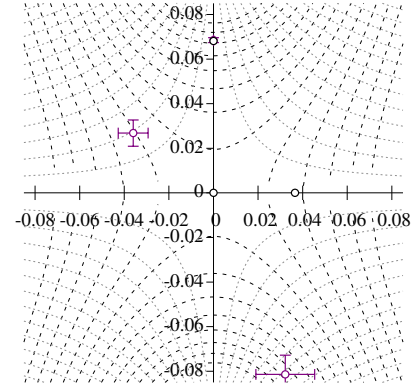

## parameter values

minimised with  $\chi^2/\text{nDoF} = 26.30 / (41 - 7) = 0.77$

|                                               |                      |      |       |       |       |       |       |      |
|-----------------------------------------------|----------------------|------|-------|-------|-------|-------|-------|------|
| JPO+_c_eta:eta/1^S_0 eta:eta/1^S_0_order0     | -1.6440 +/- 0.53864  | 1.00 | 0.86  | -0.65 | 0.33  | -0.14 | -0.35 | 0.08 |
| JPO+_c_eta:eta/1^S_0 kaon:kaon/1^S_0_order0   | -0.95289 +/- 0.31642 | 1.00 | -0.63 | 0.68  | -0.37 | -0.63 | 0.16  |      |
| JPO+_c_eta:eta/1^S_0 pi:pi/1^S_0_order0       | 0.93109 +/- 0.24208  |      | 1.00  | -0.23 | 0.01  | 0.75  | -0.77 |      |
| JPO+_c_kaon:kaon/1^S_0 kaon:kaon/1^S_0_order0 | -1.3705 +/- 0.47588  |      |       | 1.00  | -0.87 | -0.65 | 0.03  |      |
| JPO+_c_kaon:kaon/1^S_0 kaon:kaon/1^S_0_order1 | 0.45573 +/- 0.28128  |      |       |       | 1.00  | 0.38  | 0.11  |      |
| JPO+_c_kaon:kaon/1^S_0 pi:pi/1^S_0_order0     | 0.11893 +/- 0.19329  |      |       |       |       | 1.00  | -0.67 |      |
| JPO+_c_pi:pi/1^S_0 pi:pi/1^S_0_order0         | -0.20745 +/- 0.20166 |      |       |       |       |       | 1.00  |      |

## pole singularities

\*\*\*\*\*  
JP=0+ || eta:eta/1^S\_0[+] kaon:kaon/1^S\_0[+] pi:pi/1^S\_0[+]

sqrt(s)\_pole = (0.13725 +/- 0.0021127)  
+ (i/2)\*(-1.0278e-15 +/- 3.0617e-13) [ 0.01]

| eta:eta/1^S_0                | kaon:kaon/1^S_0              | pi:pi/1^S_0                  |
|------------------------------|------------------------------|------------------------------|
| k_re= -0.0000 +/- 0.0000     | k_re= -0.0000 +/- 0.0000     | k_re= -0.0000 +/- 0.0000     |
| k_im= 0.0777 +/- 0.0009      | k_im= 0.0685 +/- 0.0011      | k_im= 0.0077 +/- 0.0094      |
| corr= [-0.01]                | corr= [-0.01]                | corr= [-0.01]                |
| g = 0.0015 +/- 0.0139        | g = 0.0539 +/- 0.4184        | g = 0.0545 +/- 0.4207        |
| arg(g)/pi= 0.0011 +/- 0.0280 | arg(g)/pi= 0.9974 +/- 0.2096 | arg(g)/pi= 0.9974 +/- 0.2091 |
| g_re= 0.0015 +/- 0.0139      | g_re= -0.0539 +/- 0.4183     | g_re= -0.0545 +/- 0.4207     |
| g_im= 0.0000 +/- 0.0001      | g_im= 0.0004 +/- 0.0361      | g_im= 0.0004 +/- 0.0364      |
| corr= [-0.59]                | corr= [-0.22]                | corr= [-0.22]                |

\*\*\*\*\*  
JP=0+ || eta:eta/1^S\_0[+] kaon:kaon/1^S\_0[+] pi:pi/1^S\_0[-]

sqrt(s)\_pole = (0.20075 +/- 0.0070033)  
+ (i/2)\*(-0.038348 +/- 0.0077096) [ 0.17]

| eta:eta/1^S_0 | kaon:kaon/1^S_0 | pi:pi/1^S_0 |
|---------------|-----------------|-------------|
|---------------|-----------------|-------------|

|                          |                          |                          |
|--------------------------|--------------------------|--------------------------|
| k_re= -0.0256 +/- 0.0055 | k_re= -0.0360 +/- 0.0067 | k_re= 0.0734 +/- 0.0047  |
| k_im= 0.0376 +/- 0.0070  | k_im= 0.0268 +/- 0.0059  | k_im= -0.0131 +/- 0.0027 |
| corr= [ 0.52]            | corr= [ 0.54]            | corr= [ 0.26]            |

---

|                              |                               |                               |
|------------------------------|-------------------------------|-------------------------------|
| g = 0.1240 +/- 0.0152        | g = 0.1610 +/- 0.0188         | g = 0.1270 +/- 0.0175         |
| arg(g)/pi= 0.0331 +/- 0.0630 | arg(g)/pi= -0.7952 +/- 0.0533 | arg(g)/pi= -0.3875 +/- 0.0653 |

---

|                         |                          |                          |
|-------------------------|--------------------------|--------------------------|
| g_re= 0.1234 +/- 0.0148 | g_re= -0.1288 +/- 0.0229 | g_re= 0.0439 +/- 0.0261  |
| g_im= 0.0129 +/- 0.0248 | g_im= -0.0966 +/- 0.0236 | g_im= -0.1191 +/- 0.0175 |
| corr= [ 0.08]           | corr= [-0.35]            | corr= [ 0.15]            |

\*\*\*\*\*  
JP=0+ || eta:eta/1^S\_0[+] kaon:kaon/1^S\_0[+] pi:pi/1^S\_0[-]

sqrt(s)\_pole = (0.088076 +/- 0.023905)  
+ (i/2)\*(+5.1445e-13 +/- 1.5406e-10) [-0.03]

| eta:eta/1^S_0           | kaon:kaon/1^S_0         | pi:pi/1^S_0              |
|-------------------------|-------------------------|--------------------------|
| k_re= 0.0000 +/- 0.0000 | k_re= 0.0000 +/- 0.0000 | k_re= -0.0000 +/- 0.0000 |
| k_im= 0.0938 +/- 0.0056 | k_im= 0.0864 +/- 0.0061 | k_im= -0.0532 +/- 0.0099 |
| corr= [ 0.03]           | corr= [ 0.03]           | corr= [ 0.03]            |

---

|                              |                               |                               |
|------------------------------|-------------------------------|-------------------------------|
| g = 0.0556 +/- 0.0222        | g = 0.0699 +/- 0.0352         | g = 0.0424 +/- 0.0284         |
| arg(g)/pi= 0.0000 +/- 0.0000 | arg(g)/pi= -0.0000 +/- 0.0000 | arg(g)/pi= -0.0000 +/- 0.0000 |

---

|                         |                          |                          |
|-------------------------|--------------------------|--------------------------|
| g_re= 0.0556 +/- 0.0222 | g_re= 0.0699 +/- 0.0352  | g_re= 0.0424 +/- 0.0284  |
| g_im= 0.0000 +/- 0.0000 | g_im= -0.0000 +/- 0.0000 | g_im= -0.0000 +/- 0.0000 |
| corr= [-1.00]           | corr= [ 0.27]            | corr= [ 0.13]            |

\*\*\*\*\*  
JP=0+ || eta:eta/1^S\_0[+] kaon:kaon/1^S\_0[-] pi:pi/1^S\_0[+]

sqrt(s)\_pole = (0.08736 +/- 0.017044)  
+ (i/2)\*(+4.3669e-16 +/- 1.3061e-13) [-0.01]

| eta:eta/1^S_0           | kaon:kaon/1^S_0          | pi:pi/1^S_0             |
|-------------------------|--------------------------|-------------------------|
| k_re= 0.0000 +/- 0.0000 | k_re= -0.0000 +/- 0.0000 | k_re= 0.0000 +/- 0.0000 |
| k_im= 0.0940 +/- 0.0040 | k_im= -0.0866 +/- 0.0043 | k_im= 0.0535 +/- 0.0070 |
| corr= [ 0.01]           | corr= [ 0.01]            | corr= [ 0.01]           |

---

|                              |                              |                              |
|------------------------------|------------------------------|------------------------------|
| g = 0.0625 +/- 0.0153        | g = 0.0203 +/- 0.0050        | g = 0.0548 +/- 0.0168        |
| arg(g)/pi= 0.0000 +/- 0.0000 | arg(g)/pi= 1.0000 +/- 0.0000 | arg(g)/pi= 1.0000 +/- 0.0000 |

---

|                         |                          |                          |
|-------------------------|--------------------------|--------------------------|
| g_re= 0.0625 +/- 0.0153 | g_re= -0.0203 +/- 0.0050 | g_re= -0.0548 +/- 0.0168 |
| g_im= 0.0000 +/- 0.0000 | g_im= 0.0000 +/- 0.0000  | g_im= 0.0000 +/- 0.0000  |
| corr= [-1.00]           | corr= [ 0.19]            | corr= [ 0.11]            |

\*\*\*\*\*  
JP=0+ || eta:eta/1^S\_0[+] kaon:kaon/1^S\_0[-] pi:pi/1^S\_0[-]

sqrt(s)\_pole = (0.14346 +/- 0.027959)  
+ (i/2)\*(-0.14606 +/- 0.039704) [-0.39]

| eta:eta/1^S_0            | kaon:kaon/1^S_0          | pi:pi/1^S_0              |
|--------------------------|--------------------------|--------------------------|
| k_re= -0.0296 +/- 0.0123 | k_re= 0.0322 +/- 0.0132  | k_re= 0.0467 +/- 0.0163  |
| k_im= 0.0884 +/- 0.0083  | k_im= -0.0814 +/- 0.0086 | k_im= -0.0560 +/- 0.0095 |
| corr= [ 0.35]            | corr= [ 0.31]            | corr= [-0.02]            |

---

|                               |                              |                               |
|-------------------------------|------------------------------|-------------------------------|
| g = 0.1656 +/- 0.0480         | g = 0.0679 +/- 0.0178        | g = 0.1458 +/- 0.0381         |
| arg(g)/pi= -0.2384 +/- 0.0768 | arg(g)/pi= 0.6292 +/- 0.0723 | arg(g)/pi= -0.5418 +/- 0.0394 |

---

|                          |                          |                          |
|--------------------------|--------------------------|--------------------------|
| g_re= 0.1213 +/- 0.0503  | g_re= -0.0268 +/- 0.0156 | g_re= -0.0191 +/- 0.0176 |
| g_im= -0.1127 +/- 0.0370 | g_im= 0.0624 +/- 0.0176  | g_im= -0.1446 +/- 0.0383 |
| corr= [-0.17]            | corr= [-0.08]            | corr= [ 0.02]            |

\*\*\*\*\*  
JP=0+ || eta:eta/1^S\_0[-] kaon:kaon/1^S\_0[+] pi:pi/1^S\_0[+]

sqrt(s)\_pole = (0.13721 +/- 0.0026447)  
+ (i/2)\*(+1.946e-16 +/- 5.9302e-14) [-0.02]

| eta:eta/1^S_0            | kaon:kaon/1^S_0         | pi:pi/1^S_0             |
|--------------------------|-------------------------|-------------------------|
| k_re= -0.0000 +/- 0.0000 | k_re= 0.0000 +/- 0.0000 | k_re= 0.0000 +/- 0.0000 |
| k_im= -0.0777 +/- 0.0012 | k_im= 0.0685 +/- 0.0013 | k_im= 0.0079 +/- 0.0114 |
| corr= [ 0.02]            | corr= [ 0.02]           | corr= [ 0.02]           |

---

|                              |                              |                              |
|------------------------------|------------------------------|------------------------------|
| g = 0.0025 +/- 0.0252        | g = 0.0603 +/- 0.4273        | g = 0.0544 +/- 0.4052        |
| arg(g)/pi= 0.0005 +/- 0.0148 | arg(g)/pi= 0.9989 +/- 0.1772 | arg(g)/pi= 0.9989 +/- 0.1967 |

---

|                         |                          |                          |
|-------------------------|--------------------------|--------------------------|
| g_re= 0.0025 +/- 0.0252 | g_re= -0.0603 +/- 0.4273 | g_re= -0.0544 +/- 0.4052 |
| g_im= 0.0000 +/- 0.0001 | g_im= 0.0002 +/- 0.0339  | g_im= 0.0002 +/- 0.0340  |
| corr= [-0.52]           | corr= [-0.25]            | corr= [-0.28]            |

\*\*\*\*\*  
JP=0+ || eta:eta/1^S\_0[-] kaon:kaon/1^S\_0[+] pi:pi/1^S\_0[-]

sqrt(s)\_pole = (0.15564 +/- 0.023402)  
+ (i/2)\*(-0.026654 +/- 0.018434) [-0.32]

| eta:eta/1^S_0                 | kaon:kaon/1^S_0              | pi:pi/1^S_0                   |
|-------------------------------|------------------------------|-------------------------------|
| k_re= 0.0075 +/- 0.0063       | k_re= -0.0088 +/- 0.0078     | k_re= 0.0378 +/- 0.0228       |
| k_im= -0.0692 +/- 0.0126      | k_im= 0.0589 +/- 0.0146      | k_im= -0.0137 +/- 0.0088      |
| corr= [ 0.59]                 | corr= [ 0.63]                | corr= [ 0.27]                 |
| g = 0.0755 +/- 0.0106         | g = 0.1908 +/- 0.0251        | g = 0.0854 +/- 0.0219         |
| arg(g)/pi= -0.1777 +/- 0.0475 | arg(g)/pi= 0.9800 +/- 0.0211 | arg(g)/pi= -0.5535 +/- 0.0629 |
| g_re= 0.0640 +/- 0.0091       | g_re= -0.1904 +/- 0.0252     | g_re= -0.0143 +/- 0.0182      |
| g_im= -0.0400 +/- 0.0125      | g_im= 0.0120 +/- 0.0124      | g_im= -0.0842 +/- 0.0208      |
| corr= [-0.08]                 | corr= [ 0.08]                | corr= [ 0.41]                 |

\*\*\*\*\*

\*\*\*\*\*

JP=0+ || eta:eta/1^S\_0[-] kaon:kaon/1^S\_0[-] pi:pi/1^S\_0[-]

sqrt(s)\_pole = (0.13702 +/- 0.0018142)  
+ (i/2)\*(+1.3187e-13 +/- 3.9466e-11) [-0.01]

| eta:eta/1^S_0                | kaon:kaon/1^S_0               | pi:pi/1^S_0                  |
|------------------------------|-------------------------------|------------------------------|
| k_re= -0.0000 +/- 0.0000     | k_re= -0.0000 +/- 0.0000      | k_re= -0.0000 +/- 0.0000     |
| k_im= -0.0778 +/- 0.0008     | k_im= -0.0686 +/- 0.0009      | k_im= -0.0087 +/- 0.0071     |
| corr= [ 0.01]                | corr= [ 0.01]                 | corr= [ 0.01]                |
| g = 0.0250 +/- 0.0070        | g = 0.0074 +/- 0.0061         | g = 0.0671 +/- 0.0255        |
| arg(g)/pi= 0.5000 +/- 0.0000 | arg(g)/pi= -0.5000 +/- 0.0000 | arg(g)/pi= 0.5000 +/- 0.0000 |
| g_re= 0.0000 +/- 0.0000      | g_re= 0.0000 +/- 0.0000       | g_re= -0.0000 +/- 0.0000     |
| g_im= 0.0250 +/- 0.0070      | g_im= -0.0074 +/- 0.0061      | g_im= 0.0671 +/- 0.0255      |
| corr= [-1.00]                | corr= [-0.73]                 | corr= [ 0.50]                |

\*\*\*\*\*

# k\_poly\_lcccc

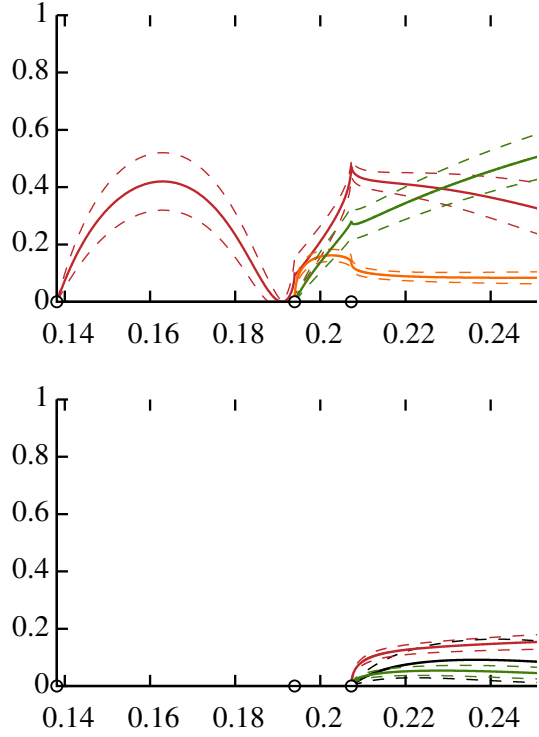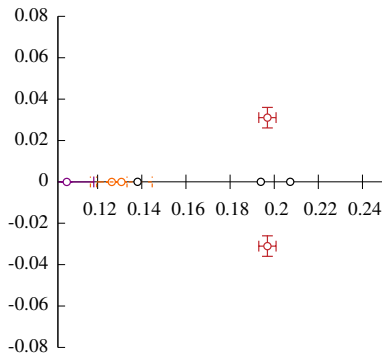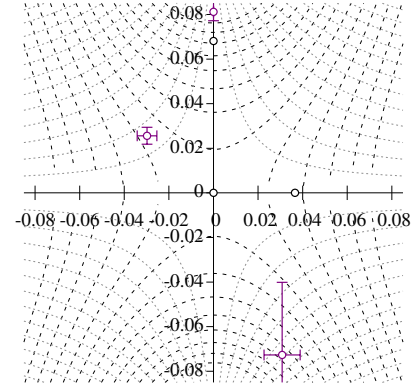

## parameter values

minimised with  $\text{chisq}/\text{nDoF} = 30.95 / (41 - 7) = 0.91$

|                                                   |                     |      |       |       |       |       |       |       |
|---------------------------------------------------|---------------------|------|-------|-------|-------|-------|-------|-------|
| JPO+_gamma_eta:eta/1^S_0 eta:eta/1^S_0_order0     | 6.9914 +/- 1.1917   | 1.00 | -0.49 | 0.68  | -0.29 | -0.03 | 0.28  | 0.09  |
| JPO+_gamma_eta:eta/1^S_0 kaon:kaon/1^S_0_order0   | -5.0077 +/- 0.47082 | 1.00 | -0.46 | -0.56 | 0.57  | -0.34 | 0.00  |       |
| JPO+_gamma_eta:eta/1^S_0 pi:pi/1^S_0_order0       | 7.2313 +/- 0.99886  |      | 1.00  | -0.21 | -0.48 | 0.79  | 0.43  |       |
| JPO+_gamma_kaon:kaon/1^S_0 kaon:kaon/1^S_0_order0 | 2.2764 +/- 0.58318  |      |       | 1.00  | -0.64 | 0.05  | -0.13 |       |
| JPO+_gamma_kaon:kaon/1^S_0 pi:pi/1^S_0_order0     | -5.1644 +/- 0.60017 |      |       |       | 1.00  | -0.71 | -0.25 |       |
| JPO+_gamma_pi:pi/1^S_0 pi:pi/1^S_0_order0         | 4.3439 +/- 1.0058   |      |       |       |       | 1.00  | 0.07  |       |
| JPO+_gamma_pi:pi/1^S_0 pi:pi/1^S_0_order1         | 1.2522 +/- 0.54095  |      |       |       |       |       | 1.00  |       |
| JPO+_gamma_eta:eta/1^S_0 eta:eta/1^S_0_order1     | 0.0000 +/- 0        |      |       |       |       |       |       | FIXED |
| JPO+_gamma_eta:eta/1^S_0 kaon:kaon/1^S_0_order1   | 0.0000 +/- 0        |      |       |       |       |       |       | FIXED |
| JPO+_gamma_eta:eta/1^S_0 pi:pi/1^S_0_order1       | 0.0000 +/- 0        |      |       |       |       |       |       | FIXED |
| JPO+_gamma_kaon:kaon/1^S_0 kaon:kaon/1^S_0_order1 | 0.0000 +/- 0        |      |       |       |       |       |       | FIXED |
| JPO+_gamma_kaon:kaon/1^S_0 pi:pi/1^S_0_order1     | 0.0000 +/- 0        |      |       |       |       |       |       | FIXED |

## pole singularities

\*\*\*\*\*  
JP=0+ || eta:eta/1^S\_0[+] kaon:kaon/1^S\_0[+] pi:pi/1^S\_0[+]

sqrt(s)\_pole = ( 0.106 +/- 0.012267)  
+ (i/2)\*(-2.3145e-10 +/- 7.1373e-08) [ 0.04]

| eta:eta/1^S_0                | kaon:kaon/1^S_0              | pi:pi/1^S_0                  |
|------------------------------|------------------------------|------------------------------|
| k_re= -0.0000 +/- 0.0000     | k_re= -0.0000 +/- 0.0000     | k_re= -0.0000 +/- 0.0000     |
| k_im= 0.0891 +/- 0.0036      | k_im= 0.0812 +/- 0.0040      | k_im= 0.0443 +/- 0.0073      |
| corr= [-0.04]                | corr= [-0.04]                | corr= [-0.04]                |
| g = 0.0465 +/- 0.0211        | g = 0.1231 +/- 0.0301        | g = 0.1728 +/- 0.0157        |
| arg(g)/pi= 0.0000 +/- 0.0000 | arg(g)/pi= 1.0000 +/- 0.0000 | arg(g)/pi= 1.0000 +/- 0.0000 |
| g_re= 0.0465 +/- 0.0211      | g_re= -0.1231 +/- 0.0301     | g_re= -0.1728 +/- 0.0157     |
| g_im= 0.0000 +/- 0.0000      | g_im= 0.0000 +/- 0.0000      | g_im= 0.0000 +/- 0.0000      |
| corr= [-1.00]                | corr= [-0.67]                | corr= [ 0.15]                |

\*\*\*\*\*

\*\*\*\*\*  
JP=0+ || eta:eta/1^S\_0[+] kaon:kaon/1^S\_0[+] pi:pi/1^S\_0[-]



```

sqrt(s)_pole = (0.19693 +/- 0.0039361)
+ (i/2)*(-0.031033 +/- 0.0049634) [-0.00]

eta:eta/1^S_0 | kaon:kaon/1^S_0 | pi:pi/1^S_0 |
=====
k_re= -0.0198 +/- 0.0034 | k_re= -0.0298 +/- 0.0044 | k_re= 0.0706 +/- 0.0027 |
k_im= 0.0387 +/- 0.0041 | k_im= 0.0256 +/- 0.0038 | k_im= -0.0108 +/- 0.0017 |
corr= [ 0.39] | corr= [ 0.41] | corr= [ 0.07] |
=====
|g|= 0.1388 +/- 0.0227 | |g|= 0.1365 +/- 0.0175 | |g|= 0.1010 +/- 0.0098 |
arg(g)/pi= 0.0219 +/- 0.0322 | arg(g)/pi= -0.8478 +/- 0.0365 | arg(g)/pi= -0.4374 +/- 0.0380 |
=====
g_re= 0.1385 +/- 0.0220 | g_re= -0.1212 +/- 0.0151 | g_re= 0.0197 +/- 0.0129 |
g_im= 0.0095 +/- 0.0151 | g_im= -0.0628 +/- 0.0180 | g_im= -0.0991 +/- 0.0088 |
corr= [ 0.70] | corr= [ 0.26] | corr= [-0.38] |
=====

```

```

*****
JP=0+ || eta:eta/1^S_0[+] kaon:kaon/1^S_0[-] pi:pi/1^S_0[-]

```

```

sqrt(s)_pole = ( 0.1538 +/- 0.052922)
+ (i/2)*(-0.11675 +/- 0.074624) [ 0.93]

eta:eta/1^S_0 | kaon:kaon/1^S_0 | pi:pi/1^S_0 |
=====
k_re= -0.0279 +/- 0.0064 | k_re= 0.0308 +/- 0.0081 | k_re= 0.0490 +/- 0.0221 |
k_im= 0.0803 +/- 0.0305 | k_im= -0.0727 +/- 0.0326 | k_im= -0.0458 +/- 0.0328 |
corr= [ 0.45] | corr= [ 0.64] | corr= [ 0.92] |
=====
|g|= 0.3053 +/- 0.1624 | |g|= 0.0830 +/- 0.0353 | |g|= 0.1074 +/- 0.0104 |
arg(g)/pi= -0.0419 +/- 0.0571 | arg(g)/pi= 0.7574 +/- 0.1121 | arg(g)/pi= -0.4943 +/- 0.0175 |
=====
g_re= 0.3027 +/- 0.1543 | g_re= -0.0600 +/- 0.0104 | g_re= 0.0019 +/- 0.0057 |
g_im= -0.0401 +/- 0.0745 | g_im= 0.0573 +/- 0.0446 | g_im= -0.1074 +/- 0.0105 |
corr= [-0.96] | corr= [-0.52] | corr= [ 0.80] |
=====

```

```

*****
JP=0+ || eta:eta/1^S_0[-] kaon:kaon/1^S_0[+] pi:pi/1^S_0[+]

```

```

sqrt(s)_pole = (0.13074 +/- 0.014008)
+ (i/2)*(-1.6685e-11 +/- 4.8453e-09) [-0.06]

eta:eta/1^S_0 | kaon:kaon/1^S_0 | pi:pi/1^S_0 |
=====
k_re= 0.0000 +/- 0.0000 | k_re= -0.0000 +/- 0.0000 | k_re= -0.0000 +/- 0.0000 |
k_im= -0.0804 +/- 0.0057 | k_im= 0.0716 +/- 0.0064 | k_im= 0.0222 +/- 0.0206 |
corr= [ 0.06] | corr= [ 0.06] | corr= [ 0.06] |
=====
|g|= 0.0399 +/- 0.0126 | |g|= 0.0899 +/- 0.1060 | |g|= 0.1360 +/- 0.0872 |
arg(g)/pi= 0.0000 +/- 0.0000 | arg(g)/pi= 1.0000 +/- 0.0000 | arg(g)/pi= -0.0000 +/- 0.0000 |
=====
g_re= 0.0399 +/- 0.0126 | g_re= -0.0899 +/- 0.1060 | g_re= 0.1360 +/- 0.0872 |
g_im= 0.0000 +/- 0.0000 | g_im= 0.0000 +/- 0.0000 | g_im= -0.0000 +/- 0.0000 |
corr= [-1.00] | corr= [-0.84] | corr= [-0.72] |
=====

```

```

*****
JP=0+ || eta:eta/1^S_0[-] kaon:kaon/1^S_0[-] pi:pi/1^S_0[+]

```

```

sqrt(s)_pole = (0.12641 +/- 0.0068893)
+ (i/2)*(-4.4522e-14 +/- 1.1048e-11) [-0.02]

eta:eta/1^S_0 | kaon:kaon/1^S_0 | pi:pi/1^S_0 |
=====
k_re= 0.0000 +/- 0.0000 | k_re= 0.0000 +/- 0.0000 | k_re= -0.0000 +/- 0.0000 |
k_im= -0.0821 +/- 0.0026 | k_im= -0.0736 +/- 0.0030 | k_im= 0.0278 +/- 0.0078 |
corr= [ 0.02] | corr= [ 0.02] | corr= [ 0.02] |
=====
|g|= 0.0232 +/- 0.0081 | |g|= 0.0052 +/- 0.0054 | |g|= 0.1524 +/- 0.0293 |
arg(g)/pi= 0.0000 +/- 0.0000 | arg(g)/pi= 1.0000 +/- 0.0000 | arg(g)/pi= -0.0000 +/- 0.0000 |
=====
g_re= 0.0232 +/- 0.0081 | g_re= -0.0052 +/- 0.0054 | g_re= 0.1524 +/- 0.0293 |
g_im= 0.0000 +/- 0.0000 | g_im= 0.0000 +/- 0.0000 | g_im= -0.0000 +/- 0.0000 |
corr= [-1.00] | corr= [-0.97] | corr= [ 0.88] |
=====

```

# k\_poly\_clcccc

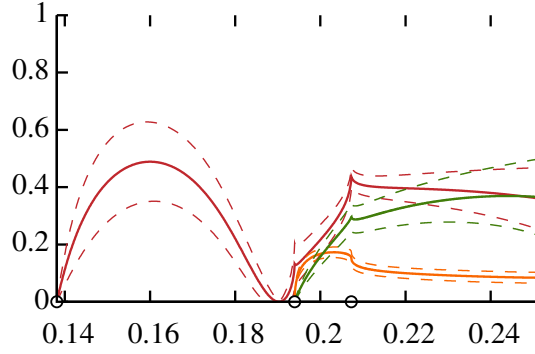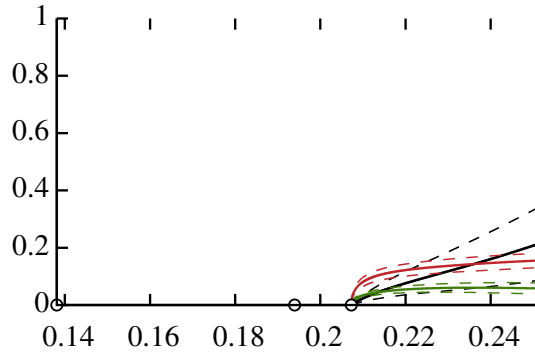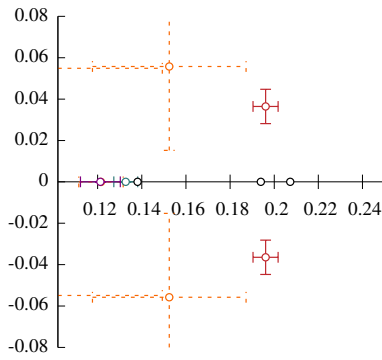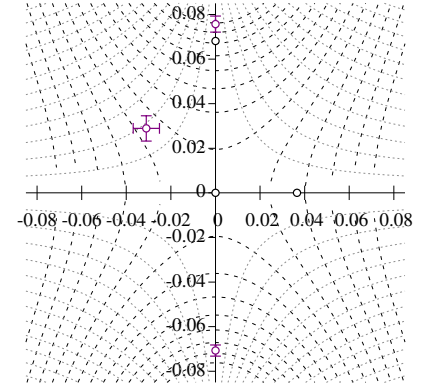

## parameter values

minimised with  $\text{chisq}/\text{nDoF} = 32.18 / (41 - 7) = 0.95$

|                                                                |                     |      |       |       |       |       |       |       |
|----------------------------------------------------------------|---------------------|------|-------|-------|-------|-------|-------|-------|
| JPO+ $_{\gamma\eta:\eta/1^1S_0 \eta:\eta/1^1S_0\text{order0}}$ | 5.1453 +/- 1.4979   | 1.00 | -0.75 | 0.85  | -0.11 | -0.26 | 0.05  | 0.50  |
| JPO+ $_{\gamma\eta:\eta/1^1S_0 K:K/1^1S_0\text{orde}}$         | -4.0879 +/- 0.65658 | 1.00 | -0.76 | -0.51 | 0.55  | 0.05  | -0.57 |       |
| JPO+ $_{\gamma\eta:\eta/1^1S_0 \pi:\pi/1^1S_0\text{order0}}$   | 5.4641 +/- 1.1152   |      | 1.00  | 0.02  | -0.55 | 0.08  | 0.86  |       |
| JPO+ $_{\gamma K:K/1^1S_0 K:K/1^1S_0\text{or}}$                | 1.8810 +/- 0.63104  |      |       | 1.00  | -0.49 | -0.18 | 0.19  |       |
| JPO+ $_{\gamma K:K/1^1S_0 \pi:\pi/1^1S_0\text{order0}}$        | -5.4512 +/- 0.76804 |      |       |       | 1.00  | -0.54 | -0.76 |       |
| JPO+ $_{\gamma K:K/1^1S_0 \pi:\pi/1^1S_0\text{order1}}$        | 0.95269 +/- 0.41937 |      |       |       |       | 1.00  | 0.14  |       |
| JPO+ $_{\gamma\pi:\pi/1^1S_0 \pi:\pi/1^1S_0\text{order0}}$     | 4.2048 +/- 1.0599   |      |       |       |       |       | 1.00  |       |
| JPO+ $_{\gamma\eta:\eta/1^1S_0 \eta:\eta/1^1S_0\text{order1}}$ | 0.0000 +/- 0        |      |       |       |       |       |       | FIXED |
| JPO+ $_{\gamma\eta:\eta/1^1S_0 K:K/1^1S_0\text{orde}}$         | 0.0000 +/- 0        |      |       |       |       |       |       | FIXED |
| JPO+ $_{\gamma\eta:\eta/1^1S_0 \pi:\pi/1^1S_0\text{order1}}$   | 0.0000 +/- 0        |      |       |       |       |       |       | FIXED |
| JPO+ $_{\gamma K:K/1^1S_0 K:K/1^1S_0\text{or}}$                | 0.0000 +/- 0        |      |       |       |       |       |       | FIXED |
| JPO+ $_{\gamma\pi:\pi/1^1S_0 \pi:\pi/1^1S_0\text{order1}}$     | 0.0000 +/- 0        |      |       |       |       |       |       | FIXED |

## pole singularities

\*\*\*\*\*  
JP=0+ ||  $\eta:\eta/1^1S_0[+]$   $K:K/1^1S_0[+]$   $\pi:\pi/1^1S_0[+]$

$\text{sqrt}(s)_{\text{pole}} = (0.12125 \pm 0.0090055)$   
+  $(i/2)*(+1.9269e-12 \pm 3.2905e-10)$  [-0.09]

| $\eta:\eta/1^1S_0$                      | $K:K/1^1S_0$                             | $\pi:\pi/1^1S_0$                         |
|-----------------------------------------|------------------------------------------|------------------------------------------|
| $k_{\text{re}} = 0.0000 \pm 0.0000$     | $k_{\text{re}} = 0.0000 \pm 0.0000$      | $k_{\text{re}} = 0.0000 \pm 0.0000$      |
| $k_{\text{im}} = 0.0841 \pm 0.0032$     | $k_{\text{im}} = 0.0757 \pm 0.0036$      | $k_{\text{im}} = 0.0331 \pm 0.0083$      |
| $\text{corr} = [0.09]$                  | $\text{corr} = [0.09]$                   | $\text{corr} = [0.09]$                   |
| $ g  = 0.0031 \pm 0.0117$               | $ g  = 0.1351 \pm 0.0243$                | $ g  = 0.1400 \pm 0.0175$                |
| $\text{arg}(g)/\pi = 0.0002 \pm 0.0015$ | $\text{arg}(g)/\pi = -0.0002 \pm 0.0022$ | $\text{arg}(g)/\pi = -0.0002 \pm 0.0022$ |
| $g_{\text{re}} = 0.0031 \pm 0.0117$     | $g_{\text{re}} = 0.1351 \pm 0.0243$      | $g_{\text{re}} = 0.1400 \pm 0.0175$      |
| $g_{\text{im}} = 0.0000 \pm 0.0000$     | $g_{\text{im}} = -0.0001 \pm 0.0009$     | $g_{\text{im}} = -0.0001 \pm 0.0010$     |
| $\text{corr} = [-0.93]$                 | $\text{corr} = [-0.28]$                  | $\text{corr} = [-0.41]$                  |

\*\*\*\*\*

\*\*\*\*\*  
JP=0+ ||  $\eta:\eta/1^1S_0[+]$   $K:K/1^1S_0[+]$   $\pi:\pi/1^1S_0[-]$

```

sqrt(s)_pole = (0.19609 +/- 0.005678)
+ (i/2)*(-0.036446 +/- 0.0083157) [ 0.05]

=====
eta:eta/1^S_0 | kaon:kaon/1^S_0 | pi:pi/1^S_0 |
=====
k_re= -0.0218 +/- 0.0048 | k_re= -0.0310 +/- 0.0059 | k_re= 0.0702 +/- 0.0039 |
k_im= 0.0410 +/- 0.0057 | k_im= 0.0289 +/- 0.0057 | k_im= -0.0127 +/- 0.0029 |
corr= [ 0.26] | corr= [ 0.31] | corr= [ 0.11] |
=====
|g|= 0.1427 +/- 0.0342 | |g|= 0.1705 +/- 0.0167 | |g|= 0.1165 +/- 0.0200 |
arg(g)/pi= -0.0442 +/- 0.0851 | arg(g)/pi= -0.8304 +/- 0.0506 | arg(g)/pi= -0.4611 +/- 0.0697 |
=====
g_re= 0.1414 +/- 0.0358 | g_re= -0.1468 +/- 0.0234 | g_re= 0.0142 +/- 0.0256 |
g_im= -0.0198 +/- 0.0367 | g_im= -0.0866 +/- 0.0216 | g_im= -0.1156 +/- 0.0199 |
corr= [ 0.31] | corr= [-0.56] | corr= [-0.01] |
=====
*****

*****
JP=0+ || eta:eta/1^S_0[+] kaon:kaon/1^S_0[-] pi:pi/1^S_0[-]

sqrt(s)_pole = (0.13274 +/- 0.0054305)
+ (i/2)*(+2.2831e-14 +/- 6.36e-12) [-0.08]

=====
eta:eta/1^S_0 | kaon:kaon/1^S_0 | pi:pi/1^S_0 |
=====
k_re= 0.0000 +/- 0.0000 | k_re= -0.0000 +/- 0.0000 | k_re= -0.0000 +/- 0.0000 |
k_im= 0.0796 +/- 0.0023 | k_im= -0.0707 +/- 0.0025 | k_im= -0.0191 +/- 0.0094 |
corr= [ 0.08] | corr= [ 0.08] | corr= [ 0.08] |
=====
|g|= 0.0882 +/- 0.0449 | |g|= 0.0274 +/- 0.0079 | |g|= 0.0799 +/- 0.0076 |
arg(g)/pi= 0.5000 +/- 0.0000 | arg(g)/pi= -0.5000 +/- 0.0000 | arg(g)/pi= 0.5000 +/- 0.0000 |
=====
g_re= 0.0000 +/- 0.0000 | g_re= 0.0000 +/- 0.0000 | g_re= -0.0000 +/- 0.0000 |
g_im= 0.0882 +/- 0.0449 | g_im= -0.0274 +/- 0.0079 | g_im= 0.0799 +/- 0.0076 |
corr= [-1.00] | corr= [ 0.94] | corr= [ 0.97] |
=====
*****

*****
JP=0+ || eta:eta/1^S_0[-] kaon:kaon/1^S_0[+] pi:pi/1^S_0[+]

sqrt(s)_pole = (0.12152 +/- 0.010072)
+ (i/2)*(-6.2128e-12 +/- 1.8383e-09) [-0.01]

=====
eta:eta/1^S_0 | kaon:kaon/1^S_0 | pi:pi/1^S_0 |
=====
k_re= 0.0000 +/- 0.0000 | k_re= -0.0000 +/- 0.0000 | k_re= -0.0000 +/- 0.0000 |
k_im= -0.0840 +/- 0.0036 | k_im= 0.0756 +/- 0.0040 | k_im= 0.0328 +/- 0.0093 |
corr= [ 0.01] | corr= [ 0.01] | corr= [ 0.01] |
=====
|g|= 0.0075 +/- 0.0339 | |g|= 0.1573 +/- 0.0980 | |g|= 0.1323 +/- 0.0437 |
arg(g)/pi= 0.0000 +/- 0.0003 | arg(g)/pi= 1.0000 +/- 0.0004 | arg(g)/pi= 1.0000 +/- 0.0005 |
=====
g_re= 0.0075 +/- 0.0339 | g_re= -0.1573 +/- 0.0980 | g_re= -0.1323 +/- 0.0437 |
g_im= 0.0000 +/- 0.0000 | g_im= 0.0000 +/- 0.0002 | g_im= 0.0000 +/- 0.0002 |
corr= [-0.91] | corr= [ 0.77] | corr= [-0.75] |
=====
*****

*****
JP=0+ || eta:eta/1^S_0[-] kaon:kaon/1^S_0[+] pi:pi/1^S_0[+]

sqrt(s)_pole = (0.15245 +/- 0.034788)
+ (i/2)*(-0.055773 +/- 0.040577) [-0.78]

=====
eta:eta/1^S_0 | kaon:kaon/1^S_0 | pi:pi/1^S_0 |
=====
k_re= 0.0146 +/- 0.0155 | k_re= -0.0167 +/- 0.0183 | k_re= -0.0396 +/- 0.0313 |
k_im= -0.0731 +/- 0.0140 | k_im= 0.0638 +/- 0.0149 | k_im= 0.0269 +/- 0.0094 |
corr= [ 0.84] | corr= [ 0.83] | corr= [-0.16] |
=====
|g|= 0.1067 +/- 0.0132 | |g|= 0.2427 +/- 0.1350 | |g|= 0.0991 +/- 0.0251 |
arg(g)/pi= 0.2625 +/- 0.0468 | arg(g)/pi= -0.7397 +/- 0.0481 | arg(g)/pi= 0.3953 +/- 0.1222 |
=====
g_re= 0.0724 +/- 0.0109 | g_re= -0.1659 +/- 0.0810 | g_re= 0.0320 +/- 0.0358 |
g_im= 0.0784 +/- 0.0174 | g_im= -0.1771 +/- 0.1140 | g_im= 0.0938 +/- 0.0283 |
corr= [-0.23] | corr= [ 0.89] | corr= [-0.35] |
=====
*****

*****
JP=0+ || eta:eta/1^S_0[-] kaon:kaon/1^S_0[+] pi:pi/1^S_0[-]

sqrt(s)_pole = (0.13374 +/- 0.032579)
+ (i/2)*(-0.084692 +/- 0.072575) [-0.69]

=====
eta:eta/1^S_0 | kaon:kaon/1^S_0 | pi:pi/1^S_0 |
=====
k_re= 0.0169 +/- 0.0181 | k_re= -0.0187 +/- 0.0200 | k_re= 0.0330 +/- 0.0284 |
k_im= -0.0837 +/- 0.0085 | k_im= 0.0757 +/- 0.0090 | k_im= -0.0429 +/- 0.0139 |
corr= [ 0.36] | corr= [ 0.30] | corr= [-0.42] |
=====
|g|= 0.0820 +/- 0.0263 | |g|= 0.3116 +/- 0.1698 | |g|= 0.0388 +/- 0.0233 |
arg(g)/pi= 0.1434 +/- 0.0606 | arg(g)/pi= -0.7966 +/- 0.0303 | arg(g)/pi= -0.6379 +/- 0.1328 |
=====
g_re= 0.0738 +/- 0.0225 | g_re= -0.2502 +/- 0.1202 | g_re= -0.0163 +/- 0.0236 |
g_im= 0.0357 +/- 0.0208 | g_im= -0.1858 +/- 0.1235 | g_im= -0.0352 +/- 0.0158 |
corr= [ 0.55] | corr= [ 0.99] | corr= [ 0.84] |
=====
*****

```

```

*****
JP=0+ || eta:eta/1^S_0[-] kaon:kaon/1^S_0[-] pi:pi/1^S_0[+]

sqrt(s)_pole = (0.10145 +/- 0.047838)
               + (i/2)*(-0.054898 +/- 0.12329) [-0.94]

=====
eta:eta/1^S_0 | kaon:kaon/1^S_0 | pi:pi/1^S_0 |
=====
k_re= 0.0076 +/- 0.0207 | k_re= 0.0083 +/- 0.0226 | k_re= -0.0138 +/- 0.0378 |
k_im= -0.0917 +/- 0.0077 | k_im= -0.0842 +/- 0.0080 | k_im= 0.0508 +/- 0.0082 |
corr= [ 0.88] | corr= [ 0.87] | corr= [ 0.69] |
=====
|g|= 0.0608 +/- 0.0418 | |g|= 0.0163 +/- 0.0080 | |g|= 0.2449 +/- 0.3483 |
arg(g)/pi= 0.1905 +/- 0.0851 | arg(g)/pi= 0.3344 +/- 0.2369 | arg(g)/pi= 0.2327 +/- 0.0310 |
=====
g_re= 0.0502 +/- 0.0267 | g_re= 0.0081 +/- 0.0088 | g_re= 0.1823 +/- 0.2441 |
g_im= 0.0342 +/- 0.0360 | g_im= 0.0142 +/- 0.0115 | g_im= 0.1636 +/- 0.2497 |
corr= [ 0.95] | corr= [-0.64] | corr= [ 1.00] |
=====
*****

```

# k\_poly\_clcccc\_noCM

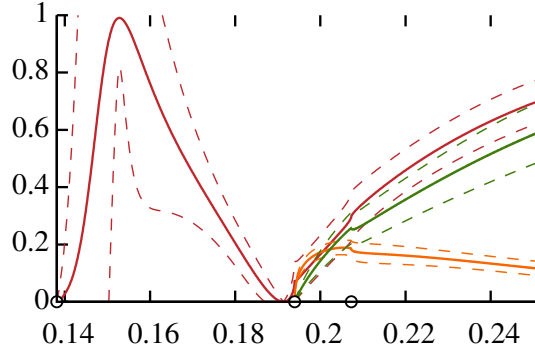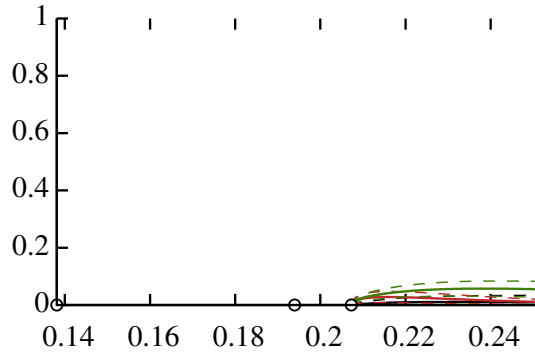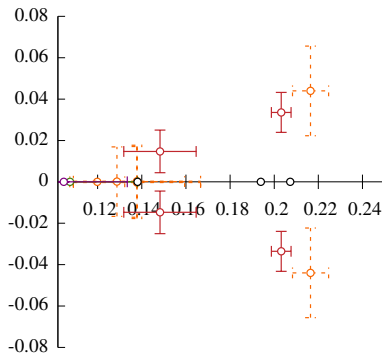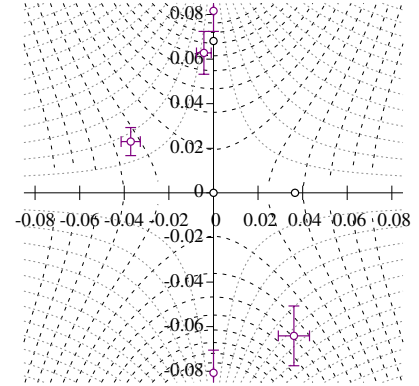

## parameter values

minimised with  $\text{chisq}/\text{nDoF} = 23.70 / (41 - 7) = 0.70$

|                                                        |                      |      |       |       |       |       |       |       |
|--------------------------------------------------------|----------------------|------|-------|-------|-------|-------|-------|-------|
| JPO+_ $\gamma$ _eta:eta/1^S_0 eta:eta/1^S_0_order0     | -0.22222 +/- 0.34062 | 1.00 | -0.28 | -0.14 | -0.33 | -0.19 | 0.07  | -0.18 |
| JPO+_ $\gamma$ _eta:eta/1^S_0 kaon:kaon/1^S_0_order0   | 0.35639 +/- 0.23357  | 1.00 | -0.50 | -0.11 | 0.58  | -0.56 | -0.24 |       |
| JPO+_ $\gamma$ _eta:eta/1^S_0 pi:pi/1^S_0_order0       | 0.89799 +/- 0.31692  |      | 1.00  | 0.05  | 0.05  | 0.03  | 0.73  |       |
| JPO+_ $\gamma$ _kaon:kaon/1^S_0 kaon:kaon/1^S_0_order0 | -1.1288 +/- 0.28418  |      |       | 1.00  | -0.50 | 0.54  | -0.08 |       |
| JPO+_ $\gamma$ _kaon:kaon/1^S_0 pi:pi/1^S_0_order0     | 1.0208 +/- 0.94904   |      |       |       | 1.00  | -0.98 | 0.01  |       |
| JPO+_ $\gamma$ _kaon:kaon/1^S_0 pi:pi/1^S_0_order1     | -2.2552 +/- 0.87078  |      |       |       |       | 1.00  | 0.04  |       |
| JPO+_ $\gamma$ _pi:pi/1^S_0 pi:pi/1^S_0_order0         | 0.73536 +/- 0.30854  |      |       |       |       |       | 1.00  |       |
| JPO+_ $\gamma$ _eta:eta/1^S_0 eta:eta/1^S_0_order1     | 0.0000 +/- 0         |      |       |       |       |       |       | FIXED |
| JPO+_ $\gamma$ _eta:eta/1^S_0 kaon:kaon/1^S_0_order1   | 0.0000 +/- 0         |      |       |       |       |       |       | FIXED |
| JPO+_ $\gamma$ _eta:eta/1^S_0 pi:pi/1^S_0_order1       | 0.0000 +/- 0         |      |       |       |       |       |       | FIXED |
| JPO+_ $\gamma$ _kaon:kaon/1^S_0 kaon:kaon/1^S_0_order1 | 0.0000 +/- 0         |      |       |       |       |       |       | FIXED |
| JPO+_ $\gamma$ _kaon:kaon/1^S_0 pi:pi/1^S_0_order1     | 0.0000 +/- 0         |      |       |       |       |       |       | FIXED |

## pole singularities

\*\*\*\*\*  
JP=0+ || eta:eta/1^S\_0[+] kaon:kaon/1^S\_0[+] pi:pi/1^S\_0[+]

$\sqrt{s}_{\text{pole}} = (0.10469 \pm 0.028727) + (i/2) * (+6.2779e-14 \pm 1.8689e-11) [0.04]$

| eta:eta/1^S_0                | kaon:kaon/1^S_0               | pi:pi/1^S_0                  |
|------------------------------|-------------------------------|------------------------------|
| k_re= 0.0000 +/- 0.0000      | k_re= 0.0000 +/- 0.0000       | k_re= 0.0000 +/- 0.0000      |
| k_im= 0.0894 +/- 0.0084      | k_im= 0.0816 +/- 0.0092       | k_im= 0.0450 +/- 0.0167      |
| corr= [-0.04]                | corr= [-0.04]                 | corr= [-0.04]                |
| g = 0.0592 +/- 0.0205        | g = 0.0215 +/- 0.0349         | g = 0.0631 +/- 0.0244        |
| arg(g)/pi= 0.0000 +/- 0.0000 | arg(g)/pi= -0.0000 +/- 0.0000 | arg(g)/pi= 1.0000 +/- 0.0000 |
| g_re= 0.0592 +/- 0.0205      | g_re= 0.0215 +/- 0.0349       | g_re= -0.0631 +/- 0.0244     |
| g_im= 0.0000 +/- 0.0000      | g_im= -0.0000 +/- 0.0000      | g_im= 0.0000 +/- 0.0000      |
| corr= [-1.00]                | corr= [-0.95]                 | corr= [0.55]                 |

\*\*\*\*\*

\*\*\*\*\*  
JP=0+ || eta:eta/1^S\_0[+] kaon:kaon/1^S\_0[+] pi:pi/1^S\_0[-]

```

sqrt(s)_pole = (0.14824 +/- 0.016378)
               + (i/2)*(-0.014719 +/- 0.0103) [-0.09]

=====
eta:eta/1^S_0 | kaon:kaon/1^S_0 | pi:pi/1^S_0 |
=====
k_re= -0.0038 +/- 0.0028 | k_re= -0.0043 +/- 0.0033 | k_re= 0.0283 +/- 0.0198 |
k_im= 0.0726 +/- 0.0083 | k_im= 0.0628 +/- 0.0096 | k_im= -0.0096 +/- 0.0079 |
corr= [ 0.36] | corr= [ 0.39] | corr= [ 0.57] |
=====
|g|= 0.0436 +/- 0.0332 | |g|= 0.1253 +/- 0.0166 | |g|= 0.0749 +/- 0.0304 |
arg(g)/pi= -0.3025 +/- 0.1642 | arg(g)/pi= 0.8944 +/- 0.0650 | arg(g)/pi= 0.8579 +/- 0.0595 |
=====
g_re= 0.0253 +/- 0.0338 | g_re= -0.1185 +/- 0.0200 | g_re= -0.0676 +/- 0.0268 |
g_im= -0.0354 +/- 0.0216 | g_im= 0.0408 +/- 0.0231 | g_im= 0.0324 +/- 0.0201 |
corr= [-0.59] | corr= [ 0.48] | corr= [-0.63] |
=====
*****

*****
JP=0+ || eta:eta/1^S_0[+] kaon:kaon/1^S_0[+] pi:pi/1^S_0[-]

sqrt(s)_pole = (0.20318 +/- 0.004441)
               + (i/2)*(-0.033569 +/- 0.0096485) [ 0.38]

=====
eta:eta/1^S_0 | kaon:kaon/1^S_0 | pi:pi/1^S_0 |
=====
k_re= -0.0253 +/- 0.0045 | k_re= -0.0371 +/- 0.0043 | k_re= 0.0749 +/- 0.0029 |
k_im= 0.0337 +/- 0.0066 | k_im= 0.0230 +/- 0.0063 | k_im= -0.0114 +/- 0.0033 |
corr= [-0.14] | corr= [ 0.17] | corr= [ 0.37] |
=====
|g|= 0.0877 +/- 0.0318 | |g|= 0.1452 +/- 0.0193 | |g|= 0.1133 +/- 0.0159 |
arg(g)/pi= 0.2312 +/- 0.1004 | arg(g)/pi= -0.7727 +/- 0.0381 | arg(g)/pi= -0.3541 +/- 0.0295 |
=====
g_re= 0.0656 +/- 0.0331 | g_re= -0.1097 +/- 0.0197 | g_re= 0.0501 +/- 0.0087 |
g_im= 0.0582 +/- 0.0261 | g_im= -0.0951 +/- 0.0169 | g_im= -0.1016 +/- 0.0169 |
corr= [ 0.11] | corr= [ 0.08] | corr= [-0.06] |
=====
*****

*****
JP=0+ || eta:eta/1^S_0[+] kaon:kaon/1^S_0[-] pi:pi/1^S_0[+]

sqrt(s)_pole = (0.10751 +/- 0.030509)
               + (i/2)*(+5.5487e-15 +/- 1.6543e-12) [ 0.02]

=====
eta:eta/1^S_0 | kaon:kaon/1^S_0 | pi:pi/1^S_0 |
=====
k_re= 0.0000 +/- 0.0000 | k_re= -0.0000 +/- 0.0000 | k_re= 0.0000 +/- 0.0000 |
k_im= 0.0886 +/- 0.0093 | k_im= -0.0807 +/- 0.0102 | k_im= 0.0433 +/- 0.0189 |
corr= [-0.02] | corr= [-0.02] | corr= [-0.02] |
=====
|g|= 0.0714 +/- 0.0209 | |g|= 0.0088 +/- 0.0131 | |g|= 0.0690 +/- 0.0239 |
arg(g)/pi= 0.0000 +/- 0.0000 | arg(g)/pi= 1.0000 +/- 0.0000 | arg(g)/pi= 1.0000 +/- 0.0000 |
=====
g_re= 0.0714 +/- 0.0209 | g_re= -0.0088 +/- 0.0131 | g_re= -0.0690 +/- 0.0239 |
g_im= 0.0000 +/- 0.0000 | g_im= 0.0000 +/- 0.0000 | g_im= 0.0000 +/- 0.0000 |
corr= [-1.00] | corr= [-0.92] | corr= [ 0.49] |
=====
*****

*****
JP=0+ || eta:eta/1^S_0[+] kaon:kaon/1^S_0[-] pi:pi/1^S_0[-]

sqrt(s)_pole = (0.17121 +/- 0.016245)
               + (i/2)*(-0.10827 +/- 0.037395) [ 0.56]

=====
eta:eta/1^S_0 | kaon:kaon/1^S_0 | pi:pi/1^S_0 |
=====
k_re= -0.0322 +/- 0.0068 | k_re= 0.0361 +/- 0.0070 | k_re= 0.0583 +/- 0.0085 |
k_im= 0.0720 +/- 0.0123 | k_im= -0.0641 +/- 0.0134 | k_im= -0.0397 +/- 0.0133 |
corr= [-0.24] | corr= [-0.13] | corr= [ 0.43] |
=====
|g|= 0.0916 +/- 0.0517 | |g|= 0.0690 +/- 0.0180 | |g|= 0.1367 +/- 0.0234 |
arg(g)/pi= 0.0795 +/- 0.1457 | arg(g)/pi= 0.5835 +/- 0.0624 | arg(g)/pi= -0.4127 +/- 0.0757 |
=====
g_re= 0.0887 +/- 0.0568 | g_re= -0.0179 +/- 0.0127 | g_re= 0.0370 +/- 0.0297 |
g_im= 0.0226 +/- 0.0347 | g_im= 0.0667 +/- 0.0186 | g_im= -0.1316 +/- 0.0269 |
corr= [-0.45] | corr= [ 0.08] | corr= [ 0.45] |
=====
*****

*****
JP=0+ || eta:eta/1^S_0[-] kaon:kaon/1^S_0[+] pi:pi/1^S_0[+]

sqrt(s)_pole = (0.17738 +/- 0.02205)
               + (i/2)*(-0.098419 +/- 0.042092) [ 0.57]

=====
eta:eta/1^S_0 | kaon:kaon/1^S_0 | pi:pi/1^S_0 |
=====
k_re= 0.0324 +/- 0.0087 | k_re= -0.0369 +/- 0.0094 | k_re= -0.0613 +/- 0.0122 |
k_im= -0.0673 +/- 0.0166 | k_im= 0.0592 +/- 0.0178 | k_im= 0.0356 +/- 0.0156 |
corr= [-0.03] | corr= [ 0.11] | corr= [ 0.54] |
=====
|g|= 0.0895 +/- 0.0166 | |g|= 0.1399 +/- 0.0094 | |g|= 0.0994 +/- 0.0145 |
arg(g)/pi= 0.3955 +/- 0.0497 | arg(g)/pi= -0.7105 +/- 0.0739 | arg(g)/pi= 0.9430 +/- 0.0341 |
=====
g_re= 0.0289 +/- 0.0138 | g_re= -0.0859 +/- 0.0241 | g_re= -0.0979 +/- 0.0153 |
g_im= 0.0847 +/- 0.0167 | g_im= -0.1104 +/- 0.0237 | g_im= 0.0177 +/- 0.0094 |
corr= [ 0.04] | corr= [-0.87] | corr= [ 0.41] |
=====
*****

```

```

*****
JP=0+  ||  eta:eta/1^S_0[-] kaon:kaon/1^S_0[+] pi:pi/1^S_0[-]

sqrt(s)_pole = (0.21647 +/- 0.0081734)
               + (i/2)*(-0.04397 +/- 0.021666) [-0.45]

=====
eta:eta/1^S_0 | kaon:kaon/1^S_0 | pi:pi/1^S_0 |
=====
k_re= 0.0411 +/- 0.0115 | k_re= -0.0521 +/- 0.0093 | k_re= 0.0838 +/- 0.0054 |
k_im= -0.0289 +/- 0.0091 | k_im= 0.0228 +/- 0.0090 | k_im= -0.0142 +/- 0.0068 |
corr= [-0.47] | corr= [-0.51] | corr= [-0.48] |
=====
|g|= 0.0776 +/- 0.0231 | |g|= 0.1541 +/- 0.0245 | |g|= 0.1048 +/- 0.0189 |
arg(g)/pi= 0.3093 +/- 0.0810 | arg(g)/pi= -0.7120 +/- 0.0184 | arg(g)/pi= -0.2558 +/- 0.0276 |
=====
g_re= 0.0437 +/- 0.0265 | g_re= -0.0952 +/- 0.0183 | g_re= 0.0728 +/- 0.0115 |
g_im= 0.0641 +/- 0.0148 | g_im= -0.1212 +/- 0.0186 | g_im= -0.0755 +/- 0.0175 |
corr= [ 0.44] | corr= [ 0.79] | corr= [-0.66] |
=====

```

```

*****
JP=0+  ||  eta:eta/1^S_0[-] kaon:kaon/1^S_0[+] pi:pi/1^S_0[-]

sqrt(s)_pole = (0.13782 +/- 0.028824)
               + (i/2)*(-0.00034183 +/- 0.017401) [ 0.29]

=====
eta:eta/1^S_0 | kaon:kaon/1^S_0 | pi:pi/1^S_0 |
=====
k_re= 0.0001 +/- 0.0037 | k_re= -0.0001 +/- 0.0041 | k_re= 0.0040 +/- 0.0785 |
k_im= -0.0774 +/- 0.0128 | k_im= 0.0682 +/- 0.0145 | k_im= -0.0054 +/- 0.0915 |
corr= [-0.27] | corr= [-0.27] | corr= [ 0.66] |
=====
|g|= 0.0497 +/- 0.2531 | |g|= 0.1663 +/- 0.5641 | |g|= 0.0342 +/- 0.3945 |
arg(g)/pi= 0.0129 +/- 1.2138 | arg(g)/pi= -0.9974 +/- 0.8351 | arg(g)/pi= 0.0411 +/- 2.5557 |
=====
g_re= 0.0496 +/- 0.2526 | g_re= -0.1663 +/- 0.5639 | g_re= 0.0340 +/- 0.3905 |
g_im= 0.0020 +/- 0.1901 | g_im= -0.0013 +/- 0.4367 | g_im= 0.0044 +/- 0.2806 |
corr= [ 0.08] | corr= [ 0.07] | corr= [ 0.16] |
=====

```

```

*****
JP=0+  ||  eta:eta/1^S_0[-] kaon:kaon/1^S_0[-] pi:pi/1^S_0[-]

sqrt(s)_pole = (0.11983 +/- 0.012464)
               + (i/2)*(+2.4122e-13 +/- 7.2004e-11) [ 0.03]

=====
eta:eta/1^S_0 | kaon:kaon/1^S_0 | pi:pi/1^S_0 |
=====
k_re= -0.0000 +/- 0.0000 | k_re= -0.0000 +/- 0.0000 | k_re= -0.0000 +/- 0.0000 |
k_im= -0.0846 +/- 0.0044 | k_im= -0.0763 +/- 0.0049 | k_im= -0.0343 +/- 0.0109 |
corr= [-0.03] | corr= [-0.03] | corr= [-0.03] |
=====
|g|= 0.0421 +/- 0.0105 | |g|= 0.0123 +/- 0.0158 | |g|= 0.0966 +/- 0.0116 |
arg(g)/pi= 0.5000 +/- 0.0000 | arg(g)/pi= 0.5000 +/- 0.0000 | arg(g)/pi= 0.5000 +/- 0.0000 |
=====
g_re= 0.0000 +/- 0.0000 | g_re= -0.0000 +/- 0.0000 | g_re= -0.0000 +/- 0.0000 |
g_im= 0.0421 +/- 0.0105 | g_im= 0.0123 +/- 0.0158 | g_im= 0.0966 +/- 0.0116 |
corr= [-1.00] | corr= [-0.96] | corr= [-0.17] |
=====

```

## $J^P = 2^+$ Amplitudes

### K with two poles plus a polynomial

All amplitudes are of the form

$$\begin{aligned} \mathbf{K}(s) = & \frac{1}{m_0^2 - s} \begin{pmatrix} (g_{\pi\pi}^{(0)})^2 & g_{\pi\pi}^{(0)} g_{K\bar{K}}^{(0)} & g_{\pi\pi}^{(0)} g_{\eta\eta}^{(0)} \\ g_{\pi\pi}^{(0)} g_{K\bar{K}}^{(0)} & (g_{K\bar{K}}^{(0)})^2 & g_{K\bar{K}}^{(0)} g_{\eta\eta}^{(0)} \\ g_{\pi\pi}^{(0)} g_{\eta\eta}^{(0)} & g_{K\bar{K}}^{(0)} g_{\eta\eta}^{(0)} & (g_{\eta\eta}^{(0)})^2 \end{pmatrix} \\ & + \frac{1}{m_1^2 - s} \begin{pmatrix} (g_{\pi\pi}^{(1)})^2 & g_{\pi\pi}^{(1)} g_{K\bar{K}}^{(1)} & g_{\pi\pi}^{(1)} g_{\eta\eta}^{(1)} \\ g_{\pi\pi}^{(1)} g_{K\bar{K}}^{(1)} & (g_{K\bar{K}}^{(1)})^2 & g_{K\bar{K}}^{(1)} g_{\eta\eta}^{(1)} \\ g_{\pi\pi}^{(1)} g_{\eta\eta}^{(1)} & g_{K\bar{K}}^{(1)} g_{\eta\eta}^{(1)} & (g_{\eta\eta}^{(1)})^2 \end{pmatrix} \\ & + \begin{pmatrix} A(s) & B(s) & C(s) \\ B(s) & D(s) & E(s) \\ C(s) & E(s) & F(s) \end{pmatrix} \end{aligned}$$

with row/column ordering  $\pi\pi, K\bar{K}, \eta\eta$ . The fit name will be something like `k_2poles_ABCDEF`, and the encoding of  $A \dots F$  indicates the order of the polynomial used in the relevant element, e.g.

$$\begin{aligned} \text{A=x} & \implies A(s) = 0 \\ \text{A=c} & \implies A(s) = \text{const} \\ \text{A=l} & \implies A(s) = a + b s \\ \text{A=q} & \implies A(s) = a + b s + c s^2 \\ \text{A=s} & \implies A(s) = b s \end{aligned}$$

If the amplitude name features `_noCM`, the naive phase-space is used,  $I_{ij}(s) = -\rho_i(s)\delta_{ij}$ , otherwise the Chew-Mandelstam phase-space subtracted **at the position of the lower mass pole**,  $s = m_0^2$ .

If the amplitude name features `_free_geta`, the parameters  $g_{\eta\eta}^{(0,1)}$  are allowed to float freely in the fit, otherwise they are fixed to have value zero.

The parameter names should be self-explanatory. See the  $J^P = 0^+$  amplitudes file for more description.



# k\_2poles\_free\_geta\_XXXXXXC\_noCM

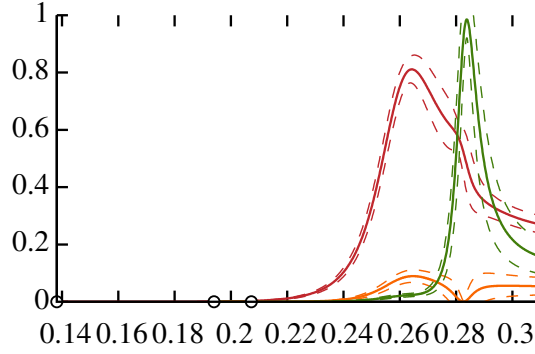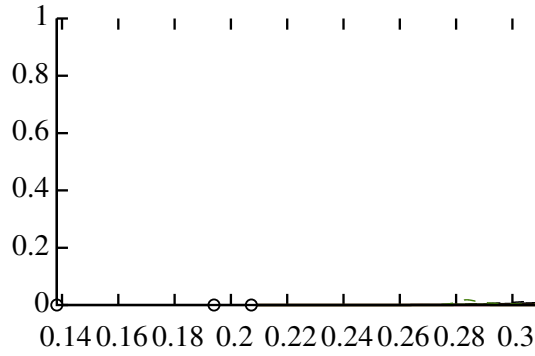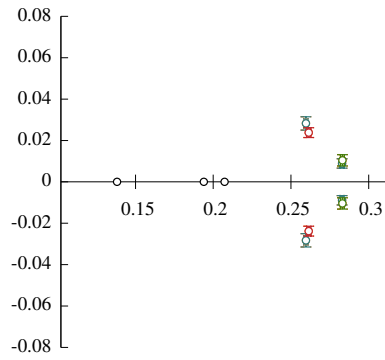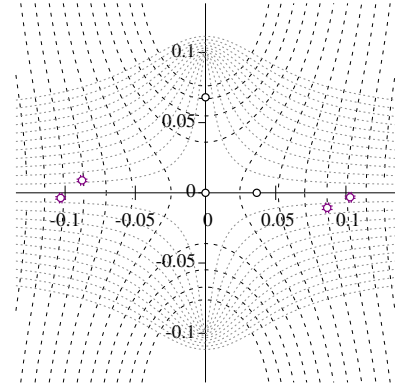

## parameter values

minimised with  $\chi^2/\text{ndof} = 28.87 / (34 - 9) = 1.15$

|                                               |                         |      |       |       |       |       |       |       |       |       |
|-----------------------------------------------|-------------------------|------|-------|-------|-------|-------|-------|-------|-------|-------|
| JP2+_g_eta:eta/1^D_2_pole0                    | -0.00019792 +/- 0.40532 | 1.00 | -0.87 | -0.01 | 0.00  | 0.00  | -0.00 | -0.02 | 0.00  | -0.01 |
| JP2+_g_eta:eta/1^D_2_pole1                    | 0.00027393 +/- 0.69654  | 1.00 | 0.01  | -0.00 | -0.00 | 0.00  | 0.00  | 0.03  | -0.00 | 0.01  |
| JP2+_g_kaon:kaon/1^D_2_pole0                  | -1.0955 +/- 0.16061     | 1.00 | 0.10  | -0.25 | 0.02  | 0.02  | 0.08  | 0.34  |       |       |
| JP2+_g_kaon:kaon/1^D_2_pole1                  | 1.4953 +/- 0.24989      | 1.00 | 0.56  | -0.83 | 0.15  | 0.48  | 0.54  |       |       |       |
| JP2+_g_pi:pi/1^D_2_pole0                      | 1.8530 +/- 0.087712     |      |       |       | 1.00  | -0.66 | 0.09  | 0.48  | 0.06  |       |
| JP2+_g_pi:pi/1^D_2_pole1                      | -0.11397 +/- 0.28848    |      |       |       | 1.00  | -0.18 | -0.57 | -0.21 |       |       |
| JP2+_gamma_eta:eta/1^D_2 eta:eta/1^D_2_order0 | 40.539 +/- 24.384       |      |       |       |       | 1.00  | -0.11 | -0.07 |       |       |
| JP2+_m_pole0                                  | 0.26416 +/- 0.0016974   |      |       |       |       |       | 1.00  | 0.35  |       |       |
| JP2+_m_pole1                                  | 0.28405 +/- 0.0014766   |      |       |       |       |       |       | 1.00  |       |       |
| JP2+_gamma_eta:eta/1^D_2 kaon:kaon/1^D_2_orde | 0.0000 +/- 0            |      |       |       |       |       |       |       | FIXED |       |
| JP2+_gamma_eta:eta/1^D_2 pi:pi/1^D_2_order0   | 0.0000 +/- 0            |      |       |       |       |       |       |       | FIXED |       |
| JP2+_gamma_kaon:kaon/1^D_2 kaon:kaon/1^D_2_or | 0.0000 +/- 0            |      |       |       |       |       |       |       | FIXED |       |
| JP2+_gamma_kaon:kaon/1^D_2 pi:pi/1^D_2_order0 | 0.0000 +/- 0            |      |       |       |       |       |       |       | FIXED |       |
| JP2+_gamma_pi:pi/1^D_2 pi:pi/1^D_2_order0     | 0.0000 +/- 0            |      |       |       |       |       |       |       | FIXED |       |

## pole singularities

\*\*\*\*\*

\*\*\*\*\*

JP=2+ || eta:eta/1^D\_2[+] kaon:kaon/1^D\_2[+] pi:pi/1^D\_2[-]

sqrt(s)\_pole = (0.26146 +/- 0.001358)  
+ (i/2)\*(-0.023807 +/- 0.0023733) [-0.36]

| eta:eta/1^D_2                 | kaon:kaon/1^D_2               | pi:pi/1^D_2                   |
|-------------------------------|-------------------------------|-------------------------------|
| k_re= -0.0801 +/- 0.0011      | k_re= -0.0879 +/- 0.0010      | k_re= 0.1111 +/- 0.0008       |
| k_im= 0.0097 +/- 0.0009       | k_im= 0.0089 +/- 0.0009       | k_im= -0.0070 +/- 0.0007      |
| corr= [-0.34]                 | corr= [-0.34]                 | corr= [-0.35]                 |
| g = 0.0005 +/- 0.0062         | g = 0.0315 +/- 0.0050         | g = 0.0889 +/- 0.0041         |
| arg(g)/pi= -0.1300 +/- 0.1243 | arg(g)/pi= -0.1117 +/- 0.0186 | arg(g)/pi= -0.0794 +/- 0.0067 |
| g_re= 0.0004 +/- 0.0057       | g_re= 0.0296 +/- 0.0049       | g_re= 0.0862 +/- 0.0036       |
| g_im= -0.0002 +/- 0.0025      | g_im= -0.0108 +/- 0.0020      | g_im= -0.0220 +/- 0.0027      |
| corr= [-1.00]                 | corr= [-0.46]                 | corr= [-0.91]                 |

\*\*\*\*\*

```

*****
JP=2+ || eta:eta/1^D_2[+] kaon:kaon/1^D_2[-] pi:pi/1^D_2[+]

sqrt(s)_pole = (0.28309 +/- 0.0012704)
               + (i/2)*(-0.010429 +/- 0.0027248) [-0.63]

=====
eta:eta/1^D_2 | kaon:kaon/1^D_2 | pi:pi/1^D_2 |
=====
k_re= -0.0964 +/- 0.0009 | k_re= 0.1031 +/- 0.0009 | k_re= -0.1236 +/- 0.0007 |
k_im= 0.0038 +/- 0.0010 | k_im= -0.0036 +/- 0.0009 | k_im= 0.0030 +/- 0.0008 |
corr= [-0.63] | corr= [-0.63] | corr= [-0.63] |
=====
|g|= 0.0012 +/- 0.0164 | |g|= 0.0656 +/- 0.0089 | |g|= 0.0160 +/- 0.0059 |
arg(g)/pi= -0.0722 +/- 0.1219 | arg(g)/pi= -0.0614 +/- 0.0115 | arg(g)/pi= -0.1999 +/- 0.2122 |
=====
g_re= 0.0012 +/- 0.0160 | g_re= 0.0644 +/- 0.0087 | g_re= 0.0129 +/- 0.0107 |
g_im= -0.0003 +/- 0.0037 | g_im= -0.0126 +/- 0.0031 | g_im= -0.0094 +/- 0.0058 |
corr= [-0.99] | corr= [-0.61] | corr= [ 0.87] |
=====
*****

*****
JP=2+ || eta:eta/1^D_2[+] kaon:kaon/1^D_2[-] pi:pi/1^D_2[-]

sqrt(s)_pole = (0.25964 +/- 0.0013419)
               + (i/2)*(-0.028243 +/- 0.0031933) [-0.21]

=====
eta:eta/1^D_2 | kaon:kaon/1^D_2 | pi:pi/1^D_2 |
=====
k_re= -0.0787 +/- 0.0011 | k_re= 0.0867 +/- 0.0010 | k_re= 0.1100 +/- 0.0008 |
k_im= 0.0116 +/- 0.0013 | k_im= -0.0106 +/- 0.0012 | k_im= -0.0083 +/- 0.0009 |
corr= [-0.24] | corr= [-0.23] | corr= [-0.22] |
=====
|g|= 0.0005 +/- 0.0070 | |g|= 0.0351 +/- 0.0058 | |g|= 0.0854 +/- 0.0045 |
arg(g)/pi= -0.1256 +/- 0.2593 | arg(g)/pi= -0.1086 +/- 0.0148 | arg(g)/pi= -0.1019 +/- 0.0113 |
=====
g_re= 0.0005 +/- 0.0064 | g_re= 0.0330 +/- 0.0054 | g_re= 0.0810 +/- 0.0034 |
g_im= -0.0002 +/- 0.0027 | g_im= -0.0117 +/- 0.0026 | g_im= -0.0269 +/- 0.0042 |
corr= [-0.99] | corr= [-0.75] | corr= [-0.91] |
=====
*****

*****
JP=2+ || eta:eta/1^D_2[+] kaon:kaon/1^D_2[-] pi:pi/1^D_2[-]

sqrt(s)_pole = (0.28287 +/- 0.0012644)
               + (i/2)*(-0.0088895 +/- 0.0022755) [-0.14]

=====
eta:eta/1^D_2 | kaon:kaon/1^D_2 | pi:pi/1^D_2 |
=====
k_re= -0.0963 +/- 0.0009 | k_re= 0.1030 +/- 0.0009 | k_re= 0.1234 +/- 0.0007 |
k_im= 0.0033 +/- 0.0008 | k_im= -0.0031 +/- 0.0008 | k_im= -0.0025 +/- 0.0007 |
corr= [-0.14] | corr= [-0.14] | corr= [-0.14] |
=====
|g|= 0.0011 +/- 0.0146 | |g|= 0.0561 +/- 0.0068 | |g|= 0.0161 +/- 0.0057 |
arg(g)/pi= -0.0778 +/- 0.2669 | arg(g)/pi= -0.0740 +/- 0.0312 | arg(g)/pi= 0.2833 +/- 0.1797 |
=====
g_re= 0.0011 +/- 0.0142 | g_re= 0.0546 +/- 0.0060 | g_re= 0.0101 +/- 0.0043 |
g_im= -0.0003 +/- 0.0037 | g_im= -0.0129 +/- 0.0064 | g_im= 0.0125 +/- 0.0098 |
corr= [-0.97] | corr= [-0.62] | corr= [-0.79] |
=====
*****

*****
JP=2+ || eta:eta/1^D_2[-] kaon:kaon/1^D_2[+] pi:pi/1^D_2[-]

sqrt(s)_pole = (0.26146 +/- 0.0013582)
               + (i/2)*(-0.023808 +/- 0.0023732) [-0.36]

=====
eta:eta/1^D_2 | kaon:kaon/1^D_2 | pi:pi/1^D_2 |
=====
k_re= 0.0801 +/- 0.0011 | k_re= -0.0879 +/- 0.0010 | k_re= 0.1111 +/- 0.0008 |
k_im= -0.0097 +/- 0.0009 | k_im= 0.0089 +/- 0.0009 | k_im= -0.0070 +/- 0.0007 |
corr= [-0.34] | corr= [-0.34] | corr= [-0.35] |
=====
|g|= 0.0005 +/- 0.0063 | |g|= 0.0315 +/- 0.0050 | |g|= 0.0889 +/- 0.0041 |
arg(g)/pi= -0.1209 +/- 0.1244 | arg(g)/pi= -0.1117 +/- 0.0186 | arg(g)/pi= -0.0794 +/- 0.0067 |
=====
g_re= 0.0004 +/- 0.0058 | g_re= 0.0296 +/- 0.0049 | g_re= 0.0862 +/- 0.0036 |
g_im= -0.0002 +/- 0.0023 | g_im= -0.0108 +/- 0.0020 | g_im= -0.0220 +/- 0.0027 |
corr= [-1.00] | corr= [-0.46] | corr= [-0.91] |
=====
*****

*****
JP=2+ || eta:eta/1^D_2[-] kaon:kaon/1^D_2[-] pi:pi/1^D_2[+]

sqrt(s)_pole = (0.28309 +/- 0.0012696)
               + (i/2)*(-0.01044 +/- 0.0027296) [-0.63]

=====
eta:eta/1^D_2 | kaon:kaon/1^D_2 | pi:pi/1^D_2 |
=====
k_re= 0.0964 +/- 0.0009 | k_re= 0.1031 +/- 0.0009 | k_re= -0.1236 +/- 0.0007 |
k_im= -0.0038 +/- 0.0010 | k_im= -0.0036 +/- 0.0009 | k_im= 0.0030 +/- 0.0008 |
corr= [-0.63] | corr= [-0.63] | corr= [-0.63] |
=====
|g|= 0.0013 +/- 0.0166 | |g|= 0.0656 +/- 0.0089 | |g|= 0.0160 +/- 0.0058 |
arg(g)/pi= -0.0484 +/- 0.1229 | arg(g)/pi= -0.0615 +/- 0.0117 | arg(g)/pi= -0.2000 +/- 0.2122 |
=====
g_re= 0.0013 +/- 0.0164 | g_re= 0.0644 +/- 0.0087 | g_re= 0.0129 +/- 0.0106 |
g_im= -0.0002 +/- 0.0026 | g_im= -0.0126 +/- 0.0031 | g_im= -0.0094 +/- 0.0059 |
=====

```

```

corr= [-0.98] | corr= [-0.61] | corr= [ 0.87] |
*****

```

```

*****
JP=2+ || eta:eta/1^D_2[-] kaon:kaon/1^D_2[-] pi:pi/1^D_2[-]

```

```

sqrt(s)_pole = (0.25964 +/- 0.0013421)
               + (i/2)*(-0.028244 +/- 0.003193) [-0.21]

```

```

===== eta:eta/1^D_2 | kaon:kaon/1^D_2 | pi:pi/1^D_2 |
k_re= 0.0787 +/- 0.0011 | k_re= 0.0867 +/- 0.0010 | k_re= 0.1100 +/- 0.0008 |
k_im= -0.0116 +/- 0.0013 | k_im= -0.0106 +/- 0.0012 | k_im= -0.0083 +/- 0.0009 |
corr= [-0.24] | corr= [-0.23] | corr= [-0.22] |
=====
|g|= 0.0005 +/- 0.0071 | |g|= 0.0351 +/- 0.0058 | |g|= 0.0854 +/- 0.0045 |
arg(g)/pi= -0.1178 +/- 0.2593 | arg(g)/pi= -0.1086 +/- 0.0148 | arg(g)/pi= -0.1019 +/- 0.0113 |
=====
g_re= 0.0005 +/- 0.0066 | g_re= 0.0330 +/- 0.0054 | g_re= 0.0810 +/- 0.0034 |
g_im= -0.0002 +/- 0.0026 | g_im= -0.0117 +/- 0.0026 | g_im= -0.0269 +/- 0.0042 |
corr= [-0.98] | corr= [-0.75] | corr= [-0.91] |
=====

```

```

*****
JP=2+ || eta:eta/1^D_2[-] kaon:kaon/1^D_2[-] pi:pi/1^D_2[-]

```

```

sqrt(s)_pole = (0.28287 +/- 0.0012613)
               + (i/2)*(-0.0088982 +/- 0.0022775) [-0.15]

```

```

===== eta:eta/1^D_2 | kaon:kaon/1^D_2 | pi:pi/1^D_2 |
k_re= 0.0963 +/- 0.0009 | k_re= 0.1030 +/- 0.0009 | k_re= 0.1234 +/- 0.0007 |
k_im= -0.0033 +/- 0.0008 | k_im= -0.0031 +/- 0.0008 | k_im= -0.0025 +/- 0.0007 |
corr= [-0.14] | corr= [-0.15] | corr= [-0.15] |
=====
|g|= 0.0011 +/- 0.0148 | |g|= 0.0561 +/- 0.0068 | |g|= 0.0161 +/- 0.0057 |
arg(g)/pi= -0.0541 +/- 0.2680 | arg(g)/pi= -0.0741 +/- 0.0311 | arg(g)/pi= 0.2832 +/- 0.1798 |
=====
g_re= 0.0011 +/- 0.0146 | g_re= 0.0546 +/- 0.0060 | g_re= 0.0101 +/- 0.0043 |
g_im= -0.0002 +/- 0.0027 | g_im= -0.0129 +/- 0.0064 | g_im= 0.0125 +/- 0.0098 |
corr= [-0.94] | corr= [-0.63] | corr= [-0.79] |
=====

```

# k\_2poles\_ccxcxc\_noCM

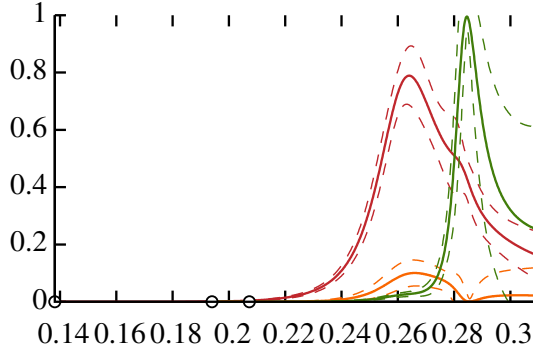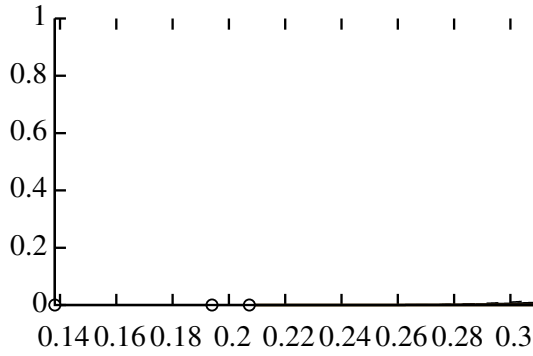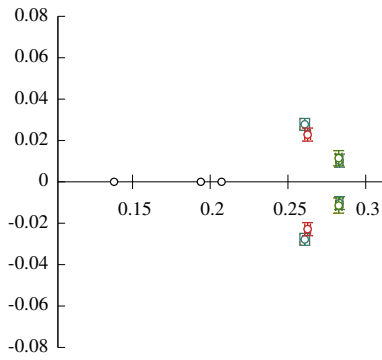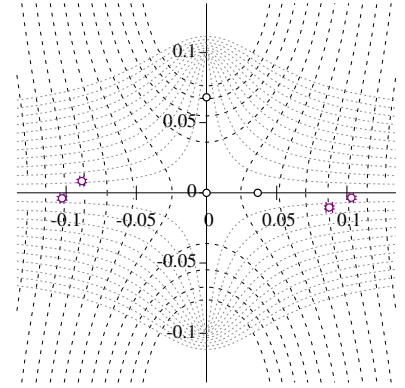

## parameter values

minimised with chisq/nDoF = 26.71 / (34 - 10) = 1.11

|                                               |                       |       |       |       |       |       |       |       |       |      |      |
|-----------------------------------------------|-----------------------|-------|-------|-------|-------|-------|-------|-------|-------|------|------|
| JP2+_g_kaon:kaon/1^D_2_pole0                  | -1.1208 +/- 0.34446   | 1.00  | -0.66 | -0.47 | 0.56  | 0.19  | 0.87  | -0.36 | 0.57  | 0.42 | 0.27 |
| JP2+_g_kaon:kaon/1^D_2_pole1                  | 1.5515 +/- 0.36012    | 1.00  | 0.46  | -0.62 | -0.08 | -0.79 | 0.24  | -0.40 | -0.10 | 0.19 |      |
| JP2+_g_pi:pi/1^D_2_pole0                      | 1.7740 +/- 0.13193    | 1.00  | -0.85 | -0.10 | -0.50 | 0.75  | -0.71 | -0.06 | -0.35 |      |      |
| JP2+_g_pi:pi/1^D_2_pole1                      | 0.057191 +/- 0.34576  | 1.00  | 0.09  | 0.63  | -0.76 | 0.72  | 0.05  | 0.33  |       |      |      |
| JP2+_gamma_eta:eta/1^D_2 eta:eta/1^D_2_order0 | 43.192 +/- 24.994     | 1.00  | 0.20  | -0.14 | 0.22  | -0.05 | -0.05 |       |       |      |      |
| JP2+_gamma_kaon:kaon/1^D_2 kaon:kaon/1^D_2_or | -22.072 +/- 147.05    | 1.00  | -0.49 | 0.65  | 0.36  | 0.13  |       |       |       |      |      |
| JP2+_gamma_kaon:kaon/1^D_2 pi:pi/1^D_2_order0 | -18.908 +/- 83.496    | 1.00  | -0.70 | -0.15 | -0.34 |       |       |       |       |      |      |
| JP2+_gamma_pi:pi/1^D_2 pi:pi/1^D_2_order0     | 32.628 +/- 32.61      | 1.00  | 0.34  | 0.29  |       |       |       |       |       |      |      |
| JP2+_m_pole0                                  | 0.26423 +/- 0.0015839 | 1.00  | 0.30  |       |       |       |       |       |       |      |      |
| JP2+_m_pole1                                  | 0.28444 +/- 0.0016372 | 1.00  |       |       |       |       |       |       |       |      |      |
| JP2+_g_eta:eta/1^D_2_pole0                    | 0.0000 +/- 0          | FIXED |       |       |       |       |       |       |       |      |      |
| JP2+_g_eta:eta/1^D_2_pole1                    | 0.0000 +/- 0          | FIXED |       |       |       |       |       |       |       |      |      |
| JP2+_gamma_eta:eta/1^D_2 kaon:kaon/1^D_2_orde | 0.0000 +/- 0          | FIXED |       |       |       |       |       |       |       |      |      |
| JP2+_gamma_eta:eta/1^D_2 pi:pi/1^D_2_order0   | 0.0000 +/- 0          | FIXED |       |       |       |       |       |       |       |      |      |

## pole singularities

\*\*\*\*\*

\*\*\*\*\*

JP=2+ || eta:eta/1^D\_2[+] kaon:kaon/1^D\_2[+] pi:pi/1^D\_2[-]

sqrt(s)\_pole = (0.26264 +/- 0.0018486)  
+ (i/2)\*(-0.022833 +/- 0.0031726) [-0.04]

| eta:eta/1^D_2                 | kaon:kaon/1^D_2               | pi:pi/1^D_2                   |
|-------------------------------|-------------------------------|-------------------------------|
| k_re= -0.0810 +/- 0.0015      | k_re= -0.0888 +/- 0.0014      | k_re= 0.1118 +/- 0.0011       |
| k_im= 0.0093 +/- 0.0013       | k_im= 0.0084 +/- 0.0012       | k_im= -0.0067 +/- 0.0009      |
| corr= [-0.01]                 | corr= [-0.02]                 | corr= [-0.03]                 |
| g = 0.0000 +/- 0.0000         | g = 0.0323 +/- 0.0112         | g = 0.0893 +/- 0.0052         |
| arg(g)/pi= -0.0735 +/- 0.0671 | arg(g)/pi= -0.1044 +/- 0.0679 | arg(g)/pi= -0.0580 +/- 0.0204 |
| g_re= 0.0000 +/- 0.0000       | g_re= 0.0306 +/- 0.0108       | g_re= 0.0878 +/- 0.0047       |
| g_im= -0.0000 +/- 0.0000      | g_im= -0.0104 +/- 0.0074      | g_im= -0.0162 +/- 0.0061      |
| corr= [-0.31]                 | corr= [-0.28]                 | corr= [-0.42]                 |

\*\*\*\*\*

\*\*\*\*\*  
JP=2+ || eta:eta/1^D\_2[+] kaon:kaon/1^D\_2[-] pi:pi/1^D\_2[+]

sqrt(s)\_pole = (0.28268 +/- 0.0020707)  
+ (i/2)\*(-0.011432 +/- 0.0036848) [ 0.43]

| eta:eta/1^D_2                 | kaon:kaon/1^D_2               | pi:pi/1^D_2                   |
|-------------------------------|-------------------------------|-------------------------------|
| k_re= -0.0962 +/- 0.0015      | k_re= 0.1029 +/- 0.0014       | k_re= -0.1233 +/- 0.0012      |
| k_im= 0.0042 +/- 0.0014       | k_im= -0.0039 +/- 0.0013      | k_im= 0.0033 +/- 0.0011       |
| corr= [ 0.43]                 | corr= [ 0.43]                 | corr= [ 0.43]                 |
| g = 0.0000 +/- 0.0000         | g = 0.0682 +/- 0.0097         | g = 0.0149 +/- 0.0103         |
| arg(g)/pi= -0.0342 +/- 0.0811 | arg(g)/pi= -0.0876 +/- 0.0728 | arg(g)/pi= -0.3799 +/- 0.3047 |
| g_re= 0.0000 +/- 0.0000       | g_re= 0.0656 +/- 0.0070       | g_re= 0.0055 +/- 0.0163       |
| g_im= -0.0000 +/- 0.0000      | g_im= -0.0185 +/- 0.0170      | g_im= -0.0139 +/- 0.0068      |
| corr= [-0.03]                 | corr= [-0.46]                 | corr= [-0.41]                 |

\*\*\*\*\*

\*\*\*\*\*  
JP=2+ || eta:eta/1^D\_2[+] kaon:kaon/1^D\_2[-] pi:pi/1^D\_2[-]

sqrt(s)\_pole = (0.26082 +/- 0.0030935)  
+ (i/2)\*(-0.027786 +/- 0.0028664) [ 0.30]

| eta:eta/1^D_2                 | kaon:kaon/1^D_2               | pi:pi/1^D_2                   |
|-------------------------------|-------------------------------|-------------------------------|
| k_re= -0.0797 +/- 0.0025      | k_re= 0.0875 +/- 0.0023       | k_re= 0.1107 +/- 0.0018       |
| k_im= 0.0114 +/- 0.0012       | k_im= -0.0104 +/- 0.0011      | k_im= -0.0082 +/- 0.0009      |
| corr= [ 0.42]                 | corr= [ 0.39]                 | corr= [ 0.33]                 |
| g = 0.0000 +/- 0.0000         | g = 0.0366 +/- 0.0096         | g = 0.0859 +/- 0.0054         |
| arg(g)/pi= -0.0912 +/- 0.0732 | arg(g)/pi= -0.1016 +/- 0.0946 | arg(g)/pi= -0.0797 +/- 0.0350 |
| g_re= 0.0000 +/- 0.0000       | g_re= 0.0348 +/- 0.0088       | g_re= 0.0832 +/- 0.0067       |
| g_im= -0.0000 +/- 0.0000      | g_im= -0.0115 +/- 0.0116      | g_im= -0.0213 +/- 0.0086      |
| corr= [-0.26]                 | corr= [-0.17]                 | corr= [ 0.64]                 |

\*\*\*\*\*

\*\*\*\*\*  
JP=2+ || eta:eta/1^D\_2[+] kaon:kaon/1^D\_2[-] pi:pi/1^D\_2[-]

sqrt(s)\_pole = (0.28316 +/- 0.0021912)  
+ (i/2)\*(-0.010237 +/- 0.0031496) [-0.11]

| eta:eta/1^D_2                 | kaon:kaon/1^D_2               | pi:pi/1^D_2                  |
|-------------------------------|-------------------------------|------------------------------|
| k_re= -0.0965 +/- 0.0016      | k_re= 0.1032 +/- 0.0015       | k_re= 0.1236 +/- 0.0013      |
| k_im= 0.0038 +/- 0.0012       | k_im= -0.0035 +/- 0.0011      | k_im= -0.0029 +/- 0.0009     |
| corr= [-0.10]                 | corr= [-0.10]                 | corr= [-0.11]                |
| g = 0.0000 +/- 0.0000         | g = 0.0599 +/- 0.0101         | g = 0.0163 +/- 0.0084        |
| arg(g)/pi= -0.0313 +/- 0.0809 | arg(g)/pi= -0.0825 +/- 0.0804 | arg(g)/pi= 0.1629 +/- 0.2463 |
| g_re= 0.0000 +/- 0.0000       | g_re= 0.0579 +/- 0.0104       | g_re= 0.0142 +/- 0.0058      |
| g_im= -0.0000 +/- 0.0000      | g_im= -0.0153 +/- 0.0149      | g_im= 0.0080 +/- 0.0140      |
| corr= [-0.12]                 | corr= [ 0.17]                 | corr= [-0.03]                |

\*\*\*\*\*

\*\*\*\*\*  
JP=2+ || eta:eta/1^D\_2[-] kaon:kaon/1^D\_2[+] pi:pi/1^D\_2[-]

sqrt(s)\_pole = (0.26264 +/- 0.0018486)  
+ (i/2)\*(-0.022833 +/- 0.0031726) [-0.04]

| eta:eta/1^D_2                 | kaon:kaon/1^D_2               | pi:pi/1^D_2                   |
|-------------------------------|-------------------------------|-------------------------------|
| k_re= 0.0810 +/- 0.0015       | k_re= -0.0888 +/- 0.0014      | k_re= 0.1118 +/- 0.0011       |
| k_im= -0.0093 +/- 0.0013      | k_im= 0.0084 +/- 0.0012       | k_im= -0.0067 +/- 0.0009      |
| corr= [-0.01]                 | corr= [-0.02]                 | corr= [-0.03]                 |
| g = 0.0000 +/- 0.0000         | g = 0.0323 +/- 0.0112         | g = 0.0893 +/- 0.0052         |
| arg(g)/pi= -0.0682 +/- 0.0732 | arg(g)/pi= -0.1044 +/- 0.0679 | arg(g)/pi= -0.0580 +/- 0.0204 |
| g_re= 0.0000 +/- 0.0000       | g_re= 0.0306 +/- 0.0108       | g_re= 0.0878 +/- 0.0047       |
| g_im= -0.0000 +/- 0.0000      | g_im= -0.0104 +/- 0.0074      | g_im= -0.0162 +/- 0.0061      |
| corr= [-0.17]                 | corr= [-0.28]                 | corr= [-0.42]                 |

\*\*\*\*\*

\*\*\*\*\*  
JP=2+ || eta:eta/1^D\_2[-] kaon:kaon/1^D\_2[-] pi:pi/1^D\_2[+]

sqrt(s)\_pole = (0.28268 +/- 0.0020707)  
+ (i/2)\*(-0.011432 +/- 0.0036848) [ 0.43]

| eta:eta/1^D_2                 | kaon:kaon/1^D_2               | pi:pi/1^D_2                   |
|-------------------------------|-------------------------------|-------------------------------|
| k_re= 0.0962 +/- 0.0015       | k_re= 0.1029 +/- 0.0014       | k_re= -0.1233 +/- 0.0012      |
| k_im= -0.0042 +/- 0.0014      | k_im= -0.0039 +/- 0.0013      | k_im= 0.0033 +/- 0.0011       |
| corr= [ 0.43]                 | corr= [ 0.43]                 | corr= [ 0.43]                 |
| g = 0.0000 +/- 0.0000         | g = 0.0682 +/- 0.0097         | g = 0.0149 +/- 0.0103         |
| arg(g)/pi= -0.0212 +/- 0.0807 | arg(g)/pi= -0.0876 +/- 0.0728 | arg(g)/pi= -0.3799 +/- 0.3047 |
| g_re= 0.0000 +/- 0.0000       | g_re= 0.0656 +/- 0.0070       | g_re= 0.0055 +/- 0.0163       |
| g_im= -0.0000 +/- 0.0000      | g_im= -0.0185 +/- 0.0170      | g_im= -0.0139 +/- 0.0068      |

```

corr= [ 0.01] | corr= [-0.46] | corr= [-0.41] |
*****

```

```

*****
JP=2+ || eta:eta/1^D_2[-] kaon:kaon/1^D_2[-] pi:pi/1^D_2[-]

```

```

sqrt(s)_pole = (0.26082 +/- 0.0030935)
+ (i/2)*(-0.027786 +/- 0.0028664) [ 0.30]

```

| eta:eta/1^D_2                 |  | kaon:kaon/1^D_2               |  | pi:pi/1^D_2                   |  |
|-------------------------------|--|-------------------------------|--|-------------------------------|--|
| k_re= 0.0797 +/- 0.0025       |  | k_re= 0.0875 +/- 0.0023       |  | k_re= 0.1107 +/- 0.0018       |  |
| k_im= -0.0114 +/- 0.0012      |  | k_im= -0.0104 +/- 0.0011      |  | k_im= -0.0082 +/- 0.0009      |  |
| corr= [ 0.42]                 |  | corr= [ 0.39]                 |  | corr= [ 0.33]                 |  |
| g = 0.0000 +/- 0.0000         |  | g = 0.0366 +/- 0.0096         |  | g = 0.0859 +/- 0.0054         |  |
| arg(g)/pi= -0.0865 +/- 0.0727 |  | arg(g)/pi= -0.1016 +/- 0.0946 |  | arg(g)/pi= -0.0797 +/- 0.0350 |  |
| g_re= 0.0000 +/- 0.0000       |  | g_re= 0.0348 +/- 0.0088       |  | g_re= 0.0832 +/- 0.0067       |  |
| g_im= -0.0000 +/- 0.0000      |  | g_im= -0.0115 +/- 0.0116      |  | g_im= -0.0213 +/- 0.0086      |  |
| corr= [-0.20]                 |  | corr= [-0.17]                 |  | corr= [ 0.64]                 |  |

```

*****
JP=2+ || eta:eta/1^D_2[-] kaon:kaon/1^D_2[-] pi:pi/1^D_2[-]

```

```

sqrt(s)_pole = (0.28316 +/- 0.0021912)
+ (i/2)*(-0.010237 +/- 0.0031496) [-0.11]

```

| eta:eta/1^D_2                 |  | kaon:kaon/1^D_2               |  | pi:pi/1^D_2                  |  |
|-------------------------------|--|-------------------------------|--|------------------------------|--|
| k_re= 0.0965 +/- 0.0016       |  | k_re= 0.1032 +/- 0.0015       |  | k_re= 0.1236 +/- 0.0013      |  |
| k_im= -0.0038 +/- 0.0012      |  | k_im= -0.0035 +/- 0.0011      |  | k_im= -0.0029 +/- 0.0009     |  |
| corr= [-0.10]                 |  | corr= [-0.10]                 |  | corr= [-0.11]                |  |
| g = 0.0000 +/- 0.0000         |  | g = 0.0599 +/- 0.0101         |  | g = 0.0163 +/- 0.0084        |  |
| arg(g)/pi= -0.0181 +/- 0.0779 |  | arg(g)/pi= -0.0825 +/- 0.0804 |  | arg(g)/pi= 0.1629 +/- 0.2463 |  |
| g_re= 0.0000 +/- 0.0000       |  | g_re= 0.0579 +/- 0.0104       |  | g_re= 0.0142 +/- 0.0058      |  |
| g_im= -0.0000 +/- 0.0000      |  | g_im= -0.0153 +/- 0.0149      |  | g_im= 0.0080 +/- 0.0140      |  |
| corr= [-0.11]                 |  | corr= [ 0.17]                 |  | corr= [-0.03]                |  |

# k\_2poles\_ccxxxxc

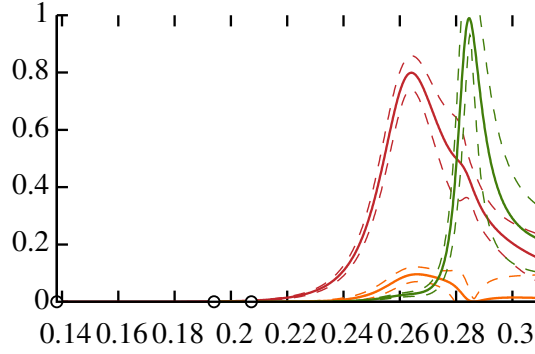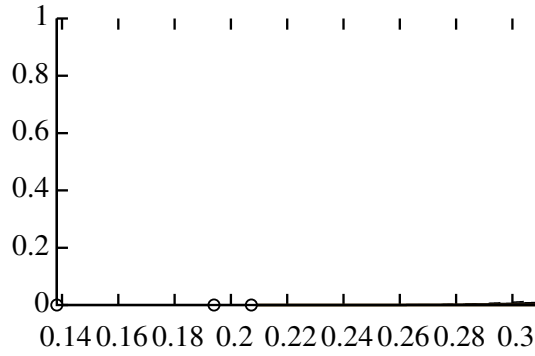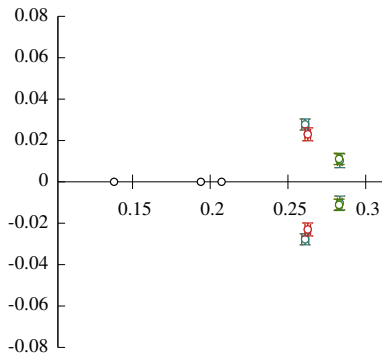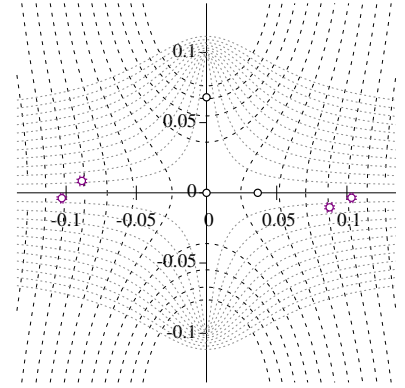

## parameter values

minimised with chisq/nDoF = 26.78 / (34 - 9) = 1.07

|                                               |                       |       |       |       |       |       |      |       |      |      |
|-----------------------------------------------|-----------------------|-------|-------|-------|-------|-------|------|-------|------|------|
| JP2+_g_kaon:kaon/1^D_2_pole0                  | -1.0529 +/- 0.16447   | 1.00  | 0.12  | -0.11 | 0.10  | 0.03  | 0.09 | 0.02  | 0.18 | 0.32 |
| JP2+_g_kaon:kaon/1^D_2_pole1                  | 1.4686 +/- 0.20231    | 1.00  | 0.07  | -0.13 | 0.12  | -0.32 | 0.30 | 0.33  | 0.42 |      |
| JP2+_g_pi:pi/1^D_2_pole0                      | 1.7166 +/- 0.11215    | 1.00  | -0.83 | -0.02 | 0.70  | -0.56 | 0.14 | -0.42 |      |      |
| JP2+_g_pi:pi/1^D_2_pole1                      | 0.11305 +/- 0.27831   | 1.00  | -0.01 | -0.74 | 0.54  | -0.19 | 0.44 |       |      |      |
| JP2+_gamma_eta:eta/1^D_2 eta:eta/1^D_2_order0 | 43.771 +/- 24.732     | 1.00  | -0.06 | 0.12  | -0.16 | -0.08 |      |       |      |      |
| JP2+_gamma_kaon:kaon/1^D_2 pi:pi/1^D_2_order0 | -26.651 +/- 78.806    | 1.00  | -0.57 | 0.01  | -0.39 |       |      |       |      |      |
| JP2+_gamma_pi:pi/1^D_2 pi:pi/1^D_2_order0     | 37.369 +/- 22.564     | 1.00  | 0.20  | 0.31  |       |       |      |       |      |      |
| JP2+_m_pole0                                  | 0.26430 +/- 0.0015557 | 1.00  | 0.27  |       |       |       |      |       |      |      |
| JP2+_m_pole1                                  | 0.28393 +/- 0.0015843 | 1.00  |       |       |       |       |      |       |      |      |
| JP2+_g_eta:eta/1^D_2_pole0                    | 0.0000 +/- 0          | FIXED |       |       |       |       |      |       |      |      |
| JP2+_g_eta:eta/1^D_2_pole1                    | 0.0000 +/- 0          | FIXED |       |       |       |       |      |       |      |      |
| JP2+_gamma_eta:eta/1^D_2 kaon:kaon/1^D_2_orde | 0.0000 +/- 0          | FIXED |       |       |       |       |      |       |      |      |
| JP2+_gamma_eta:eta/1^D_2 pi:pi/1^D_2_order0   | 0.0000 +/- 0          | FIXED |       |       |       |       |      |       |      |      |
| JP2+_gamma_kaon:kaon/1^D_2 kaon:kaon/1^D_2_or | 0.0000 +/- 0          | FIXED |       |       |       |       |      |       |      |      |

## pole singularities

\*\*\*\*\*

\*\*\*\*\*

JP=2+ || eta:eta/1^D\_2[+] kaon:kaon/1^D\_2[+] pi:pi/1^D\_2[-]

sqrt(s)\_pole = (0.26273 +/- 0.001749)  
+ (i/2)\*(-0.022984 +/- 0.003121) [ 0.08]

| eta:eta/1^D_2                 | kaon:kaon/1^D_2               | pi:pi/1^D_2                   |
|-------------------------------|-------------------------------|-------------------------------|
| k_re= -0.0811 +/- 0.0014      | k_re= -0.0888 +/- 0.0013      | k_re= 0.1118 +/- 0.0010       |
| k_im= 0.0093 +/- 0.0013       | k_im= 0.0085 +/- 0.0012       | k_im= -0.0068 +/- 0.0009      |
| corr= [ 0.09]                 | corr= [ 0.09]                 | corr= [ 0.08]                 |
| g = 0.0000 +/- 0.0000         | g = 0.0312 +/- 0.0056         | g = 0.0895 +/- 0.0050         |
| arg(g)/pi= -0.0743 +/- 0.0739 | arg(g)/pi= -0.1040 +/- 0.0739 | arg(g)/pi= -0.0571 +/- 0.0196 |
| g_re= 0.0000 +/- 0.0000       | g_re= 0.0296 +/- 0.0062       | g_re= 0.0880 +/- 0.0047       |
| g_im= -0.0000 +/- 0.0000      | g_im= -0.0100 +/- 0.0068      | g_im= -0.0160 +/- 0.0058      |
| corr= [-0.20]                 | corr= [ 0.28]                 | corr= [-0.33]                 |

\*\*\*\*\*

\*\*\*\*\*  
JP=2+ || eta:eta/1^D\_2[+] kaon:kaon/1^D\_2[-] pi:pi/1^D\_2[+]

sqrt(s)\_pole = (0.28287 +/- 0.0011991)  
+ (i/2)\*(-0.011107 +/- 0.0027016) [-0.31]

| eta:eta/1^D_2                 | kaon:kaon/1^D_2               | pi:pi/1^D_2                   |
|-------------------------------|-------------------------------|-------------------------------|
| k_re= -0.0963 +/- 0.0009      | k_re= 0.1030 +/- 0.0008       | k_re= -0.1234 +/- 0.0007      |
| k_im= 0.0041 +/- 0.0010       | k_im= -0.0038 +/- 0.0009      | k_im= 0.0032 +/- 0.0008       |
| corr= [-0.32]                 | corr= [-0.32]                 | corr= [-0.32]                 |
| g = 0.0000 +/- 0.0000         | g = 0.0673 +/- 0.0071         | g = 0.0140 +/- 0.0059         |
| arg(g)/pi= -0.0330 +/- 0.0827 | arg(g)/pi= -0.0804 +/- 0.0233 | arg(g)/pi= -0.4088 +/- 0.3455 |
| g_re= 0.0000 +/- 0.0000       | g_re= 0.0652 +/- 0.0065       | g_re= 0.0039 +/- 0.0156       |
| g_im= -0.0000 +/- 0.0000      | g_im= -0.0168 +/- 0.0057      | g_im= -0.0134 +/- 0.0047      |
| corr= [-0.11]                 | corr= [-0.51]                 | corr= [ 0.12]                 |

\*\*\*\*\*

\*\*\*\*\*  
JP=2+ || eta:eta/1^D\_2[+] kaon:kaon/1^D\_2[-] pi:pi/1^D\_2[-]

sqrt(s)\_pole = (0.26107 +/- 0.0022563)  
+ (i/2)\*(-0.027732 +/- 0.0026733) [ 0.06]

| eta:eta/1^D_2                 | kaon:kaon/1^D_2               | pi:pi/1^D_2                   |
|-------------------------------|-------------------------------|-------------------------------|
| k_re= -0.0799 +/- 0.0018      | k_re= 0.0877 +/- 0.0017       | k_re= 0.1109 +/- 0.0013       |
| k_im= 0.0113 +/- 0.0011       | k_im= -0.0103 +/- 0.0010      | k_im= -0.0082 +/- 0.0008      |
| corr= [ 0.16]                 | corr= [ 0.13]                 | corr= [ 0.09]                 |
| g = 0.0000 +/- 0.0000         | g = 0.0358 +/- 0.0071         | g = 0.0866 +/- 0.0044         |
| arg(g)/pi= -0.0900 +/- 0.0749 | arg(g)/pi= -0.0946 +/- 0.0747 | arg(g)/pi= -0.0770 +/- 0.0269 |
| g_re= 0.0000 +/- 0.0000       | g_re= 0.0342 +/- 0.0081       | g_re= 0.0840 +/- 0.0050       |
| g_im= -0.0000 +/- 0.0000      | g_im= -0.0105 +/- 0.0074      | g_im= -0.0207 +/- 0.0070      |
| corr= [-0.18]                 | corr= [ 0.44]                 | corr= [ 0.41]                 |

\*\*\*\*\*

\*\*\*\*\*  
JP=2+ || eta:eta/1^D\_2[+] kaon:kaon/1^D\_2[-] pi:pi/1^D\_2[-]

sqrt(s)\_pole = (0.28337 +/- 0.0014723)  
+ (i/2)\*(-0.010207 +/- 0.0033368) [-0.48]

| eta:eta/1^D_2                 | kaon:kaon/1^D_2               | pi:pi/1^D_2                  |
|-------------------------------|-------------------------------|------------------------------|
| k_re= -0.0966 +/- 0.0011      | k_re= 0.1033 +/- 0.0010       | k_re= 0.1237 +/- 0.0008      |
| k_im= 0.0037 +/- 0.0012       | k_im= -0.0035 +/- 0.0011      | k_im= -0.0029 +/- 0.0010     |
| corr= [-0.48]                 | corr= [-0.48]                 | corr= [-0.48]                |
| g = 0.0000 +/- 0.0000         | g = 0.0601 +/- 0.0105         | g = 0.0155 +/- 0.0042        |
| arg(g)/pi= -0.0308 +/- 0.0771 | arg(g)/pi= -0.0739 +/- 0.0294 | arg(g)/pi= 0.1397 +/- 0.2905 |
| g_re= 0.0000 +/- 0.0000       | g_re= 0.0585 +/- 0.0094       | g_re= 0.0141 +/- 0.0055      |
| g_im= -0.0000 +/- 0.0000      | g_im= -0.0138 +/- 0.0073      | g_im= 0.0066 +/- 0.0137      |
| corr= [-0.09]                 | corr= [-0.80]                 | corr= [-0.70]                |

\*\*\*\*\*

\*\*\*\*\*  
JP=2+ || eta:eta/1^D\_2[-] kaon:kaon/1^D\_2[+] pi:pi/1^D\_2[-]

sqrt(s)\_pole = (0.26273 +/- 0.001749)  
+ (i/2)\*(-0.022984 +/- 0.003121) [ 0.08]

| eta:eta/1^D_2                 | kaon:kaon/1^D_2               | pi:pi/1^D_2                   |
|-------------------------------|-------------------------------|-------------------------------|
| k_re= 0.0811 +/- 0.0014       | k_re= -0.0888 +/- 0.0013      | k_re= 0.1118 +/- 0.0010       |
| k_im= -0.0093 +/- 0.0013      | k_im= 0.0085 +/- 0.0012       | k_im= -0.0068 +/- 0.0009      |
| corr= [ 0.09]                 | corr= [ 0.09]                 | corr= [ 0.08]                 |
| g = 0.0000 +/- 0.0000         | g = 0.0312 +/- 0.0056         | g = 0.0895 +/- 0.0050         |
| arg(g)/pi= -0.0682 +/- 0.0733 | arg(g)/pi= -0.1040 +/- 0.0739 | arg(g)/pi= -0.0571 +/- 0.0196 |
| g_re= 0.0000 +/- 0.0000       | g_re= 0.0296 +/- 0.0062       | g_re= 0.0880 +/- 0.0047       |
| g_im= -0.0000 +/- 0.0000      | g_im= -0.0100 +/- 0.0068      | g_im= -0.0160 +/- 0.0058      |
| corr= [-0.16]                 | corr= [ 0.28]                 | corr= [-0.33]                 |

\*\*\*\*\*

\*\*\*\*\*  
JP=2+ || eta:eta/1^D\_2[-] kaon:kaon/1^D\_2[-] pi:pi/1^D\_2[+]

sqrt(s)\_pole = (0.28287 +/- 0.0011991)  
+ (i/2)\*(-0.011107 +/- 0.0027016) [-0.31]

| eta:eta/1^D_2                 | kaon:kaon/1^D_2               | pi:pi/1^D_2                   |
|-------------------------------|-------------------------------|-------------------------------|
| k_re= 0.0963 +/- 0.0009       | k_re= 0.1030 +/- 0.0008       | k_re= -0.1234 +/- 0.0007      |
| k_im= -0.0041 +/- 0.0010      | k_im= -0.0038 +/- 0.0009      | k_im= 0.0032 +/- 0.0008       |
| corr= [-0.32]                 | corr= [-0.32]                 | corr= [-0.32]                 |
| g = 0.0000 +/- 0.0000         | g = 0.0673 +/- 0.0071         | g = 0.0140 +/- 0.0059         |
| arg(g)/pi= -0.0197 +/- 0.0816 | arg(g)/pi= -0.0804 +/- 0.0233 | arg(g)/pi= -0.4088 +/- 0.3455 |
| g_re= 0.0000 +/- 0.0000       | g_re= 0.0652 +/- 0.0065       | g_re= 0.0039 +/- 0.0156       |
| g_im= -0.0000 +/- 0.0000      | g_im= -0.0168 +/- 0.0057      | g_im= -0.0134 +/- 0.0047      |



```

corr= [-0.04] | corr= [-0.51] | corr= [ 0.12] |
*****

```

```

*****
JP=2+ || eta:eta/1^D_2[-] kaon:kaon/1^D_2[-] pi:pi/1^D_2[-]

```

```

sqrt(s)_pole = (0.26107 +/- 0.0022563)
               + (i/2)*(-0.027732 +/- 0.0026733) [ 0.06]

```

```

===== eta:eta/1^D_2 | kaon:kaon/1^D_2 | pi:pi/1^D_2 |
k_re= 0.0799 +/- 0.0018 | k_re= 0.0877 +/- 0.0017 | k_re= 0.1109 +/- 0.0013 |
k_im= -0.0113 +/- 0.0011 | k_im= -0.0103 +/- 0.0010 | k_im= -0.0082 +/- 0.0008 |
corr= [ 0.16] | corr= [ 0.13] | corr= [ 0.09] |
=====
|g|= 0.0000 +/- 0.0000 | |g|= 0.0358 +/- 0.0071 | |g|= 0.0866 +/- 0.0044 |
arg(g)/pi= -0.0853 +/- 0.0786 | arg(g)/pi= -0.0946 +/- 0.0747 | arg(g)/pi= -0.0770 +/- 0.0269 |
=====
g_re= 0.0000 +/- 0.0000 | g_re= 0.0342 +/- 0.0081 | g_re= 0.0840 +/- 0.0050 |
g_im= -0.0000 +/- 0.0000 | g_im= -0.0105 +/- 0.0074 | g_im= -0.0207 +/- 0.0070 |
corr= [-0.14] | corr= [ 0.44] | corr= [ 0.41] |
=====

```

```

*****
JP=2+ || eta:eta/1^D_2[-] kaon:kaon/1^D_2[-] pi:pi/1^D_2[-]

```

```

sqrt(s)_pole = (0.28337 +/- 0.0014723)
               + (i/2)*(-0.010207 +/- 0.0033368) [-0.48]

```

```

===== eta:eta/1^D_2 | kaon:kaon/1^D_2 | pi:pi/1^D_2 |
k_re= 0.0966 +/- 0.0011 | k_re= 0.1033 +/- 0.0010 | k_re= 0.1237 +/- 0.0008 |
k_im= -0.0037 +/- 0.0012 | k_im= -0.0035 +/- 0.0011 | k_im= -0.0029 +/- 0.0010 |
corr= [-0.48] | corr= [-0.48] | corr= [-0.48] |
=====
|g|= 0.0000 +/- 0.0000 | |g|= 0.0601 +/- 0.0105 | |g|= 0.0155 +/- 0.0042 |
arg(g)/pi= -0.0177 +/- 0.0800 | arg(g)/pi= -0.0739 +/- 0.0294 | arg(g)/pi= 0.1397 +/- 0.2905 |
=====
g_re= 0.0000 +/- 0.0000 | g_re= 0.0585 +/- 0.0094 | g_re= 0.0141 +/- 0.0055 |
g_im= -0.0000 +/- 0.0000 | g_im= -0.0138 +/- 0.0073 | g_im= 0.0066 +/- 0.0137 |
corr= [ 0.01] | corr= [-0.80] | corr= [-0.70] |
=====

```

# k\_2poles\_ccxxxc\_noCM

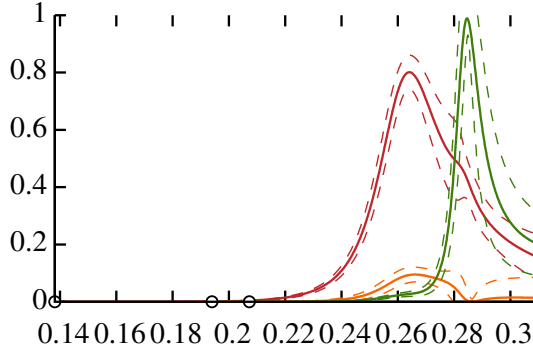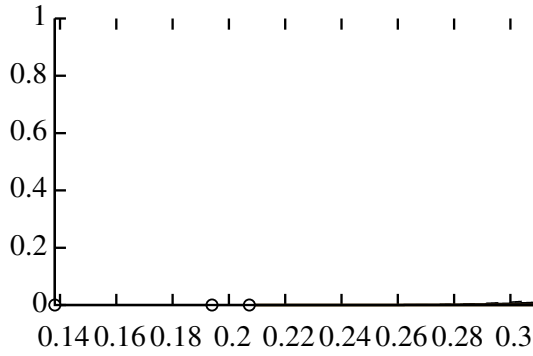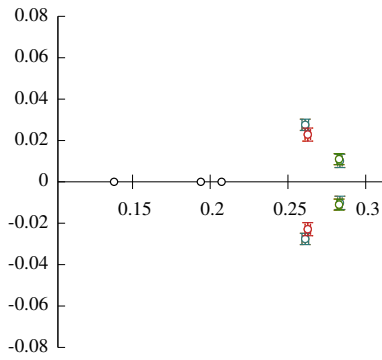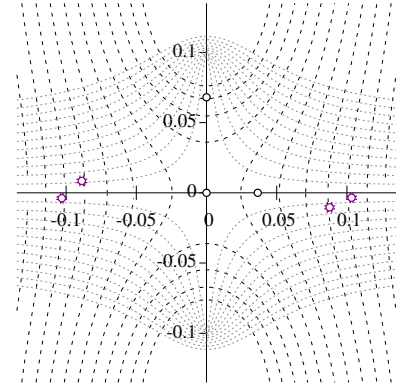

## parameter values

minimised with  $\chi^2/\text{nDoF} = 26.74 / (34 - 9) = 1.07$

|                                               |                       |      |      |       |       |       |       |       |       |       |
|-----------------------------------------------|-----------------------|------|------|-------|-------|-------|-------|-------|-------|-------|
| JP2+_g_kaon:kaon/1^D_2_pole0                  | -1.0758 +/- 0.16999   | 1.00 | 0.09 | -0.11 | 0.08  | 0.03  | 0.13  | -0.00 | 0.15  | 0.30  |
| JP2+_g_kaon:kaon/1^D_2_pole1                  | 1.5063 +/- 0.21767    | 1.00 | 0.08 | -0.16 | 0.12  | -0.32 | 0.29  | 0.32  | 0.47  |       |
| JP2+_g_pi:pi/1^D_2_pole0                      | 1.7633 +/- 0.11909    |      | 1.00 | -0.83 | -0.03 | 0.68  | -0.57 | 0.20  | -0.39 |       |
| JP2+_g_pi:pi/1^D_2_pole1                      | 0.093150 +/- 0.29663  |      |      | 1.00  | -0.01 | -0.72 | 0.53  | -0.26 | 0.41  |       |
| JP2+_gamma_eta:eta/1^D_2 eta:eta/1^D_2_order0 | 44.099 +/- 24.621     |      |      |       | 1.00  | -0.06 | 0.12  | -0.17 | -0.07 |       |
| JP2+_gamma_kaon:kaon/1^D_2 pi:pi/1^D_2_order0 | -25.264 +/- 81.025    |      |      |       |       | 1.00  | -0.57 | 0.06  | -0.39 |       |
| JP2+_gamma_pi:pi/1^D_2 pi:pi/1^D_2_order0     | 35.810 +/- 24.465     |      |      |       |       |       | 1.00  | 0.16  | 0.32  |       |
| JP2+_m_pole0                                  | 0.26429 +/- 0.001616  |      |      |       |       |       |       | 1.00  | 0.23  |       |
| JP2+_m_pole1                                  | 0.28446 +/- 0.0016883 |      |      |       |       |       |       |       | 1.00  |       |
| JP2+_g_eta:eta/1^D_2_pole0                    | 0.0000 +/- 0          |      |      |       |       |       |       |       |       | FIXED |
| JP2+_g_eta:eta/1^D_2_pole1                    | 0.0000 +/- 0          |      |      |       |       |       |       |       |       | FIXED |
| JP2+_gamma_eta:eta/1^D_2 kaon:kaon/1^D_2_orde | 0.0000 +/- 0          |      |      |       |       |       |       |       |       | FIXED |
| JP2+_gamma_eta:eta/1^D_2 pi:pi/1^D_2_order0   | 0.0000 +/- 0          |      |      |       |       |       |       |       |       | FIXED |
| JP2+_gamma_kaon:kaon/1^D_2 kaon:kaon/1^D_2_or | 0.0000 +/- 0          |      |      |       |       |       |       |       |       | FIXED |

## pole singularities

\*\*\*\*\*

\*\*\*\*\*  
JP=2+ || eta:eta/1^D\_2[+] kaon:kaon/1^D\_2[+] pi:pi/1^D\_2[-]

sqrt(s)\_pole = (0.26274 +/- 0.0017397)  
+ (i/2)\*(-0.022869 +/- 0.0031683) [ 0.01]

| eta:eta/1^D_2             | kaon:kaon/1^D_2               | pi:pi/1^D_2                  |
|---------------------------|-------------------------------|------------------------------|
| k_re= -0.0811 +/- 0.0014  | k_re= -0.0888 +/- 0.0013      | k_re= 0.1118 +/- 0.0010      |
| k_im= 0.0093 +/- 0.0013   | k_im= 0.0085 +/- 0.0012       | k_im= -0.0067 +/- 0.0009     |
| corr= [ 0.02]             | corr= [ 0.02]                 | corr= [ 0.01]                |
| g = 0.0000 +/- nan        | g = 0.0309 +/- 0.0056         | g = 0.0891 +/- 0.0052        |
| arg(g)/pi= 0.0000 +/- nan | arg(g)/pi= -0.1035 +/- 0.0710 | arg(g)/pi= 0.9435 +/- 0.0185 |
| g_re= 0.0000 +/- 0.0000   | g_re= 0.0293 +/- 0.0062       | g_re= -0.0877 +/- 0.0048     |
| g_im= 0.0000 +/- 0.0000   | g_im= -0.0099 +/- 0.0064      | g_im= 0.0157 +/- 0.0055      |
| corr= [ 0.00]             | corr= [ 0.28]                 | corr= [-0.37]                |

\*\*\*\*\*

```
*****
JP=2+ || eta:eta/1^D_2[+] kaon:kaon/1^D_2[-] pi:pi/1^D_2[+]

sqrt(s)_pole = (0.28292 +/- 0.0012016)
               + (i/2)*(-0.010998 +/- 0.0026855) [-0.34]

=====
eta:eta/1^D_2 | kaon:kaon/1^D_2 | pi:pi/1^D_2 |
=====
k_re= -0.0963 +/- 0.0009 | k_re= 0.1030 +/- 0.0008 | k_re= -0.1235 +/- 0.0007 |
k_im= 0.0040 +/- 0.0010 | k_im= -0.0038 +/- 0.0009 | k_im= 0.0032 +/- 0.0008 |
corr= [-0.34] | corr= [-0.34] | corr= [-0.34] |
=====
|g|= 0.0000 +/- nan | |g|= 0.0671 +/- 0.0071 | |g|= 0.0138 +/- 0.0052 |
arg(g)/pi= 0.0000 +/- nan | arg(g)/pi= -0.0775 +/- 0.0237 | arg(g)/pi= 0.5891 +/- 0.3345 |
=====
g_re= 0.0000 +/- 0.0000 | g_re= 0.0651 +/- 0.0065 | g_re= -0.0038 +/- 0.0147 |
g_im= 0.0000 +/- 0.0000 | g_im= -0.0162 +/- 0.0058 | g_im= 0.0132 +/- 0.0046 |
corr= [ 0.00] | corr= [-0.49] | corr= [ 0.24] |
=====
*****
```

```
*****
JP=2+ || eta:eta/1^D_2[+] kaon:kaon/1^D_2[-] pi:pi/1^D_2[-]

sqrt(s)_pole = (0.28341 +/- 0.0014498)
               + (i/2)*(-0.010131 +/- 0.0032175) [-0.47]

=====
eta:eta/1^D_2 | kaon:kaon/1^D_2 | pi:pi/1^D_2 |
=====
k_re= -0.0967 +/- 0.0011 | k_re= 0.1034 +/- 0.0010 | k_re= 0.1237 +/- 0.0008 |
k_im= 0.0037 +/- 0.0012 | k_im= -0.0035 +/- 0.0011 | k_im= -0.0029 +/- 0.0009 |
corr= [-0.47] | corr= [-0.47] | corr= [-0.47] |
=====
|g|= 0.0000 +/- nan | |g|= 0.0600 +/- 0.0102 | |g|= 0.0153 +/- 0.0039 |
arg(g)/pi= 0.0000 +/- nan | arg(g)/pi= -0.0709 +/- 0.0291 | arg(g)/pi= 0.1392 +/- 0.2814 |
=====
g_re= 0.0000 +/- 0.0000 | g_re= 0.0586 +/- 0.0091 | g_re= 0.0139 +/- 0.0056 |
g_im= 0.0000 +/- 0.0000 | g_im= -0.0133 +/- 0.0071 | g_im= 0.0065 +/- 0.0129 |
corr= [ 0.00] | corr= [-0.80] | corr= [-0.73] |
=====
*****
```

```
*****
JP=2+ || eta:eta/1^D_2[+] kaon:kaon/1^D_2[-] pi:pi/1^D_2[-]

sqrt(s)_pole = (0.26113 +/- 0.0021345)
               + (i/2)*(-0.027569 +/- 0.0027357) [ 0.06]

=====
eta:eta/1^D_2 | kaon:kaon/1^D_2 | pi:pi/1^D_2 |
=====
k_re= -0.0799 +/- 0.0017 | k_re= 0.0877 +/- 0.0016 | k_re= 0.1109 +/- 0.0013 |
k_im= 0.0113 +/- 0.0011 | k_im= -0.0103 +/- 0.0010 | k_im= -0.0081 +/- 0.0008 |
corr= [ 0.14] | corr= [ 0.12] | corr= [ 0.08] |
=====
|g|= 0.0000 +/- nan | |g|= 0.0355 +/- 0.0070 | |g|= 0.0863 +/- 0.0042 |
arg(g)/pi= 0.0000 +/- nan | arg(g)/pi= -0.0917 +/- 0.0715 | arg(g)/pi= 0.9242 +/- 0.0256 |
=====
g_re= 0.0000 +/- 0.0000 | g_re= 0.0341 +/- 0.0079 | g_re= -0.0839 +/- 0.0044 |
g_im= 0.0000 +/- 0.0000 | g_im= -0.0101 +/- 0.0071 | g_im= 0.0204 +/- 0.0068 |
corr= [ 0.00] | corr= [ 0.41] | corr= [ 0.27] |
=====
*****
```

```
*****
JP=2+ || eta:eta/1^D_2[-] kaon:kaon/1^D_2[+] pi:pi/1^D_2[-]

sqrt(s)_pole = (0.26274 +/- 0.0017397)
               + (i/2)*(-0.022869 +/- 0.0031683) [ 0.01]

=====
eta:eta/1^D_2 | kaon:kaon/1^D_2 | pi:pi/1^D_2 |
=====
k_re= 0.0811 +/- 0.0014 | k_re= -0.0888 +/- 0.0013 | k_re= 0.1118 +/- 0.0010 |
k_im= -0.0093 +/- 0.0013 | k_im= 0.0085 +/- 0.0012 | k_im= -0.0067 +/- 0.0009 |
corr= [ 0.02] | corr= [ 0.02] | corr= [ 0.01] |
=====
|g|= 0.0000 +/- nan | |g|= 0.0309 +/- 0.0056 | |g|= 0.0891 +/- 0.0052 |
arg(g)/pi= 0.0000 +/- nan | arg(g)/pi= -0.1035 +/- 0.0710 | arg(g)/pi= 0.9435 +/- 0.0185 |
=====
g_re= 0.0000 +/- 0.0000 | g_re= 0.0293 +/- 0.0062 | g_re= -0.0877 +/- 0.0048 |
g_im= 0.0000 +/- 0.0000 | g_im= -0.0099 +/- 0.0064 | g_im= 0.0157 +/- 0.0055 |
corr= [ 0.00] | corr= [ 0.28] | corr= [-0.37] |
=====
*****
```

```
*****
JP=2+ || eta:eta/1^D_2[-] kaon:kaon/1^D_2[-] pi:pi/1^D_2[+]

sqrt(s)_pole = (0.28292 +/- 0.0012016)
               + (i/2)*(-0.010998 +/- 0.0026855) [-0.34]

=====
eta:eta/1^D_2 | kaon:kaon/1^D_2 | pi:pi/1^D_2 |
=====
k_re= 0.0963 +/- 0.0009 | k_re= 0.1030 +/- 0.0008 | k_re= -0.1235 +/- 0.0007 |
k_im= -0.0040 +/- 0.0010 | k_im= -0.0038 +/- 0.0009 | k_im= 0.0032 +/- 0.0008 |
corr= [-0.34] | corr= [-0.34] | corr= [-0.34] |
=====
|g|= 0.0000 +/- nan | |g|= 0.0671 +/- 0.0071 | |g|= 0.0138 +/- 0.0052 |
arg(g)/pi= 0.0000 +/- nan | arg(g)/pi= -0.0775 +/- 0.0237 | arg(g)/pi= 0.5891 +/- 0.3345 |
=====
g_re= 0.0000 +/- 0.0000 | g_re= 0.0651 +/- 0.0065 | g_re= -0.0038 +/- 0.0147 |
g_im= 0.0000 +/- 0.0000 | g_im= -0.0162 +/- 0.0058 | g_im= 0.0132 +/- 0.0046 |
=====
*****
```

```

corr= [ 0.00] | corr= [-0.49] | corr= [ 0.24] |
*****

```

```

*****
JP=2+ || eta:eta/1^D_2[-] kaon:kaon/1^D_2[-] pi:pi/1^D_2[-]

```

```

sqrt(s)_pole = (0.28341 +/- 0.0014498)
               + (i/2)*(-0.010131 +/- 0.0032175) [-0.47]

```

| eta:eta/1^D_2             |  | kaon:kaon/1^D_2               |  | pi:pi/1^D_2                  |  |
|---------------------------|--|-------------------------------|--|------------------------------|--|
| k_re= 0.0967 +/- 0.0011   |  | k_re= 0.1034 +/- 0.0010       |  | k_re= 0.1237 +/- 0.0008      |  |
| k_im= -0.0037 +/- 0.0012  |  | k_im= -0.0035 +/- 0.0011      |  | k_im= -0.0029 +/- 0.0009     |  |
| corr= [-0.47]             |  | corr= [-0.47]                 |  | corr= [-0.47]                |  |
| -----                     |  |                               |  |                              |  |
| g = 0.0000 +/- nan        |  | g = 0.0600 +/- 0.0102         |  | g = 0.0153 +/- 0.0039        |  |
| arg(g)/pi= 0.0000 +/- nan |  | arg(g)/pi= -0.0709 +/- 0.0291 |  | arg(g)/pi= 0.1392 +/- 0.2814 |  |
| -----                     |  |                               |  |                              |  |
| g_re= 0.0000 +/- 0.0000   |  | g_re= 0.0586 +/- 0.0091       |  | g_re= 0.0139 +/- 0.0056      |  |
| g_im= 0.0000 +/- 0.0000   |  | g_im= -0.0133 +/- 0.0071      |  | g_im= 0.0065 +/- 0.0129      |  |
| corr= [ 0.00]             |  | corr= [-0.80]                 |  | corr= [-0.73]                |  |

```

*****
JP=2+ || eta:eta/1^D_2[-] kaon:kaon/1^D_2[-] pi:pi/1^D_2[-]

```

```

sqrt(s)_pole = (0.26113 +/- 0.0021345)
               + (i/2)*(-0.027569 +/- 0.0027357) [ 0.06]

```

| eta:eta/1^D_2             |  | kaon:kaon/1^D_2               |  | pi:pi/1^D_2                  |  |
|---------------------------|--|-------------------------------|--|------------------------------|--|
| k_re= 0.0799 +/- 0.0017   |  | k_re= 0.0877 +/- 0.0016       |  | k_re= 0.1109 +/- 0.0013      |  |
| k_im= -0.0113 +/- 0.0011  |  | k_im= -0.0103 +/- 0.0010      |  | k_im= -0.0081 +/- 0.0008     |  |
| corr= [ 0.14]             |  | corr= [ 0.12]                 |  | corr= [ 0.08]                |  |
| -----                     |  |                               |  |                              |  |
| g = 0.0000 +/- nan        |  | g = 0.0355 +/- 0.0070         |  | g = 0.0863 +/- 0.0042        |  |
| arg(g)/pi= 0.0000 +/- nan |  | arg(g)/pi= -0.0917 +/- 0.0715 |  | arg(g)/pi= 0.9242 +/- 0.0256 |  |
| -----                     |  |                               |  |                              |  |
| g_re= 0.0000 +/- 0.0000   |  | g_re= 0.0341 +/- 0.0079       |  | g_re= -0.0839 +/- 0.0044     |  |
| g_im= 0.0000 +/- 0.0000   |  | g_im= -0.0101 +/- 0.0071      |  | g_im= 0.0204 +/- 0.0068      |  |
| corr= [ 0.00]             |  | corr= [ 0.41]                 |  | corr= [ 0.27]                |  |

# k\_2poles\_cxxcxc\_noCM

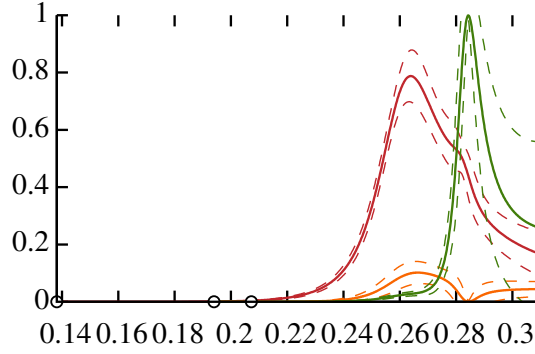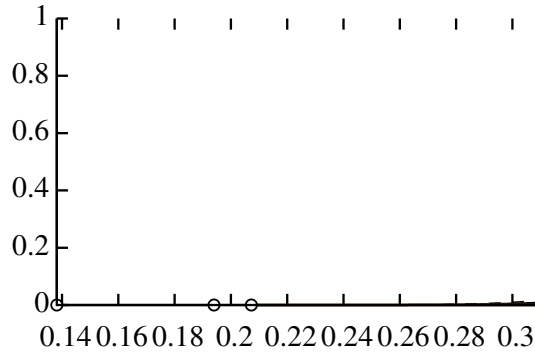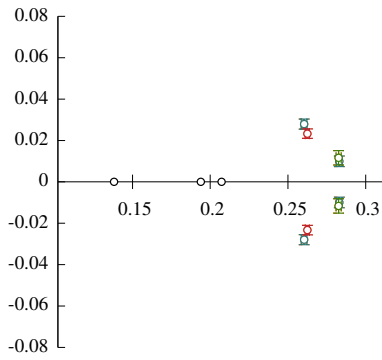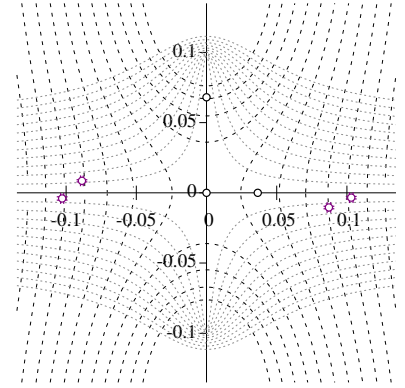

## parameter values

minimised with  $\text{chisq}/\text{nDoF} = 26.78 / (34 - 9) = 1.07$

|                                               |                       |       |       |       |       |       |       |       |      |      |
|-----------------------------------------------|-----------------------|-------|-------|-------|-------|-------|-------|-------|------|------|
| JP2+_g_kaon:kaon/1^D_2_pole0                  | -1.1406 +/- 0.28082   | 1.00  | -0.60 | -0.30 | 0.41  | 0.13  | 0.84  | 0.42  | 0.45 | 0.10 |
| JP2+_g_kaon:kaon/1^D_2_pole1                  | 1.5668 +/- 0.33899    | 1.00  | 0.38  | -0.68 | -0.01 | -0.79 | -0.31 | -0.14 | 0.35 |      |
| JP2+_g_pi:pi/1^D_2_pole0                      | 1.7964 +/- 0.08641    | 1.00  | -0.63 | 0.04  | -0.18 | -0.44 | -0.03 | -0.17 |      |      |
| JP2+_g_pi:pi/1^D_2_pole1                      | 0.0032155 +/- 0.21339 | 1.00  | -0.08 | 0.41  | 0.44  | -0.01 | 0.06  |       |      |      |
| JP2+_gamma_eta:eta/1^D_2 eta:eta/1^D_2_order0 | 42.473 +/- 24.501     | 1.00  | 0.14  | 0.17  | -0.01 | -0.09 |       |       |      |      |
| JP2+_gamma_kaon:kaon/1^D_2 kaon:kaon/1^D_2_or | -35.991 +/- 119.66    | 1.00  | 0.43  | 0.38  | -0.12 |       |       |       |      |      |
| JP2+_gamma_pi:pi/1^D_2 pi:pi/1^D_2_order0     | 27.325 +/- 22.901     | 1.00  | 0.29  | 0.04  |       |       |       |       |      |      |
| JP2+_m_pole0                                  | 0.26420 +/- 0.0010298 | 1.00  | 0.20  |       |       |       |       |       |      |      |
| JP2+_m_pole1                                  | 0.28434 +/- 0.0014938 | 1.00  |       |       |       |       |       |       |      |      |
| JP2+_g_eta:eta/1^D_2_pole0                    | 0.0000 +/- 0          | FIXED |       |       |       |       |       |       |      |      |
| JP2+_g_eta:eta/1^D_2_pole1                    | 0.0000 +/- 0          | FIXED |       |       |       |       |       |       |      |      |
| JP2+_gamma_eta:eta/1^D_2 kaon:kaon/1^D_2_orde | 0.0000 +/- 0          | FIXED |       |       |       |       |       |       |      |      |
| JP2+_gamma_eta:eta/1^D_2 pi:pi/1^D_2_order0   | 0.0000 +/- 0          | FIXED |       |       |       |       |       |       |      |      |
| JP2+_gamma_kaon:kaon/1^D_2 pi:pi/1^D_2_order0 | 0.0000 +/- 0          | FIXED |       |       |       |       |       |       |      |      |

## pole singularities

\*\*\*\*\*

\*\*\*\*\*

JP=2+ || eta:eta/1^D\_2[+] kaon:kaon/1^D\_2[+] pi:pi/1^D\_2[-]

$\text{sqrt}(s)_{\text{pole}} = (0.2625 \pm 0.0013167) + (i/2)(-0.023307 \pm 0.0022781) [-0.05]$

| eta:eta/1^D_2             | kaon:kaon/1^D_2               | pi:pi/1^D_2                  |
|---------------------------|-------------------------------|------------------------------|
| k_re= -0.0809 +/- 0.0011  | k_re= -0.0887 +/- 0.0010      | k_re= 0.1117 +/- 0.0008      |
| k_im= 0.0095 +/- 0.0009   | k_im= 0.0086 +/- 0.0008       | k_im= -0.0068 +/- 0.0007     |
| corr= [-0.03]             | corr= [-0.04]                 | corr= [-0.05]                |
| g = 0.0000 +/- nan        | g = 0.0328 +/- 0.0092         | g = 0.0901 +/- 0.0034        |
| arg(g)/pi= 0.0000 +/- nan | arg(g)/pi= -0.1184 +/- 0.0346 | arg(g)/pi= 0.9386 +/- 0.0148 |
| g_re= 0.0000 +/- 0.0000   | g_re= 0.0306 +/- 0.0097       | g_re= -0.0885 +/- 0.0035     |
| g_im= 0.0000 +/- 0.0000   | g_im= -0.0119 +/- 0.0020      | g_im= 0.0173 +/- 0.0041      |
| corr= [0.00]              | corr= [-0.24]                 | corr= [0.14]                 |

\*\*\*\*\*

\*\*\*\*\*  
JP=2+ || eta:eta/1^D\_2[+] kaon:kaon/1^D\_2[-] pi:pi/1^D\_2[+]

sqrt(s)\_pole = ( 0.2826 +/- 0.0016799)  
+ (i/2)\*(-0.011615 +/- 0.0034803) [ 0.33]

| eta:eta/1^D_2             | kaon:kaon/1^D_2               | pi:pi/1^D_2                  |
|---------------------------|-------------------------------|------------------------------|
| k_re= -0.0961 +/- 0.0012  | k_re= 0.1028 +/- 0.0011       | k_re= -0.1233 +/- 0.0010     |
| k_im= 0.0043 +/- 0.0013   | k_im= -0.0040 +/- 0.0012      | k_im= 0.0033 +/- 0.0010      |
| corr= [ 0.33]             | corr= [ 0.33]                 | corr= [ 0.33]                |
| g = 0.0000 +/- nan        | g = 0.0689 +/- 0.0092         | g = 0.0168 +/- 0.0052        |
| arg(g)/pi= 0.0000 +/- nan | arg(g)/pi= -0.0891 +/- 0.0624 | arg(g)/pi= 0.6619 +/- 0.1725 |
| g_re= 0.0000 +/- 0.0000   | g_re= 0.0662 +/- 0.0065       | g_re= -0.0082 +/- 0.0089     |
| g_im= 0.0000 +/- 0.0000   | g_im= -0.0190 +/- 0.0149      | g_im= 0.0147 +/- 0.0056      |
| corr= [ 0.00]             | corr= [-0.53]                 | corr= [ 0.36]                |

\*\*\*\*\*

\*\*\*\*\*  
JP=2+ || eta:eta/1^D\_2[+] kaon:kaon/1^D\_2[-] pi:pi/1^D\_2[-]

sqrt(s)\_pole = ( 0.2604 +/- 0.0018128)  
+ (i/2)\*(-0.027911 +/- 0.0024398) [ 0.49]

| eta:eta/1^D_2             | kaon:kaon/1^D_2               | pi:pi/1^D_2                  |
|---------------------------|-------------------------------|------------------------------|
| k_re= -0.0793 +/- 0.0014  | k_re= 0.0872 +/- 0.0013       | k_re= 0.1105 +/- 0.0011      |
| k_im= 0.0115 +/- 0.0011   | k_im= -0.0104 +/- 0.0009      | k_im= -0.0082 +/- 0.0007     |
| corr= [ 0.54]             | corr= [ 0.53]                 | corr= [ 0.51]                |
| g = 0.0000 +/- nan        | g = 0.0364 +/- 0.0084         | g = 0.0854 +/- 0.0037        |
| arg(g)/pi= 0.0000 +/- nan | arg(g)/pi= -0.1197 +/- 0.0222 | arg(g)/pi= 0.9148 +/- 0.0201 |
| g_re= 0.0000 +/- 0.0000   | g_re= 0.0338 +/- 0.0072       | g_re= -0.0824 +/- 0.0040     |
| g_im= 0.0000 +/- 0.0000   | g_im= -0.0134 +/- 0.0050      | g_im= 0.0226 +/- 0.0052      |
| corr= [ 0.00]             | corr= [-0.91]                 | corr= [ 0.29]                |

\*\*\*\*\*

\*\*\*\*\*  
JP=2+ || eta:eta/1^D\_2[+] kaon:kaon/1^D\_2[-] pi:pi/1^D\_2[-]

sqrt(s)\_pole = ( 0.283 +/- 0.0018286)  
+ (i/2)\*(-0.0099319 +/- 0.0025652) [ 0.09]

| eta:eta/1^D_2             | kaon:kaon/1^D_2               | pi:pi/1^D_2                  |
|---------------------------|-------------------------------|------------------------------|
| k_re= -0.0964 +/- 0.0013  | k_re= 0.1031 +/- 0.0013       | k_re= 0.1235 +/- 0.0010      |
| k_im= 0.0036 +/- 0.0009   | k_im= -0.0034 +/- 0.0009      | k_im= -0.0028 +/- 0.0007     |
| corr= [ 0.10]             | corr= [ 0.10]                 | corr= [ 0.09]                |
| g = 0.0000 +/- nan        | g = 0.0585 +/- 0.0067         | g = 0.0176 +/- 0.0050        |
| arg(g)/pi= 0.0000 +/- nan | arg(g)/pi= -0.0850 +/- 0.0693 | arg(g)/pi= 0.1953 +/- 0.1377 |
| g_re= 0.0000 +/- 0.0000   | g_re= 0.0564 +/- 0.0059       | g_re= 0.0144 +/- 0.0056      |
| g_im= 0.0000 +/- 0.0000   | g_im= -0.0154 +/- 0.0131      | g_im= 0.0102 +/- 0.0072      |
| corr= [ 0.00]             | corr= [-0.02]                 | corr= [-0.34]                |

\*\*\*\*\*

\*\*\*\*\*  
JP=2+ || eta:eta/1^D\_2[-] kaon:kaon/1^D\_2[+] pi:pi/1^D\_2[-]

sqrt(s)\_pole = ( 0.2625 +/- 0.0013167)  
+ (i/2)\*(-0.023307 +/- 0.0022781) [-0.05]

| eta:eta/1^D_2             | kaon:kaon/1^D_2               | pi:pi/1^D_2                  |
|---------------------------|-------------------------------|------------------------------|
| k_re= 0.0809 +/- 0.0011   | k_re= -0.0887 +/- 0.0010      | k_re= 0.1117 +/- 0.0008      |
| k_im= -0.0095 +/- 0.0009  | k_im= 0.0086 +/- 0.0008       | k_im= -0.0068 +/- 0.0007     |
| corr= [-0.03]             | corr= [-0.04]                 | corr= [-0.05]                |
| g = 0.0000 +/- nan        | g = 0.0328 +/- 0.0092         | g = 0.0901 +/- 0.0034        |
| arg(g)/pi= 0.0000 +/- nan | arg(g)/pi= -0.1184 +/- 0.0346 | arg(g)/pi= 0.9386 +/- 0.0148 |
| g_re= 0.0000 +/- 0.0000   | g_re= 0.0306 +/- 0.0097       | g_re= -0.0885 +/- 0.0035     |
| g_im= 0.0000 +/- 0.0000   | g_im= -0.0119 +/- 0.0020      | g_im= 0.0173 +/- 0.0041      |
| corr= [ 0.00]             | corr= [-0.24]                 | corr= [ 0.14]                |

\*\*\*\*\*

\*\*\*\*\*  
JP=2+ || eta:eta/1^D\_2[-] kaon:kaon/1^D\_2[-] pi:pi/1^D\_2[+]

sqrt(s)\_pole = ( 0.2826 +/- 0.0016799)  
+ (i/2)\*(-0.011615 +/- 0.0034803) [ 0.33]

| eta:eta/1^D_2             | kaon:kaon/1^D_2               | pi:pi/1^D_2                  |
|---------------------------|-------------------------------|------------------------------|
| k_re= 0.0961 +/- 0.0012   | k_re= 0.1028 +/- 0.0011       | k_re= -0.1233 +/- 0.0010     |
| k_im= -0.0043 +/- 0.0013  | k_im= -0.0040 +/- 0.0012      | k_im= 0.0033 +/- 0.0010      |
| corr= [ 0.33]             | corr= [ 0.33]                 | corr= [ 0.33]                |
| g = 0.0000 +/- nan        | g = 0.0689 +/- 0.0092         | g = 0.0168 +/- 0.0052        |
| arg(g)/pi= 0.0000 +/- nan | arg(g)/pi= -0.0891 +/- 0.0624 | arg(g)/pi= 0.6619 +/- 0.1725 |
| g_re= 0.0000 +/- 0.0000   | g_re= 0.0662 +/- 0.0065       | g_re= -0.0082 +/- 0.0089     |
| g_im= 0.0000 +/- 0.0000   | g_im= -0.0190 +/- 0.0149      | g_im= 0.0147 +/- 0.0056      |

```

corr= [ 0.00] | corr= [-0.53] | corr= [ 0.36] |
*****

```

```

*****
JP=2+ || eta:eta/1^D_2[-] kaon:kaon/1^D_2[-] pi:pi/1^D_2[-]

```

```

sqrt(s)_pole = ( 0.2604 +/- 0.0018128)
               + (i/2)*(-0.027911 +/- 0.0024398) [ 0.49]

```

```

===== eta:eta/1^D_2 | kaon:kaon/1^D_2 | pi:pi/1^D_2 |
k_re= 0.0793 +/- 0.0014 | k_re= 0.0872 +/- 0.0013 | k_re= 0.1105 +/- 0.0011 |
k_im= -0.0115 +/- 0.0011 | k_im= -0.0104 +/- 0.0009 | k_im= -0.0082 +/- 0.0007 |
corr= [ 0.54] | corr= [ 0.53] | corr= [ 0.51] |
=====
|g|= 0.0000 +/- nan | |g|= 0.0364 +/- 0.0084 | |g|= 0.0854 +/- 0.0037 |
arg(g)/pi= 0.0000 +/- nan | arg(g)/pi= -0.1197 +/- 0.0222 | arg(g)/pi= 0.9148 +/- 0.0201 |
=====
g_re= 0.0000 +/- 0.0000 | g_re= 0.0338 +/- 0.0072 | g_re= -0.0824 +/- 0.0040 |
g_im= 0.0000 +/- 0.0000 | g_im= -0.0134 +/- 0.0050 | g_im= 0.0226 +/- 0.0052 |
corr= [ 0.00] | corr= [-0.91] | corr= [ 0.29] |
=====

```

```

*****
JP=2+ || eta:eta/1^D_2[-] kaon:kaon/1^D_2[-] pi:pi/1^D_2[-]

```

```

sqrt(s)_pole = ( 0.283 +/- 0.0018286)
               + (i/2)*(-0.0099319 +/- 0.0025652) [ 0.09]

```

```

===== eta:eta/1^D_2 | kaon:kaon/1^D_2 | pi:pi/1^D_2 |
k_re= 0.0964 +/- 0.0013 | k_re= 0.1031 +/- 0.0013 | k_re= 0.1235 +/- 0.0010 |
k_im= -0.0036 +/- 0.0009 | k_im= -0.0034 +/- 0.0009 | k_im= -0.0028 +/- 0.0007 |
corr= [ 0.10] | corr= [ 0.10] | corr= [ 0.09] |
=====
|g|= 0.0000 +/- nan | |g|= 0.0585 +/- 0.0067 | |g|= 0.0176 +/- 0.0050 |
arg(g)/pi= 0.0000 +/- nan | arg(g)/pi= -0.0850 +/- 0.0693 | arg(g)/pi= 0.1953 +/- 0.1377 |
=====
g_re= 0.0000 +/- 0.0000 | g_re= 0.0564 +/- 0.0059 | g_re= 0.0144 +/- 0.0056 |
g_im= 0.0000 +/- 0.0000 | g_im= -0.0154 +/- 0.0131 | g_im= 0.0102 +/- 0.0072 |
corr= [ 0.00] | corr= [-0.02] | corr= [-0.34] |
=====

```

# k\_2poles\_cxxxxc

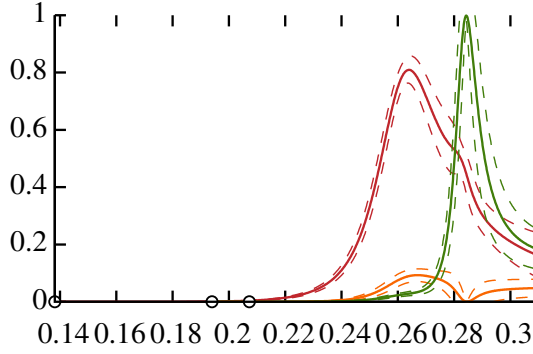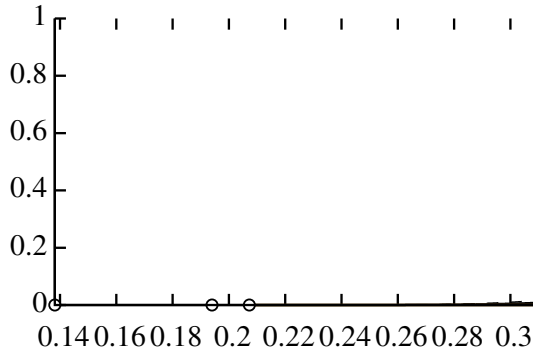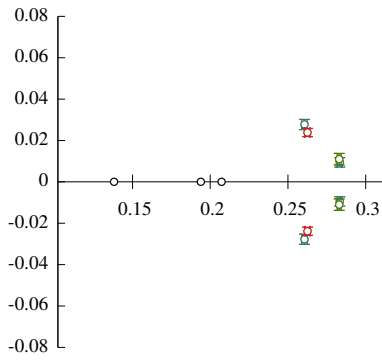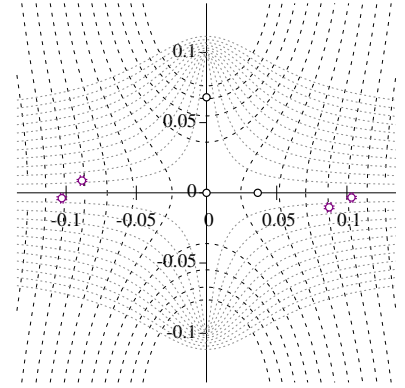

## parameter values

minimised with  $\text{chisq}/\text{nDoF} = 26.92 / (34 - 8) = 1.04$

|                                               |                       |      |      |       |       |       |       |       |       |
|-----------------------------------------------|-----------------------|------|------|-------|-------|-------|-------|-------|-------|
| JP2+_g_kaon:kaon/1^D_2_pole0                  | -1.0404 +/- 0.16622   | 1.00 | 0.22 | -0.28 | 0.16  | 0.01  | 0.16  | 0.32  | 0.42  |
| JP2+_g_kaon:kaon/1^D_2_pole1                  | 1.4471 +/- 0.19708    | 1.00 | 0.37 | -0.60 | 0.14  | 0.11  | 0.34  | 0.37  |       |
| JP2+_g_pi:pi/1^D_2_pole0                      | 1.7445 +/- 0.084187   |      | 1.00 | -0.66 | 0.05  | -0.41 | 0.07  | -0.26 |       |
| JP2+_g_pi:pi/1^D_2_pole1                      | 0.052175 +/- 0.18974  |      |      | 1.00  | -0.12 | 0.33  | -0.22 | 0.19  |       |
| JP2+_gamma_eta:eta/1^D_2 eta:eta/1^D_2_order0 | 43.209 +/- 24.563     |      |      |       | 1.00  | 0.10  | -0.12 | -0.11 |       |
| JP2+_gamma_pi:pi/1^D_2 pi:pi/1^D_2_order0     | 32.053 +/- 19.929     |      |      |       |       | 1.00  | 0.22  | 0.17  |       |
| JP2+_m_pole0                                  | 0.26432 +/- 0.0013724 |      |      |       |       |       | 1.00  | 0.34  |       |
| JP2+_m_pole1                                  | 0.28376 +/- 0.0014513 |      |      |       |       |       |       | 1.00  |       |
| JP2+_g_eta:eta/1^D_2_pole0                    | 0.0000 +/- 0          |      |      |       |       |       |       |       | FIXED |
| JP2+_g_eta:eta/1^D_2_pole1                    | 0.0000 +/- 0          |      |      |       |       |       |       |       | FIXED |
| JP2+_gamma_eta:eta/1^D_2 kaon:kaon/1^D_2_orde | 0.0000 +/- 0          |      |      |       |       |       |       |       | FIXED |
| JP2+_gamma_eta:eta/1^D_2 pi:pi/1^D_2_order0   | 0.0000 +/- 0          |      |      |       |       |       |       |       | FIXED |
| JP2+_gamma_kaon:kaon/1^D_2 kaon:kaon/1^D_2_or | 0.0000 +/- 0          |      |      |       |       |       |       |       | FIXED |
| JP2+_gamma_kaon:kaon/1^D_2 pi:pi/1^D_2_order0 | 0.0000 +/- 0          |      |      |       |       |       |       |       | FIXED |

## pole singularities

\*\*\*\*\*

JP=2+ || eta:eta/1^D\_2[+] kaon:kaon/1^D\_2[+] pi:pi/1^D\_2[-]

$\text{sqrt}(s)_{\text{pole}} = (0.26255 \pm 0.0016675) + (i/2) * (-0.023858 \pm 0.0019785) [-0.11]$

| eta:eta/1^D_2             | kaon:kaon/1^D_2               | pi:pi/1^D_2                  |
|---------------------------|-------------------------------|------------------------------|
| k_re= -0.0809 +/- 0.0013  | k_re= -0.0887 +/- 0.0012      | k_re= 0.1117 +/- 0.0010      |
| k_im= 0.0097 +/- 0.0008   | k_im= 0.0088 +/- 0.0007       | k_im= -0.0070 +/- 0.0006     |
| corr= [-0.03]             | corr= [-0.05]                 | corr= [-0.09]                |
| g = 0.0000 +/- nan        | g = 0.0306 +/- 0.0053         | g = 0.0906 +/- 0.0037        |
| arg(g)/pi= 0.0000 +/- nan | arg(g)/pi= -0.1314 +/- 0.0196 | arg(g)/pi= 0.9376 +/- 0.0157 |
| g_re= 0.0000 +/- 0.0000   | g_re= 0.0281 +/- 0.0053       | g_re= -0.0888 +/- 0.0038     |
| g_im= 0.0000 +/- 0.0000   | g_im= -0.0123 +/- 0.0020      | g_im= 0.0176 +/- 0.0044      |
| corr= [ 0.00]             | corr= [-0.55]                 | corr= [ 0.13]                |

\*\*\*\*\*



```

*****
JP=2+ || eta:eta/1^D_2[+] kaon:kaon/1^D_2[-] pi:pi/1^D_2[+]

sqrt(s)_pole = (0.28296 +/- 0.0012535)
               + (i/2)*(-0.010991 +/- 0.0028063) [-0.48]

eta:eta/1^D_2 | kaon:kaon/1^D_2 | pi:pi/1^D_2 |
=====|=====|=====|
k_re= -0.0964 +/- 0.0009 | k_re= 0.1030 +/- 0.0009 | k_re= -0.1235 +/- 0.0007 |
k_im= 0.0040 +/- 0.0010 | k_im= -0.0038 +/- 0.0010 | k_im= 0.0031 +/- 0.0008 |
corr= [-0.49] | corr= [-0.48] | corr= [-0.48] |
=====|=====|=====|
|g|= 0.0000 +/- nan | |g|= 0.0673 +/- 0.0080 | |g|= 0.0160 +/- 0.0029 |
arg(g)/pi= 0.0000 +/- nan | arg(g)/pi= -0.0723 +/- 0.0114 | arg(g)/pi= 0.6602 +/- 0.2021 |
-----|-----|-----|
g_re= 0.0000 +/- 0.0000 | g_re= 0.0656 +/- 0.0075 | g_re= -0.0077 +/- 0.0095 |
g_im= 0.0000 +/- 0.0000 | g_im= -0.0152 +/- 0.0036 | g_im= 0.0140 +/- 0.0045 |
corr= [ 0.00] | corr= [-0.79] | corr= [ 0.78] |
*****

```

```

*****
JP=2+ || eta:eta/1^D_2[+] kaon:kaon/1^D_2[-] pi:pi/1^D_2[-]

sqrt(s)_pole = (0.26062 +/- 0.0017768)
               + (i/2)*(-0.027722 +/- 0.0024885) [ 0.16]

eta:eta/1^D_2 | kaon:kaon/1^D_2 | pi:pi/1^D_2 |
=====|=====|=====|
k_re= -0.0795 +/- 0.0014 | k_re= 0.0874 +/- 0.0013 | k_re= 0.1106 +/- 0.0010 |
k_im= 0.0114 +/- 0.0010 | k_im= -0.0103 +/- 0.0009 | k_im= -0.0082 +/- 0.0007 |
corr= [ 0.22] | corr= [ 0.20] | corr= [ 0.17] |
=====|=====|=====|
|g|= 0.0000 +/- nan | |g|= 0.0342 +/- 0.0054 | |g|= 0.0859 +/- 0.0035 |
arg(g)/pi= 0.0000 +/- nan | arg(g)/pi= -0.1201 +/- 0.0136 | arg(g)/pi= 0.9165 +/- 0.0185 |
-----|-----|-----|
g_re= 0.0000 +/- 0.0000 | g_re= 0.0318 +/- 0.0049 | g_re= -0.0830 +/- 0.0035 |
g_im= 0.0000 +/- 0.0000 | g_im= -0.0126 +/- 0.0026 | g_im= 0.0223 +/- 0.0050 |
corr= [ 0.00] | corr= [-0.80] | corr= [ 0.04] |
*****

```

```

*****
JP=2+ || eta:eta/1^D_2[+] kaon:kaon/1^D_2[-] pi:pi/1^D_2[-]

sqrt(s)_pole = (0.28331 +/- 0.0015185)
               + (i/2)*(-0.0094783 +/- 0.0022939) [-0.44]

eta:eta/1^D_2 | kaon:kaon/1^D_2 | pi:pi/1^D_2 |
=====|=====|=====|
k_re= -0.0966 +/- 0.0011 | k_re= 0.1033 +/- 0.0010 | k_re= 0.1237 +/- 0.0009 |
k_im= 0.0035 +/- 0.0008 | k_im= -0.0033 +/- 0.0008 | k_im= -0.0027 +/- 0.0007 |
corr= [-0.43] | corr= [-0.43] | corr= [-0.43] |
=====|=====|=====|
|g|= 0.0000 +/- nan | |g|= 0.0576 +/- 0.0071 | |g|= 0.0168 +/- 0.0028 |
arg(g)/pi= 0.0000 +/- nan | arg(g)/pi= -0.0668 +/- 0.0249 | arg(g)/pi= 0.1959 +/- 0.1642 |
-----|-----|-----|
g_re= 0.0000 +/- 0.0000 | g_re= 0.0564 +/- 0.0066 | g_re= 0.0137 +/- 0.0048 |
g_im= 0.0000 +/- 0.0000 | g_im= -0.0120 +/- 0.0052 | g_im= 0.0097 +/- 0.0077 |
corr= [ 0.00] | corr= [-0.56] | corr= [-0.78] |
*****

```

```

*****
JP=2+ || eta:eta/1^D_2[-] kaon:kaon/1^D_2[+] pi:pi/1^D_2[-]

sqrt(s)_pole = (0.26255 +/- 0.0016675)
               + (i/2)*(-0.023858 +/- 0.0019785) [-0.11]

eta:eta/1^D_2 | kaon:kaon/1^D_2 | pi:pi/1^D_2 |
=====|=====|=====|
k_re= 0.0809 +/- 0.0013 | k_re= -0.0887 +/- 0.0012 | k_re= 0.1117 +/- 0.0010 |
k_im= -0.0097 +/- 0.0008 | k_im= 0.0088 +/- 0.0007 | k_im= -0.0070 +/- 0.0006 |
corr= [-0.03] | corr= [-0.05] | corr= [-0.09] |
=====|=====|=====|
|g|= 0.0000 +/- nan | |g|= 0.0306 +/- 0.0053 | |g|= 0.0906 +/- 0.0037 |
arg(g)/pi= 0.0000 +/- nan | arg(g)/pi= -0.1314 +/- 0.0196 | arg(g)/pi= 0.9376 +/- 0.0157 |
-----|-----|-----|
g_re= 0.0000 +/- 0.0000 | g_re= 0.0281 +/- 0.0053 | g_re= -0.0888 +/- 0.0038 |
g_im= 0.0000 +/- 0.0000 | g_im= -0.0123 +/- 0.0020 | g_im= 0.0176 +/- 0.0044 |
corr= [ 0.00] | corr= [-0.55] | corr= [ 0.13] |
*****

```

```

*****
JP=2+ || eta:eta/1^D_2[-] kaon:kaon/1^D_2[-] pi:pi/1^D_2[+]

sqrt(s)_pole = (0.28296 +/- 0.0012535)
               + (i/2)*(-0.010991 +/- 0.0028063) [-0.48]

eta:eta/1^D_2 | kaon:kaon/1^D_2 | pi:pi/1^D_2 |
=====|=====|=====|
k_re= 0.0964 +/- 0.0009 | k_re= 0.1030 +/- 0.0009 | k_re= -0.1235 +/- 0.0007 |
k_im= -0.0040 +/- 0.0010 | k_im= -0.0038 +/- 0.0010 | k_im= 0.0031 +/- 0.0008 |
corr= [-0.49] | corr= [-0.48] | corr= [-0.48] |
=====|=====|=====|
|g|= 0.0000 +/- nan | |g|= 0.0673 +/- 0.0080 | |g|= 0.0160 +/- 0.0029 |
arg(g)/pi= 0.0000 +/- nan | arg(g)/pi= -0.0723 +/- 0.0114 | arg(g)/pi= 0.6602 +/- 0.2021 |
-----|-----|-----|
g_re= 0.0000 +/- 0.0000 | g_re= 0.0656 +/- 0.0075 | g_re= -0.0077 +/- 0.0095 |
g_im= 0.0000 +/- 0.0000 | g_im= -0.0152 +/- 0.0036 | g_im= 0.0140 +/- 0.0045 |

```

```

corr= [ 0.00] | corr= [-0.79] | corr= [ 0.78] |
*****

```

```

*****
JP=2+ || eta:eta/1^D_2[-] kaon:kaon/1^D_2[-] pi:pi/1^D_2[-]

```

```

sqrt(s)_pole = (0.26062 +/- 0.0017768)
               + (i/2)*(-0.027722 +/- 0.0024885) [ 0.16]

```

```

===== eta:eta/1^D_2 | kaon:kaon/1^D_2 | pi:pi/1^D_2 |
k_re= 0.0795 +/- 0.0014 | k_re= 0.0874 +/- 0.0013 | k_re= 0.1106 +/- 0.0010 |
k_im= -0.0114 +/- 0.0010 | k_im= -0.0103 +/- 0.0009 | k_im= -0.0082 +/- 0.0007 |
corr= [ 0.22] | corr= [ 0.20] | corr= [ 0.17] |
=====
|g|= 0.0000 +/- nan | |g|= 0.0342 +/- 0.0054 | |g|= 0.0859 +/- 0.0035 |
arg(g)/pi= 0.0000 +/- nan | arg(g)/pi= -0.1201 +/- 0.0136 | arg(g)/pi= 0.9165 +/- 0.0185 |
=====
g_re= 0.0000 +/- 0.0000 | g_re= 0.0318 +/- 0.0049 | g_re= -0.0830 +/- 0.0035 |
g_im= 0.0000 +/- 0.0000 | g_im= -0.0126 +/- 0.0026 | g_im= 0.0223 +/- 0.0050 |
corr= [ 0.00] | corr= [-0.80] | corr= [ 0.04] |
=====

```

```

*****
JP=2+ || eta:eta/1^D_2[-] kaon:kaon/1^D_2[-] pi:pi/1^D_2[-]

```

```

sqrt(s)_pole = (0.28331 +/- 0.0015185)
               + (i/2)*(-0.0094783 +/- 0.0022939) [-0.44]

```

```

===== eta:eta/1^D_2 | kaon:kaon/1^D_2 | pi:pi/1^D_2 |
k_re= 0.0966 +/- 0.0011 | k_re= 0.1033 +/- 0.0010 | k_re= 0.1237 +/- 0.0009 |
k_im= -0.0035 +/- 0.0008 | k_im= -0.0033 +/- 0.0008 | k_im= -0.0027 +/- 0.0007 |
corr= [-0.43] | corr= [-0.43] | corr= [-0.43] |
=====
|g|= 0.0000 +/- nan | |g|= 0.0576 +/- 0.0071 | |g|= 0.0168 +/- 0.0028 |
arg(g)/pi= 0.0000 +/- nan | arg(g)/pi= -0.0668 +/- 0.0249 | arg(g)/pi= 0.1959 +/- 0.1642 |
=====
g_re= 0.0000 +/- 0.0000 | g_re= 0.0564 +/- 0.0066 | g_re= 0.0137 +/- 0.0048 |
g_im= 0.0000 +/- 0.0000 | g_im= -0.0120 +/- 0.0052 | g_im= 0.0097 +/- 0.0077 |
corr= [ 0.00] | corr= [-0.56] | corr= [-0.78] |
=====

```

# k\_2poles\_cxxxxc\_noCM

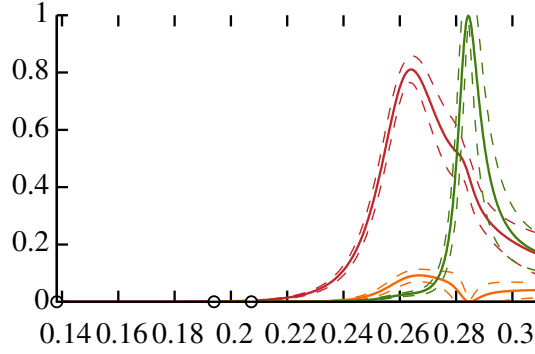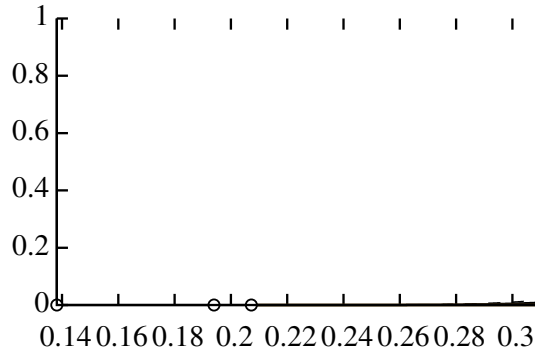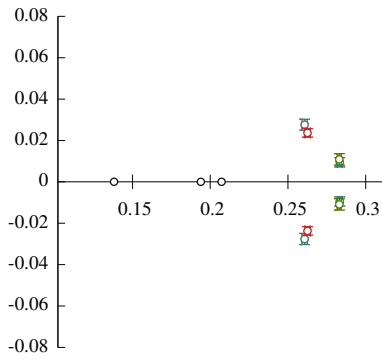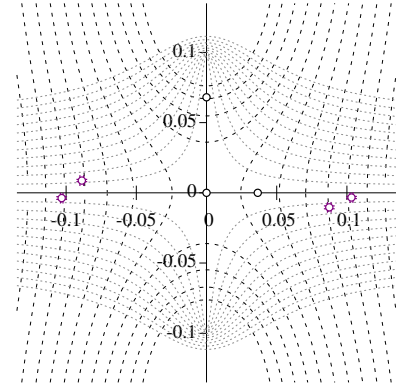

## parameter values

minimised with  $\text{chisq}/\text{nDoF} = 26.86 / (34 - 8) = 1.03$

|                                               |                       |       |       |       |       |      |       |      |      |
|-----------------------------------------------|-----------------------|-------|-------|-------|-------|------|-------|------|------|
| JP2+_g_kaon:kaon/1^D_2_pole0                  | -1.0631 +/- 0.16708   | 1.00  | 0.16  | -0.29 | 0.18  | 0.03 | 0.14  | 0.18 | 0.39 |
| JP2+_g_kaon:kaon/1^D_2_pole1                  | 1.4841 +/- 0.21222    | 1.00  | 0.42  | -0.64 | 0.12  | 0.09 | 0.36  | 0.42 |      |
| JP2+_g_pi:pi/1^D_2_pole0                      | 1.7898 +/- 0.091489   | 1.00  | -0.67 | 0.03  | -0.39 | 0.21 | -0.19 |      |      |
| JP2+_g_pi:pi/1^D_2_pole1                      | 0.034618 +/- 0.20811  | 1.00  | -0.10 | 0.30  | -0.32 | 0.12 |       |      |      |
| JP2+_gamma_eta:eta/1^D_2 eta:eta/1^D_2_order0 | 43.591 +/- 24.499     | 1.00  | 0.10  | -0.15 | -0.09 |      |       |      |      |
| JP2+_gamma_pi:pi/1^D_2 pi:pi/1^D_2_order0     | 30.582 +/- 21.251     | 1.00  | 0.19  | 0.16  |       |      |       |      |      |
| JP2+_m_pole0                                  | 0.26432 +/- 0.0015386 | 1.00  | 0.30  |       |       |      |       |      |      |
| JP2+_m_pole1                                  | 0.28430 +/- 0.001538  | 1.00  |       |       |       |      |       |      |      |
| JP2+_g_eta:eta/1^D_2_pole0                    | 0.0000 +/- 0          | FIXED |       |       |       |      |       |      |      |
| JP2+_g_eta:eta/1^D_2_pole1                    | 0.0000 +/- 0          | FIXED |       |       |       |      |       |      |      |
| JP2+_gamma_eta:eta/1^D_2 kaon:kaon/1^D_2_orde | 0.0000 +/- 0          | FIXED |       |       |       |      |       |      |      |
| JP2+_gamma_eta:eta/1^D_2 pi:pi/1^D_2_order0   | 0.0000 +/- 0          | FIXED |       |       |       |      |       |      |      |
| JP2+_gamma_kaon:kaon/1^D_2 kaon:kaon/1^D_2_or | 0.0000 +/- 0          | FIXED |       |       |       |      |       |      |      |
| JP2+_gamma_kaon:kaon/1^D_2 pi:pi/1^D_2_order0 | 0.0000 +/- 0          | FIXED |       |       |       |      |       |      |      |

## pole singularities

\*\*\*\*\*

\*\*\*\*\*

JP=2+ || eta:eta/1^D\_2[+] kaon:kaon/1^D\_2[+] pi:pi/1^D\_2[-]

$\text{sqrt}(s)_{\text{pole}} = (0.26261 \pm 0.0017421) + (i/2) \cdot (-0.023684 \pm 0.0020747) [-0.21]$

| eta:eta/1^D_2             | kaon:kaon/1^D_2               | pi:pi/1^D_2                  |
|---------------------------|-------------------------------|------------------------------|
| k_re= -0.0810 +/- 0.0014  | k_re= -0.0888 +/- 0.0013      | k_re= 0.1117 +/- 0.0010      |
| k_im= 0.0096 +/- 0.0008   | k_im= 0.0088 +/- 0.0008       | k_im= -0.0070 +/- 0.0006     |
| corr= [-0.13]             | corr= [-0.15]                 | corr= [-0.19]                |
| g = 0.0000 +/- nan        | g = 0.0304 +/- 0.0052         | g = 0.0902 +/- 0.0039        |
| arg(g)/pi= 0.0000 +/- nan | arg(g)/pi= -0.1277 +/- 0.0204 | arg(g)/pi= 0.9392 +/- 0.0153 |
| g_re= 0.0000 +/- 0.0000   | g_re= 0.0280 +/- 0.0052       | g_re= -0.0886 +/- 0.0039     |
| g_im= 0.0000 +/- 0.0000   | g_im= -0.0119 +/- 0.0020      | g_im= 0.0171 +/- 0.0043      |
| corr= [0.00]              | corr= [-0.50]                 | corr= [0.05]                 |

\*\*\*\*\*

\*\*\*\*\*  
JP=2+ || eta:eta/1^D\_2[+] kaon:kaon/1^D\_2[-] pi:pi/1^D\_2[+]

sqrt(s)\_pole = ( 0.283 +/- 0.0012612)  
+ (i/2)\*(-0.010864 +/- 0.0027907) [-0.49]

| eta:eta/1^D_2 |                    |  | kaon:kaon/1^D_2 |                    |  | pi:pi/1^D_2 |                    |  |
|---------------|--------------------|--|-----------------|--------------------|--|-------------|--------------------|--|
| k_re=         | -0.0964 +/- 0.0009 |  | k_re=           | 0.1031 +/- 0.0009  |  | k_re=       | -0.1235 +/- 0.0007 |  |
| k_im=         | 0.0040 +/- 0.0010  |  | k_im=           | -0.0037 +/- 0.0010 |  | k_im=       | 0.0031 +/- 0.0008  |  |
| corr=         | [-0.50]            |  | corr=           | [-0.50]            |  | corr=       | [-0.49]            |  |
| =====         |                    |  |                 |                    |  |             |                    |  |
| g =           | 0.0000 +/- nan     |  | g =             | 0.0669 +/- 0.0080  |  | g =         | 0.0154 +/- 0.0027  |  |
| arg(g)/pi=    | 0.0000 +/- nan     |  | arg(g)/pi=      | -0.0700 +/- 0.0107 |  | arg(g)/pi=  | 0.6491 +/- 0.2118  |  |
| -----         |                    |  |                 |                    |  |             |                    |  |
| g_re=         | 0.0000 +/- 0.0000  |  | g_re=           | 0.0653 +/- 0.0075  |  | g_re=       | -0.0069 +/- 0.0095 |  |
| g_im=         | 0.0000 +/- 0.0000  |  | g_im=           | -0.0146 +/- 0.0034 |  | g_im=       | 0.0137 +/- 0.0046  |  |
| corr=         | [ 0.00]            |  | corr=           | [-0.78]            |  | corr=       | [ 0.80]            |  |

\*\*\*\*\*

\*\*\*\*\*  
JP=2+ || eta:eta/1^D\_2[+] kaon:kaon/1^D\_2[-] pi:pi/1^D\_2[-]

sqrt(s)\_pole = (0.26076 +/- 0.0017598)  
+ (i/2)\*(-0.027622 +/- 0.0027022) [ 0.00]

| eta:eta/1^D_2 |                    |  | kaon:kaon/1^D_2 |                    |  | pi:pi/1^D_2 |                    |  |
|---------------|--------------------|--|-----------------|--------------------|--|-------------|--------------------|--|
| k_re=         | -0.0796 +/- 0.0014 |  | k_re=           | 0.0875 +/- 0.0013  |  | k_re=       | 0.1107 +/- 0.0010  |  |
| k_im=         | 0.0113 +/- 0.0011  |  | k_im=           | -0.0103 +/- 0.0010 |  | k_im=       | -0.0081 +/- 0.0008 |  |
| corr=         | [ 0.05]            |  | corr=           | [ 0.03]            |  | corr=       | [ 0.01]            |  |
| =====         |                    |  |                 |                    |  |             |                    |  |
| g =           | 0.0000 +/- nan     |  | g =             | 0.0342 +/- 0.0056  |  | g =         | 0.0859 +/- 0.0038  |  |
| arg(g)/pi=    | 0.0000 +/- nan     |  | arg(g)/pi=      | -0.1144 +/- 0.0138 |  | arg(g)/pi=  | 0.9186 +/- 0.0179  |  |
| -----         |                    |  |                 |                    |  |             |                    |  |
| g_re=         | 0.0000 +/- 0.0000  |  | g_re=           | 0.0320 +/- 0.0052  |  | g_re=       | -0.0832 +/- 0.0036 |  |
| g_im=         | 0.0000 +/- 0.0000  |  | g_im=           | -0.0120 +/- 0.0025 |  | g_im=       | 0.0217 +/- 0.0050  |  |
| corr=         | [ 0.00]            |  | corr=           | [-0.78]            |  | corr=       | [-0.13]            |  |

\*\*\*\*\*

\*\*\*\*\*  
JP=2+ || eta:eta/1^D\_2[+] kaon:kaon/1^D\_2[-] pi:pi/1^D\_2[-]

sqrt(s)\_pole = (0.28338 +/- 0.0015006)  
+ (i/2)\*(-0.0094925 +/- 0.0022691) [-0.44]

| eta:eta/1^D_2 |                    |  | kaon:kaon/1^D_2 |                    |  | pi:pi/1^D_2 |                    |  |
|---------------|--------------------|--|-----------------|--------------------|--|-------------|--------------------|--|
| k_re=         | -0.0967 +/- 0.0011 |  | k_re=           | 0.1033 +/- 0.0010  |  | k_re=       | 0.1237 +/- 0.0009  |  |
| k_im=         | 0.0035 +/- 0.0008  |  | k_im=           | -0.0033 +/- 0.0008 |  | k_im=       | -0.0027 +/- 0.0006 |  |
| corr=         | [-0.43]            |  | corr=           | [-0.43]            |  | corr=       | [-0.43]            |  |
| =====         |                    |  |                 |                    |  |             |                    |  |
| g =           | 0.0000 +/- nan     |  | g =             | 0.0579 +/- 0.0071  |  | g =         | 0.0163 +/- 0.0027  |  |
| arg(g)/pi=    | 0.0000 +/- nan     |  | arg(g)/pi=      | -0.0641 +/- 0.0243 |  | arg(g)/pi=  | 0.1883 +/- 0.1727  |  |
| -----         |                    |  |                 |                    |  |             |                    |  |
| g_re=         | 0.0000 +/- 0.0000  |  | g_re=           | 0.0567 +/- 0.0066  |  | g_re=       | 0.0135 +/- 0.0049  |  |
| g_im=         | 0.0000 +/- 0.0000  |  | g_im=           | -0.0116 +/- 0.0052 |  | g_im=       | 0.0091 +/- 0.0078  |  |
| corr=         | [ 0.00]            |  | corr=           | [-0.58]            |  | corr=       | [-0.80]            |  |

\*\*\*\*\*

\*\*\*\*\*  
JP=2+ || eta:eta/1^D\_2[-] kaon:kaon/1^D\_2[+] pi:pi/1^D\_2[-]

sqrt(s)\_pole = (0.26261 +/- 0.0017421)  
+ (i/2)\*(-0.023684 +/- 0.0020747) [-0.21]

| eta:eta/1^D_2 |                    |  | kaon:kaon/1^D_2 |                    |  | pi:pi/1^D_2 |                    |  |
|---------------|--------------------|--|-----------------|--------------------|--|-------------|--------------------|--|
| k_re=         | 0.0810 +/- 0.0014  |  | k_re=           | -0.0888 +/- 0.0013 |  | k_re=       | 0.1117 +/- 0.0010  |  |
| k_im=         | -0.0096 +/- 0.0008 |  | k_im=           | 0.0088 +/- 0.0008  |  | k_im=       | -0.0070 +/- 0.0006 |  |
| corr=         | [-0.13]            |  | corr=           | [-0.15]            |  | corr=       | [-0.19]            |  |
| =====         |                    |  |                 |                    |  |             |                    |  |
| g =           | 0.0000 +/- nan     |  | g =             | 0.0304 +/- 0.0052  |  | g =         | 0.0902 +/- 0.0039  |  |
| arg(g)/pi=    | 0.0000 +/- nan     |  | arg(g)/pi=      | -0.1277 +/- 0.0204 |  | arg(g)/pi=  | 0.9392 +/- 0.0153  |  |
| -----         |                    |  |                 |                    |  |             |                    |  |
| g_re=         | 0.0000 +/- 0.0000  |  | g_re=           | 0.0280 +/- 0.0052  |  | g_re=       | -0.0886 +/- 0.0039 |  |
| g_im=         | 0.0000 +/- 0.0000  |  | g_im=           | -0.0119 +/- 0.0020 |  | g_im=       | 0.0171 +/- 0.0043  |  |
| corr=         | [ 0.00]            |  | corr=           | [-0.50]            |  | corr=       | [ 0.05]            |  |

\*\*\*\*\*

\*\*\*\*\*  
JP=2+ || eta:eta/1^D\_2[-] kaon:kaon/1^D\_2[-] pi:pi/1^D\_2[+]

sqrt(s)\_pole = ( 0.283 +/- 0.0012612)  
+ (i/2)\*(-0.010864 +/- 0.0027907) [-0.49]

| eta:eta/1^D_2 |                    |  | kaon:kaon/1^D_2 |                    |  | pi:pi/1^D_2 |                    |  |
|---------------|--------------------|--|-----------------|--------------------|--|-------------|--------------------|--|
| k_re=         | 0.0964 +/- 0.0009  |  | k_re=           | 0.1031 +/- 0.0009  |  | k_re=       | -0.1235 +/- 0.0007 |  |
| k_im=         | -0.0040 +/- 0.0010 |  | k_im=           | -0.0037 +/- 0.0010 |  | k_im=       | 0.0031 +/- 0.0008  |  |
| corr=         | [-0.50]            |  | corr=           | [-0.50]            |  | corr=       | [-0.49]            |  |
| =====         |                    |  |                 |                    |  |             |                    |  |
| g =           | 0.0000 +/- nan     |  | g =             | 0.0669 +/- 0.0080  |  | g =         | 0.0154 +/- 0.0027  |  |
| arg(g)/pi=    | 0.0000 +/- nan     |  | arg(g)/pi=      | -0.0700 +/- 0.0107 |  | arg(g)/pi=  | 0.6491 +/- 0.2118  |  |
| -----         |                    |  |                 |                    |  |             |                    |  |
| g_re=         | 0.0000 +/- 0.0000  |  | g_re=           | 0.0653 +/- 0.0075  |  | g_re=       | -0.0069 +/- 0.0095 |  |
| g_im=         | 0.0000 +/- 0.0000  |  | g_im=           | -0.0146 +/- 0.0034 |  | g_im=       | 0.0137 +/- 0.0046  |  |

```

corr= [ 0.00] | corr= [-0.78] | corr= [ 0.80] |
*****

```

```

*****
JP=2+ || eta:eta/1^D_2[-] kaon:kaon/1^D_2[-] pi:pi/1^D_2[-]

```

```

sqrt(s)_pole = (0.26076 +/- 0.0017598)
+ (i/2)*(-0.027622 +/- 0.0027022) [ 0.00]

```

```

===== eta:eta/1^D_2 | kaon:kaon/1^D_2 | pi:pi/1^D_2 |
k_re= 0.0796 +/- 0.0014 | k_re= 0.0875 +/- 0.0013 | k_re= 0.1107 +/- 0.0010 |
k_im= -0.0113 +/- 0.0011 | k_im= -0.0103 +/- 0.0010 | k_im= -0.0081 +/- 0.0008 |
corr= [ 0.05] | corr= [ 0.03] | corr= [ 0.01] |
=====
|g|= 0.0000 +/- nan | |g|= 0.0342 +/- 0.0056 | |g|= 0.0859 +/- 0.0038 |
arg(g)/pi= 0.0000 +/- nan | arg(g)/pi= -0.1144 +/- 0.0138 | arg(g)/pi= 0.9186 +/- 0.0179 |
=====
g_re= 0.0000 +/- 0.0000 | g_re= 0.0320 +/- 0.0052 | g_re= -0.0832 +/- 0.0036 |
g_im= 0.0000 +/- 0.0000 | g_im= -0.0120 +/- 0.0025 | g_im= 0.0217 +/- 0.0050 |
corr= [ 0.00] | corr= [-0.78] | corr= [-0.13] |
=====

```

```

*****
JP=2+ || eta:eta/1^D_2[-] kaon:kaon/1^D_2[-] pi:pi/1^D_2[-]

```

```

sqrt(s)_pole = (0.28338 +/- 0.0015006)
+ (i/2)*(-0.0094925 +/- 0.0022691) [-0.44]

```

```

===== eta:eta/1^D_2 | kaon:kaon/1^D_2 | pi:pi/1^D_2 |
k_re= 0.0967 +/- 0.0011 | k_re= 0.1033 +/- 0.0010 | k_re= 0.1237 +/- 0.0009 |
k_im= -0.0035 +/- 0.0008 | k_im= -0.0033 +/- 0.0008 | k_im= -0.0027 +/- 0.0006 |
corr= [-0.43] | corr= [-0.43] | corr= [-0.43] |
=====
|g|= 0.0000 +/- nan | |g|= 0.0579 +/- 0.0071 | |g|= 0.0163 +/- 0.0027 |
arg(g)/pi= 0.0000 +/- nan | arg(g)/pi= -0.0641 +/- 0.0243 | arg(g)/pi= 0.1883 +/- 0.1727 |
=====
g_re= 0.0000 +/- 0.0000 | g_re= 0.0567 +/- 0.0066 | g_re= 0.0135 +/- 0.0049 |
g_im= 0.0000 +/- 0.0000 | g_im= -0.0116 +/- 0.0052 | g_im= 0.0091 +/- 0.0078 |
corr= [ 0.00] | corr= [-0.58] | corr= [-0.80] |
=====

```

# k\_2poles\_free\_geta\_cxxxxc\_noCM

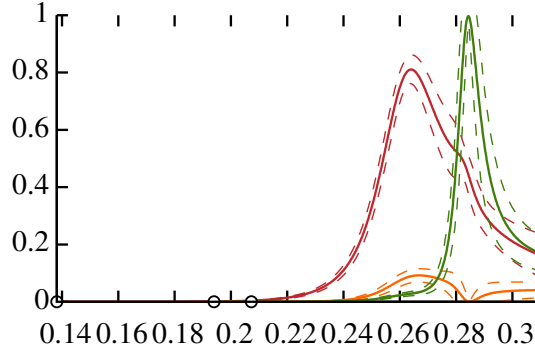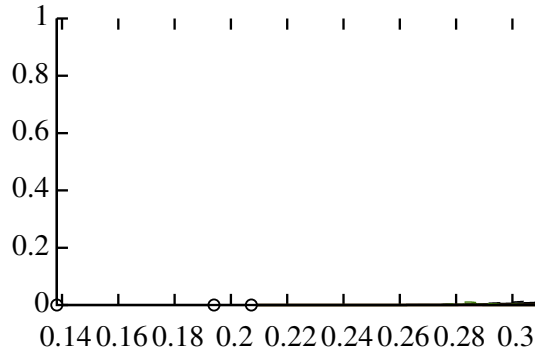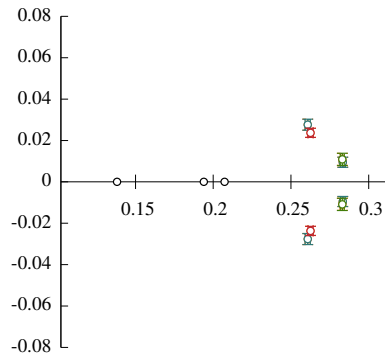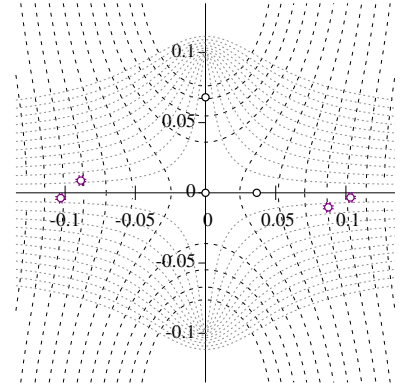

## parameter values

minimised with chisq/nDoF = 26.86 / (34 - 10) = 1.12

|                                                   |                         |      |       |       |       |      |       |       |       |       |
|---------------------------------------------------|-------------------------|------|-------|-------|-------|------|-------|-------|-------|-------|
| JP2+_g_eta:eta/1^D_2_pole0                        | -8.0439e-05 +/- 0.32518 | 1.00 | -0.81 | -0.01 | -0.00 | 0.00 | -0.00 | -0.00 | 0.00  | -0.01 |
| JP2+_g_eta:eta/1^D_2_pole1                        | -0.00016964 +/- 0.56527 | 1.00 | 0.01  | 0.00  | -0.00 | 0.00 | 0.02  | 0.00  | 0.00  | 0.01  |
| JP2+_g_kaon:kaon/1^D_2_pole0                      | -1.0630 +/- 0.16748     | 1.00 | 0.17  | -0.28 | 0.18  | 0.03 | 0.14  | 0.20  | 0.39  |       |
| JP2+_g_kaon:kaon/1^D_2_pole1                      | 1.4844 +/- 0.21205      | 1.00 | 0.41  | -0.64 | 0.12  | 0.09 | 0.36  | 0.42  |       |       |
| JP2+_g_pi:pi/1^D_2_pole0                          | 1.7897 +/- 0.091238     |      |       |       |       | 1.00 | -0.67 | 0.03  | -0.40 | 0.20  |
| JP2+_g_pi:pi/1^D_2_pole1                          | 0.034348 +/- 0.20759    |      |       |       |       |      | 1.00  | -0.10 | 0.30  | -0.31 |
| JP2+_gamma_eta:eta/1^D_2 eta:eta/1^D_2_order0     | 43.537 +/- 24.49        |      |       |       |       |      |       | 1.00  | 0.10  | -0.14 |
| JP2+_gamma_pi:pi/1^D_2 pi:pi/1^D_2_order0         | 30.643 +/- 21.262       |      |       |       |       |      |       |       | 1.00  | 0.19  |
| JP2+_m_pole0                                      | 0.26432 +/- 0.0015167   |      |       |       |       |      |       |       |       | 1.00  |
| JP2+_m_pole1                                      | 0.28430 +/- 0.0015391   |      |       |       |       |      |       |       |       |       |
| JP2+_gamma_eta:eta/1^D_2 kaon:kaon/1^D_2_order0   | 0.0000 +/- 0            |      |       |       |       |      |       |       |       |       |
| JP2+_gamma_eta:eta/1^D_2 pi:pi/1^D_2_order0       | 0.0000 +/- 0            |      |       |       |       |      |       |       |       |       |
| JP2+_gamma_kaon:kaon/1^D_2 kaon:kaon/1^D_2_order0 | 0.0000 +/- 0            |      |       |       |       |      |       |       |       |       |
| JP2+_gamma_kaon:kaon/1^D_2 pi:pi/1^D_2_order0     | 0.0000 +/- 0            |      |       |       |       |      |       |       |       |       |

## pole singularities

\*\*\*\*\*

\*\*\*\*\*

JP=2+ || eta:eta/1^D\_2[+] kaon:kaon/1^D\_2[+] pi:pi/1^D\_2[-]

sqrt(s)\_pole = (0.26261 +/- 0.0016399)  
+ (i/2)\*(-0.023688 +/- 0.0021897) [-0.17]

| eta:eta/1^D_2                 | kaon:kaon/1^D_2               | pi:pi/1^D_2                   |
|-------------------------------|-------------------------------|-------------------------------|
| k_re= -0.0810 +/- 0.0013      | k_re= -0.0888 +/- 0.0012      | k_re= 0.1117 +/- 0.0010       |
| k_im= 0.0096 +/- 0.0009       | k_im= 0.0088 +/- 0.0008       | k_im= -0.0070 +/- 0.0006      |
| corr= [-0.11]                 | corr= [-0.13]                 | corr= [-0.16]                 |
| g = 0.0004 +/- 0.0049         | g = 0.0304 +/- 0.0054         | g = 0.0902 +/- 0.0039         |
| arg(g)/pi= -0.1431 +/- 0.3748 | arg(g)/pi= -0.1277 +/- 0.0198 | arg(g)/pi= -0.0608 +/- 0.0148 |
| g_re= 0.0003 +/- 0.0044       | g_re= 0.0280 +/- 0.0054       | g_re= 0.0886 +/- 0.0039       |
| g_im= -0.0002 +/- 0.0022      | g_im= -0.0119 +/- 0.0020      | g_im= -0.0171 +/- 0.0042      |
| corr= [-0.98]                 | corr= [-0.55]                 | corr= [-0.03]                 |

\*\*\*\*\*

```

*****
JP=2+ || eta:eta/1^D_2[+] kaon:kaon/1^D_2[-] pi:pi/1^D_2[+]

sqrt(s)_pole = ( 0.283 +/- 0.0012761)
               + (i/2)*(-0.010864 +/- 0.0029397) [-0.45]

eta:eta/1^D_2 | kaon:kaon/1^D_2 | pi:pi/1^D_2 |
=====|=====|=====|
k_re= -0.0964 +/- 0.0009 | k_re= 0.1031 +/- 0.0009 | k_re= -0.1235 +/- 0.0007 |
k_im= 0.0040 +/- 0.0011 | k_im= -0.0037 +/- 0.0010 | k_im= 0.0031 +/- 0.0008 |
corr= [-0.46] | corr= [-0.46] | corr= [-0.46] |
=====|=====|=====|
|g|= 0.0010 +/- 0.0133 | |g|= 0.0669 +/- 0.0083 | |g|= 0.0154 +/- 0.0027 |
arg(g)/pi= -0.0792 +/- 0.2363 | arg(g)/pi= -0.0700 +/- 0.0105 | arg(g)/pi= -0.3506 +/- 0.2036 |
-----|-----|-----|
g_re= 0.0010 +/- 0.0129 | g_re= 0.0653 +/- 0.0079 | g_re= 0.0069 +/- 0.0092 |
g_im= -0.0002 +/- 0.0034 | g_im= -0.0146 +/- 0.0034 | g_im= -0.0137 +/- 0.0044 |
corr= [-0.97] | corr= [-0.80] | corr= [ 0.78] |
*****

*****
JP=2+ || eta:eta/1^D_2[+] kaon:kaon/1^D_2[-] pi:pi/1^D_2[-]

sqrt(s)_pole = (0.26077 +/- 0.0016805)
               + (i/2)*(-0.027627 +/- 0.0026613) [ 0.03]

eta:eta/1^D_2 | kaon:kaon/1^D_2 | pi:pi/1^D_2 |
=====|=====|=====|
k_re= -0.0796 +/- 0.0014 | k_re= 0.0875 +/- 0.0012 | k_re= 0.1107 +/- 0.0010 |
k_im= 0.0113 +/- 0.0011 | k_im= -0.0103 +/- 0.0010 | k_im= -0.0081 +/- 0.0008 |
corr= [ 0.07] | corr= [ 0.06] | corr= [ 0.04] |
=====|=====|=====|
|g|= 0.0004 +/- 0.0055 | |g|= 0.0342 +/- 0.0057 | |g|= 0.0860 +/- 0.0039 |
arg(g)/pi= -0.1340 +/- 0.1935 | arg(g)/pi= -0.1144 +/- 0.0141 | arg(g)/pi= -0.0814 +/- 0.0171 |
-----|-----|-----|
g_re= 0.0004 +/- 0.0050 | g_re= 0.0320 +/- 0.0053 | g_re= 0.0832 +/- 0.0036 |
g_im= -0.0002 +/- 0.0022 | g_im= -0.0120 +/- 0.0026 | g_im= -0.0217 +/- 0.0049 |
corr= [-0.99] | corr= [-0.78] | corr= [-0.17] |
*****

*****
JP=2+ || eta:eta/1^D_2[+] kaon:kaon/1^D_2[-] pi:pi/1^D_2[-]

sqrt(s)_pole = (0.28338 +/- 0.0015265)
               + (i/2)*(-0.0094915 +/- 0.0024232) [-0.41]

eta:eta/1^D_2 | kaon:kaon/1^D_2 | pi:pi/1^D_2 |
=====|=====|=====|
k_re= -0.0967 +/- 0.0011 | k_re= 0.1033 +/- 0.0011 | k_re= 0.1237 +/- 0.0009 |
k_im= 0.0035 +/- 0.0009 | k_im= -0.0033 +/- 0.0008 | k_im= -0.0027 +/- 0.0007 |
corr= [-0.40] | corr= [-0.40] | corr= [-0.41] |
=====|=====|=====|
|g|= 0.0009 +/- 0.0120 | |g|= 0.0579 +/- 0.0076 | |g|= 0.0163 +/- 0.0027 |
arg(g)/pi= -0.0719 +/- 0.2251 | arg(g)/pi= -0.0642 +/- 0.0243 | arg(g)/pi= 0.1886 +/- 0.1665 |
-----|-----|-----|
g_re= 0.0009 +/- 0.0117 | g_re= 0.0567 +/- 0.0070 | g_re= 0.0135 +/- 0.0047 |
g_im= -0.0002 +/- 0.0028 | g_im= -0.0116 +/- 0.0053 | g_im= 0.0091 +/- 0.0076 |
corr= [-0.97] | corr= [-0.63] | corr= [-0.78] |
*****

*****
JP=2+ || eta:eta/1^D_2[-] kaon:kaon/1^D_2[+] pi:pi/1^D_2[-]

sqrt(s)_pole = (0.26261 +/- 0.001639)
               + (i/2)*(-0.023689 +/- 0.0021885) [-0.18]

eta:eta/1^D_2 | kaon:kaon/1^D_2 | pi:pi/1^D_2 |
=====|=====|=====|
k_re= 0.0810 +/- 0.0013 | k_re= -0.0888 +/- 0.0012 | k_re= 0.1117 +/- 0.0010 |
k_im= -0.0096 +/- 0.0009 | k_im= 0.0088 +/- 0.0008 | k_im= -0.0070 +/- 0.0006 |
corr= [-0.11] | corr= [-0.13] | corr= [-0.16] |
=====|=====|=====|
|g|= 0.0004 +/- 0.0050 | |g|= 0.0304 +/- 0.0054 | |g|= 0.0902 +/- 0.0039 |
arg(g)/pi= -0.1326 +/- 0.3749 | arg(g)/pi= -0.1277 +/- 0.0198 | arg(g)/pi= -0.0608 +/- 0.0148 |
-----|-----|-----|
g_re= 0.0003 +/- 0.0045 | g_re= 0.0280 +/- 0.0054 | g_re= 0.0886 +/- 0.0039 |
g_im= -0.0002 +/- 0.0021 | g_im= -0.0119 +/- 0.0020 | g_im= -0.0171 +/- 0.0042 |
corr= [-0.97] | corr= [-0.55] | corr= [-0.03] |
*****

*****
JP=2+ || eta:eta/1^D_2[-] kaon:kaon/1^D_2[-] pi:pi/1^D_2[+]

sqrt(s)_pole = ( 0.283 +/- 0.0012757)
               + (i/2)*(-0.010871 +/- 0.0029244) [-0.46]

eta:eta/1^D_2 | kaon:kaon/1^D_2 | pi:pi/1^D_2 |
=====|=====|=====|
k_re= 0.0964 +/- 0.0009 | k_re= 0.1031 +/- 0.0009 | k_re= -0.1235 +/- 0.0007 |
k_im= -0.0040 +/- 0.0011 | k_im= -0.0037 +/- 0.0010 | k_im= 0.0031 +/- 0.0008 |
corr= [-0.46] | corr= [-0.46] | corr= [-0.46] |
=====|=====|=====|
|g|= 0.0010 +/- 0.0135 | |g|= 0.0669 +/- 0.0083 | |g|= 0.0154 +/- 0.0027 |
arg(g)/pi= -0.0536 +/- 0.2368 | arg(g)/pi= -0.0700 +/- 0.0105 | arg(g)/pi= -0.3506 +/- 0.2035 |
-----|-----|-----|
g_re= 0.0010 +/- 0.0133 | g_re= 0.0653 +/- 0.0079 | g_re= 0.0070 +/- 0.0092 |
g_im= -0.0002 +/- 0.0024 | g_im= -0.0146 +/- 0.0034 | g_im= -0.0137 +/- 0.0044 |

```

```

corr= [-0.95] | corr= [-0.80] | corr= [ 0.78] |
*****

```

```

*****
JP=2+ || eta:eta/1^D_2[-] kaon:kaon/1^D_2[-] pi:pi/1^D_2[-]

```

```

sqrt(s)_pole = (0.26077 +/- 0.0016797)
               + (i/2)*(-0.027628 +/- 0.0026602) [ 0.03]

```

```

===== eta:eta/1^D_2 | kaon:kaon/1^D_2 | pi:pi/1^D_2 |
=====
k_re= 0.0796 +/- 0.0014 | k_re= 0.0875 +/- 0.0012 | k_re= 0.1107 +/- 0.0010 |
k_im= -0.0113 +/- 0.0011 | k_im= -0.0103 +/- 0.0010 | k_im= -0.0081 +/- 0.0008 |
corr= [ 0.07] | corr= [ 0.06] | corr= [ 0.04] |
=====
|g|= 0.0004 +/- 0.0056 | |g|= 0.0342 +/- 0.0057 | |g|= 0.0860 +/- 0.0039 |
arg(g)/pi= -0.1250 +/- 0.1934 | arg(g)/pi= -0.1144 +/- 0.0141 | arg(g)/pi= -0.0814 +/- 0.0171 |
=====
g_re= 0.0004 +/- 0.0052 | g_re= 0.0320 +/- 0.0053 | g_re= 0.0832 +/- 0.0036 |
g_im= -0.0002 +/- 0.0021 | g_im= -0.0120 +/- 0.0026 | g_im= -0.0217 +/- 0.0049 |
corr= [-0.99] | corr= [-0.78] | corr= [-0.18] |
=====

```

```

*****
JP=2+ || eta:eta/1^D_2[-] kaon:kaon/1^D_2[-] pi:pi/1^D_2[-]

```

```

sqrt(s)_pole = (0.28338 +/- 0.001525)
               + (i/2)*(-0.0094974 +/- 0.0024127) [-0.42]

```

```

===== eta:eta/1^D_2 | kaon:kaon/1^D_2 | pi:pi/1^D_2 |
=====
k_re= 0.0966 +/- 0.0011 | k_re= 0.1033 +/- 0.0011 | k_re= 0.1237 +/- 0.0009 |
k_im= -0.0035 +/- 0.0009 | k_im= -0.0033 +/- 0.0008 | k_im= -0.0027 +/- 0.0007 |
corr= [-0.41] | corr= [-0.41] | corr= [-0.41] |
=====
|g|= 0.0009 +/- 0.0122 | |g|= 0.0579 +/- 0.0076 | |g|= 0.0163 +/- 0.0027 |
arg(g)/pi= -0.0458 +/- 0.2256 | arg(g)/pi= -0.0642 +/- 0.0242 | arg(g)/pi= 0.1885 +/- 0.1664 |
=====
g_re= 0.0009 +/- 0.0121 | g_re= 0.0567 +/- 0.0071 | g_re= 0.0135 +/- 0.0047 |
g_im= -0.0001 +/- 0.0019 | g_im= -0.0116 +/- 0.0053 | g_im= 0.0091 +/- 0.0076 |
corr= [-0.94] | corr= [-0.63] | corr= [-0.78] |
=====

```



# k\_2poles\_free\_geta\_xxcxxc\_noCM

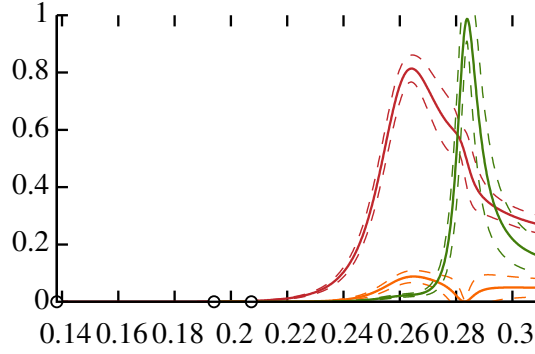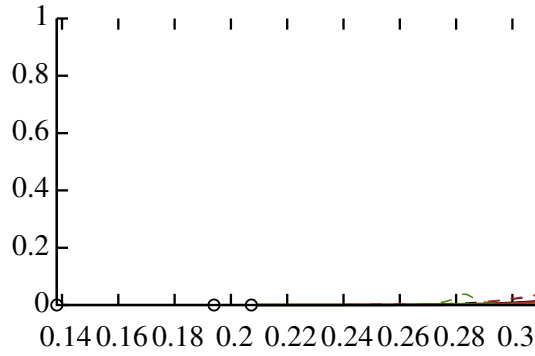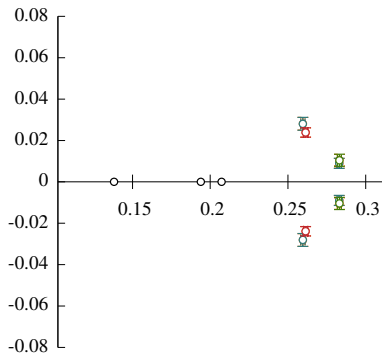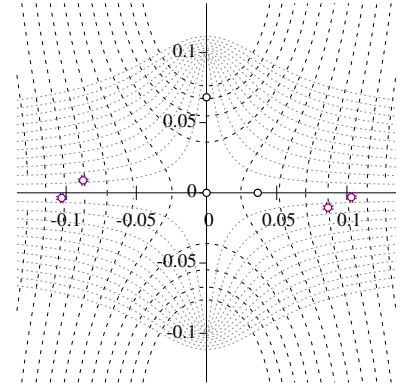

## parameter values

minimised with  $\chi^2/\text{nDoF} = 28.61 / (34 - 10) = 1.19$

|                                                   |                       |      |       |       |       |       |       |       |       |       |       |
|---------------------------------------------------|-----------------------|------|-------|-------|-------|-------|-------|-------|-------|-------|-------|
| JP2+_g_eta:eta/1^D_2_pole0                        | 0.055052 +/- 0.31601  | 1.00 | -0.61 | 0.04  | 0.05  | -0.06 | 0.09  | 0.30  | 0.25  | -0.01 | 0.07  |
| JP2+_g_eta:eta/1^D_2_pole1                        | 0.091007 +/- 0.53209  |      | 1.00  | -0.01 | -0.12 | 0.05  | -0.02 | -0.20 | 0.46  | 0.02  | -0.07 |
| JP2+_g_kaon:kaon/1^D_2_pole0                      | -1.0862 +/- 0.16277   |      |       | 1.00  | 0.10  | -0.26 | 0.07  | 0.08  | -0.01 | 0.05  | 0.33  |
| JP2+_g_kaon:kaon/1^D_2_pole1                      | 1.4871 +/- 0.24048    |      |       |       | 1.00  | 0.54  | -0.78 | 0.07  | -0.08 | 0.45  | 0.52  |
| JP2+_g_pi:pi/1^D_2_pole0                          | 1.8529 +/- 0.088852   |      |       |       |       | 1.00  | -0.65 | 0.04  | 0.02  | 0.48  | 0.03  |
| JP2+_g_pi:pi/1^D_2_pole1                          | -0.078821 +/- 0.27253 |      |       |       |       |       | 1.00  | 0.11  | 0.10  | -0.55 | -0.14 |
| JP2+_gamma_eta:eta/1^D_2 eta:eta/1^D_2_order0     | 54.164 +/- 40.678     |      |       |       |       |       |       | 1.00  | 0.42  | -0.11 | 0.02  |
| JP2+_gamma_eta:eta/1^D_2 pi:pi/1^D_2_order0       | 43.491 +/- 53.82      |      |       |       |       |       |       |       | 1.00  | 0.00  | -0.03 |
| JP2+_m_pole0                                      | 0.26411 +/- 0.0017274 |      |       |       |       |       |       |       |       | 1.00  | 0.33  |
| JP2+_m_pole1                                      | 0.28408 +/- 0.0014787 |      |       |       |       |       |       |       |       |       | 1.00  |
| JP2+_gamma_eta:eta/1^D_2 kaon:kaon/1^D_2_order0   | 0.0000 +/- 0          |      |       |       |       |       |       |       |       |       | FIXED |
| JP2+_gamma_kaon:kaon/1^D_2 kaon:kaon/1^D_2_order0 | 0.0000 +/- 0          |      |       |       |       |       |       |       |       |       | FIXED |
| JP2+_gamma_kaon:kaon/1^D_2 pi:pi/1^D_2_order0     | 0.0000 +/- 0          |      |       |       |       |       |       |       |       |       | FIXED |
| JP2+_gamma_pi:pi/1^D_2 pi:pi/1^D_2_order0         | 0.0000 +/- 0          |      |       |       |       |       |       |       |       |       | FIXED |

## pole singularities

\*\*\*\*\*

\*\*\*\*\*

JP=2+ || eta:eta/1^D\_2[+] kaon:kaon/1^D\_2[+] pi:pi/1^D\_2[-]

sqrt(s)\_pole = (0.26137 +/- 0.0013695)  
+ (i/2)\*(-0.023844 +/- 0.0022702) [-0.31]

| eta:eta/1^D_2                | kaon:kaon/1^D_2               | pi:pi/1^D_2                   |
|------------------------------|-------------------------------|-------------------------------|
| k_re= -0.0800 +/- 0.0011     | k_re= -0.0878 +/- 0.0010      | k_re= 0.1110 +/- 0.0008       |
| k_im= 0.0097 +/- 0.0009      | k_im= 0.0089 +/- 0.0008       | k_im= -0.0070 +/- 0.0007      |
| corr= [-0.28]                | corr= [-0.29]                 | corr= [-0.31]                 |
| g = 0.0048 +/- 0.0074        | g = 0.0309 +/- 0.0053         | g = 0.0888 +/- 0.0039         |
| arg(g)/pi= 0.1971 +/- 0.4256 | arg(g)/pi= -0.1147 +/- 0.0194 | arg(g)/pi= -0.0804 +/- 0.0068 |
| g_re= 0.0039 +/- 0.0087      | g_re= 0.0289 +/- 0.0053       | g_re= 0.0860 +/- 0.0034       |
| g_im= 0.0028 +/- 0.0045      | g_im= -0.0109 +/- 0.0019      | g_im= -0.0222 +/- 0.0027      |
| corr= [-0.07]                | corr= [-0.47]                 | corr= [-0.89]                 |

\*\*\*\*\*

```

*****
JP=2+ || eta:eta/1^D_2[+] kaon:kaon/1^D_2[-] pi:pi/1^D_2[+]

sqrt(s)_pole = (0.28308 +/- 0.001253)
               + (i/2)*(-0.01043 +/- 0.0029434) [-0.58]

=====
eta:eta/1^D_2 | kaon:kaon/1^D_2 | pi:pi/1^D_2 |
=====
k_re= -0.0964 +/- 0.0009 | k_re= 0.1031 +/- 0.0009 | k_re= -0.1236 +/- 0.0007 |
k_im= 0.0038 +/- 0.0011 | k_im= -0.0036 +/- 0.0010 | k_im= 0.0030 +/- 0.0008 |
corr= [-0.58] | corr= [-0.58] | corr= [-0.58] |
=====
|g|= 0.0042 +/- 0.0191 | |g|= 0.0656 +/- 0.0089 | |g|= 0.0152 +/- 0.0050 |
arg(g)/pi= 0.0257 +/- 0.4375 | arg(g)/pi= -0.0630 +/- 0.0121 | arg(g)/pi= -0.2262 +/- 0.2289 |
=====
g_re= 0.0041 +/- 0.0195 | g_re= 0.0643 +/- 0.0086 | g_re= 0.0116 +/- 0.0105 |
g_im= 0.0003 +/- 0.0043 | g_im= -0.0129 +/- 0.0034 | g_im= -0.0099 +/- 0.0059 |
corr= [-0.91] | corr= [-0.68] | corr= [ 0.86] |
=====
*****

*****
JP=2+ || eta:eta/1^D_2[+] kaon:kaon/1^D_2[-] pi:pi/1^D_2[-]

sqrt(s)_pole = (0.25959 +/- 0.0013672)
               + (i/2)*(-0.028063 +/- 0.0030961) [-0.17]

=====
eta:eta/1^D_2 | kaon:kaon/1^D_2 | pi:pi/1^D_2 |
=====
k_re= -0.0787 +/- 0.0011 | k_re= 0.0866 +/- 0.0010 | k_re= 0.1100 +/- 0.0008 |
k_im= 0.0116 +/- 0.0012 | k_im= -0.0105 +/- 0.0011 | k_im= -0.0083 +/- 0.0009 |
corr= [-0.19] | corr= [-0.19] | corr= [-0.18] |
=====
|g|= 0.0042 +/- 0.0072 | |g|= 0.0344 +/- 0.0060 | |g|= 0.0852 +/- 0.0042 |
arg(g)/pi= 0.1606 +/- 0.4911 | arg(g)/pi= -0.1096 +/- 0.0148 | arg(g)/pi= -0.1016 +/- 0.0113 |
=====
g_re= 0.0037 +/- 0.0088 | g_re= 0.0324 +/- 0.0056 | g_re= 0.0809 +/- 0.0032 |
g_im= 0.0020 +/- 0.0040 | g_im= -0.0116 +/- 0.0026 | g_im= -0.0267 +/- 0.0041 |
corr= [-0.39] | corr= [-0.76] | corr= [-0.89] |
=====
*****

*****
JP=2+ || eta:eta/1^D_2[+] kaon:kaon/1^D_2[-] pi:pi/1^D_2[-]

sqrt(s)_pole = (0.28299 +/- 0.001433)
               + (i/2)*(-0.0089649 +/- 0.0024558) [-0.29]

=====
eta:eta/1^D_2 | kaon:kaon/1^D_2 | pi:pi/1^D_2 |
=====
k_re= -0.0964 +/- 0.0011 | k_re= 0.1031 +/- 0.0010 | k_re= 0.1235 +/- 0.0008 |
k_im= 0.0033 +/- 0.0009 | k_im= -0.0031 +/- 0.0008 | k_im= -0.0026 +/- 0.0007 |
corr= [-0.28] | corr= [-0.28] | corr= [-0.29] |
=====
|g|= 0.0028 +/- 0.0159 | |g|= 0.0566 +/- 0.0074 | |g|= 0.0155 +/- 0.0049 |
arg(g)/pi= 0.0701 +/- 0.8613 | arg(g)/pi= -0.0710 +/- 0.0296 | arg(g)/pi= 0.2581 +/- 0.1948 |
=====
g_re= 0.0027 +/- 0.0171 | g_re= 0.0551 +/- 0.0067 | g_re= 0.0107 +/- 0.0046 |
g_im= 0.0006 +/- 0.0042 | g_im= -0.0125 +/- 0.0061 | g_im= 0.0113 +/- 0.0096 |
corr= [-0.87] | corr= [-0.56] | corr= [-0.78] |
=====
*****

*****
JP=2+ || eta:eta/1^D_2[-] kaon:kaon/1^D_2[+] pi:pi/1^D_2[-]

sqrt(s)_pole = (0.26142 +/- 0.0013796)
               + (i/2)*(-0.02388 +/- 0.0022549) [-0.31]

=====
eta:eta/1^D_2 | kaon:kaon/1^D_2 | pi:pi/1^D_2 |
=====
k_re= 0.0800 +/- 0.0011 | k_re= -0.0879 +/- 0.0010 | k_re= 0.1110 +/- 0.0008 |
k_im= -0.0098 +/- 0.0009 | k_im= 0.0089 +/- 0.0008 | k_im= -0.0070 +/- 0.0007 |
corr= [-0.28] | corr= [-0.29] | corr= [-0.31] |
=====
|g|= 0.0050 +/- 0.0077 | |g|= 0.0310 +/- 0.0053 | |g|= 0.0889 +/- 0.0039 |
arg(g)/pi= 0.2100 +/- 0.4272 | arg(g)/pi= -0.1153 +/- 0.0195 | arg(g)/pi= -0.0794 +/- 0.0066 |
=====
g_re= 0.0039 +/- 0.0090 | g_re= 0.0290 +/- 0.0053 | g_re= 0.0862 +/- 0.0034 |
g_im= 0.0030 +/- 0.0047 | g_im= -0.0110 +/- 0.0020 | g_im= -0.0220 +/- 0.0026 |
corr= [-0.00] | corr= [-0.47] | corr= [-0.88] |
=====
*****

*****
JP=2+ || eta:eta/1^D_2[-] kaon:kaon/1^D_2[-] pi:pi/1^D_2[+]

sqrt(s)_pole = (0.28308 +/- 0.0012502)
               + (i/2)*(-0.010518 +/- 0.0027984) [-0.61]

=====
eta:eta/1^D_2 | kaon:kaon/1^D_2 | pi:pi/1^D_2 |
=====
k_re= 0.0964 +/- 0.0009 | k_re= 0.1031 +/- 0.0009 | k_re= -0.1236 +/- 0.0007 |
k_im= -0.0039 +/- 0.0010 | k_im= -0.0036 +/- 0.0010 | k_im= 0.0030 +/- 0.0008 |
corr= [-0.61] | corr= [-0.61] | corr= [-0.61] |
=====
|g|= 0.0042 +/- 0.0196 | |g|= 0.0657 +/- 0.0088 | |g|= 0.0155 +/- 0.0051 |
arg(g)/pi= 0.0575 +/- 0.4444 | arg(g)/pi= -0.0628 +/- 0.0117 | arg(g)/pi= -0.2275 +/- 0.2237 |
=====
g_re= 0.0042 +/- 0.0203 | g_re= 0.0644 +/- 0.0086 | g_re= 0.0117 +/- 0.0106 |
g_im= 0.0008 +/- 0.0028 | g_im= -0.0129 +/- 0.0033 | g_im= -0.0102 +/- 0.0057 |
=====

```

```

corr= [-0.73] | corr= [-0.67] | corr= [ 0.86] |
*****

```

```

*****
JP=2+ || eta:eta/1^D_2[-] kaon:kaon/1^D_2[-] pi:pi/1^D_2[-]

```

```

sqrt(s)_pole = (0.25963 +/- 0.0013701)
               + (i/2)*(-0.02811 +/- 0.0030716) [-0.17]

```

```

===== eta:eta/1^D_2 | kaon:kaon/1^D_2 | pi:pi/1^D_2 |
k_re= 0.0787 +/- 0.0011 | k_re= 0.0866 +/- 0.0010 | k_re= 0.1100 +/- 0.0008 |
k_im= -0.0116 +/- 0.0012 | k_im= -0.0105 +/- 0.0011 | k_im= -0.0083 +/- 0.0009 |
corr= [-0.19] | corr= [-0.19] | corr= [-0.18] |
=====
|g|= 0.0043 +/- 0.0075 | |g|= 0.0345 +/- 0.0060 | |g|= 0.0853 +/- 0.0042 |
arg(g)/pi= 0.1717 +/- 0.4932 | arg(g)/pi= -0.1102 +/- 0.0150 | arg(g)/pi= -0.1008 +/- 0.0111 |
=====
g_re= 0.0037 +/- 0.0092 | g_re= 0.0324 +/- 0.0056 | g_re= 0.0810 +/- 0.0032 |
g_im= 0.0022 +/- 0.0041 | g_im= -0.0117 +/- 0.0027 | g_im= -0.0266 +/- 0.0040 |
corr= [-0.33] | corr= [-0.76] | corr= [-0.89] |
=====

```

```

*****
JP=2+ || eta:eta/1^D_2[-] kaon:kaon/1^D_2[-] pi:pi/1^D_2[-]

```

```

sqrt(s)_pole = ( 0.283 +/- 0.0014309)
               + (i/2)*(-0.0090021 +/- 0.0023422) [-0.28]

```

```

===== eta:eta/1^D_2 | kaon:kaon/1^D_2 | pi:pi/1^D_2 |
k_re= 0.0964 +/- 0.0011 | k_re= 0.1031 +/- 0.0010 | k_re= 0.1235 +/- 0.0008 |
k_im= -0.0033 +/- 0.0009 | k_im= -0.0031 +/- 0.0008 | k_im= -0.0026 +/- 0.0007 |
corr= [-0.28] | corr= [-0.28] | corr= [-0.28] |
=====
|g|= 0.0028 +/- 0.0161 | |g|= 0.0565 +/- 0.0075 | |g|= 0.0157 +/- 0.0049 |
arg(g)/pi= 0.1033 +/- 0.8639 | arg(g)/pi= -0.0707 +/- 0.0295 | arg(g)/pi= 0.2583 +/- 0.1904 |
=====
g_re= 0.0027 +/- 0.0176 | g_re= 0.0551 +/- 0.0068 | g_re= 0.0108 +/- 0.0045 |
g_im= 0.0009 +/- 0.0028 | g_im= -0.0124 +/- 0.0061 | g_im= 0.0114 +/- 0.0096 |
corr= [-0.67] | corr= [-0.57] | corr= [-0.80] |
=====

```

# k\_2poles\_free\_geta\_xxxxxxc

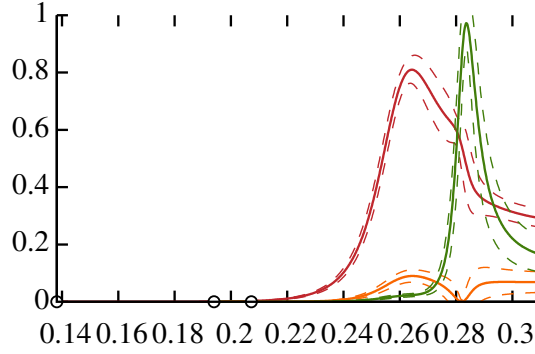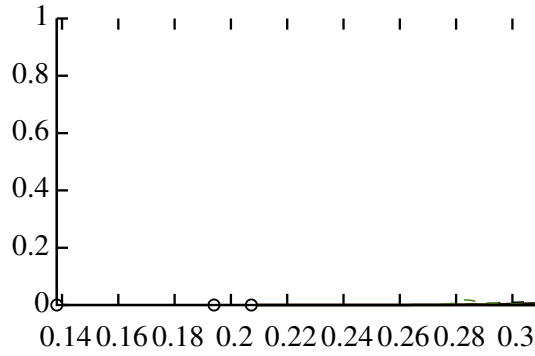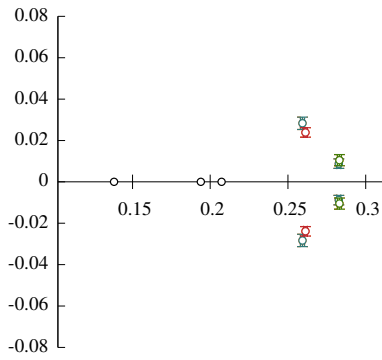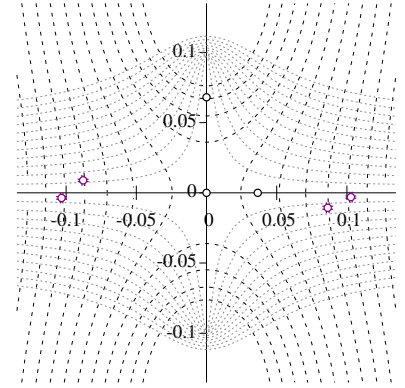

## parameter values

minimised with  $\text{chisq}/\text{nDoF} = 29.45 / (34 - 9) = 1.18$

|                                               |                         |      |       |       |       |      |       |       |       |       |
|-----------------------------------------------|-------------------------|------|-------|-------|-------|------|-------|-------|-------|-------|
| JP2+_g_eta:eta/1^D_2_pole0                    | 0.00012294 +/- 0.40295  | 1.00 | -0.88 | -0.01 | -0.00 | 0.00 | 0.00  | -0.02 | -0.00 | -0.01 |
| JP2+_g_eta:eta/1^D_2_pole1                    | -0.00017773 +/- 0.68049 | 1.00 | 0.01  | -0.00 | -0.00 | 0.00 | 0.00  | 0.04  | 0.00  | 0.01  |
| JP2+_g_kaon:kaon/1^D_2_pole0                  | -1.0742 +/- 0.15602     | 1.00 | 0.17  | -0.20 | -0.07 | 0.01 | 0.20  | 0.37  |       |       |
| JP2+_g_kaon:kaon/1^D_2_pole1                  | 1.4587 +/- 0.23523      | 1.00 | 0.54  | -0.83 | 0.18  | 0.48 | 0.51  |       |       |       |
| JP2+_g_pi:pi/1^D_2_pole0                      | 1.8095 +/- 0.079243     |      |       |       |       | 1.00 | -0.63 | 0.12  | 0.41  | 0.02  |
| JP2+_g_pi:pi/1^D_2_pole1                      | -0.11807 +/- 0.27679    |      |       |       |       | 1.00 | -0.21 | -0.55 | -0.19 |       |
| JP2+_gamma_eta:eta/1^D_2 eta:eta/1^D_2_order0 | 40.034 +/- 24.537       |      |       |       |       |      |       | 1.00  | -0.08 | -0.08 |
| JP2+_m_pole0                                  | 0.26415 +/- 0.0015455   |      |       |       |       |      |       |       | 1.00  | 0.39  |
| JP2+_m_pole1                                  | 0.28351 +/- 0.0013633   |      |       |       |       |      |       |       |       | 1.00  |
| JP2+_gamma_eta:eta/1^D_2 kaon:kaon/1^D_2_orde | 0.0000 +/- 0            |      |       |       |       |      |       |       |       |       |
| JP2+_gamma_eta:eta/1^D_2 pi:pi/1^D_2_order0   | 0.0000 +/- 0            |      |       |       |       |      |       |       |       |       |
| JP2+_gamma_kaon:kaon/1^D_2 kaon:kaon/1^D_2_or | 0.0000 +/- 0            |      |       |       |       |      |       |       |       |       |
| JP2+_gamma_kaon:kaon/1^D_2 pi:pi/1^D_2_order0 | 0.0000 +/- 0            |      |       |       |       |      |       |       |       |       |
| JP2+_gamma_pi:pi/1^D_2 pi:pi/1^D_2_order0     | 0.0000 +/- 0            |      |       |       |       |      |       |       |       |       |

## pole singularities

\*\*\*\*\*

\*\*\*\*\*

JP=2+ || eta:eta/1^D\_2[+] kaon:kaon/1^D\_2[+] pi:pi/1^D\_2[-]

sqrt(s)\_pole = (0.26125 +/- 0.001227)  
+ (i/2)\*(-0.023881 +/- 0.0022824) [-0.26]

| eta:eta/1^D_2                 | kaon:kaon/1^D_2               | pi:pi/1^D_2                   |
|-------------------------------|-------------------------------|-------------------------------|
| k_re= -0.0799 +/- 0.0010      | k_re= -0.0878 +/- 0.0009      | k_re= 0.1109 +/- 0.0007       |
| k_im= 0.0098 +/- 0.0009       | k_im= 0.0089 +/- 0.0008       | k_im= -0.0070 +/- 0.0007      |
| corr= [-0.24]                 | corr= [-0.25]                 | corr= [-0.25]                 |
| g = 0.0005 +/- 0.0063         | g = 0.0319 +/- 0.0049         | g = 0.0888 +/- 0.0038         |
| arg(g)/pi= -0.1315 +/- 0.0889 | arg(g)/pi= -0.1136 +/- 0.0182 | arg(g)/pi= -0.0834 +/- 0.0069 |
| g_re= 0.0004 +/- 0.0058       | g_re= 0.0299 +/- 0.0048       | g_re= 0.0858 +/- 0.0033       |
| g_im= -0.0002 +/- 0.0025      | g_im= -0.0111 +/- 0.0020      | g_im= -0.0230 +/- 0.0028      |
| corr= [-1.00]                 | corr= [-0.49]                 | corr= [-0.91]                 |

\*\*\*\*\*

```

*****
JP=2+ || eta:eta/1^D_2[+] kaon:kaon/1^D_2[-] pi:pi/1^D_2[+]

sqrt(s)_pole = (0.28312 +/- 0.0012973)
               + (i/2)*(-0.010469 +/- 0.0026955) [-0.65]

=====
eta:eta/1^D_2 | kaon:kaon/1^D_2 | pi:pi/1^D_2 |
=====
k_re= -0.0965 +/- 0.0010 | k_re= 0.1032 +/- 0.0009 | k_re= -0.1236 +/- 0.0007 |
k_im= 0.0038 +/- 0.0010 | k_im= -0.0036 +/- 0.0009 | k_im= 0.0030 +/- 0.0008 |
corr= [-0.65] | corr= [-0.65] | corr= [-0.65] |
=====
|g|= 0.0013 +/- 0.0164 | |g|= 0.0661 +/- 0.0092 | |g|= 0.0174 +/- 0.0072 |
arg(g)/pi= -0.0720 +/- 0.1026 | arg(g)/pi= -0.0611 +/- 0.0131 | arg(g)/pi= -0.1647 +/- 0.1949 |
=====
g_re= 0.0012 +/- 0.0160 | g_re= 0.0649 +/- 0.0090 | g_re= 0.0151 +/- 0.0112 |
g_im= -0.0003 +/- 0.0037 | g_im= -0.0126 +/- 0.0033 | g_im= -0.0086 +/- 0.0063 |
corr= [-0.99] | corr= [-0.56] | corr= [ 0.87] |
=====
*****

*****
JP=2+ || eta:eta/1^D_2[+] kaon:kaon/1^D_2[-] pi:pi/1^D_2[-]

sqrt(s)_pole = (0.25935 +/- 0.0012983)
               + (i/2)*(-0.028305 +/- 0.0030035) [-0.06]

=====
eta:eta/1^D_2 | kaon:kaon/1^D_2 | pi:pi/1^D_2 |
=====
k_re= -0.0785 +/- 0.0011 | k_re= 0.0864 +/- 0.0010 | k_re= 0.1098 +/- 0.0008 |
k_im= 0.0117 +/- 0.0012 | k_im= -0.0106 +/- 0.0011 | k_im= -0.0084 +/- 0.0009 |
corr= [-0.09] | corr= [-0.08] | corr= [-0.07] |
=====
|g|= 0.0005 +/- 0.0071 | |g|= 0.0352 +/- 0.0054 | |g|= 0.0849 +/- 0.0042 |
arg(g)/pi= -0.1306 +/- 0.2504 | arg(g)/pi= -0.1137 +/- 0.0147 | arg(g)/pi= -0.1067 +/- 0.0116 |
=====
g_re= 0.0005 +/- 0.0065 | g_re= 0.0329 +/- 0.0050 | g_re= 0.0802 +/- 0.0031 |
g_im= -0.0002 +/- 0.0029 | g_im= -0.0123 +/- 0.0027 | g_im= -0.0279 +/- 0.0042 |
corr= [-0.99] | corr= [-0.76] | corr= [-0.87] |
=====
*****

*****
JP=2+ || eta:eta/1^D_2[+] kaon:kaon/1^D_2[-] pi:pi/1^D_2[-]

sqrt(s)_pole = ( 0.2827 +/- 0.0012747)
               + (i/2)*(-0.0088061 +/- 0.0022981) [-0.08]

=====
eta:eta/1^D_2 | kaon:kaon/1^D_2 | pi:pi/1^D_2 |
=====
k_re= -0.0961 +/- 0.0009 | k_re= 0.1029 +/- 0.0009 | k_re= 0.1233 +/- 0.0007 |
k_im= 0.0032 +/- 0.0008 | k_im= -0.0030 +/- 0.0008 | k_im= -0.0025 +/- 0.0007 |
corr= [-0.08] | corr= [-0.08] | corr= [-0.08] |
=====
|g|= 0.0011 +/- 0.0144 | |g|= 0.0555 +/- 0.0066 | |g|= 0.0171 +/- 0.0067 |
arg(g)/pi= -0.0815 +/- 0.2986 | arg(g)/pi= -0.0794 +/- 0.0333 | arg(g)/pi= 0.3056 +/- 0.1627 |
=====
g_re= 0.0011 +/- 0.0139 | g_re= 0.0537 +/- 0.0057 | g_re= 0.0098 +/- 0.0042 |
g_im= -0.0003 +/- 0.0038 | g_im= -0.0137 +/- 0.0067 | g_im= 0.0140 +/- 0.0102 |
corr= [-0.96] | corr= [-0.58] | corr= [-0.77] |
=====
*****

*****
JP=2+ || eta:eta/1^D_2[-] kaon:kaon/1^D_2[+] pi:pi/1^D_2[-]

sqrt(s)_pole = (0.26125 +/- 0.0012273)
               + (i/2)*(-0.023883 +/- 0.0022823) [-0.26]

=====
eta:eta/1^D_2 | kaon:kaon/1^D_2 | pi:pi/1^D_2 |
=====
k_re= 0.0799 +/- 0.0010 | k_re= -0.0878 +/- 0.0009 | k_re= 0.1109 +/- 0.0007 |
k_im= -0.0098 +/- 0.0009 | k_im= 0.0089 +/- 0.0008 | k_im= -0.0070 +/- 0.0007 |
corr= [-0.24] | corr= [-0.25] | corr= [-0.25] |
=====
|g|= 0.0005 +/- 0.0064 | |g|= 0.0319 +/- 0.0049 | |g|= 0.0888 +/- 0.0038 |
arg(g)/pi= -0.1226 +/- 0.0892 | arg(g)/pi= -0.1136 +/- 0.0182 | arg(g)/pi= -0.0834 +/- 0.0069 |
=====
g_re= 0.0004 +/- 0.0060 | g_re= 0.0299 +/- 0.0048 | g_re= 0.0858 +/- 0.0033 |
g_im= -0.0002 +/- 0.0024 | g_im= -0.0111 +/- 0.0020 | g_im= -0.0230 +/- 0.0028 |
corr= [-1.00] | corr= [-0.49] | corr= [-0.91] |
=====
*****

*****
JP=2+ || eta:eta/1^D_2[-] kaon:kaon/1^D_2[-] pi:pi/1^D_2[+]

sqrt(s)_pole = (0.28312 +/- 0.0012964)
               + (i/2)*(-0.01048 +/- 0.0027023) [-0.65]

=====
eta:eta/1^D_2 | kaon:kaon/1^D_2 | pi:pi/1^D_2 |
=====
k_re= 0.0965 +/- 0.0010 | k_re= 0.1032 +/- 0.0009 | k_re= -0.1236 +/- 0.0007 |
k_im= -0.0038 +/- 0.0010 | k_im= -0.0036 +/- 0.0009 | k_im= 0.0030 +/- 0.0008 |
corr= [-0.65] | corr= [-0.65] | corr= [-0.65] |
=====
|g|= 0.0013 +/- 0.0167 | |g|= 0.0661 +/- 0.0092 | |g|= 0.0174 +/- 0.0072 |
arg(g)/pi= -0.0486 +/- 0.1037 | arg(g)/pi= -0.0612 +/- 0.0133 | arg(g)/pi= -0.1648 +/- 0.1951 |
=====
g_re= 0.0013 +/- 0.0165 | g_re= 0.0649 +/- 0.0090 | g_re= 0.0152 +/- 0.0112 |
g_im= -0.0002 +/- 0.0026 | g_im= -0.0126 +/- 0.0034 | g_im= -0.0086 +/- 0.0063 |
=====

```

```

corr= [-0.99] | corr= [-0.55] | corr= [ 0.87] |
*****

```

```

*****
JP=2+ || eta:eta/1^D_2[-] kaon:kaon/1^D_2[-] pi:pi/1^D_2[-]

```

```

sqrt(s)_pole = (0.25935 +/- 0.0012985)
               + (i/2)*(-0.028307 +/- 0.003003) [-0.06]

```

```

===== eta:eta/1^D_2 | kaon:kaon/1^D_2 | pi:pi/1^D_2 |
k_re= 0.0785 +/- 0.0011 | k_re= 0.0864 +/- 0.0010 | k_re= 0.1098 +/- 0.0008 |
k_im= -0.0117 +/- 0.0012 | k_im= -0.0106 +/- 0.0011 | k_im= -0.0084 +/- 0.0009 |
corr= [-0.09] | corr= [-0.08] | corr= [-0.07] |
=====
|g|= 0.0005 +/- 0.0072 | |g|= 0.0352 +/- 0.0054 | |g|= 0.0849 +/- 0.0042 |
arg(g)/pi= -0.1230 +/- 0.2504 | arg(g)/pi= -0.1137 +/- 0.0147 | arg(g)/pi= -0.1067 +/- 0.0116 |
=====
g_re= 0.0005 +/- 0.0067 | g_re= 0.0329 +/- 0.0050 | g_re= 0.0802 +/- 0.0031 |
g_im= -0.0002 +/- 0.0028 | g_im= -0.0123 +/- 0.0027 | g_im= -0.0279 +/- 0.0042 |
corr= [-0.99] | corr= [-0.76] | corr= [-0.87] |
=====

```

```

*****
JP=2+ || eta:eta/1^D_2[-] kaon:kaon/1^D_2[-] pi:pi/1^D_2[-]

```

```

sqrt(s)_pole = ( 0.2827 +/- 0.0012712)
               + (i/2)*(-0.0088144 +/- 0.0023) [-0.08]

```

```

===== eta:eta/1^D_2 | kaon:kaon/1^D_2 | pi:pi/1^D_2 |
k_re= 0.0961 +/- 0.0009 | k_re= 0.1029 +/- 0.0009 | k_re= 0.1233 +/- 0.0007 |
k_im= -0.0032 +/- 0.0008 | k_im= -0.0030 +/- 0.0008 | k_im= -0.0025 +/- 0.0007 |
corr= [-0.08] | corr= [-0.08] | corr= [-0.08] |
=====
|g|= 0.0011 +/- 0.0146 | |g|= 0.0555 +/- 0.0066 | |g|= 0.0171 +/- 0.0067 |
arg(g)/pi= -0.0585 +/- 0.2994 | arg(g)/pi= -0.0795 +/- 0.0333 | arg(g)/pi= 0.3055 +/- 0.1629 |
=====
g_re= 0.0011 +/- 0.0143 | g_re= 0.0537 +/- 0.0057 | g_re= 0.0098 +/- 0.0042 |
g_im= -0.0002 +/- 0.0029 | g_im= -0.0137 +/- 0.0067 | g_im= 0.0140 +/- 0.0102 |
corr= [-0.93] | corr= [-0.58] | corr= [-0.76] |
=====

```

# k\_2poles\_ssxxxs\_noCM

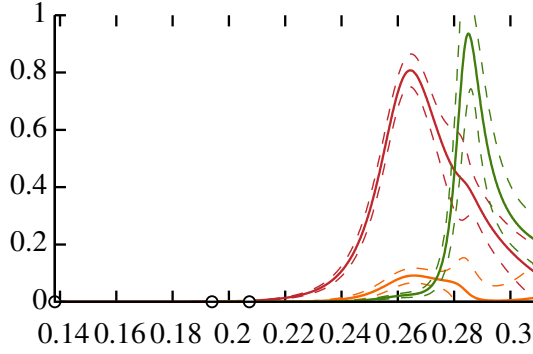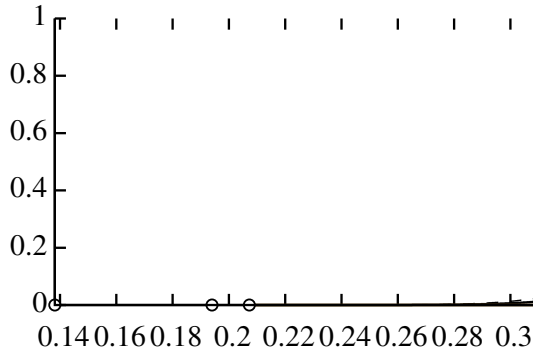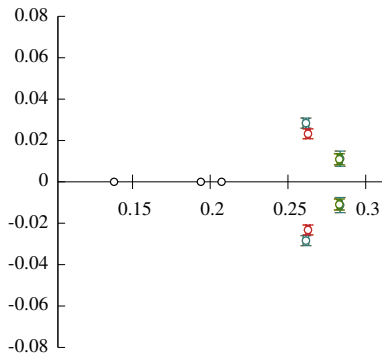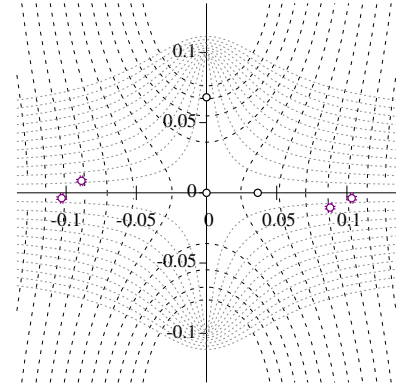

## parameter values

minimised with  $\chi^2/\text{nDoF} = 26.76 / (34 - 9) = 1.07$

|                                                   |                       |      |       |       |       |       |       |       |       |       |
|---------------------------------------------------|-----------------------|------|-------|-------|-------|-------|-------|-------|-------|-------|
| JP2+_g_kaon:kaon/1^D_2_pole0                      | -1.0500 +/- 0.17567   | 1.00 | 0.19  | -0.22 | 0.29  | 0.05  | -0.12 | -0.03 | 0.33  | 0.40  |
| JP2+_g_kaon:kaon/1^D_2_pole1                      | 1.5299 +/- 0.21221    | 1.00 | 0.10  | 0.22  | 0.13  | -0.49 | 0.11  | 0.26  | 0.51  |       |
| JP2+_g_pi:pi/1^D_2_pole0                          | 1.7596 +/- 0.084889   | 1.00 | -0.64 | 0.04  | 0.47  | -0.02 | -0.07 | -0.42 |       |       |
| JP2+_g_pi:pi/1^D_2_pole1                          | 0.23679 +/- 0.39265   | 1.00 | -0.02 | -0.86 | -0.03 | 0.14  | 0.65  |       |       |       |
| JP2+_gamma_eta:eta/1^D_2 eta:eta/1^D_2_order1     | 552.36 +/- 302.65     |      |       |       | 1.00  | -0.03 | 0.15  | -0.09 | -0.05 |       |
| JP2+_gamma_kaon:kaon/1^D_2 pi:pi/1^D_2_order1     | -887.24 +/- 1478.6    |      |       |       | 1.00  | 0.08  | -0.16 | -0.56 |       |       |
| JP2+_gamma_pi:pi/1^D_2 pi:pi/1^D_2_order1         | 612.42 +/- 307.08     |      |       |       |       | 1.00  | 0.22  | -0.06 |       |       |
| JP2+_m_pole0                                      | 0.26448 +/- 0.0009868 |      |       |       |       |       | 1.00  | 0.30  |       |       |
| JP2+_m_pole1                                      | 0.28491 +/- 0.0019192 |      |       |       |       |       |       | 1.00  |       |       |
| JP2+_g_eta:eta/1^D_2_pole0                        | 0.0000 +/- 0          |      |       |       |       |       |       |       |       | FIXED |
| JP2+_g_eta:eta/1^D_2_pole1                        | 0.0000 +/- 0          |      |       |       |       |       |       |       |       | FIXED |
| JP2+_gamma_eta:eta/1^D_2 eta:eta/1^D_2_order0     | 0.0000 +/- 0          |      |       |       |       |       |       |       |       | FIXED |
| JP2+_gamma_eta:eta/1^D_2 kaon:kaon/1^D_2_order0   | 0.0000 +/- 0          |      |       |       |       |       |       |       |       | FIXED |
| JP2+_gamma_eta:eta/1^D_2 kaon:kaon/1^D_2_order1   | 0.0000 +/- 0          |      |       |       |       |       |       |       |       | FIXED |
| JP2+_gamma_eta:eta/1^D_2 pi:pi/1^D_2_order0       | 0.0000 +/- 0          |      |       |       |       |       |       |       |       | FIXED |
| JP2+_gamma_eta:eta/1^D_2 pi:pi/1^D_2_order1       | 0.0000 +/- 0          |      |       |       |       |       |       |       |       | FIXED |
| JP2+_gamma_kaon:kaon/1^D_2 kaon:kaon/1^D_2_order0 | 0.0000 +/- 0          |      |       |       |       |       |       |       |       | FIXED |
| JP2+_gamma_kaon:kaon/1^D_2 kaon:kaon/1^D_2_order1 | 0.0000 +/- 0          |      |       |       |       |       |       |       |       | FIXED |
| JP2+_gamma_kaon:kaon/1^D_2 pi:pi/1^D_2_order0     | 0.0000 +/- 0          |      |       |       |       |       |       |       |       | FIXED |
| JP2+_gamma_pi:pi/1^D_2 pi:pi/1^D_2_order0         | 0.0000 +/- 0          |      |       |       |       |       |       |       |       | FIXED |

## pole singularities

\*\*\*\*\*

\*\*\*\*\*  
JP=2+ || eta:eta/1^D\_2[+] kaon:kaon/1^D\_2[+] pi:pi/1^D\_2[-]

$\sqrt{s}_{\text{pole}} = (0.2629 \pm 0.0012733) + (i/2)(-0.023227 \pm 0.0023595) [-0.10]$

| eta:eta/1^D_2             | kaon:kaon/1^D_2               | pi:pi/1^D_2                  |
|---------------------------|-------------------------------|------------------------------|
| k_re= -0.0812 +/- 0.0010  | k_re= -0.0890 +/- 0.0009      | k_re= 0.1119 +/- 0.0007      |
| k_im= 0.0094 +/- 0.0009   | k_im= 0.0086 +/- 0.0009       | k_im= -0.0068 +/- 0.0007     |
| corr= [-0.09]             | corr= [-0.09]                 | corr= [-0.10]                |
| g = 0.0000 +/- nan        | g = 0.0307 +/- 0.0058         | g = 0.0904 +/- 0.0048        |
| arg(g)/pi= 0.0000 +/- nan | arg(g)/pi= -0.0818 +/- 0.0765 | arg(g)/pi= 0.9435 +/- 0.0132 |

```

-----|-----|-----|
g_re= 0.0000 +/- 0.0000 | g_re= 0.0297 +/- 0.0060 | g_re= -0.0890 +/- 0.0050 |
g_im= 0.0000 +/- 0.0000 | g_im= -0.0078 +/- 0.0072 | g_im= 0.0160 +/- 0.0035 |
corr= [ 0.00] | corr= [ 0.18] | corr= [ 0.26] |
*****

*****
JP=2+ || eta:eta/1^D_2[+] kaon:kaon/1^D_2[-] pi:pi/1^D_2[+]

sqrt(s)_pole = (0.28306 +/- 0.0013665)
+ (i/2)*(-0.01094 +/- 0.0026603) [-0.15]

eta:eta/1^D_2 | kaon:kaon/1^D_2 | pi:pi/1^D_2 |
-----|-----|-----|
k_re= -0.0964 +/- 0.0010 | k_re= 0.1031 +/- 0.0009 | k_re= -0.1235 +/- 0.0008 |
k_im= 0.0040 +/- 0.0010 | k_im= -0.0038 +/- 0.0009 | k_im= 0.0031 +/- 0.0008 |
corr= [-0.15] | corr= [-0.15] | corr= [-0.15] |
-----|-----|-----|
|g|= 0.0000 +/- nan | |g|= 0.0675 +/- 0.0073 | |g|= 0.0123 +/- 0.0057 |
arg(g)/pi= 0.0000 +/- nan | arg(g)/pi= -0.0823 +/- 0.0144 | arg(g)/pi= 0.4300 +/- 0.4678 |
-----|-----|-----|
g_re= 0.0000 +/- 0.0000 | g_re= 0.0652 +/- 0.0066 | g_re= 0.0027 +/- 0.0181 |
g_im= 0.0000 +/- 0.0000 | g_im= -0.0172 +/- 0.0044 | g_im= 0.0120 +/- 0.0056 |
corr= [ 0.00] | corr= [-0.80] | corr= [-0.32] |
-----|-----|-----|
*****

*****
JP=2+ || eta:eta/1^D_2[+] kaon:kaon/1^D_2[-] pi:pi/1^D_2[-]

sqrt(s)_pole = (0.26159 +/- 0.001785)
+ (i/2)*(-0.028401 +/- 0.0024218) [ 0.03]

eta:eta/1^D_2 | kaon:kaon/1^D_2 | pi:pi/1^D_2 |
-----|-----|-----|
k_re= -0.0803 +/- 0.0014 | k_re= 0.0881 +/- 0.0013 | k_re= 0.1112 +/- 0.0010 |
k_im= 0.0116 +/- 0.0010 | k_im= -0.0105 +/- 0.0009 | k_im= -0.0084 +/- 0.0007 |
corr= [ 0.10] | corr= [ 0.09] | corr= [ 0.05] |
-----|-----|-----|
|g|= 0.0000 +/- nan | |g|= 0.0365 +/- 0.0075 | |g|= 0.0897 +/- 0.0057 |
arg(g)/pi= 0.0000 +/- nan | arg(g)/pi= -0.0717 +/- 0.0795 | arg(g)/pi= 0.9267 +/- 0.0185 |
-----|-----|-----|
g_re= 0.0000 +/- 0.0000 | g_re= 0.0356 +/- 0.0083 | g_re= -0.0874 +/- 0.0062 |
g_im= 0.0000 +/- 0.0000 | g_im= -0.0081 +/- 0.0084 | g_im= 0.0205 +/- 0.0046 |
corr= [ 0.00] | corr= [ 0.40] | corr= [ 0.39] |
-----|-----|-----|
*****

*****
JP=2+ || eta:eta/1^D_2[+] kaon:kaon/1^D_2[-] pi:pi/1^D_2[-]

sqrt(s)_pole = ( 0.2836 +/- 0.001295)
+ (i/2)*(-0.011227 +/- 0.0036346) [-0.35]

eta:eta/1^D_2 | kaon:kaon/1^D_2 | pi:pi/1^D_2 |
-----|-----|-----|
k_re= -0.0968 +/- 0.0010 | k_re= 0.1035 +/- 0.0009 | k_re= 0.1239 +/- 0.0007 |
k_im= 0.0041 +/- 0.0013 | k_im= -0.0038 +/- 0.0012 | k_im= -0.0032 +/- 0.0010 |
corr= [-0.36] | corr= [-0.36] | corr= [-0.35] |
-----|-----|-----|
|g|= 0.0000 +/- nan | |g|= 0.0629 +/- 0.0095 | |g|= 0.0147 +/- 0.0065 |
arg(g)/pi= 0.0000 +/- nan | arg(g)/pi= -0.0758 +/- 0.0256 | arg(g)/pi= -0.0130 +/- 0.4492 |
-----|-----|-----|
g_re= 0.0000 +/- 0.0000 | g_re= 0.0611 +/- 0.0083 | g_re= 0.0147 +/- 0.0061 |
g_im= 0.0000 +/- 0.0000 | g_im= -0.0148 +/- 0.0068 | g_im= -0.0006 +/- 0.0209 |
corr= [ 0.00] | corr= [-0.84] | corr= [-0.40] |
-----|-----|-----|
*****

*****
JP=2+ || eta:eta/1^D_2[-] kaon:kaon/1^D_2[+] pi:pi/1^D_2[-]

sqrt(s)_pole = ( 0.2629 +/- 0.0012733)
+ (i/2)*(-0.023227 +/- 0.0023595) [-0.10]

eta:eta/1^D_2 | kaon:kaon/1^D_2 | pi:pi/1^D_2 |
-----|-----|-----|
k_re= 0.0812 +/- 0.0010 | k_re= -0.0890 +/- 0.0009 | k_re= 0.1119 +/- 0.0007 |
k_im= -0.0094 +/- 0.0009 | k_im= 0.0086 +/- 0.0009 | k_im= -0.0068 +/- 0.0007 |
corr= [-0.09] | corr= [-0.09] | corr= [-0.10] |
-----|-----|-----|
|g|= 0.0000 +/- nan | |g|= 0.0307 +/- 0.0058 | |g|= 0.0904 +/- 0.0048 |
arg(g)/pi= 0.0000 +/- nan | arg(g)/pi= -0.0818 +/- 0.0765 | arg(g)/pi= 0.9435 +/- 0.0132 |
-----|-----|-----|
g_re= 0.0000 +/- 0.0000 | g_re= 0.0297 +/- 0.0060 | g_re= -0.0890 +/- 0.0050 |
g_im= 0.0000 +/- 0.0000 | g_im= -0.0078 +/- 0.0072 | g_im= 0.0160 +/- 0.0035 |
corr= [ 0.00] | corr= [ 0.18] | corr= [ 0.26] |
-----|-----|-----|
*****

*****
JP=2+ || eta:eta/1^D_2[-] kaon:kaon/1^D_2[-] pi:pi/1^D_2[+]

sqrt(s)_pole = (0.28306 +/- 0.0013665)
+ (i/2)*(-0.01094 +/- 0.0026603) [-0.15]

eta:eta/1^D_2 | kaon:kaon/1^D_2 | pi:pi/1^D_2 |
-----|-----|-----|
k_re= 0.0964 +/- 0.0010 | k_re= 0.1031 +/- 0.0009 | k_re= -0.1235 +/- 0.0008 |
k_im= -0.0040 +/- 0.0010 | k_im= -0.0038 +/- 0.0009 | k_im= 0.0031 +/- 0.0008 |
corr= [-0.15] | corr= [-0.15] | corr= [-0.15] |
-----|-----|-----|

```



```

=====|=====|=====|
|g|= 0.0000 +/- nan | |g|= 0.0675 +/- 0.0073 | |g|= 0.0123 +/- 0.0057 |
arg(g)/pi= 0.0000 +/- nan |arg(g)/pi= -0.0823 +/- 0.0144 |arg(g)/pi= 0.4300 +/- 0.4678 |
-----|-----|-----|
g_re= 0.0000 +/- 0.0000 | g_re= 0.0652 +/- 0.0066 | g_re= 0.0027 +/- 0.0181 |
g_im= 0.0000 +/- 0.0000 | g_im= -0.0172 +/- 0.0044 | g_im= 0.0120 +/- 0.0056 |
corr= [ 0.00] | corr= [-0.80] | corr= [-0.32] |
*****

```

```

*****
JP=2+ || eta:eta/1^D_2[-] kaon:kaon/1^D_2[-] pi:pi/1^D_2[-]

```

```

sqrt(s)_pole = (0.26159 +/- 0.001785)
+ (i/2)*(-0.028401 +/- 0.0024218) [ 0.03]

```

```

eta:eta/1^D_2 | kaon:kaon/1^D_2 | pi:pi/1^D_2 |
=====|=====|=====|
k_re= 0.0803 +/- 0.0014 | k_re= 0.0881 +/- 0.0013 | k_re= 0.1112 +/- 0.0010 |
k_im= -0.0116 +/- 0.0010 | k_im= -0.0105 +/- 0.0009 | k_im= -0.0084 +/- 0.0007 |
corr= [ 0.10] | corr= [ 0.09] | corr= [ 0.05] |
-----|-----|-----|
|g|= 0.0000 +/- nan | |g|= 0.0365 +/- 0.0075 | |g|= 0.0897 +/- 0.0057 |
arg(g)/pi= 0.0000 +/- nan |arg(g)/pi= -0.0717 +/- 0.0795 |arg(g)/pi= 0.9267 +/- 0.0185 |
-----|-----|-----|
g_re= 0.0000 +/- 0.0000 | g_re= 0.0356 +/- 0.0083 | g_re= -0.0874 +/- 0.0062 |
g_im= 0.0000 +/- 0.0000 | g_im= -0.0081 +/- 0.0084 | g_im= 0.0205 +/- 0.0046 |
corr= [ 0.00] | corr= [ 0.40] | corr= [ 0.39] |
*****

```

```

*****
JP=2+ || eta:eta/1^D_2[-] kaon:kaon/1^D_2[-] pi:pi/1^D_2[-]

```

```

sqrt(s)_pole = ( 0.2836 +/- 0.001295)
+ (i/2)*(-0.011227 +/- 0.0036346) [-0.35]

```

```

eta:eta/1^D_2 | kaon:kaon/1^D_2 | pi:pi/1^D_2 |
=====|=====|=====|
k_re= 0.0968 +/- 0.0010 | k_re= 0.1035 +/- 0.0009 | k_re= 0.1239 +/- 0.0007 |
k_im= -0.0041 +/- 0.0013 | k_im= -0.0038 +/- 0.0012 | k_im= -0.0032 +/- 0.0010 |
corr= [-0.36] | corr= [-0.36] | corr= [-0.35] |
-----|-----|-----|
|g|= 0.0000 +/- nan | |g|= 0.0629 +/- 0.0095 | |g|= 0.0147 +/- 0.0065 |
arg(g)/pi= 0.0000 +/- nan |arg(g)/pi= -0.0758 +/- 0.0256 |arg(g)/pi= -0.0130 +/- 0.4492 |
-----|-----|-----|
g_re= 0.0000 +/- 0.0000 | g_re= 0.0611 +/- 0.0083 | g_re= 0.0147 +/- 0.0061 |
g_im= 0.0000 +/- 0.0000 | g_im= -0.0148 +/- 0.0068 | g_im= -0.0006 +/- 0.0209 |
corr= [ 0.00] | corr= [-0.84] | corr= [-0.40] |
*****

```

## k\_2poles\_sxxxxs\_noCM

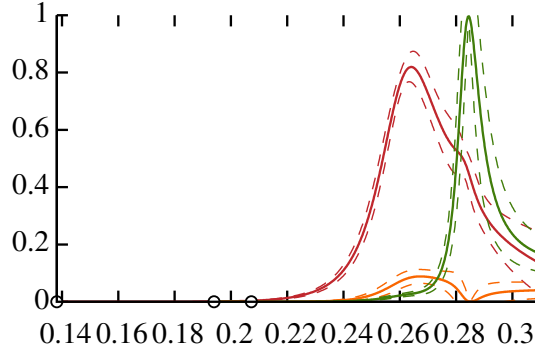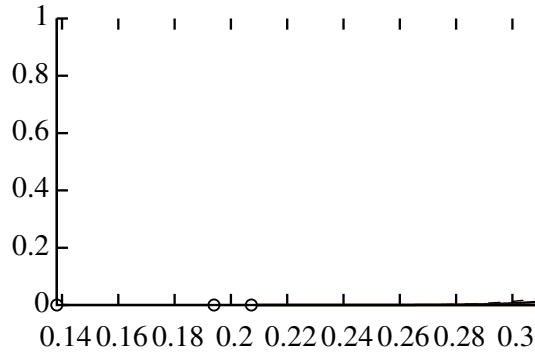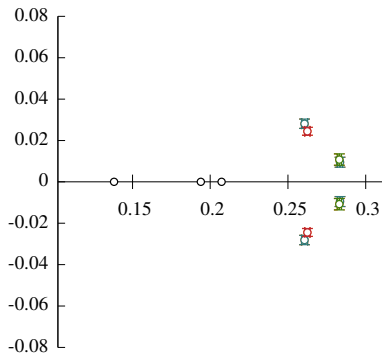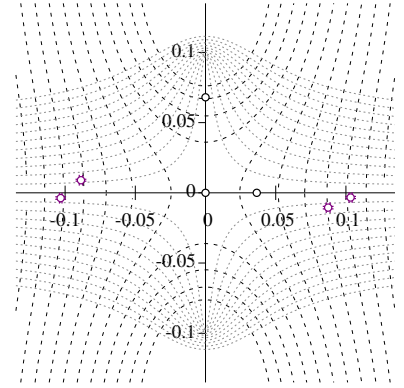

### parameter values

minimised with  $\text{chisq}/\text{nDoF} = 27.08 / (34 - 8) = 1.04$

|                                                   |                       |      |      |       |       |       |       |       |       |
|---------------------------------------------------|-----------------------|------|------|-------|-------|-------|-------|-------|-------|
| JP2+_g_kaon:kaon/1^D_2_pole0                      | -1.0442 +/- 0.20649   | 1.00 | 0.25 | -0.44 | 0.29  | 0.00  | 0.37  | 0.60  | 0.53  |
| JP2+_g_kaon:kaon/1^D_2_pole1                      | 1.4752 +/- 0.20577    | 1.00 | 0.30 | -0.53 | 0.15  | 0.10  | 0.29  | 0.42  |       |
| JP2+_g_pi:pi/1^D_2_pole0                          | 1.8077 +/- 0.091172   |      | 1.00 | -0.66 | 0.09  | -0.45 | -0.28 | -0.37 |       |
| JP2+_g_pi:pi/1^D_2_pole1                          | 0.050318 +/- 0.21185  |      |      | 1.00  | -0.14 | 0.47  | 0.08  | 0.28  |       |
| JP2+_gamma_eta:eta/1^D_2 eta:eta/1^D_2_order1     | 541.15 +/- 302.71     |      |      |       | 1.00  | 0.08  | -0.08 | -0.08 |       |
| JP2+_gamma_pi:pi/1^D_2 pi:pi/1^D_2_order1         | 451.24 +/- 380.98     |      |      |       |       | 1.00  | 0.39  | 0.31  |       |
| JP2+_m_pole0                                      | 0.26439 +/- 0.0012186 |      |      |       |       |       | 1.00  | 0.46  |       |
| JP2+_m_pole1                                      | 0.28435 +/- 0.0016711 |      |      |       |       |       |       | 1.00  |       |
| JP2+_g_eta:eta/1^D_2_pole0                        | 0.0000 +/- 0          |      |      |       |       |       |       |       | FIXED |
| JP2+_g_eta:eta/1^D_2_pole1                        | 0.0000 +/- 0          |      |      |       |       |       |       |       | FIXED |
| JP2+_gamma_eta:eta/1^D_2 eta:eta/1^D_2_order0     | 0.0000 +/- 0          |      |      |       |       |       |       |       | FIXED |
| JP2+_gamma_eta:eta/1^D_2 kaon:kaon/1^D_2_order0   | 0.0000 +/- 0          |      |      |       |       |       |       |       | FIXED |
| JP2+_gamma_eta:eta/1^D_2 kaon:kaon/1^D_2_order1   | 0.0000 +/- 0          |      |      |       |       |       |       |       | FIXED |
| JP2+_gamma_eta:eta/1^D_2 pi:pi/1^D_2_order0       | 0.0000 +/- 0          |      |      |       |       |       |       |       | FIXED |
| JP2+_gamma_eta:eta/1^D_2 pi:pi/1^D_2_order1       | 0.0000 +/- 0          |      |      |       |       |       |       |       | FIXED |
| JP2+_gamma_kaon:kaon/1^D_2 kaon:kaon/1^D_2_order0 | 0.0000 +/- 0          |      |      |       |       |       |       |       | FIXED |
| JP2+_gamma_kaon:kaon/1^D_2 kaon:kaon/1^D_2_order1 | 0.0000 +/- 0          |      |      |       |       |       |       |       | FIXED |
| JP2+_gamma_kaon:kaon/1^D_2 pi:pi/1^D_2_order0     | 0.0000 +/- 0          |      |      |       |       |       |       |       | FIXED |
| JP2+_gamma_kaon:kaon/1^D_2 pi:pi/1^D_2_order1     | 0.0000 +/- 0          |      |      |       |       |       |       |       | FIXED |
| JP2+_gamma_pi:pi/1^D_2 pi:pi/1^D_2_order0         | 0.0000 +/- 0          |      |      |       |       |       |       |       | FIXED |

### pole singularities

\*\*\*\*\*

\*\*\*\*\*  
JP=2+ || eta:eta/1^D\_2[+] kaon:kaon/1^D\_2[+] pi:pi/1^D\_2[-]

$\text{sqrt}(s)_{\text{pole}} = (0.26251 \pm 0.0016895) + (i/2)(-0.024443 \pm 0.0019027) [-0.13]$

| eta:eta/1^D_2             | kaon:kaon/1^D_2               | pi:pi/1^D_2                  |
|---------------------------|-------------------------------|------------------------------|
| k_re= -0.0809 +/- 0.0014  | k_re= -0.0887 +/- 0.0012      | k_re= 0.1117 +/- 0.0010      |
| k_im= 0.0099 +/- 0.0008   | k_im= 0.0090 +/- 0.0007       | k_im= -0.0072 +/- 0.0006     |
| corr= [-0.04]             | corr= [-0.06]                 | corr= [-0.11]                |
| g = 0.0000 +/- nan        | g = 0.0297 +/- 0.0062         | g = 0.0918 +/- 0.0041        |
| arg(g)/pi= 0.0000 +/- nan | arg(g)/pi= -0.1328 +/- 0.0256 | arg(g)/pi= 0.9353 +/- 0.0155 |

```

-----|-----|-----|
g_re= 0.0000 +/- 0.0000 | g_re= 0.0272 +/- 0.0063 | g_re= -0.0899 +/- 0.0045 |
g_im= 0.0000 +/- 0.0000 | g_im= -0.0120 +/- 0.0022 | g_im= 0.0185 +/- 0.0041 |
corr= [ 0.00] | corr= [-0.47] | corr= [ 0.37] |
*****

*****
JP=2+ || eta:eta/1^D_2[+] kaon:kaon/1^D_2[-] pi:pi/1^D_2[+]

sqrt(s)_pole = (0.28306 +/- 0.0013343)
+ (i/2)*(-0.010786 +/- 0.0027275) [-0.50]

eta:eta/1^D_2 | kaon:kaon/1^D_2 | pi:pi/1^D_2 |
-----|-----|-----|
k_re= -0.0964 +/- 0.0010 | k_re= 0.1031 +/- 0.0009 | k_re= -0.1235 +/- 0.0008 |
k_im= 0.0040 +/- 0.0010 | k_im= -0.0037 +/- 0.0009 | k_im= 0.0031 +/- 0.0008 |
corr= [-0.50] | corr= [-0.50] | corr= [-0.50] |
-----|-----|-----|
|g|= 0.0000 +/- nan | |g|= 0.0666 +/- 0.0077 | |g|= 0.0152 +/- 0.0027 |
arg(g)/pi= 0.0000 +/- nan | arg(g)/pi= -0.0694 +/- 0.0107 | arg(g)/pi= 0.6356 +/- 0.2196 |
-----|-----|-----|
g_re= 0.0000 +/- 0.0000 | g_re= 0.0651 +/- 0.0073 | g_re= -0.0063 +/- 0.0097 |
g_im= 0.0000 +/- 0.0000 | g_im= -0.0144 +/- 0.0033 | g_im= 0.0138 +/- 0.0047 |
corr= [ 0.00] | corr= [-0.79] | corr= [ 0.79] |
-----|-----|-----|
*****

*****
JP=2+ || eta:eta/1^D_2[+] kaon:kaon/1^D_2[-] pi:pi/1^D_2[-]

sqrt(s)_pole = (0.26068 +/- 0.0019809)
+ (i/2)*(-0.028087 +/- 0.0022803) [ 0.38]

eta:eta/1^D_2 | kaon:kaon/1^D_2 | pi:pi/1^D_2 |
-----|-----|-----|
k_re= -0.0796 +/- 0.0016 | k_re= 0.0874 +/- 0.0014 | k_re= 0.1106 +/- 0.0012 |
k_im= 0.0115 +/- 0.0010 | k_im= -0.0105 +/- 0.0009 | k_im= -0.0083 +/- 0.0007 |
corr= [ 0.46] | corr= [ 0.44] | corr= [ 0.40] |
-----|-----|-----|
|g|= 0.0000 +/- nan | |g|= 0.0333 +/- 0.0060 | |g|= 0.0873 +/- 0.0037 |
arg(g)/pi= 0.0000 +/- nan | arg(g)/pi= -0.1192 +/- 0.0162 | arg(g)/pi= 0.9157 +/- 0.0198 |
-----|-----|-----|
g_re= 0.0000 +/- 0.0000 | g_re= 0.0310 +/- 0.0056 | g_re= -0.0843 +/- 0.0041 |
g_im= 0.0000 +/- 0.0000 | g_im= -0.0122 +/- 0.0027 | g_im= 0.0229 +/- 0.0051 |
corr= [ 0.00] | corr= [-0.75] | corr= [ 0.36] |
-----|-----|-----|
*****

*****
JP=2+ || eta:eta/1^D_2[+] kaon:kaon/1^D_2[-] pi:pi/1^D_2[-]

sqrt(s)_pole = (0.28349 +/- 0.0016503)
+ (i/2)*(-0.0095062 +/- 0.0024215) [-0.54]

eta:eta/1^D_2 | kaon:kaon/1^D_2 | pi:pi/1^D_2 |
-----|-----|-----|
k_re= -0.0967 +/- 0.0012 | k_re= 0.1034 +/- 0.0011 | k_re= 0.1238 +/- 0.0009 |
k_im= 0.0035 +/- 0.0009 | k_im= -0.0033 +/- 0.0008 | k_im= -0.0027 +/- 0.0007 |
corr= [-0.54] | corr= [-0.54] | corr= [-0.54] |
-----|-----|-----|
|g|= 0.0000 +/- nan | |g|= 0.0579 +/- 0.0076 | |g|= 0.0163 +/- 0.0027 |
arg(g)/pi= 0.0000 +/- nan | arg(g)/pi= -0.0612 +/- 0.0236 | arg(g)/pi= 0.1735 +/- 0.1782 |
-----|-----|-----|
g_re= 0.0000 +/- 0.0000 | g_re= 0.0568 +/- 0.0073 | g_re= 0.0139 +/- 0.0055 |
g_im= 0.0000 +/- 0.0000 | g_im= -0.0111 +/- 0.0049 | g_im= 0.0085 +/- 0.0078 |
corr= [ 0.00] | corr= [-0.49] | corr= [-0.82] |
-----|-----|-----|
*****

*****
JP=2+ || eta:eta/1^D_2[-] kaon:kaon/1^D_2[+] pi:pi/1^D_2[-]

sqrt(s)_pole = (0.26251 +/- 0.0016895)
+ (i/2)*(-0.024443 +/- 0.0019027) [-0.13]

eta:eta/1^D_2 | kaon:kaon/1^D_2 | pi:pi/1^D_2 |
-----|-----|-----|
k_re= 0.0809 +/- 0.0014 | k_re= -0.0887 +/- 0.0012 | k_re= 0.1117 +/- 0.0010 |
k_im= -0.0099 +/- 0.0008 | k_im= 0.0090 +/- 0.0007 | k_im= -0.0072 +/- 0.0006 |
corr= [-0.04] | corr= [-0.06] | corr= [-0.11] |
-----|-----|-----|
|g|= 0.0000 +/- nan | |g|= 0.0297 +/- 0.0062 | |g|= 0.0918 +/- 0.0041 |
arg(g)/pi= 0.0000 +/- nan | arg(g)/pi= -0.1328 +/- 0.0256 | arg(g)/pi= 0.9353 +/- 0.0155 |
-----|-----|-----|
g_re= 0.0000 +/- 0.0000 | g_re= 0.0272 +/- 0.0063 | g_re= -0.0899 +/- 0.0045 |
g_im= 0.0000 +/- 0.0000 | g_im= -0.0120 +/- 0.0022 | g_im= 0.0185 +/- 0.0041 |
corr= [ 0.00] | corr= [-0.47] | corr= [ 0.37] |
-----|-----|-----|
*****

*****
JP=2+ || eta:eta/1^D_2[-] kaon:kaon/1^D_2[-] pi:pi/1^D_2[+]

sqrt(s)_pole = (0.28306 +/- 0.0013343)
+ (i/2)*(-0.010786 +/- 0.0027275) [-0.50]

eta:eta/1^D_2 | kaon:kaon/1^D_2 | pi:pi/1^D_2 |
-----|-----|-----|
k_re= 0.0964 +/- 0.0010 | k_re= 0.1031 +/- 0.0009 | k_re= -0.1235 +/- 0.0008 |
k_im= -0.0040 +/- 0.0010 | k_im= -0.0037 +/- 0.0009 | k_im= 0.0031 +/- 0.0008 |
corr= [-0.50] | corr= [-0.50] | corr= [-0.50] |
-----|-----|-----|

```

```

=====|=====|=====|
|g|= 0.0000 +/- nan | |g|= 0.0666 +/- 0.0077 | |g|= 0.0152 +/- 0.0027 |
arg(g)/pi= 0.0000 +/- nan |arg(g)/pi= -0.0694 +/- 0.0107 |arg(g)/pi= 0.6356 +/- 0.2196 |
-----|-----|-----|
g_re= 0.0000 +/- 0.0000 | g_re= 0.0651 +/- 0.0073 | g_re= -0.0063 +/- 0.0097 |
g_im= 0.0000 +/- 0.0000 | g_im= -0.0144 +/- 0.0033 | g_im= 0.0138 +/- 0.0047 |
corr= [ 0.00] | corr= [-0.79] | corr= [ 0.79] |
*****

```

```

*****
JP=2+ || eta:eta/1^D_2[-] kaon:kaon/1^D_2[-] pi:pi/1^D_2[-]

```

```

sqrt(s)_pole = (0.26068 +/- 0.0019809)
               + (i/2)*(-0.028087 +/- 0.0022803) [ 0.38]

```

```

           eta:eta/1^D_2 |           kaon:kaon/1^D_2 |           pi:pi/1^D_2 |
=====|=====|=====|
k_re= 0.0796 +/- 0.0016 | k_re= 0.0874 +/- 0.0014 | k_re= 0.1106 +/- 0.0012 |
k_im= -0.0115 +/- 0.0010 | k_im= -0.0105 +/- 0.0009 | k_im= -0.0083 +/- 0.0007 |
corr= [ 0.46] | corr= [ 0.44] | corr= [ 0.40] |
-----|-----|-----|
|g|= 0.0000 +/- nan | |g|= 0.0333 +/- 0.0060 | |g|= 0.0873 +/- 0.0037 |
arg(g)/pi= 0.0000 +/- nan |arg(g)/pi= -0.1192 +/- 0.0162 |arg(g)/pi= 0.9157 +/- 0.0198 |
-----|-----|-----|
g_re= 0.0000 +/- 0.0000 | g_re= 0.0310 +/- 0.0056 | g_re= -0.0843 +/- 0.0041 |
g_im= 0.0000 +/- 0.0000 | g_im= -0.0122 +/- 0.0027 | g_im= 0.0229 +/- 0.0051 |
corr= [ 0.00] | corr= [-0.75] | corr= [ 0.36] |
*****

```

```

*****
JP=2+ || eta:eta/1^D_2[-] kaon:kaon/1^D_2[-] pi:pi/1^D_2[-]

```

```

sqrt(s)_pole = (0.28349 +/- 0.0016503)
               + (i/2)*(-0.0095062 +/- 0.0024215) [-0.54]

```

```

           eta:eta/1^D_2 |           kaon:kaon/1^D_2 |           pi:pi/1^D_2 |
=====|=====|=====|
k_re= 0.0967 +/- 0.0012 | k_re= 0.1034 +/- 0.0011 | k_re= 0.1238 +/- 0.0009 |
k_im= -0.0035 +/- 0.0009 | k_im= -0.0033 +/- 0.0008 | k_im= -0.0027 +/- 0.0007 |
corr= [-0.54] | corr= [-0.54] | corr= [-0.54] |
-----|-----|-----|
|g|= 0.0000 +/- nan | |g|= 0.0579 +/- 0.0076 | |g|= 0.0163 +/- 0.0027 |
arg(g)/pi= 0.0000 +/- nan |arg(g)/pi= -0.0612 +/- 0.0236 |arg(g)/pi= 0.1735 +/- 0.1782 |
-----|-----|-----|
g_re= 0.0000 +/- 0.0000 | g_re= 0.0568 +/- 0.0073 | g_re= 0.0139 +/- 0.0055 |
g_im= 0.0000 +/- 0.0000 | g_im= -0.0111 +/- 0.0049 | g_im= 0.0085 +/- 0.0078 |
corr= [ 0.00] | corr= [-0.49] | corr= [-0.82] |
*****

```

# k\_2poles\_xxcxcc\_noCM

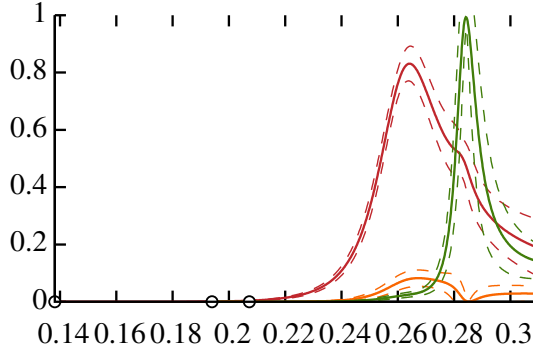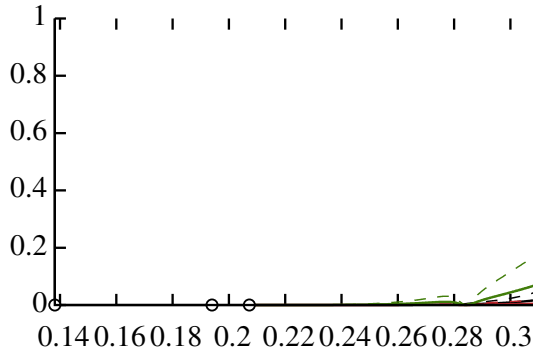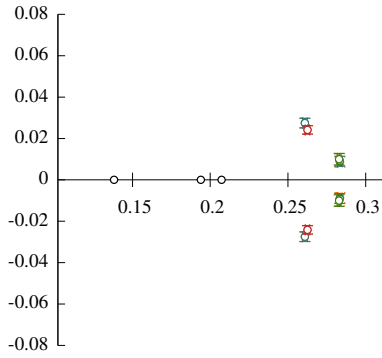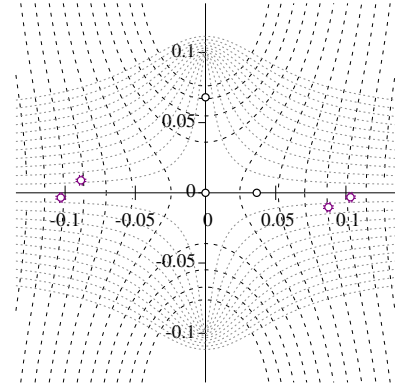

## parameter values

minimised with  $\chi^2/\text{nDoF} = 26.46 / (34 - 10) = 1.10$

|                                                   |                       |      |       |       |       |       |       |      |       |      |       |
|---------------------------------------------------|-----------------------|------|-------|-------|-------|-------|-------|------|-------|------|-------|
| JP2+_g_kaon:kaon/1^D_2_pole0                      | -1.0004 +/- 0.20406   | 1.00 | -0.12 | -0.20 | 0.31  | -0.04 | 0.49  | 0.23 | 0.02  | 0.34 | 0.26  |
| JP2+_g_kaon:kaon/1^D_2_pole1                      | 1.4069 +/- 0.22917    | 1.00 | 0.31  | -0.63 | 0.35  | -0.40 | -0.08 | 0.12 | 0.09  | 0.39 |       |
| JP2+_g_pi:pi/1^D_2_pole0                          | 1.7976 +/- 0.092568   | 1.00 | -0.59 | 0.13  | 0.09  | -0.16 | -0.48 | 0.00 | -0.24 |      |       |
| JP2+_g_pi:pi/1^D_2_pole1                          | 0.069742 +/- 0.21117  | 1.00 | -0.13 | 0.17  | 0.38  | 0.25  | -0.06 | 0.17 |       |      |       |
| JP2+_gamma_eta:eta/1^D_2 eta:eta/1^D_2_order0     | 37.722 +/- 47.245     | 1.00 | -0.34 | 0.62  | -0.03 | -0.10 | 0.17  |      |       |      |       |
| JP2+_gamma_eta:eta/1^D_2 kaon:kaon/1^D_2_order0   | 139.49 +/- 111.21     | 1.00 | -0.04 | -0.10 | 0.22  | -0.15 |       |      |       |      |       |
| JP2+_gamma_eta:eta/1^D_2 pi:pi/1^D_2_order0       | 9.5556 +/- 51.81      | 1.00 | 0.01  | -0.05 | 0.22  |       |       |      |       |      |       |
| JP2+_gamma_pi:pi/1^D_2 pi:pi/1^D_2_order0         | 27.351 +/- 22.773     | 1.00 | 0.15  | 0.14  |       |       |       |      |       |      |       |
| JP2+_m_pole0                                      | 0.26449 +/- 0.0009598 |      |       |       |       |       |       | 1.00 | 0.21  |      |       |
| JP2+_m_pole1                                      | 0.28413 +/- 0.0015125 |      |       |       |       |       |       |      | 1.00  |      |       |
| JP2+_g_eta:eta/1^D_2_pole0                        | 0.0000 +/- 0          |      |       |       |       |       |       |      |       |      | FIXED |
| JP2+_g_eta:eta/1^D_2_pole1                        | 0.0000 +/- 0          |      |       |       |       |       |       |      |       |      | FIXED |
| JP2+_gamma_kaon:kaon/1^D_2 kaon:kaon/1^D_2_order0 | 0.0000 +/- 0          |      |       |       |       |       |       |      |       |      | FIXED |
| JP2+_gamma_kaon:kaon/1^D_2 pi:pi/1^D_2_order0     | 0.0000 +/- 0          |      |       |       |       |       |       |      |       |      | FIXED |

## pole singularities

\*\*\*\*\*

\*\*\*\*\*

JP=2+ || eta:eta/1^D\_2[+] kaon:kaon/1^D\_2[+] pi:pi/1^D\_2[-]

sqrt(s)\_pole = (0.26255 +/- 0.0013576)  
+ (i/2)\*(-0.024129 +/- 0.0020326) [ 0.20]

| eta:eta/1^D_2                | kaon:kaon/1^D_2              | pi:pi/1^D_2                   |
|------------------------------|------------------------------|-------------------------------|
| k_re= -0.0809 +/- 0.0011     | k_re= -0.0887 +/- 0.0010     | k_re= 0.1117 +/- 0.0008       |
| k_im= 0.0098 +/- 0.0008      | k_im= 0.0089 +/- 0.0008      | k_im= -0.0071 +/- 0.0006      |
| corr= [ 0.24]                | corr= [ 0.23]                | corr= [ 0.21]                 |
| g = 0.0032 +/- 0.0051        | g = 0.0283 +/- 0.0068        | g = 0.0902 +/- 0.0033         |
| arg(g)/pi= 0.2387 +/- 0.1093 | arg(g)/pi= 0.8709 +/- 0.0203 | arg(g)/pi= -0.0645 +/- 0.0173 |
| g_re= 0.0023 +/- 0.0031      | g_re= -0.0260 +/- 0.0067     | g_re= 0.0884 +/- 0.0034       |
| g_im= 0.0022 +/- 0.0042      | g_im= 0.0112 +/- 0.0023      | g_im= -0.0182 +/- 0.0049      |
| corr= [ 0.98]                | corr= [-0.73]                | corr= [ 0.14]                 |

\*\*\*\*\*

```

*****
JP=2+  ||  eta:eta/1^D_2[+] kaon:kaon/1^D_2[-] pi:pi/1^D_2[+]

sqrt(s)_pole = (0.28291 +/- 0.0011527)
               + (i/2)*(-0.0099972 +/- 0.0027921) [-0.40]

eta:eta/1^D_2 | kaon:kaon/1^D_2 | pi:pi/1^D_2 |
=====|=====|=====|
k_re= -0.0963 +/- 0.0009 | k_re= 0.1030 +/- 0.0008 | k_re= -0.1235 +/- 0.0007 |
k_im= 0.0037 +/- 0.0010 | k_im= -0.0034 +/- 0.0010 | k_im= 0.0029 +/- 0.0008 |
corr= [-0.41] | corr= [-0.41] | corr= [-0.41] |
=====|=====|=====|
|g|= 0.0105 +/- 0.0084 | |g|= 0.0647 +/- 0.0080 | |g|= 0.0143 +/- 0.0031 |
arg(g)/pi= 0.3619 +/- 0.0558 | arg(g)/pi= -0.0700 +/- 0.0114 | arg(g)/pi= 0.6185 +/- 0.2140 |
-----|-----|-----|
g_re= 0.0044 +/- 0.0037 | g_re= 0.0632 +/- 0.0076 | g_re= -0.0052 +/- 0.0090 |
g_im= 0.0095 +/- 0.0078 | g_im= -0.0141 +/- 0.0035 | g_im= 0.0133 +/- 0.0045 |
corr= [ 0.85] | corr= [-0.81] | corr= [ 0.69] |
*****

```

```

*****
JP=2+  ||  eta:eta/1^D_2[+] kaon:kaon/1^D_2[-] pi:pi/1^D_2[-]

sqrt(s)_pole = (0.26092 +/- 0.0014797)
               + (i/2)*(-0.027471 +/- 0.0023312) [ 0.40]

eta:eta/1^D_2 | kaon:kaon/1^D_2 | pi:pi/1^D_2 |
=====|=====|=====|
k_re= -0.0797 +/- 0.0012 | k_re= 0.0876 +/- 0.0011 | k_re= 0.1108 +/- 0.0009 |
k_im= 0.0112 +/- 0.0010 | k_im= -0.0102 +/- 0.0009 | k_im= -0.0081 +/- 0.0007 |
corr= [ 0.43] | corr= [ 0.42] | corr= [ 0.41] |
=====|=====|=====|
|g|= 0.0015 +/- 0.0049 | |g|= 0.0317 +/- 0.0071 | |g|= 0.0863 +/- 0.0032 |
arg(g)/pi= 0.1499 +/- 0.3747 | arg(g)/pi= -0.1181 +/- 0.0144 | arg(g)/pi= 0.9183 +/- 0.0184 |
-----|-----|-----|
g_re= 0.0014 +/- 0.0036 | g_re= 0.0296 +/- 0.0067 | g_re= -0.0834 +/- 0.0031 |
g_im= 0.0007 +/- 0.0038 | g_im= -0.0115 +/- 0.0027 | g_im= 0.0219 +/- 0.0050 |
corr= [ 0.99] | corr= [-0.84] | corr= [ 0.06] |
*****

```

```

*****
JP=2+  ||  eta:eta/1^D_2[+] kaon:kaon/1^D_2[-] pi:pi/1^D_2[-]

sqrt(s)_pole = (0.28336 +/- 0.0013831)
               + (i/2)*(-0.0089925 +/- 0.0023757) [-0.47]

eta:eta/1^D_2 | kaon:kaon/1^D_2 | pi:pi/1^D_2 |
=====|=====|=====|
k_re= -0.0966 +/- 0.0010 | k_re= 0.1033 +/- 0.0010 | k_re= 0.1237 +/- 0.0008 |
k_im= 0.0033 +/- 0.0009 | k_im= -0.0031 +/- 0.0008 | k_im= -0.0026 +/- 0.0007 |
corr= [-0.46] | corr= [-0.46] | corr= [-0.46] |
=====|=====|=====|
|g|= 0.0095 +/- 0.0080 | |g|= 0.0571 +/- 0.0075 | |g|= 0.0152 +/- 0.0030 |
arg(g)/pi= 0.3903 +/- 0.0389 | arg(g)/pi= -0.0594 +/- 0.0219 | arg(g)/pi= 0.1463 +/- 0.1886 |
-----|-----|-----|
g_re= 0.0032 +/- 0.0028 | g_re= 0.0561 +/- 0.0071 | g_re= 0.0136 +/- 0.0050 |
g_im= 0.0089 +/- 0.0076 | g_im= -0.0106 +/- 0.0046 | g_im= 0.0068 +/- 0.0081 |
corr= [ 0.90] | corr= [-0.59] | corr= [-0.74] |
*****

```

```

*****
JP=2+  ||  eta:eta/1^D_2[-] kaon:kaon/1^D_2[+] pi:pi/1^D_2[-]

sqrt(s)_pole = (0.26257 +/- 0.0013525)
               + (i/2)*(-0.024133 +/- 0.002041) [ 0.20]

eta:eta/1^D_2 | kaon:kaon/1^D_2 | pi:pi/1^D_2 |
=====|=====|=====|
k_re= 0.0810 +/- 0.0011 | k_re= -0.0887 +/- 0.0010 | k_re= 0.1117 +/- 0.0008 |
k_im= -0.0098 +/- 0.0008 | k_im= 0.0089 +/- 0.0008 | k_im= -0.0071 +/- 0.0006 |
corr= [ 0.23] | corr= [ 0.23] | corr= [ 0.21] |
=====|=====|=====|
|g|= 0.0033 +/- 0.0053 | |g|= 0.0286 +/- 0.0066 | |g|= 0.0903 +/- 0.0033 |
arg(g)/pi= 0.2447 +/- 0.1192 | arg(g)/pi= 0.8668 +/- 0.0237 | arg(g)/pi= -0.0644 +/- 0.0173 |
-----|-----|-----|
g_re= 0.0023 +/- 0.0031 | g_re= -0.0261 +/- 0.0066 | g_re= 0.0885 +/- 0.0033 |
g_im= 0.0023 +/- 0.0044 | g_im= 0.0116 +/- 0.0021 | g_im= -0.0181 +/- 0.0049 |
corr= [ 0.97] | corr= [-0.61] | corr= [ 0.13] |
*****

```

```

*****
JP=2+  ||  eta:eta/1^D_2[-] kaon:kaon/1^D_2[-] pi:pi/1^D_2[+]

sqrt(s)_pole = (0.28309 +/- 0.0012011)
               + (i/2)*(-0.0096228 +/- 0.0030182) [-0.29]

eta:eta/1^D_2 | kaon:kaon/1^D_2 | pi:pi/1^D_2 |
=====|=====|=====|
k_re= 0.0964 +/- 0.0009 | k_re= 0.1031 +/- 0.0008 | k_re= -0.1236 +/- 0.0007 |
k_im= -0.0035 +/- 0.0011 | k_im= -0.0033 +/- 0.0010 | k_im= 0.0028 +/- 0.0009 |
corr= [-0.30] | corr= [-0.30] | corr= [-0.30] |
=====|=====|=====|
|g|= 0.0102 +/- 0.0076 | |g|= 0.0623 +/- 0.0101 | |g|= 0.0138 +/- 0.0035 |
arg(g)/pi= 0.3963 +/- 0.0422 | arg(g)/pi= -0.0599 +/- 0.0181 | arg(g)/pi= 0.6283 +/- 0.2134 |
-----|-----|-----|
g_re= 0.0033 +/- 0.0022 | g_re= 0.0612 +/- 0.0094 | g_re= -0.0054 +/- 0.0086 |
g_im= 0.0097 +/- 0.0074 | g_im= -0.0116 +/- 0.0050 | g_im= 0.0127 +/- 0.0048 |

```

```

corr= [ 0.82] | corr= [-0.86] | corr= [ 0.63] |
*****

```

```

*****
JP=2+ || eta:eta/1^D_2[-] kaon:kaon/1^D_2[-] pi:pi/1^D_2[-]

```

```

sqrt(s)_pole = (0.26092 +/- 0.0014807)
               + (i/2)*(-0.027477 +/- 0.0023362) [ 0.39]

```

| eta:eta/1^D_2                |  | kaon:kaon/1^D_2               |  | pi:pi/1^D_2                  |  |
|------------------------------|--|-------------------------------|--|------------------------------|--|
| k_re= 0.0797 +/- 0.0012      |  | k_re= 0.0876 +/- 0.0011       |  | k_re= 0.1108 +/- 0.0009      |  |
| k_im= -0.0112 +/- 0.0010     |  | k_im= -0.0102 +/- 0.0009      |  | k_im= -0.0081 +/- 0.0007     |  |
| corr= [ 0.42]                |  | corr= [ 0.41]                 |  | corr= [ 0.40]                |  |
| g = 0.0016 +/- 0.0049        |  | g = 0.0317 +/- 0.0071         |  | g = 0.0863 +/- 0.0033        |  |
| arg(g)/pi= 0.1610 +/- 0.3690 |  | arg(g)/pi= -0.1160 +/- 0.0146 |  | arg(g)/pi= 0.9181 +/- 0.0183 |  |
| g_re= 0.0014 +/- 0.0035      |  | g_re= 0.0296 +/- 0.0067       |  | g_re= -0.0835 +/- 0.0032     |  |
| g_im= 0.0008 +/- 0.0039      |  | g_im= -0.0113 +/- 0.0028      |  | g_im= 0.0220 +/- 0.0050      |  |
| corr= [ 0.99]                |  | corr= [-0.83]                 |  | corr= [ 0.04]                |  |

\*\*\*\*\*

```

*****
JP=2+ || eta:eta/1^D_2[-] kaon:kaon/1^D_2[-] pi:pi/1^D_2[-]

```

```

sqrt(s)_pole = (0.28348 +/- 0.001413)
               + (i/2)*(-0.0086427 +/- 0.0024817) [-0.38]

```

| eta:eta/1^D_2                |  | kaon:kaon/1^D_2               |  | pi:pi/1^D_2                  |  |
|------------------------------|--|-------------------------------|--|------------------------------|--|
| k_re= 0.0967 +/- 0.0010      |  | k_re= 0.1034 +/- 0.0010       |  | k_re= 0.1238 +/- 0.0008      |  |
| k_im= -0.0032 +/- 0.0009     |  | k_im= -0.0030 +/- 0.0008      |  | k_im= -0.0025 +/- 0.0007     |  |
| corr= [-0.38]                |  | corr= [-0.38]                 |  | corr= [-0.38]                |  |
| g = 0.0092 +/- 0.0072        |  | g = 0.0549 +/- 0.0083         |  | g = 0.0146 +/- 0.0036        |  |
| arg(g)/pi= 0.4229 +/- 0.0488 |  | arg(g)/pi= -0.0513 +/- 0.0276 |  | arg(g)/pi= 0.1554 +/- 0.1871 |  |
| g_re= 0.0022 +/- 0.0018      |  | g_re= 0.0542 +/- 0.0078       |  | g_re= 0.0129 +/- 0.0050      |  |
| g_im= 0.0090 +/- 0.0071      |  | g_im= -0.0088 +/- 0.0056      |  | g_im= 0.0068 +/- 0.0078      |  |
| corr= [ 0.66]                |  | corr= [-0.69]                 |  | corr= [-0.63]                |  |

\*\*\*\*\*

# k\_2poles\_xxxxxc

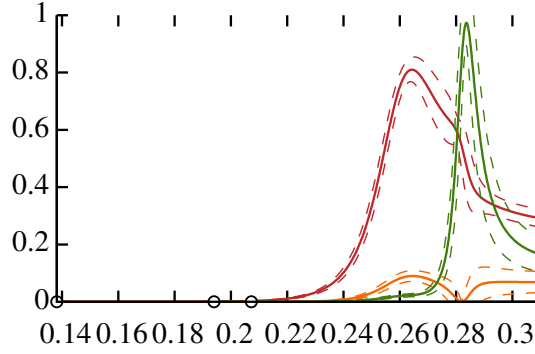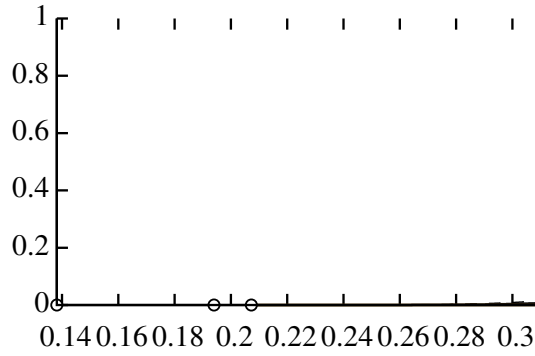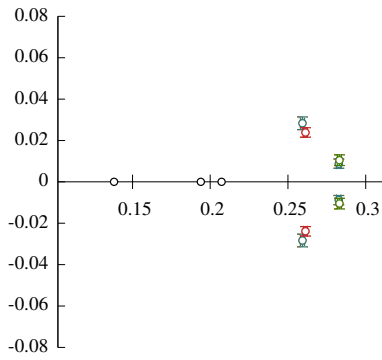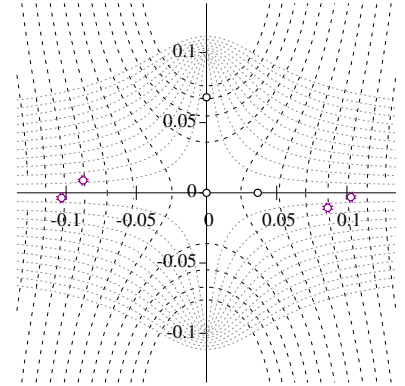

## parameter values

minimised with chisq/nDoF = 29.45 / (34 - 7) = 1.09

|                                               |                       |      |      |       |       |       |       |       |
|-----------------------------------------------|-----------------------|------|------|-------|-------|-------|-------|-------|
| JP2+_g_kaon:kaon/1^D_2_pole0                  | -1.0741 +/- 0.15654   | 1.00 | 0.17 | -0.20 | -0.08 | 0.01  | 0.22  | 0.38  |
| JP2+_g_kaon:kaon/1^D_2_pole1                  | 1.4593 +/- 0.2346     | 1.00 | 0.53 | -0.82 | 0.18  | 0.47  | 0.51  |       |
| JP2+_g_pi:pi/1^D_2_pole0                      | 1.8096 +/- 0.078596   |      | 1.00 | -0.62 | 0.12  | 0.39  | 0.01  |       |
| JP2+_g_pi:pi/1^D_2_pole1                      | -0.11870 +/- 0.27544  |      |      | 1.00  | -0.22 | -0.55 | -0.19 |       |
| JP2+_gamma_eta:eta/1^D_2 eta:eta/1^D_2_order0 | 40.046 +/- 24.512     |      |      |       | 1.00  | -0.08 | -0.08 |       |
| JP2+_m_pole0                                  | 0.26415 +/- 0.0015188 |      |      |       |       | 1.00  | 0.39  |       |
| JP2+_m_pole1                                  | 0.28352 +/- 0.0013639 |      |      |       |       |       | 1.00  |       |
| JP2+_g_eta:eta/1^D_2_pole0                    | 0.0000 +/- 0          |      |      |       |       |       |       | FIXED |
| JP2+_g_eta:eta/1^D_2_pole1                    | 0.0000 +/- 0          |      |      |       |       |       |       | FIXED |
| JP2+_gamma_eta:eta/1^D_2 kaon:kaon/1^D_2_orde | 0.0000 +/- 0          |      |      |       |       |       |       | FIXED |
| JP2+_gamma_eta:eta/1^D_2 pi:pi/1^D_2_order0   | 0.0000 +/- 0          |      |      |       |       |       |       | FIXED |
| JP2+_gamma_kaon:kaon/1^D_2 kaon:kaon/1^D_2_or | 0.0000 +/- 0          |      |      |       |       |       |       | FIXED |
| JP2+_gamma_kaon:kaon/1^D_2 pi:pi/1^D_2_order0 | 0.0000 +/- 0          |      |      |       |       |       |       | FIXED |
| JP2+_gamma_pi:pi/1^D_2 pi:pi/1^D_2_order0     | 0.0000 +/- 0          |      |      |       |       |       |       | FIXED |

## pole singularities

\*\*\*\*\*

\*\*\*\*\*

JP=2+ || eta:eta/1^D\_2[+] kaon:kaon/1^D\_2[+] pi:pi/1^D\_2[-]

sqrt(s)\_pole = (0.26125 +/- 0.0012331)  
+ (i/2)\*(-0.023887 +/- 0.0022774) [-0.31]

| eta:eta/1^D_2             | kaon:kaon/1^D_2               | pi:pi/1^D_2                  |
|---------------------------|-------------------------------|------------------------------|
| k_re= -0.0799 +/- 0.0010  | k_re= -0.0878 +/- 0.0009      | k_re= 0.1109 +/- 0.0007      |
| k_im= 0.0098 +/- 0.0009   | k_im= 0.0089 +/- 0.0008       | k_im= -0.0070 +/- 0.0007     |
| corr= [-0.30]             | corr= [-0.30]                 | corr= [-0.31]                |
| g = 0.0000 +/- nan        | g = 0.0319 +/- 0.0049         | g = 0.0888 +/- 0.0039        |
| arg(g)/pi= 0.0000 +/- nan | arg(g)/pi= -0.1135 +/- 0.0173 | arg(g)/pi= 0.9166 +/- 0.0068 |
| g_re= 0.0000 +/- 0.0000   | g_re= 0.0299 +/- 0.0049       | g_re= -0.0858 +/- 0.0034     |
| g_im= 0.0000 +/- 0.0000   | g_im= -0.0111 +/- 0.0019      | g_im= 0.0230 +/- 0.0028      |
| corr= [ 0.00]             | corr= [-0.51]                 | corr= [-0.92]                |

\*\*\*\*\*



\*\*\*\*\*  
JP=2+ || eta:eta/1^D\_2[+] kaon:kaon/1^D\_2[-] pi:pi/1^D\_2[+]

sqrt(s)\_pole = (0.28312 +/- 0.0012977)  
+ (i/2)\*(-0.010478 +/- 0.0025876) [-0.61]

| eta:eta/1^D_2 |                    |  | kaon:kaon/1^D_2 |                    |  | pi:pi/1^D_2 |                    |  |
|---------------|--------------------|--|-----------------|--------------------|--|-------------|--------------------|--|
| k_re=         | -0.0965 +/- 0.0010 |  | k_re=           | 0.1032 +/- 0.0009  |  | k_re=       | -0.1236 +/- 0.0007 |  |
| k_im=         | 0.0038 +/- 0.0009  |  | k_im=           | -0.0036 +/- 0.0009 |  | k_im=       | 0.0030 +/- 0.0007  |  |
| corr=         | [-0.60]            |  | corr=           | [-0.61]            |  | corr=       | [-0.61]            |  |
| -----         |                    |  |                 |                    |  |             |                    |  |
| g =           | 0.0000 +/- nan     |  | g =             | 0.0661 +/- 0.0087  |  | g =         | 0.0174 +/- 0.0069  |  |
| arg(g)/pi=    | 0.0000 +/- nan     |  | arg(g)/pi=      | -0.0611 +/- 0.0132 |  | arg(g)/pi=  | 0.8357 +/- 0.1884  |  |
| -----         |                    |  |                 |                    |  |             |                    |  |
| g_re=         | 0.0000 +/- 0.0000  |  | g_re=           | 0.0649 +/- 0.0085  |  | g_re=       | -0.0152 +/- 0.0108 |  |
| g_im=         | 0.0000 +/- 0.0000  |  | g_im=           | -0.0126 +/- 0.0033 |  | g_im=       | 0.0086 +/- 0.0061  |  |
| corr=         | [ 0.00]            |  | corr=           | [-0.56]            |  | corr=       | [ 0.88]            |  |

\*\*\*\*\*

\*\*\*\*\*  
JP=2+ || eta:eta/1^D\_2[+] kaon:kaon/1^D\_2[-] pi:pi/1^D\_2[-]

sqrt(s)\_pole = (0.25935 +/- 0.0013291)  
+ (i/2)\*(-0.028313 +/- 0.0030811) [-0.06]

| eta:eta/1^D_2 |                    |  | kaon:kaon/1^D_2 |                    |  | pi:pi/1^D_2 |                    |  |
|---------------|--------------------|--|-----------------|--------------------|--|-------------|--------------------|--|
| k_re=         | -0.0785 +/- 0.0011 |  | k_re=           | 0.0864 +/- 0.0010  |  | k_re=       | 0.1098 +/- 0.0008  |  |
| k_im=         | 0.0117 +/- 0.0013  |  | k_im=           | -0.0106 +/- 0.0011 |  | k_im=       | -0.0084 +/- 0.0009 |  |
| corr=         | [-0.09]            |  | corr=           | [-0.08]            |  | corr=       | [-0.07]            |  |
| -----         |                    |  |                 |                    |  |             |                    |  |
| g =           | 0.0000 +/- nan     |  | g =             | 0.0352 +/- 0.0054  |  | g =         | 0.0849 +/- 0.0042  |  |
| arg(g)/pi=    | 0.0000 +/- nan     |  | arg(g)/pi=      | -0.1136 +/- 0.0144 |  | arg(g)/pi=  | 0.8933 +/- 0.0119  |  |
| -----         |                    |  |                 |                    |  |             |                    |  |
| g_re=         | 0.0000 +/- 0.0000  |  | g_re=           | 0.0330 +/- 0.0049  |  | g_re=       | -0.0802 +/- 0.0030 |  |
| g_im=         | 0.0000 +/- 0.0000  |  | g_im=           | -0.0123 +/- 0.0027 |  | g_im=       | 0.0280 +/- 0.0043  |  |
| corr=         | [ 0.00]            |  | corr=           | [-0.79]            |  | corr=       | [-0.88]            |  |

\*\*\*\*\*

\*\*\*\*\*  
JP=2+ || eta:eta/1^D\_2[+] kaon:kaon/1^D\_2[-] pi:pi/1^D\_2[-]

sqrt(s)\_pole = ( 0.2827 +/- 0.001429)  
+ (i/2)\*(-0.0088138 +/- 0.0022255) [-0.17]

| eta:eta/1^D_2 |                    |  | kaon:kaon/1^D_2 |                    |  | pi:pi/1^D_2 |                    |  |
|---------------|--------------------|--|-----------------|--------------------|--|-------------|--------------------|--|
| k_re=         | -0.0961 +/- 0.0011 |  | k_re=           | 0.1029 +/- 0.0010  |  | k_re=       | 0.1233 +/- 0.0008  |  |
| k_im=         | 0.0032 +/- 0.0008  |  | k_im=           | -0.0030 +/- 0.0008 |  | k_im=       | -0.0025 +/- 0.0006 |  |
| corr=         | [-0.16]            |  | corr=           | [-0.16]            |  | corr=       | [-0.16]            |  |
| -----         |                    |  |                 |                    |  |             |                    |  |
| g =           | 0.0000 +/- nan     |  | g =             | 0.0555 +/- 0.0066  |  | g =         | 0.0171 +/- 0.0064  |  |
| arg(g)/pi=    | 0.0000 +/- nan     |  | arg(g)/pi=      | -0.0795 +/- 0.0313 |  | arg(g)/pi=  | 0.3059 +/- 0.1522  |  |
| -----         |                    |  |                 |                    |  |             |                    |  |
| g_re=         | 0.0000 +/- 0.0000  |  | g_re=           | 0.0537 +/- 0.0059  |  | g_re=       | 0.0098 +/- 0.0039  |  |
| g_im=         | 0.0000 +/- 0.0000  |  | g_im=           | -0.0137 +/- 0.0062 |  | g_im=       | 0.0140 +/- 0.0096  |  |
| corr=         | [ 0.00]            |  | corr=           | [-0.49]            |  | corr=       | [-0.75]            |  |

\*\*\*\*\*

\*\*\*\*\*  
JP=2+ || eta:eta/1^D\_2[-] kaon:kaon/1^D\_2[+] pi:pi/1^D\_2[-]

sqrt(s)\_pole = (0.26125 +/- 0.0012331)  
+ (i/2)\*(-0.023887 +/- 0.0022774) [-0.31]

| eta:eta/1^D_2 |                    |  | kaon:kaon/1^D_2 |                    |  | pi:pi/1^D_2 |                    |  |
|---------------|--------------------|--|-----------------|--------------------|--|-------------|--------------------|--|
| k_re=         | 0.0799 +/- 0.0010  |  | k_re=           | -0.0878 +/- 0.0009 |  | k_re=       | 0.1109 +/- 0.0007  |  |
| k_im=         | -0.0098 +/- 0.0009 |  | k_im=           | 0.0089 +/- 0.0008  |  | k_im=       | -0.0070 +/- 0.0007 |  |
| corr=         | [-0.30]            |  | corr=           | [-0.30]            |  | corr=       | [-0.31]            |  |
| -----         |                    |  |                 |                    |  |             |                    |  |
| g =           | 0.0000 +/- nan     |  | g =             | 0.0319 +/- 0.0049  |  | g =         | 0.0888 +/- 0.0039  |  |
| arg(g)/pi=    | 0.0000 +/- nan     |  | arg(g)/pi=      | -0.1135 +/- 0.0173 |  | arg(g)/pi=  | 0.9166 +/- 0.0068  |  |
| -----         |                    |  |                 |                    |  |             |                    |  |
| g_re=         | 0.0000 +/- 0.0000  |  | g_re=           | 0.0299 +/- 0.0049  |  | g_re=       | -0.0858 +/- 0.0034 |  |
| g_im=         | 0.0000 +/- 0.0000  |  | g_im=           | -0.0111 +/- 0.0019 |  | g_im=       | 0.0230 +/- 0.0028  |  |
| corr=         | [ 0.00]            |  | corr=           | [-0.51]            |  | corr=       | [-0.92]            |  |

\*\*\*\*\*

\*\*\*\*\*  
JP=2+ || eta:eta/1^D\_2[-] kaon:kaon/1^D\_2[-] pi:pi/1^D\_2[+]

sqrt(s)\_pole = (0.28312 +/- 0.0012977)  
+ (i/2)\*(-0.010478 +/- 0.0025876) [-0.61]

| eta:eta/1^D_2 |                    |  | kaon:kaon/1^D_2 |                    |  | pi:pi/1^D_2 |                    |  |
|---------------|--------------------|--|-----------------|--------------------|--|-------------|--------------------|--|
| k_re=         | 0.0965 +/- 0.0010  |  | k_re=           | 0.1032 +/- 0.0009  |  | k_re=       | -0.1236 +/- 0.0007 |  |
| k_im=         | -0.0038 +/- 0.0009 |  | k_im=           | -0.0036 +/- 0.0009 |  | k_im=       | 0.0030 +/- 0.0007  |  |
| corr=         | [-0.60]            |  | corr=           | [-0.61]            |  | corr=       | [-0.61]            |  |
| -----         |                    |  |                 |                    |  |             |                    |  |
| g =           | 0.0000 +/- nan     |  | g =             | 0.0661 +/- 0.0087  |  | g =         | 0.0174 +/- 0.0069  |  |
| arg(g)/pi=    | 0.0000 +/- nan     |  | arg(g)/pi=      | -0.0611 +/- 0.0132 |  | arg(g)/pi=  | 0.8357 +/- 0.1884  |  |
| -----         |                    |  |                 |                    |  |             |                    |  |
| g_re=         | 0.0000 +/- 0.0000  |  | g_re=           | 0.0649 +/- 0.0085  |  | g_re=       | -0.0152 +/- 0.0108 |  |
| g_im=         | 0.0000 +/- 0.0000  |  | g_im=           | -0.0126 +/- 0.0033 |  | g_im=       | 0.0086 +/- 0.0061  |  |

```

corr= [ 0.00] | corr= [-0.56] | corr= [ 0.88] |
*****

```

```

*****
JP=2+ || eta:eta/1^D_2[-] kaon:kaon/1^D_2[-] pi:pi/1^D_2[-]

```

```

sqrt(s)_pole = (0.25935 +/- 0.0013291)
               + (i/2)*(-0.028313 +/- 0.0030811) [-0.06]

```

| eta:eta/1^D_2             |  | kaon:kaon/1^D_2               |  | pi:pi/1^D_2                  |  |
|---------------------------|--|-------------------------------|--|------------------------------|--|
| k_re= 0.0785 +/- 0.0011   |  | k_re= 0.0864 +/- 0.0010       |  | k_re= 0.1098 +/- 0.0008      |  |
| k_im= -0.0117 +/- 0.0013  |  | k_im= -0.0106 +/- 0.0011      |  | k_im= -0.0084 +/- 0.0009     |  |
| corr= [-0.09]             |  | corr= [-0.08]                 |  | corr= [-0.07]                |  |
| -----                     |  |                               |  |                              |  |
| g = 0.0000 +/- nan        |  | g = 0.0352 +/- 0.0054         |  | g = 0.0849 +/- 0.0042        |  |
| arg(g)/pi= 0.0000 +/- nan |  | arg(g)/pi= -0.1136 +/- 0.0144 |  | arg(g)/pi= 0.8933 +/- 0.0119 |  |
| -----                     |  |                               |  |                              |  |
| g_re= 0.0000 +/- 0.0000   |  | g_re= 0.0330 +/- 0.0049       |  | g_re= -0.0802 +/- 0.0030     |  |
| g_im= 0.0000 +/- 0.0000   |  | g_im= -0.0123 +/- 0.0027      |  | g_im= 0.0280 +/- 0.0043      |  |
| corr= [ 0.00]             |  | corr= [-0.79]                 |  | corr= [-0.88]                |  |

\*\*\*\*\*

```

*****
JP=2+ || eta:eta/1^D_2[-] kaon:kaon/1^D_2[-] pi:pi/1^D_2[-]

```

```

sqrt(s)_pole = ( 0.2827 +/- 0.001429)
               + (i/2)*(-0.0088138 +/- 0.0022255) [-0.17]

```

| eta:eta/1^D_2             |  | kaon:kaon/1^D_2               |  | pi:pi/1^D_2                  |  |
|---------------------------|--|-------------------------------|--|------------------------------|--|
| k_re= 0.0961 +/- 0.0011   |  | k_re= 0.1029 +/- 0.0010       |  | k_re= 0.1233 +/- 0.0008      |  |
| k_im= -0.0032 +/- 0.0008  |  | k_im= -0.0030 +/- 0.0008      |  | k_im= -0.0025 +/- 0.0006     |  |
| corr= [-0.16]             |  | corr= [-0.16]                 |  | corr= [-0.16]                |  |
| -----                     |  |                               |  |                              |  |
| g = 0.0000 +/- nan        |  | g = 0.0555 +/- 0.0066         |  | g = 0.0171 +/- 0.0064        |  |
| arg(g)/pi= 0.0000 +/- nan |  | arg(g)/pi= -0.0795 +/- 0.0313 |  | arg(g)/pi= 0.3059 +/- 0.1522 |  |
| -----                     |  |                               |  |                              |  |
| g_re= 0.0000 +/- 0.0000   |  | g_re= 0.0537 +/- 0.0059       |  | g_re= 0.0098 +/- 0.0039      |  |
| g_im= 0.0000 +/- 0.0000   |  | g_im= -0.0137 +/- 0.0062      |  | g_im= 0.0140 +/- 0.0096      |  |
| corr= [ 0.00]             |  | corr= [-0.49]                 |  | corr= [-0.75]                |  |

\*\*\*\*\*

# k\_2poles\_xxxxxc\_noCM

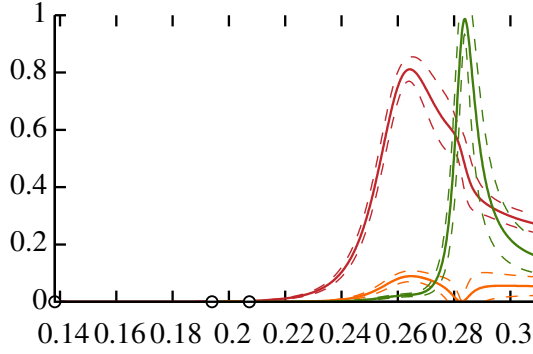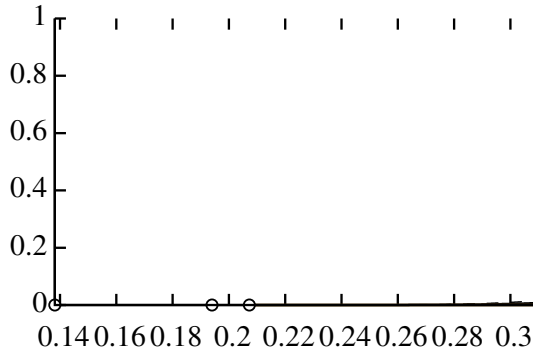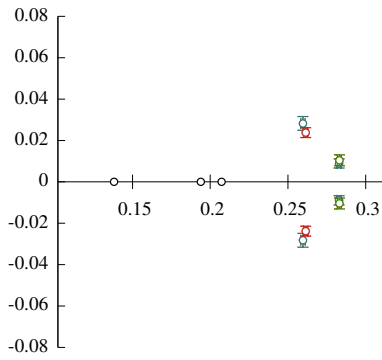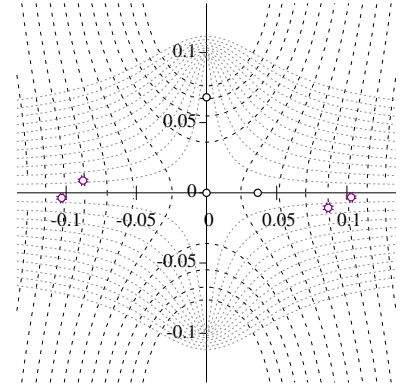

## parameter values

minimised with  $\text{chisq}/\text{nDoF} = 28.87 / (34 - 7) = 1.07$

|                                               |                       |      |      |       |       |       |       |       |
|-----------------------------------------------|-----------------------|------|------|-------|-------|-------|-------|-------|
| JP2+_g_kaon:kaon/1^D_2_pole0                  | -1.0955 +/- 0.16096   | 1.00 | 0.11 | -0.24 | 0.02  | 0.02  | 0.10  | 0.34  |
| JP2+_g_kaon:kaon/1^D_2_pole1                  | 1.4951 +/- 0.25028    | 1.00 | 0.56 | -0.83 | 0.15  | 0.48  | 0.54  |       |
| JP2+_g_pi:pi/1^D_2_pole0                      | 1.8529 +/- 0.087575   |      | 1.00 | -0.66 | 0.09  | 0.47  | 0.05  |       |
| JP2+_g_pi:pi/1^D_2_pole1                      | -0.11366 +/- 0.28875  |      |      | 1.00  | -0.18 | -0.57 | -0.21 |       |
| JP2+_gamma_eta:eta/1^D_2 eta:eta/1^D_2_order0 | 40.565 +/- 24.362     |      |      |       | 1.00  | -0.11 | -0.08 |       |
| JP2+_m_pole0                                  | 0.26416 +/- 0.0016932 |      |      |       |       | 1.00  | 0.36  |       |
| JP2+_m_pole1                                  | 0.28405 +/- 0.0014789 |      |      |       |       |       | 1.00  |       |
| JP2+_g_eta:eta/1^D_2_pole0                    | 0.0000 +/- 0          |      |      |       |       |       |       | FIXED |
| JP2+_g_eta:eta/1^D_2_pole1                    | 0.0000 +/- 0          |      |      |       |       |       |       | FIXED |
| JP2+_gamma_eta:eta/1^D_2 kaon:kaon/1^D_2_orde | 0.0000 +/- 0          |      |      |       |       |       |       | FIXED |
| JP2+_gamma_eta:eta/1^D_2 pi:pi/1^D_2_order0   | 0.0000 +/- 0          |      |      |       |       |       |       | FIXED |
| JP2+_gamma_kaon:kaon/1^D_2 kaon:kaon/1^D_2_or | 0.0000 +/- 0          |      |      |       |       |       |       | FIXED |
| JP2+_gamma_kaon:kaon/1^D_2 pi:pi/1^D_2_order0 | 0.0000 +/- 0          |      |      |       |       |       |       | FIXED |
| JP2+_gamma_pi:pi/1^D_2 pi:pi/1^D_2_order0     | 0.0000 +/- 0          |      |      |       |       |       |       | FIXED |

## pole singularities

\*\*\*\*\*

\*\*\*\*\*  
JP=2+ || eta:eta/1^D\_2[+] kaon:kaon/1^D\_2[+] pi:pi/1^D\_2[-]

sqrt(s)\_pole = (0.26146 +/- 0.001383)  
+ (i/2)\*(-0.023804 +/- 0.0024011) [-0.44]

| eta:eta/1^D_2             | kaon:kaon/1^D_2               | pi:pi/1^D_2                  |
|---------------------------|-------------------------------|------------------------------|
| k_re= -0.0800 +/- 0.0012  | k_re= -0.0879 +/- 0.0010      | k_re= 0.1111 +/- 0.0008      |
| k_im= 0.0097 +/- 0.0009   | k_im= 0.0088 +/- 0.0009       | k_im= -0.0070 +/- 0.0007     |
| corr= [-0.42]             | corr= [-0.42]                 | corr= [-0.43]                |
| g = 0.0000 +/- nan        | g = 0.0315 +/- 0.0051         | g = 0.0889 +/- 0.0042        |
| arg(g)/pi= 0.0000 +/- nan | arg(g)/pi= -0.1117 +/- 0.0180 | arg(g)/pi= 0.9206 +/- 0.0066 |
| g_re= 0.0000 +/- 0.0000   | g_re= 0.0296 +/- 0.0051       | g_re= -0.0862 +/- 0.0037     |
| g_im= 0.0000 +/- 0.0000   | g_im= -0.0108 +/- 0.0018      | g_im= 0.0220 +/- 0.0027      |
| corr= [ 0.00]             | corr= [-0.46]                 | corr= [-0.92]                |

\*\*\*\*\*

\*\*\*\*\*  
JP=2+ || eta:eta/1^D\_2[+] kaon:kaon/1^D\_2[-] pi:pi/1^D\_2[+]

sqrt(s)\_pole = (0.28309 +/- 0.0012858)  
+ (i/2)\*(-0.010433 +/- 0.0026159) [-0.58]

| eta:eta/1^D_2 |                    |  | kaon:kaon/1^D_2 |                    |  | pi:pi/1^D_2 |                    |  |
|---------------|--------------------|--|-----------------|--------------------|--|-------------|--------------------|--|
| k_re=         | -0.0964 +/- 0.0010 |  | k_re=           | 0.1031 +/- 0.0009  |  | k_re=       | -0.1236 +/- 0.0007 |  |
| k_im=         | 0.0038 +/- 0.0009  |  | k_im=           | -0.0036 +/- 0.0009 |  | k_im=       | 0.0030 +/- 0.0007  |  |
| corr=         | [-0.58]            |  | corr=           | [-0.58]            |  | corr=       | [-0.58]            |  |
| g =           | 0.0000 +/- nan     |  | g =             | 0.0656 +/- 0.0085  |  | g =         | 0.0160 +/- 0.0058  |  |
| arg(g)/pi=    | 0.0000 +/- nan     |  | arg(g)/pi=      | -0.0615 +/- 0.0117 |  | arg(g)/pi=  | 0.7998 +/- 0.2090  |  |
| g_re=         | 0.0000 +/- 0.0000  |  | g_re=           | 0.0644 +/- 0.0082  |  | g_re=       | -0.0129 +/- 0.0105 |  |
| g_im=         | 0.0000 +/- 0.0000  |  | g_im=           | -0.0126 +/- 0.0031 |  | g_im=       | 0.0094 +/- 0.0057  |  |
| corr=         | [ 0.00]            |  | corr=           | [-0.61]            |  | corr=       | [ 0.89]            |  |

\*\*\*\*\*

\*\*\*\*\*  
JP=2+ || eta:eta/1^D\_2[+] kaon:kaon/1^D\_2[-] pi:pi/1^D\_2[-]

sqrt(s)\_pole = (0.25964 +/- 0.001381)  
+ (i/2)\*(-0.028238 +/- 0.0033231) [-0.23]

| eta:eta/1^D_2 |                    |  | kaon:kaon/1^D_2 |                    |  | pi:pi/1^D_2 |                    |  |
|---------------|--------------------|--|-----------------|--------------------|--|-------------|--------------------|--|
| k_re=         | -0.0787 +/- 0.0012 |  | k_re=           | 0.0867 +/- 0.0010  |  | k_re=       | 0.1100 +/- 0.0008  |  |
| k_im=         | 0.0116 +/- 0.0013  |  | k_im=           | -0.0106 +/- 0.0012 |  | k_im=       | -0.0083 +/- 0.0010 |  |
| corr=         | [-0.26]            |  | corr=           | [-0.25]            |  | corr=       | [-0.24]            |  |
| g =           | 0.0000 +/- nan     |  | g =             | 0.0351 +/- 0.0059  |  | g =         | 0.0854 +/- 0.0046  |  |
| arg(g)/pi=    | 0.0000 +/- nan     |  | arg(g)/pi=      | -0.1086 +/- 0.0142 |  | arg(g)/pi=  | 0.8981 +/- 0.0118  |  |
| g_re=         | 0.0000 +/- 0.0000  |  | g_re=           | 0.0330 +/- 0.0054  |  | g_re=       | -0.0810 +/- 0.0034 |  |
| g_im=         | 0.0000 +/- 0.0000  |  | g_im=           | -0.0117 +/- 0.0027 |  | g_im=       | 0.0269 +/- 0.0043  |  |
| corr=         | [ 0.00]            |  | corr=           | [-0.78]            |  | corr=       | [-0.92]            |  |

\*\*\*\*\*

\*\*\*\*\*  
JP=2+ || eta:eta/1^D\_2[+] kaon:kaon/1^D\_2[-] pi:pi/1^D\_2[-]

sqrt(s)\_pole = (0.28287 +/- 0.0014221)  
+ (i/2)\*(-0.0088936 +/- 0.0022128) [-0.22]

| eta:eta/1^D_2 |                    |  | kaon:kaon/1^D_2 |                    |  | pi:pi/1^D_2 |                    |  |
|---------------|--------------------|--|-----------------|--------------------|--|-------------|--------------------|--|
| k_re=         | -0.0963 +/- 0.0010 |  | k_re=           | 0.1030 +/- 0.0010  |  | k_re=       | 0.1234 +/- 0.0008  |  |
| k_im=         | 0.0033 +/- 0.0008  |  | k_im=           | -0.0031 +/- 0.0008 |  | k_im=       | -0.0025 +/- 0.0006 |  |
| corr=         | [-0.21]            |  | corr=           | [-0.21]            |  | corr=       | [-0.21]            |  |
| g =           | 0.0000 +/- nan     |  | g =             | 0.0561 +/- 0.0068  |  | g =         | 0.0161 +/- 0.0055  |  |
| arg(g)/pi=    | 0.0000 +/- nan     |  | arg(g)/pi=      | -0.0740 +/- 0.0297 |  | arg(g)/pi=  | 0.2831 +/- 0.1708  |  |
| g_re=         | 0.0000 +/- 0.0000  |  | g_re=           | 0.0546 +/- 0.0061  |  | g_re=       | 0.0101 +/- 0.0041  |  |
| g_im=         | 0.0000 +/- 0.0000  |  | g_im=           | -0.0129 +/- 0.0060 |  | g_im=       | 0.0125 +/- 0.0094  |  |
| corr=         | [ 0.00]            |  | corr=           | [-0.53]            |  | corr=       | [-0.79]            |  |

\*\*\*\*\*

\*\*\*\*\*  
JP=2+ || eta:eta/1^D\_2[-] kaon:kaon/1^D\_2[+] pi:pi/1^D\_2[-]

sqrt(s)\_pole = (0.26146 +/- 0.001383)  
+ (i/2)\*(-0.023804 +/- 0.0024011) [-0.44]

| eta:eta/1^D_2 |                    |  | kaon:kaon/1^D_2 |                    |  | pi:pi/1^D_2 |                    |  |
|---------------|--------------------|--|-----------------|--------------------|--|-------------|--------------------|--|
| k_re=         | 0.0800 +/- 0.0012  |  | k_re=           | -0.0879 +/- 0.0010 |  | k_re=       | 0.1111 +/- 0.0008  |  |
| k_im=         | -0.0097 +/- 0.0009 |  | k_im=           | 0.0088 +/- 0.0009  |  | k_im=       | -0.0070 +/- 0.0007 |  |
| corr=         | [-0.42]            |  | corr=           | [-0.42]            |  | corr=       | [-0.43]            |  |
| g =           | 0.0000 +/- nan     |  | g =             | 0.0315 +/- 0.0051  |  | g =         | 0.0889 +/- 0.0042  |  |
| arg(g)/pi=    | 0.0000 +/- nan     |  | arg(g)/pi=      | -0.1117 +/- 0.0180 |  | arg(g)/pi=  | 0.9206 +/- 0.0066  |  |
| g_re=         | 0.0000 +/- 0.0000  |  | g_re=           | 0.0296 +/- 0.0051  |  | g_re=       | -0.0862 +/- 0.0037 |  |
| g_im=         | 0.0000 +/- 0.0000  |  | g_im=           | -0.0108 +/- 0.0018 |  | g_im=       | 0.0220 +/- 0.0027  |  |
| corr=         | [ 0.00]            |  | corr=           | [-0.46]            |  | corr=       | [-0.92]            |  |

\*\*\*\*\*

\*\*\*\*\*  
JP=2+ || eta:eta/1^D\_2[-] kaon:kaon/1^D\_2[-] pi:pi/1^D\_2[+]

sqrt(s)\_pole = (0.28309 +/- 0.0012858)  
+ (i/2)\*(-0.010433 +/- 0.0026159) [-0.58]

| eta:eta/1^D_2 |                    |  | kaon:kaon/1^D_2 |                    |  | pi:pi/1^D_2 |                    |  |
|---------------|--------------------|--|-----------------|--------------------|--|-------------|--------------------|--|
| k_re=         | 0.0964 +/- 0.0010  |  | k_re=           | 0.1031 +/- 0.0009  |  | k_re=       | -0.1236 +/- 0.0007 |  |
| k_im=         | -0.0038 +/- 0.0009 |  | k_im=           | -0.0036 +/- 0.0009 |  | k_im=       | 0.0030 +/- 0.0007  |  |
| corr=         | [-0.58]            |  | corr=           | [-0.58]            |  | corr=       | [-0.58]            |  |
| g =           | 0.0000 +/- nan     |  | g =             | 0.0656 +/- 0.0085  |  | g =         | 0.0160 +/- 0.0058  |  |
| arg(g)/pi=    | 0.0000 +/- nan     |  | arg(g)/pi=      | -0.0615 +/- 0.0117 |  | arg(g)/pi=  | 0.7998 +/- 0.2090  |  |
| g_re=         | 0.0000 +/- 0.0000  |  | g_re=           | 0.0644 +/- 0.0082  |  | g_re=       | -0.0129 +/- 0.0105 |  |
| g_im=         | 0.0000 +/- 0.0000  |  | g_im=           | -0.0126 +/- 0.0031 |  | g_im=       | 0.0094 +/- 0.0057  |  |

```

corr= [ 0.00] | corr= [-0.61] | corr= [ 0.89] |
*****

```

```

*****
JP=2+ || eta:eta/1^D_2[-] kaon:kaon/1^D_2[-] pi:pi/1^D_2[-]

```

```

sqrt(s)_pole = (0.25964 +/- 0.001381)
+ (i/2)*(-0.028238 +/- 0.0033231) [-0.23]

```

```

=====
eta:eta/1^D_2 | kaon:kaon/1^D_2 | pi:pi/1^D_2 |
=====
k_re= 0.0787 +/- 0.0012 | k_re= 0.0867 +/- 0.0010 | k_re= 0.1100 +/- 0.0008 |
k_im= -0.0116 +/- 0.0013 | k_im= -0.0106 +/- 0.0012 | k_im= -0.0083 +/- 0.0010 |
corr= [-0.26] | corr= [-0.25] | corr= [-0.24] |
=====
|g|= 0.0000 +/- nan | |g|= 0.0351 +/- 0.0059 | |g|= 0.0854 +/- 0.0046 |
arg(g)/pi= 0.0000 +/- nan | arg(g)/pi= -0.1086 +/- 0.0142 | arg(g)/pi= 0.8981 +/- 0.0118 |
=====
g_re= 0.0000 +/- 0.0000 | g_re= 0.0330 +/- 0.0054 | g_re= -0.0810 +/- 0.0034 |
g_im= 0.0000 +/- 0.0000 | g_im= -0.0117 +/- 0.0027 | g_im= 0.0269 +/- 0.0043 |
corr= [ 0.00] | corr= [-0.78] | corr= [-0.92] |
=====

```

```

*****
JP=2+ || eta:eta/1^D_2[-] kaon:kaon/1^D_2[-] pi:pi/1^D_2[-]

```

```

sqrt(s)_pole = (0.28287 +/- 0.0014221)
+ (i/2)*(-0.0088936 +/- 0.0022128) [-0.22]

```

```

=====
eta:eta/1^D_2 | kaon:kaon/1^D_2 | pi:pi/1^D_2 |
=====
k_re= 0.0963 +/- 0.0010 | k_re= 0.1030 +/- 0.0010 | k_re= 0.1234 +/- 0.0008 |
k_im= -0.0033 +/- 0.0008 | k_im= -0.0031 +/- 0.0008 | k_im= -0.0025 +/- 0.0006 |
corr= [-0.21] | corr= [-0.21] | corr= [-0.21] |
=====
|g|= 0.0000 +/- nan | |g|= 0.0561 +/- 0.0068 | |g|= 0.0161 +/- 0.0055 |
arg(g)/pi= 0.0000 +/- nan | arg(g)/pi= -0.0740 +/- 0.0297 | arg(g)/pi= 0.2831 +/- 0.1708 |
=====
g_re= 0.0000 +/- 0.0000 | g_re= 0.0546 +/- 0.0061 | g_re= 0.0101 +/- 0.0041 |
g_im= 0.0000 +/- 0.0000 | g_im= -0.0129 +/- 0.0060 | g_im= 0.0125 +/- 0.0094 |
corr= [ 0.00] | corr= [-0.53] | corr= [-0.79] |
=====

```

# k\_2poles\_xxxxxs\_noCM

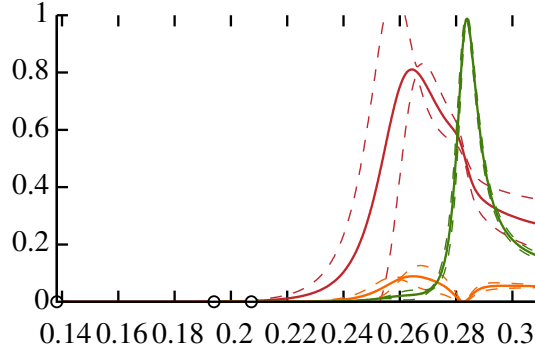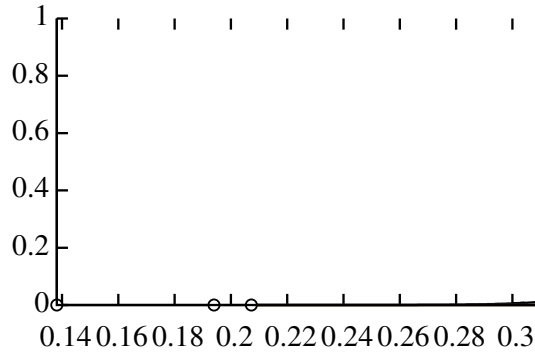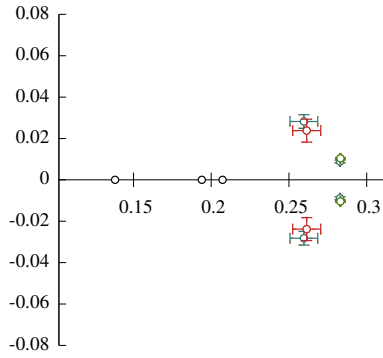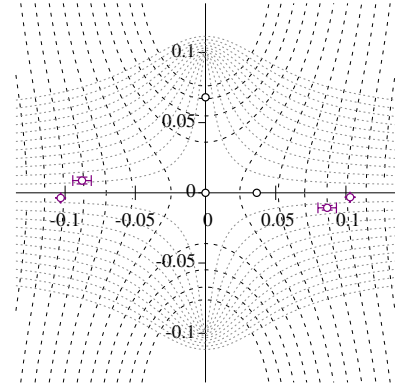

## parameter values

minimised with  $\text{chisq}/\text{nDoF} = 28.60 / (34 - 7) = 1.06$

|                                               |                        |      |       |       |       |       |       |      |
|-----------------------------------------------|------------------------|------|-------|-------|-------|-------|-------|------|
| JP2+_g_kaon:kaon/1^D_2_pole0                  | -1.0935 +/- 0.040448   | 1.00 | -0.26 | -0.48 | -0.17 | -0.14 | 0.48  | 0.30 |
| JP2+_g_kaon:kaon/1^D_2_pole1                  | 1.4955 +/- 0.028877    | 1.00 | 0.54  | 0.15  | 0.16  | -0.54 | -0.29 |      |
| JP2+_g_pi:pi/1^D_2_pole0                      | 1.8527 +/- 0.32039     | 1.00 | 0.34  | 0.29  | -1.00 | -0.59 |       |      |
| JP2+_g_pi:pi/1^D_2_pole1                      | -0.11513 +/- 0.031789  | 1.00 | 0.09  | -0.34 | -0.18 |       |       |      |
| JP2+_gamma_eta:eta/1^D_2 eta:eta/1^D_2_order1 | 519.59 +/- 74.526      |      |       |       | 1.00  | -0.29 | -0.18 |      |
| JP2+_m_pole0                                  | 0.26414 +/- 0.007068   |      |       |       | 1.00  | 0.59  |       |      |
| JP2+_m_pole1                                  | 0.28404 +/- 0.00028966 |      |       |       |       | 1.00  |       |      |
| JP2+_g_eta:eta/1^D_2_pole0                    | 0.0000 +/- 0           |      |       |       |       |       |       |      |
| JP2+_g_eta:eta/1^D_2_pole1                    | 0.0000 +/- 0           |      |       |       |       |       |       |      |
| JP2+_gamma_eta:eta/1^D_2 eta:eta/1^D_2_order0 | 0.0000 +/- 0           |      |       |       |       |       |       |      |
| JP2+_gamma_eta:eta/1^D_2 kaon:kaon/1^D_2_orde | 0.0000 +/- 0           |      |       |       |       |       |       |      |
| JP2+_gamma_eta:eta/1^D_2 kaon:kaon/1^D_2_orde | 0.0000 +/- 0           |      |       |       |       |       |       |      |
| JP2+_gamma_eta:eta/1^D_2 pi:pi/1^D_2_order0   | 0.0000 +/- 0           |      |       |       |       |       |       |      |
| JP2+_gamma_eta:eta/1^D_2 pi:pi/1^D_2_order1   | 0.0000 +/- 0           |      |       |       |       |       |       |      |
| JP2+_gamma_kaon:kaon/1^D_2 kaon:kaon/1^D_2_or | 0.0000 +/- 0           |      |       |       |       |       |       |      |
| JP2+_gamma_kaon:kaon/1^D_2 kaon:kaon/1^D_2_or | 0.0000 +/- 0           |      |       |       |       |       |       |      |
| JP2+_gamma_kaon:kaon/1^D_2 pi:pi/1^D_2_order0 | 0.0000 +/- 0           |      |       |       |       |       |       |      |
| JP2+_gamma_kaon:kaon/1^D_2 pi:pi/1^D_2_order1 | 0.0000 +/- 0           |      |       |       |       |       |       |      |
| JP2+_gamma_pi:pi/1^D_2 pi:pi/1^D_2_order0     | 0.0000 +/- 0           |      |       |       |       |       |       |      |
| JP2+_gamma_pi:pi/1^D_2 pi:pi/1^D_2_order1     | 0.0000 +/- 0           |      |       |       |       |       |       |      |

## pole singularities

\*\*\*\*\*

JP=2+ || eta:eta/1^D\_2[+] kaon:kaon/1^D\_2[+] pi:pi/1^D\_2[-]

$\text{sqrt}(s)_{\text{pole}} = (0.26144 \pm 0.0090323) + (i/2) * (-0.023794 \pm 0.0055301) [1.00]$

| eta:eta/1^D_2                 | kaon:kaon/1^D_2               | pi:pi/1^D_2                   |
|-------------------------------|-------------------------------|-------------------------------|
| k_re= -0.0800 +/- 0.0071      | k_re= -0.0879 +/- 0.0066      | k_re= 0.1110 +/- 0.0053       |
| k_im= 0.0097 +/- 0.0028       | k_im= 0.0088 +/- 0.0024       | k_im= -0.0070 +/- 0.0017      |
| corr= [ 1.00]                 | corr= [ 1.00]                 | corr= [ 1.00]                 |
| g = 0.0000 +/- 0.0000         | g = 0.0314 +/- 0.0036         | g = 0.0889 +/- 0.0065         |
| arg(g)/pi= -0.0920 +/- 0.0799 | arg(g)/pi= -0.1116 +/- 0.0244 | arg(g)/pi= -0.0794 +/- 0.0223 |

```

-----|-----|-----|
g_re= 0.0000 +/- 0.0000 | g_re= 0.0295 +/- 0.0042 | g_re= 0.0861 +/- 0.0048 |
g_im= -0.0000 +/- 0.0000 | g_im= -0.0108 +/- 0.0011 | g_im= -0.0219 +/- 0.0076 |
corr= [ 0.13] | corr= [ 0.87] | corr= [-1.00] |
*****

```

```

*****
JP=2+ || eta:eta/1^D_2[+] kaon:kaon/1^D_2[-] pi:pi/1^D_2[+]

```

```

sqrt(s)_pole = (0.28308 +/- 0.00029539)
+ (i/2)*(-0.010429 +/- 0.00036421) [ 0.27]

```

```

eta:eta/1^D_2 | kaon:kaon/1^D_2 | pi:pi/1^D_2 |
-----|-----|-----|
k_re= -0.0964 +/- 0.0002 | k_re= 0.1031 +/- 0.0002 | k_re= -0.1236 +/- 0.0002 |
k_im= 0.0038 +/- 0.0001 | k_im= -0.0036 +/- 0.0001 | k_im= 0.0030 +/- 0.0001 |
corr= [ 0.29] | corr= [ 0.29] | corr= [ 0.28] |
-----|-----|-----|
|g|= 0.0000 +/- 0.0000 | |g|= 0.0656 +/- 0.0011 | |g|= 0.0159 +/- 0.0023 |
arg(g)/pi= -0.0373 +/- 0.0809 | arg(g)/pi= -0.0613 +/- 0.0042 | arg(g)/pi= -0.1989 +/- 0.0235 |
-----|-----|-----|
g_re= 0.0000 +/- 0.0000 | g_re= 0.0644 +/- 0.0010 | g_re= 0.0129 +/- 0.0021 |
g_im= -0.0000 +/- 0.0000 | g_im= -0.0126 +/- 0.0010 | g_im= -0.0093 +/- 0.0015 |
corr= [-0.03] | corr= [-0.78] | corr= [-0.54] |
*****

```

```

*****
JP=2+ || eta:eta/1^D_2[+] kaon:kaon/1^D_2[-] pi:pi/1^D_2[-]

```

```

sqrt(s)_pole = (0.25963 +/- 0.0089313)
+ (i/2)*(-0.028218 +/- 0.0033161) [ 1.00]

```

```

eta:eta/1^D_2 | kaon:kaon/1^D_2 | pi:pi/1^D_2 |
-----|-----|-----|
k_re= -0.0787 +/- 0.0071 | k_re= 0.0867 +/- 0.0066 | k_re= 0.1100 +/- 0.0052 |
k_im= 0.0116 +/- 0.0020 | k_im= -0.0106 +/- 0.0017 | k_im= -0.0083 +/- 0.0011 |
corr= [ 1.00] | corr= [ 1.00] | corr= [ 1.00] |
-----|-----|-----|
|g|= 0.0000 +/- 0.0000 | |g|= 0.0350 +/- 0.0072 | |g|= 0.0854 +/- 0.0057 |
arg(g)/pi= -0.1104 +/- 0.0899 | arg(g)/pi= -0.1084 +/- 0.0359 | arg(g)/pi= -0.1018 +/- 0.0142 |
-----|-----|-----|
g_re= 0.0000 +/- 0.0000 | g_re= 0.0330 +/- 0.0081 | g_re= 0.0810 +/- 0.0042 |
g_im= -0.0000 +/- 0.0000 | g_im= -0.0117 +/- 0.0014 | g_im= -0.0268 +/- 0.0054 |
corr= [ 0.03] | corr= [ 0.90] | corr= [-1.00] |
*****

```

```

*****
JP=2+ || eta:eta/1^D_2[+] kaon:kaon/1^D_2[-] pi:pi/1^D_2[-]

```

```

sqrt(s)_pole = (0.28286 +/- 0.00025502)
+ (i/2)*(-0.0088937 +/- 0.00068262) [ 0.21]

```

```

eta:eta/1^D_2 | kaon:kaon/1^D_2 | pi:pi/1^D_2 |
-----|-----|-----|
k_re= -0.0963 +/- 0.0002 | k_re= 0.1030 +/- 0.0002 | k_re= 0.1234 +/- 0.0001 |
k_im= 0.0033 +/- 0.0003 | k_im= -0.0031 +/- 0.0002 | k_im= -0.0025 +/- 0.0002 |
corr= [ 0.19] | corr= [ 0.20] | corr= [ 0.20] |
-----|-----|-----|
|g|= 0.0000 +/- 0.0000 | |g|= 0.0561 +/- 0.0028 | |g|= 0.0161 +/- 0.0029 |
arg(g)/pi= -0.0330 +/- 0.0790 | arg(g)/pi= -0.0740 +/- 0.0125 | arg(g)/pi= 0.2847 +/- 0.0235 |
-----|-----|-----|
g_re= 0.0000 +/- 0.0000 | g_re= 0.0546 +/- 0.0032 | g_re= 0.0101 +/- 0.0021 |
g_im= -0.0000 +/- 0.0000 | g_im= -0.0129 +/- 0.0016 | g_im= 0.0125 +/- 0.0023 |
corr= [-0.05] | corr= [ 0.88] | corr= [ 0.70] |
*****

```

```

*****
JP=2+ || eta:eta/1^D_2[-] kaon:kaon/1^D_2[+] pi:pi/1^D_2[-]

```

```

sqrt(s)_pole = (0.26144 +/- 0.0090323)
+ (i/2)*(-0.023794 +/- 0.0055301) [ 1.00]

```

```

eta:eta/1^D_2 | kaon:kaon/1^D_2 | pi:pi/1^D_2 |
-----|-----|-----|
k_re= 0.0800 +/- 0.0071 | k_re= -0.0879 +/- 0.0066 | k_re= 0.1110 +/- 0.0053 |
k_im= -0.0097 +/- 0.0028 | k_im= 0.0088 +/- 0.0024 | k_im= -0.0070 +/- 0.0017 |
corr= [ 1.00] | corr= [ 1.00] | corr= [ 1.00] |
-----|-----|-----|
|g|= 0.0000 +/- 0.0000 | |g|= 0.0314 +/- 0.0036 | |g|= 0.0889 +/- 0.0065 |
arg(g)/pi= -0.0876 +/- 0.0865 | arg(g)/pi= -0.1116 +/- 0.0244 | arg(g)/pi= -0.0794 +/- 0.0223 |
-----|-----|-----|
g_re= 0.0000 +/- 0.0000 | g_re= 0.0295 +/- 0.0042 | g_re= 0.0861 +/- 0.0048 |
g_im= -0.0000 +/- 0.0000 | g_im= -0.0108 +/- 0.0011 | g_im= -0.0219 +/- 0.0076 |
corr= [ 0.13] | corr= [ 0.87] | corr= [-1.00] |
*****

```

```

*****
JP=2+ || eta:eta/1^D_2[-] kaon:kaon/1^D_2[-] pi:pi/1^D_2[+]

```

```

sqrt(s)_pole = (0.28308 +/- 0.00029539)
+ (i/2)*(-0.010429 +/- 0.00036421) [ 0.27]

```

```

eta:eta/1^D_2 | kaon:kaon/1^D_2 | pi:pi/1^D_2 |
-----|-----|-----|
k_re= 0.0964 +/- 0.0002 | k_re= 0.1031 +/- 0.0002 | k_re= -0.1236 +/- 0.0002 |
k_im= -0.0038 +/- 0.0001 | k_im= -0.0036 +/- 0.0001 | k_im= 0.0030 +/- 0.0001 |
corr= [ 0.29] | corr= [ 0.29] | corr= [ 0.28] |

```

```

=====|=====|=====|
|g|= 0.0000 +/- 0.0000 | |g|= 0.0656 +/- 0.0011 | |g|= 0.0159 +/- 0.0023 |
arg(g)/pi= -0.0243 +/- 0.0814 |arg(g)/pi= -0.0613 +/- 0.0042 |arg(g)/pi= -0.1989 +/- 0.0235 |
-----|-----|-----|
g_re= 0.0000 +/- 0.0000 | g_re= 0.0644 +/- 0.0010 | g_re= 0.0129 +/- 0.0021 |
g_im= -0.0000 +/- 0.0000 | g_im= -0.0126 +/- 0.0010 | g_im= -0.0093 +/- 0.0015 |
corr= [ 0.03] | corr= [-0.78] | corr= [-0.54] |
*****

```

```

*****
JP=2+ || eta:eta/1^D_2[-] kaon:kaon/1^D_2[-] pi:pi/1^D_2[-]

```

```

sqrt(s)_pole = (0.25963 +/- 0.0089313)
+ (i/2)*(-0.028218 +/- 0.0033161) [ 1.00]

```

```

eta:eta/1^D_2 | kaon:kaon/1^D_2 | pi:pi/1^D_2 |
=====|=====|=====|
k_re= 0.0787 +/- 0.0071 | k_re= 0.0867 +/- 0.0066 | k_re= 0.1100 +/- 0.0052 |
k_im= -0.0116 +/- 0.0020 | k_im= -0.0106 +/- 0.0017 | k_im= -0.0083 +/- 0.0011 |
corr= [ 1.00] | corr= [ 1.00] | corr= [ 1.00] |
-----|-----|-----|
|g|= 0.0000 +/- 0.0000 | |g|= 0.0350 +/- 0.0072 | |g|= 0.0854 +/- 0.0057 |
arg(g)/pi= -0.1068 +/- 0.0861 |arg(g)/pi= -0.1084 +/- 0.0359 |arg(g)/pi= -0.1018 +/- 0.0142 |
-----|-----|-----|
g_re= 0.0000 +/- 0.0000 | g_re= 0.0330 +/- 0.0081 | g_re= 0.0810 +/- 0.0042 |
g_im= -0.0000 +/- 0.0000 | g_im= -0.0117 +/- 0.0014 | g_im= -0.0268 +/- 0.0054 |
corr= [ 0.17] | corr= [ 0.90] | corr= [-1.00] |
*****

```

```

*****
JP=2+ || eta:eta/1^D_2[-] kaon:kaon/1^D_2[-] pi:pi/1^D_2[-]

```

```

sqrt(s)_pole = (0.28286 +/- 0.00025502)
+ (i/2)*(-0.0088937 +/- 0.00068262) [ 0.21]

```

```

eta:eta/1^D_2 | kaon:kaon/1^D_2 | pi:pi/1^D_2 |
=====|=====|=====|
k_re= 0.0963 +/- 0.0002 | k_re= 0.1030 +/- 0.0002 | k_re= 0.1234 +/- 0.0001 |
k_im= -0.0033 +/- 0.0003 | k_im= -0.0031 +/- 0.0002 | k_im= -0.0025 +/- 0.0002 |
corr= [ 0.19] | corr= [ 0.20] | corr= [ 0.20] |
-----|-----|-----|
|g|= 0.0000 +/- 0.0000 | |g|= 0.0561 +/- 0.0028 | |g|= 0.0161 +/- 0.0029 |
arg(g)/pi= -0.0198 +/- 0.0793 |arg(g)/pi= -0.0740 +/- 0.0125 |arg(g)/pi= 0.2847 +/- 0.0235 |
-----|-----|-----|
g_re= 0.0000 +/- 0.0000 | g_re= 0.0546 +/- 0.0032 | g_re= 0.0101 +/- 0.0021 |
g_im= -0.0000 +/- 0.0000 | g_im= -0.0129 +/- 0.0016 | g_im= 0.0125 +/- 0.0023 |
corr= [-0.04] | corr= [ 0.88] | corr= [ 0.70] |
*****

```
